# Supplementary material for: Proofs of life: molecular-biology reasoning simulates cell behaviors from first principles
Source: arXiv:1811.02478 ancillary file (2019-03-18)
Supplement: Supplementary file 1 [file supplementary.pdf]

Proofs of life: molecular-biology reasoning  
simulates cell behaviors from first principles  
(*supplementary text*)

René Vestergaard\*

March 18, 2019

## S1 CEq theory: ab-intra structure

Formal proofs are tree structures that are built according to a system of rules that define the permitted steps of reasoning. A logic, i.e., a theory of properties enjoying certain properties of its own, see Section S1.3.2, is often axiomatized by a formal proof system but may also be defined in other ways. The proof systems in Sections S1.1–S1.2 are said to be in *natural deduction* style: we state how to introduce and eliminate each logical connective. The choice of proof rules is dictated by the intended usages and the ability to prove desired results about all proofs and/or the axiomatized logic, e.g., consistency. Such results are known as *meta-theory*: theory about theory. Formal proofs differ from (Boolean) truth tables, say. Truth tables provide a semantics for ‘classical’ propositional logic: a propositional formula is classically provable if and only if it evaluates to true across its entire truth table. We focus on issues related to axiomatizations rather than just what is being axiomatized: 1) the process and benefits of making a detailed case for something, 2) *verification*, of rule compliance, 3) subtler distinctions than truth in ‘intuitionistic’ propositional logic in order to guarantee *constructivity*: the ability to decompose any proof of a compound formula into proofs of constituent formulas that can be recomposed to establish the compound formula, and (briefly) 4) extensibility, for application purposes.

We present only strictly-necessary motivation. See main body for discussion. See Section S2 for usage. The material in Sections S1.1–S1.2 and Lemmas S26,S27 provides background and is not new.

---

\*Corresponding author: [renevestergaard@acm.org](mailto:renevestergaard@acm.org)

## S1.1 Background: formal reasoning

We present the necessary logic background for the CEq framework.

### S1.1.1 Inductive definitions

The key technology behind formal proof systems is inductive definitions, a mature and active research area in its own right: what styles guarantee well-formedness, and more? An inductive definition is a type of axiomatization that often shows how to assemble the entities of interest. We use only the most basic of inductive definitions, and informal motivation suffices.

The inductive-definition archetype is the natural numbers. Informally, the natural numbers are 0, 1, 2, and so on. An inductive definition is precise also about “and so on”. We can think of the definition we give as being of the least set that contains a constant for zero and is closed under a successor function. Formally, we write the following, where ‘ $::=$ ’ (“is inductively defined by”) and ‘ $|$ ’ (separating possibilities) are part of the inductive-definition meta-language:

$$\text{Nat} ::= \text{zero} \mid \text{succ}(\text{Nat})$$

In the terminology, **zero** and **succ** are *constructors* of **Nat**, the first-principle natural numbers. The constructors take none and one **Nat** arguments and produce a **Nat**. This is the right-to-left reading of the definition. The left-to-right reading says that nothing else is a **Nat**. An example **Nat** is **succ(succ(zero))**. The way to think about the definition is that it introduces three new symbols: **Nat**, **zero**, and **succ**, and stipulates how they relate to each other. Nothing beyond the symbols and their relationships is assumed, may be used, or is necessary. In particular, **zero** is not 0 and **succ** is not +1, or anything seemingly more concrete than the given first-principle form: the more recognizable concepts are less precise than ours.

We occasionally write inductive definitions as ‘proof rules’, e.g., for ‘ $: \text{Nat}$ ’ (“is a **Nat**”), where  $n$  and the horizontal line (“from [top] conclude [bottom]”) are meta-language:

$$\frac{}{\text{zero} : \text{Nat}} \qquad \frac{n : \text{Nat}}{\text{succ}(n) : \text{Nat}}$$

We need proof-rule style, e.g., for things that are not constructor-based or if we need several ingoing things to be the same: this will be indicated by multiple occurrences of  $n$ , say.

Inductively defining a formal proof system involves a binary relation, often written ‘ $\vdash$ ’ (turnstile), between a collection of *assumptions*, ranged over by  $\Gamma$ , and what can be established as following from there. When defining **Nat**, our

meta-language automatically provides us with the following in return:

$$\frac{\Gamma \vdash q[\mathbf{zero}] \quad \Gamma, q[m] \vdash q[\mathbf{succ}(m)]}{\Gamma \vdash \forall n \in \mathbf{Nat} . q[n]} \quad \begin{array}{l} \mathbf{Plus}(\mathbf{zero}, k) \doteq k \\ \mathbf{Plus}(\mathbf{succ}(m), k) \doteq \mathbf{succ}(\mathbf{Plus}(m, k)) \end{array}$$

**left** a *structural-induction* rule to prove that some  $q$  with holes for a  $\mathbf{Nat}$  (the ‘ $q[\cdot]$ ’ notation) will hold for all  $\mathbf{Nats}$ : ‘ $\forall n \in \mathbf{Nat} . \_$ ’ is ( $\mathbf{Nat}$ -)bounded universal quantification.

**right** the ability to define ( $\doteq$ ) functions over  $\mathbf{Nats}$  by *structural recursion*.

Structural induction for  $\mathbf{Nat}$  is also known as (weak) number induction and should be familiar to all: if you prove base and step cases, you have proved something that holds for everything considered. Structural recursion behaves the same as structural induction: following  $\mathbf{Nat}$ ’s structure, with the only difference being that recursion may produce values of an arbitrary sort rather than specifically the sort we use for things that are subject to being proved, see Section S1.2. The universal quantification on the left corresponds to totality on the right:  $\mathbf{Plus}$  is guaranteed to produce a result for any  $\mathbf{Nat}$  given as first argument. Both induction and recursion allow us to assume that we know the relevant outcomes for any sub-terms: the induction hypotheses vs the recursive calls.

With the above, we would then develop everything we want to know about the natural numbers. This implies that the specific definition given for a concept may be more or less useful. In some cases, multiple definitions are made, proved equivalent, and used in different circumstances. In a few cases, an inductive definition precisely captures years of experience and, in effect, marks the difference between impenetrable and fully-resolved for a given subject matter.

### S1.1.2 Propositional proofs

Propositional logic is defined over a language of ‘formulas’ by means of a binary relation:  $\vdash$ . Here,  $\vdash$  relates a collection of formulas on its left, the *assumptions*, to a single formula on the right, the *consequence*. We inductively define intuitionistic provability by a collection of *proof rules* below: a collection of provability relationships above a horizontal line, the *premises*, and a single provability relationship below the line, the *conclusion*. These relationships should be understood as patterns in the meta-language that must be instantiated in the object language when used, e.g.,  $\mathbf{succ}(n)$  vs  $\mathbf{succ}(\mathbf{zero})$ . The proof rules are used to build *derivations*: a derivation starts from a rule without premises (like  $\mathbf{zero}$  in Section S1.1.1), aka *axioms*, and proceeds downwards by composing already-constructed derivations whose final conclusions match the patterns in the premises of a given rule (like  $\mathbf{succ}$  in Section S1.1.1). This includes respecting overlaps between patterns and instantiating the pattern in the conclusion. Viewed in the upwards direction, premises are possible proof obligations for a given conclusion. We often refer to the final conclusion as the *conclusion of*

a *derivation*. A derivation whose conclusion has an empty set of assumptions is called a *proof*. The consequence in the conclusion of a proof is said to be a *theorem* of the considered proof system. We write  $\vdash p$  if  $p$  is a theorem of  $\vdash$ .

**Definition S1 (Propositional formulas)** Consider a set of variable names,  $\mathcal{V}$ , ranged over by  $v$ , and let  $\mathbf{F}$  be a constant (to represent false — to be defined, by proof rules). Let the (propositional) formulas be any variable or  $\mathbf{F}$ , and let them be closed under conjunction ( $\wedge$ ), disjunction ( $\vee$ ), and implication ( $\rightarrow$ ):

$$P ::= \mathcal{V} \mid \mathbf{F} \mid P \wedge P \mid P \vee P \mid P \rightarrow P$$

Let  $p$  range over  $P$ , write  $\neg p$  for  $p \rightarrow \mathbf{F}$  (non-primitive negation), indicate scope with parentheses, e.g.,  $v_a \rightarrow (\mathbf{F} \rightarrow v_b)$  vs  $(v_a \rightarrow \mathbf{F}) \rightarrow v_b$ , and write  $v_a \rightarrow \mathbf{F} \rightarrow v_b$  to mean  $v_a \rightarrow (\mathbf{F} \rightarrow v_b)$ .

**Definition S2 (Intuitionistic logic)** Let  $\Gamma$  range over collections of formulas. Define intuitionistic logic,  $\vdash$ , by allowing assumptions to be used freely; so all bets are off if false can be established; and by introducing: ( $I_-$ ), and eliminating: ( $E_-$ ), the formula connectives:

$$\begin{array}{c} \frac{}{\Gamma_1, p, \Gamma_2 \vdash p} (Assm) \quad \frac{\Gamma \vdash \mathbf{F}}{\Gamma \vdash p} (E_{\mathbf{F}}) \\[10pt] \frac{\Gamma \vdash p_l \quad \Gamma \vdash p_r}{\Gamma \vdash p_l \wedge p_r} (I_{\wedge}) \quad \frac{\Gamma \vdash p_l \wedge p_r}{\Gamma \vdash p_l} (E_{\wedge}^l) \quad \frac{\Gamma \vdash p_l \wedge p_r}{\Gamma \vdash p_r} (E_{\wedge}^r) \\[10pt] \frac{\Gamma \vdash p_l}{\Gamma \vdash p_l \vee p_r} (I_{\vee}) \quad \frac{\Gamma \vdash p_r}{\Gamma \vdash p_l \vee p_r} (I_{\vee}^r) \\[10pt] \frac{\Gamma \vdash p_l \vee p_r \quad \Gamma, p_l \vdash p \quad \Gamma, p_r \vdash p}{\Gamma \vdash p} (E_{\vee}) \\[10pt] \frac{\Gamma_1, p_a, \Gamma_2 \vdash p_b}{\Gamma_1, \Gamma_2 \vdash p_a \rightarrow p_b} (I_{\rightarrow}) \quad \frac{\Gamma \vdash p_a \rightarrow p_b \quad \Gamma \vdash p_a}{\Gamma \vdash p_b} (E_{\rightarrow}) \end{array}$$

Rule ( $E_{\mathbf{F}}$ ) is also called *ex falso quodlibet* ('from false, whatever pleases'); there is no ( $I_{\mathbf{F}}$ ) rule (but see proof of Theorem S3). Note the near-symmetry between the ( $I_-$ ) and ( $E_-$ ) rules for  $\vee$  vs  $\wedge$  — the symmetry is perfect in other presentations.

Intuitionistic logic will serve as a main reference point for our discussion of molecular-biology reasoning. See Section S1.1.6 for the precise definition of classical logic (of truth-table-semantics fame). Intuitionistic logic makes subtler distinctions than classical logic. For example,  $p \rightarrow \neg\neg p$  and  $\neg\neg p \rightarrow p$  both evaluate to true whether  $p$  is true or false in a truth table, implying that both are classical theorems. Only the former is an intuitionistic theorem.

**Theorem S3** For any  $p$ :

$$\vdash p \rightarrow \neg\neg p$$

**Proof:** Formula  $p \rightarrow \neg\neg p$  written in full is  $p \rightarrow ((p \rightarrow \mathbf{F}) \rightarrow \mathbf{F})$ .

$$\frac{\frac{\frac{}{p, \neg p \vdash p \rightarrow \mathbf{F}} (Assm) \quad \frac{}{p, \neg p \vdash p} (Assm)}{p, \neg p \vdash \mathbf{F}} (E_{\rightarrow})}{\frac{p, \neg p \vdash \mathbf{F}}{p \vdash \neg\neg p} (I_{\rightarrow})} (I_{\rightarrow})$$

See also supporting file `coext.v`. Instead of the other direction, we can prove that intuitionistic double-negation is a particular form of “absence of counter-examples”.

**Theorem S4** *For any  $p$ , if we have established the double-negation of  $p$  then the fact of a forced choice between  $p$  or a counter-example to  $p$  means we have established  $p$ , and vice versa:*

$$\vdash \neg\neg p \rightarrow ((p \vee \neg p) \rightarrow p) \quad \wedge \quad ((p \vee \neg p) \rightarrow p) \rightarrow \neg\neg p$$

**Proof:** We prove the two conjuncts separately, per  $(I_{\wedge})$  — the two vertical lines are informal notation to tie the derivations together, for horizontal space:

$$\frac{\frac{\frac{}{\neg\neg p, p \vee \neg p, \neg p \vdash \neg p \rightarrow \mathbf{F}} (Assm) \quad \frac{}{\neg\neg p, p \vee \neg p, \neg p \vdash \neg p} (Assm)}{\neg\neg p, p \vee \neg p, \neg p \vdash \mathbf{F}} (E_{\rightarrow})}{\frac{\neg\neg p, p \vee \neg p, \neg p \vdash \mathbf{F}}{\neg\neg p, p \vee \neg p, \neg p \vdash p} (E_{\mathbf{F}})} (E_{\vee})$$

$$\frac{\frac{\frac{}{\neg\neg p, p \vee \neg p \vdash p \vee \neg p} (Assm) \quad \frac{}{\neg\neg p, p \vee \neg p, p \vdash p} (Assm)}{\neg\neg p, p \vee \neg p \vdash p} (E_{\vee})}{\frac{\neg\neg p, p \vee \neg p \vdash p}{\neg\neg p \vdash (p \vee \neg p) \rightarrow p} (I_{\rightarrow})} (I_{\rightarrow})$$

$$\vdash \neg\neg p \rightarrow ((p \vee \neg p) \rightarrow p)$$

$$\frac{\frac{\frac{}{\neg p, (p \vee \neg p) \rightarrow p \vdash (p \vee \neg p) \rightarrow p} (Assm) \quad \frac{\frac{}{\neg p, (p \vee \neg p) \rightarrow p \vdash \neg p} (Assm)}{\neg p, (p \vee \neg p) \rightarrow p \vdash p \vee \neg p} (I_{\vee})}{\neg p, (p \vee \neg p) \rightarrow p \vdash p} (E_{\rightarrow})}{\neg p, (p \vee \neg p) \rightarrow p \vdash p} (E_{\rightarrow})$$

$$\frac{\frac{\frac{}{\neg p, (p \vee \neg p) \rightarrow p \vdash p \rightarrow \mathbf{F}} (Assm)}{\neg p, (p \vee \neg p) \rightarrow p \vdash \mathbf{F}} (E_{\rightarrow})}{\frac{\neg p, (p \vee \neg p) \rightarrow p \vdash \mathbf{F}}{(p \vee \neg p) \rightarrow p \vdash \neg p \rightarrow \mathbf{F}} (I_{\rightarrow})} (I_{\rightarrow})$$

$$\vdash ((p \vee \neg p) \rightarrow p) \rightarrow \neg\neg p$$

See also supporting file `coext.v`.

### S1.1.3 Verification

In general, it may be hard to arrive at a proof but subsequent checking tends to be simpler. In the formal case, checking is also called verification. Specifically, verification is the process of going through derivations, like those above, horizontal line by horizontal line and ensuring that each complies with a proof rule, here from Definition S2. The process is typically sufficiently simple that we can have high confidence in well-written verification software and, if need be, can typically program a verifier ourselves. One view on formal reasoning is that it shifts nearly the full checking burden to the proof developer in return for tool support for development and assuredness at all granularities, including some notion of certification in many cases.

### S1.1.4 Meta-theory: consistency

The first thing we typically want to prove for a formal proof system is that it is consistent: there is no  $p$  such that both  $p$  and  $\neg p$  are theorems of the system. An alternative formulation of consistency is:  $\mathbf{F}$  is not a theorem of the system. Some languages of formulas do not allow for one or both of these definitions and a third formulation is that not all formulas are theorems of the system. The last property is typically said to establish that the considered system is *non-trivial* in the sense that it makes distinctions, whatever they may be. The three properties are equivalent for most systems that can express them, including for intuitionistic logic, see  $(E_{\rightarrow})$  and  $(E_F)$ .

If we consider only derivations with no occurrences of  $(E_{\rightarrow})$  with an  $(I_{\rightarrow})$  in their left premise (and similar constraints for the other connectives), we can prove *the sub-formula property*: all formulas inside a derivation will occur in its conclusion. In the forbidden scenario,  $p_a$  may violate the sub-formula constraint:

$$\frac{\frac{\frac{\vdots \pi_b}{\Gamma_1, p_a, \Gamma_2 \vdash p_b} (I_{\rightarrow})}{\Gamma_1, \Gamma_2 \vdash p_a \rightarrow p_b} \quad \frac{\vdots \pi_a}{\Gamma_1, \Gamma_2 \vdash p_a} (E_{\rightarrow})}{\Gamma_1, \Gamma_2 \vdash p_b} (E_{\rightarrow})$$

The sub-formula property implies consistency of the relevant logic fragment:  $\mathbf{F}$  has no (strict) sub-formulas, i.e., no constrained proof can establish  $\mathbf{F}$ .<sup>1</sup>

### S1.1.5 Proof theory: proof reading

When trying to understand how we arrived at  $p_b$  from  $\Gamma_1, \Gamma_2$  above, we can take  $p_a \rightarrow p_b$  as a lemma, as done above. Alternatively, we can start tracing  $p_a$ -connections through  $\pi_b$ . This is the starting point of proof theory. In this case,

<sup>1</sup> $\mathbf{F}$  is a sub-formula of itself, meaning there may be a possible proof ending with an occurrence of  $(E_F)$  but that would have to be preceded by an occurrence of  $(E_F)$ , etc., which cannot be a proof: all derivations are finite.

we can do away with the assumed  $p_a$  throughout  $\pi_b$  by plugging (adaptations of) derivation  $\pi_a$ , ending in  $\Gamma_1, \Gamma_2 \vdash p_a$ , in for the relevant (*Assm*) occurrences:

$$\begin{array}{c} \vdots \pi'_a \qquad \qquad \qquad \vdots \pi''_a \\ \Gamma_1, \Gamma_2, \Gamma' \vdash p_a \qquad \Gamma_1, \Gamma_2, \Gamma'' \vdash p_a \\ \vdots \pi_b^- \\ \Gamma_1, \Gamma_2 \vdash p_b \end{array}$$

This will have the effect of duplicating some rule occurrences but it also removes the two we consider above, along with the relevant (*Assm*) occurrences, and it results in a derivation with the same conclusion as we started from. We can prove that repeating this process for pairs of rule occurrences for all connectives always terminates for  $\vdash$ , meaning an arbitrary derivation can be transformed into one with the same conclusion that enjoys the sub-formula property, implying that the whole logic is consistent: **F** is not a  $\vdash$ -theorem. More generally, the outlined process establishes how to read the proofs in a mathematical sense. The reading reflects the inner structure of the axiomatization: its geometry.

### S1.1.6 Classical vs intuitionistic logic

While  $p$  and  $\neg\neg p$  are equivalent in classical but not in intuitionistic logic,  $\neg p$  and  $\neg\neg\neg p$  (and deeper negation pairs) are equivalent in both, for any  $p$ . More, Glivenko's Theorem says that  $p$  is provable in classical logic if and only if  $\neg\neg p$  is provable in intuitionistic logic, implying that intuitionistic logic retains 'truth' as a notion but makes subtler distinctions for non-double-negated formulas. In fact, classical logic is obtained by collapsing the subtler intuitionistic distinctions in the following sense.

**Theorem S5** *Classical logic (the logic of truth tables) can be equivalently defined as reductio ad absurdum (RAA), double-negation elimination (DNE), or the law of excluded middle (LEM) plus each their copies of the rules of intuitionistic logic, see Definition S2:*

$$\frac{\Gamma_1, \neg p, \Gamma_2 \vdash^{\bullet'} \mathbf{F}}{\Gamma_1, \Gamma_2 \vdash^{\bullet'} p} (RAA) \qquad \frac{}{\Gamma \vdash^{\bullet''} \neg\neg p \rightarrow p} (DNE) \qquad \frac{}{\Gamma \vdash^{\bullet'''} p \vee \neg p} (LEM)$$

*To be explicit:  $\vdash^{\bullet'}$ ,  $\vdash^{\bullet''}$ , and  $\vdash^{\bullet'''}$  are new provability relations defined by the listed rule and copies of the rules in Definition S2 with the respective marks added. We will write  $\vdash^{\bullet}$  if we care only about the axiomatized relationships and not the specific axiomatization.*

The classical (*RAA*) contrasts with the intuitionistic (*E<sub>F</sub>*) of Definition S2: in classical logic, false elimination is strengtened to say that we may have arrived at false by assuming the existence of a counter-example to what we wish to conclude. The intuitionistic (*E<sub>F</sub>*) requires us to ferret out a contradiction among an unchanging set of assumptions, see the proof of Theorem S3. The

classical (*RAA*) allows us to hide a contradictee (e.g., against  $\neg\neg p$ ), meaning the rule makes it look as if we have proof positive for the concluded  $p$  for the remainder of the proof. This is made clear in (*DNE*), which outrightly allows us to conclude that something holds as long as stipulating that it holds does not violate consistency:  $\neg\neg p$  means that  $\neg p$  does not hold in a consistent logic. A related presentation of the extra reasoning allowance in classical logic is provided by (*LEM*): we may explicitly reason in terms of whether something ought to be true or false with no other possibility allowed, where ‘true’ and ‘false’ are notions that are external to the proof system.

For reasons discussed in Section S1.1.9, we note that LEM suffices at the level of variables.

**Lemma S6** *For any  $p$ , with variables in  $p$  ranged over by  $v$ :*

$$\vdash^\bullet p \quad \text{if and only if} \quad \vdash \left( \bigwedge_{v \in p} (v \vee \neg v) \right) \rightarrow p$$

### S1.1.7 Disjunctive normal form

A propositional formula is in disjunctive normal form (DNF) if all disjunctions are outermost and these connect only conjunctions of *literals*: arbitrarily-negated variables. All DNFs are formulas but not vice versa.

**Definition S7 (Disjunctive normal form, DNF)** *Let  $D \subset P$  (Definition S1) be:*

$$\begin{aligned} D &::= C \mid D \vee D \\ C &::= L \mid C \wedge C \\ L &::= \mathcal{V} \mid \neg L \end{aligned}$$

There are different embeddings of  $P$  into  $D$  that respect different notions of provability, i.e., of converting an arbitrary formula into an *equivalent* DNF: the original formula is provable if-and-only-if the DNF is. One method of conversion is to create the truth table for a given formula and construct the canonical DNF with the same truth table from there: for any assignment of truth values to the variables for which the formula evaluates to true, conjunct together the variables that are assigned true and the negations of those that are assigned false, and then disjunct together all the reconstituted cases. This method is the logical form of state-space modeling. It is valid in classical but not in intuitionistic logic. For example,  $\neg(p \wedge \neg p)$  is intuitionistically provable.

**Theorem S8** *For any  $p$ :*

$$\vdash \neg(p \wedge \neg p)$$

**Proof:**

$$\begin{array}{c}
\frac{}{p \wedge \neg p \vdash p \wedge \neg p} (Assm) \quad \frac{}{p \wedge \neg p \vdash p \wedge \neg p} (Assm) \\
\frac{}{p \wedge \neg p \vdash p \wedge \neg p} (E_{\wedge}^r) \quad \frac{}{p \wedge \neg p \vdash p \wedge \neg p} (E_{\wedge}^l) \\
\frac{}{p \wedge \neg p \vdash p \rightarrow \mathbf{F}} (E_{\rightarrow}) \quad \frac{}{p \wedge \neg p \vdash p} (E_{\rightarrow}) \\
\frac{}{p \wedge \neg p \vdash \mathbf{F}} (I_{\rightarrow}) \\
\vdash \neg(p \wedge \neg p)
\end{array}$$

See also supporting file `coext.v`. The formula above is also classically provable: 1) the above is a classical proof when marks are added to the rule names and 2) the formula's truth table lists true everywhere. This means that we are looking at  $p \vee \neg p$  as the truth-table-derived DNF, which is not intuitionistically provable for arbitrary  $p$ .

Instead of using truth tables, we can convert to DNF by ‘distributive laws’:

- $\neg(p_a \wedge p_b) \leftrightarrow (\neg p_a \vee \neg p_b)$
- $\neg(p_a \vee p_b) \leftrightarrow (\neg p_a \wedge \neg p_b)$
- $(p_a \wedge (p_b \vee p_c)) \leftrightarrow ((p_a \wedge p_b) \vee (p_a \wedge p_c))$

Here, ‘ $p_a \leftrightarrow p_b$ ’ is ‘ $(p_a \rightarrow p_b) \wedge (p_b \rightarrow p_a)$ ’. We want to exhaustively apply these left to right: the top two (De Morgan’s Laws) first followed by the bottom one.<sup>2</sup> The laws are classically valid: they connect formulas with identical truth tables. Only five are intuitionistically valid.

**Theorem S9** *For any  $p_a$ ,  $p_b$ , and  $p_c$ :*

$$\begin{array}{l}
\vdash (\neg p_a \vee \neg p_b) \rightarrow \neg(p_a \wedge p_b) \\
\vdash \neg(p_a \vee p_b) \rightarrow (\neg p_a \wedge \neg p_b) \quad \vdash (\neg p_a \wedge \neg p_b) \rightarrow \neg(p_a \vee p_b) \\
\vdash (p_a \wedge (p_b \vee p_c)) \rightarrow ((p_a \wedge p_b) \vee (p_a \wedge p_c)) \quad \vdash ((p_a \wedge p_b) \vee (p_a \wedge p_c)) \rightarrow (p_a \wedge (p_b \vee p_c))
\end{array}$$

**Proof:** See supporting file `coext.v`. The De Morgan Law that introduces a disjunction is not intuitionistically valid:  $\neg(p_a \wedge p_b) \rightarrow \neg p_a \vee \neg p_b$ , and it is one of the “left-to-right” three we would want to use for DNF conversion.

### S1.1.8 De Morgan vs intuitionistic logic

**Theorem S10** *The law of weak excluded middle ( $LwEM$ ) validates the remaining De Morgan’s Law relative to intuitionistic logic — here,  $\vdash^*$  is a new provability relation defined by the following rule and copies of the rules in Definition S2 with  $\star$  added:*

$$\frac{}{\Gamma \vdash^* \neg p \vee \neg \neg p} (LwEM)$$

<sup>2</sup>The bottom one would need to be either in generalized form or used with symmetry:  $p_a \wedge p_b \leftrightarrow p_b \wedge p_a$ .

Specifically, for any  $p_a$  and  $p_b$ :

$$\vdash^* \neg(p_a \wedge p_b) \rightarrow \neg p_a \vee \neg p_b \quad \text{and} \quad \vdash (\neg p_a \vee \neg \neg p_a) \rightarrow \neg(p_a \wedge p_b) \rightarrow (\neg p_a \vee \neg p_b)$$

The theory associated with  $\vdash^*$  is called *De Morgan or Jankov or testability logic*.

**Proof:** See supporting file `coext.v`. The preceding result should be understood in the context of Theorem S5. Similarly, see Lemma S6 for the variable-only scenario and Section S1.1.9:

**Lemma S11 ([17])** *For any  $p$ , with variables in  $p$  ranged over by  $v$ :*

$$\vdash^* p \quad \text{if and only if} \quad \vdash \left( \bigwedge_{v \in p} (\neg v \vee \neg \neg v) \right) \rightarrow p$$

### S1.1.9 The big picture, with real-world considerations

Firstly, intuitionistic is De Morgan is classical provability, but not vice versa:  $\vdash \subset \vdash^* \subset \vdash^\bullet$ . Of these, only intuitionistic logic is constructive: we can decompose any intuitionistic proof of a compound formula to proofs of constituent formulas that can be recomposed to prove the original formula. Classical and De Morgan logic are defined by the rules for intuitionistic logic plus the axioms that  $p \vee \neg p$  (the law of excluded middle, LEM) respectively  $\neg p \vee \neg \neg p$  (the law of weak excluded middle, LwEM) hold for arbitrary formulas,  $p$ . Any specific formula that matches either of these schemas is trivially provable in the relevant logic, by the axiom in question. In intuitionistic logic, a proof will need to prove one of the disjuncts. Constructively,  $p \vee \neg p$  expresses that  $p$  is *decidable* in the technical sense: the establishing proof will prove one or the other thereby deciding  $p$ . Constructively,  $\neg p \vee \neg \neg p$  expresses *testability* of  $p$ : if we “add in”  $p$ , we must be able to detect if that creates a conflict (with  $\neg p$ ) or not ( $\neg \neg p$ ).

There are two aspects of decidability and testability to understand in case of real-world applications. ‘Real-world’ means that some variables within formulas may be designated as being external references and that other formulas may no longer be substituted into the locations where they are used. (1) We must ensure that any extra-logical entities represented by variables that the principles are applied to allow for it: we may not subject a variable representing an undecidable problem to the law of excluded middle, for example. (2) If the principles are applied only to formulas that only contain variables that represent extra-logical entities, we can guarantee that the intra-logical/formalism-bound part of the reasoning is undertaken constructively, see Lemmas S6,S11.

## S1.2 Background: extensible reasoning

We outline one particular way in which the reasoning framework in Section S1.1 can be made practical. Specifically, we show how intuitionistic logic generalizes to intuitionistic type theory, except we do not provide the details of the key technical side-condition because they are not instructive here. Indeed, it is safe to skip this section.

**Definition S12** Consider a set  $\mathcal{V}$  of variable names, ranged over by  $v$ ; a set  $\mathcal{F}$  of function symbols, ranged over by  $f$ ; and a set  $\mathcal{A}$  of ad-hoc logical symbols, ranged over by  $a$ . The sets are assumed to be disjoint. Let  $n$  range over  $\mathcal{V} \cup \mathcal{F}$ .

**Definition S13** Consider terms  $T ::= \mathcal{V} \mid \mathcal{F} \mid T(T)$ ; let  $t$  range over  $T$ .

Terms may occur inside formulas, either by themselves or as arguments to ad-hoc logical symbols.

**Definition S14 (Formulas)** Let  $\vec{X}$  denote lists of  $X$ s and let  $U$  be a set of ‘user-specified sorts’, see below. Inductively define formulas:

$$P^+ ::= T \mid \mathbf{F} \mid P^+ \wedge P^+ \mid P^+ \vee P^+ \mid P^+ \rightarrow P^+ \mid \forall \mathcal{V} \in U. P^+ \mid \mathcal{A}(\vec{T})$$

Let  $p$  range over  $P^+$  and note that  $\forall \mathcal{V} \in U. P^+$  is bounded universal quantification, e.g.,  $\forall v \in \mathbf{Nat}. p$ , where  $v$  may occur in  $p$ .

In order to ensure that terms are used meaningfully, we introduce a notion of sorts with the principal aim that only PROPOSITION-sorted terms, i.e., fully-applied predicates, may occur as formulas, i.e., be considered for provability. For example, a term with sort  $\mathbf{Nat} \rightarrow \mathbf{PROPOSITION}$  will be a predicate on the natural numbers. The result of applying it to a natural number may be provable.

**Definition S15** Let  $\mathbf{PROPOSITION}$  be a constant; let sorts  $S$  ranged over by  $s$  be:

$$S ::= U \mid \mathbf{PROPOSITION} \mid S \rightarrow S$$

**Definition S16** Let  $\Delta$  range over pairs  $\langle \Delta_T, \Delta_A \rangle$ , where  $\Delta_T$  ranges over finite functions from  $\mathcal{V} \cup \mathcal{F}$  to  $S$ , with  $\mathcal{V}$  always mapped to  $\mathbf{PROPOSITION}$ , and where  $\Delta_A$  ranges over finite functions from  $\mathcal{A}$  to  $\vec{S}$ .<sup>3</sup> Let  $\oplus$  range over  $\{\wedge, \vee, \rightarrow\}$  and define well-sortedness for terms,  $\triangleright_t$ , and for formulas,  $\triangleright_f$ :

$$\begin{array}{c} \frac{\Delta \triangleright_t t_f : s_a \rightarrow s_r \quad \Delta \triangleright_t t_a : s_a}{\Delta \triangleright_t t_f(t_a) : s_r} \quad \frac{\Delta_T(n) = s}{\Delta \triangleright_t n : s} \quad \frac{\Delta \triangleright_f p}{\Delta \triangleright_t p : \mathbf{PROPOSITION}} \\[10pt] \frac{\Delta \triangleright_f p \quad \Delta_T(v) = s}{\Delta \triangleright_f \forall v \in s. p} \quad \frac{\overrightarrow{\Delta \triangleright_t t_i : s_i} \quad \Delta_A(a) = \vec{s}_i}{\Delta \triangleright_f a(\vec{t}_i)} \quad \frac{\Delta \triangleright_f p_1 \quad \Delta \triangleright_f p_2}{\Delta \triangleright_f p_1 \oplus p_2} \quad \frac{}{\Delta \triangleright_f \mathbf{F}} \quad \frac{\Delta \triangleright_t t : \mathbf{PROPOSITION}}{\Delta \triangleright_f t} \end{array}$$

<sup>3</sup>Formally,  $\Delta$  should be set up as what is called a dependently-typed list.

Other than ensuring that only terms of sort PROPOSITION are used as formulas, the rules for intuitionistic provability remain unchanged.

**Definition S17 (Intuitionistic type theory)** *Let  $\Gamma$  range over lists of formulas.*

$$\begin{array}{c}
\frac{}{\Gamma_1, p, \Gamma_2 \vdash^\Delta p} (Assm) \text{ if } \Delta \triangleright_f p \qquad \frac{\Gamma \vdash^\Delta \mathbf{F}}{\Gamma \vdash^\Delta p} (E_{\mathbf{F}}) \text{ if } \Delta \triangleright_f p \\
\\
\frac{\Gamma \vdash^\Delta p_l \quad \Gamma \vdash^\Delta p_r}{\Gamma \vdash^\Delta p_l \wedge p_r} (I_\wedge) \qquad \frac{\Gamma \vdash^\Delta p_l \wedge p_r}{\Gamma \vdash^\Delta p_l} (E_\wedge^l) \qquad \frac{\Gamma \vdash^\Delta p_l \wedge p_r}{\Gamma \vdash^\Delta p_r} (E_\wedge^r) \\
\\
\frac{\Gamma \vdash^\Delta p_l}{\Gamma \vdash^\Delta p_l \vee p_r} (I_\vee) \text{ if } \Delta \triangleright_f p_r \qquad \frac{\Gamma \vdash^\Delta p_r}{\Gamma \vdash^\Delta p_l \vee p_r} (I_\vee) \text{ if } \Delta \triangleright_f p_l \\
\\
\frac{\Gamma \vdash^\Delta p_l \vee p_r \quad \Gamma, p_l \vdash^\Delta p \quad \Gamma, p_r \vdash^\Delta p}{\Gamma \vdash^\Delta p} (E_\vee) \\
\\
\frac{\Gamma_1, p_a, \Gamma_2 \vdash^\Delta p_b}{\Gamma_1, \Gamma_2 \vdash^\Delta p_a \rightarrow p_b} (I_\rightarrow) \text{ if } \Delta \triangleright_f p_a \qquad \frac{\Gamma \vdash^\Delta p_a \rightarrow p_b \quad \Gamma \vdash^\Delta p_a}{\Gamma \vdash^\Delta p_b} (E_\rightarrow)
\end{array}$$

**Definition S18** *For Inductively defined sorts, add the sort name to  $U$ , the defining constructor names to  $\mathcal{F}$ , the relevant sorting information to  $\Delta_T$  (e.g.,  $\Delta_T(\mathbf{zero}) = \mathbf{Nat}$  and  $\Delta_T(\mathbf{succ}) = \mathbf{Nat} \rightarrow \mathbf{Nat}$ ), and structural-induction rules to the provability relation, see Section S1.1.1:*

$$\frac{\Gamma \vdash^\Delta q[\mathbf{zero}] \quad \Gamma, q[m] \vdash^{\Delta, m: \mathbf{Nat}} q[\mathbf{succ}(m)]}{\Gamma \vdash^\Delta \forall n \in \mathbf{Nat} . q[n]} (Ind_{\mathbf{Nat}}^{q[\cdot]}) \quad \text{if } n, m \text{ not used in } \Gamma, \Delta$$

$q[\cdot]$  is a “formula with fillable holes”

For  $\mathbf{Nat}$ , structural induction is known as (weak) number induction. We also allow for the definition ( $\doteq$ ) by *structural recursion* of new function symbols over inductively-defined sorts, see Section S1.1.1, e.g. — with  $\neg \mathbf{F}$  non-primitive true:

$$\begin{array}{lcl}
\text{IsEven}(\mathbf{zero}) & \doteq & \neg \mathbf{F} \\
\text{IsEven}(\mathbf{succ}(n)) & \doteq & \neg \text{IsEven}(n)
\end{array}$$

**Definition S19** *For a structural-recursively defined symbol, add the symbol to  $\mathcal{F}$  and add to  $\Delta_T$  a mapping of the symbol to the argument sorts implying the result sort, e.g.,  $\Delta_T(\text{IsEven}) = \mathbf{Nat} \rightarrow \mathbf{PROPOSITION}$ . Also include reasoning-by-simplification as a proof rule:*

$$\frac{\Gamma \vdash^\Delta p_0}{\Gamma \vdash^\Delta p} (simp) \quad \text{if } \downarrow p = p_0 \text{ and } \Delta \triangleright_f p$$

$\downarrow$  is a form of deterministic computation that includes “exhaustive definition unfolding”.

With this, we are able to formally prove that, e.g., zero and two are even.

$$\begin{array}{c}
\frac{}{\mathbf{F} \vdash^{\Delta} \mathbf{F}} (Assm) \\
\frac{}{\vdash^{\Delta} \mathbf{F} \rightarrow \mathbf{F}} (I_{\rightarrow}) \\
\frac{}{\vdash^{\Delta} \text{IsEven}(\mathbf{zero})} (simp) \\
\\
\frac{}{(\mathbf{F} \rightarrow \mathbf{F}) \rightarrow \mathbf{F} \vdash^{\Delta} (\mathbf{F} \rightarrow \mathbf{F}) \rightarrow \mathbf{F}} (Assm) \quad \frac{}{(\mathbf{F} \rightarrow \mathbf{F}) \rightarrow \mathbf{F}, \mathbf{F} \vdash^{\Delta} \mathbf{F}} (Assm) \\
\frac{}{(\mathbf{F} \rightarrow \mathbf{F}) \rightarrow \mathbf{F} \vdash^{\Delta} (\mathbf{F} \rightarrow \mathbf{F}) \rightarrow \mathbf{F}} (I_{\rightarrow}) \quad \frac{}{(\mathbf{F} \rightarrow \mathbf{F}) \rightarrow \mathbf{F} \vdash^{\Delta} \mathbf{F} \rightarrow \mathbf{F}} (I_{\rightarrow}) \\
\frac{}{(\mathbf{F} \rightarrow \mathbf{F}) \rightarrow \mathbf{F} \vdash^{\Delta} \mathbf{F}} (E_{\rightarrow}) \\
\frac{}{\vdash^{\Delta} ((\mathbf{F} \rightarrow \mathbf{F}) \rightarrow \mathbf{F}) \rightarrow \mathbf{F}} (I_{\rightarrow}) \\
\frac{}{\vdash^{\Delta} \text{IsEven}(\text{succ}(\text{succ}(\mathbf{zero})))} (simp)
\end{array}$$

We may also conservatively extend the considered formalism with ad-hoc logical symbols:

$$\frac{}{LEq^{\text{Nat}}(t, t)} \quad \frac{LEq^{\text{Nat}}(\text{succ}(t_1), t_2)}{LEq^{\text{Nat}}(t_1, t_2)}$$

**Definition S20** For ad-hoc logical symbols, add the symbol to  $\mathcal{A}$ , add to  $\Delta_{\mathcal{A}}$  a mapping of the symbol to the arguments sorts (e.g.,  $\Delta_{\mathcal{A}}(LEq^{\text{Nat}}) = \langle \text{Nat}, \text{Nat} \rangle$ ), and include the defining rules as proof rules, with usage called rule induction:

$$\frac{}{\Gamma \vdash^{\Delta} LEq^{\text{Nat}}(t, t)} (rInd_{LEq^{\text{Nat}}}^1) \quad \text{if } \Delta \triangleright_t t : \text{Nat} \\
\frac{\Gamma \vdash^{\Delta} LEq^{\text{Nat}}(\text{succ}(t_1), t_2)}{\Gamma \vdash^{\Delta} LEq^{\text{Nat}}(t_1, t_2)} (rInd_{LEq^{\text{Nat}}}^2)$$

We say that  $\vdash^{\Delta}$  is an *extensible type theory* over an intuitionistic base logic. Under certain additional constraints, specifically *dependent typing of  $\Delta$* ,  $\Gamma$ , we can guarantee that any user-made extensions to  $\Delta$ , etc., preserves consistency. The proof of this will typically use a richer, non-extensible type theory that is consistent and contains functions that, e.g., send the definition of  $\text{Nat}$  to its structural-induction and -recursion rules.

Formal proofs can quickly become very big. While certainly a problem for humans, computerized systems do not suffer from similar short-comings and happily check proofs of any size for rule compliance. Hardware is not a constraint in practice.

### S1.3 CEq principles: molecular-programmed interference

We present the core logical principles of CEq, see Figure 2.

#### S1.3.1 Form-to-function compilation: genotypes to causations

For examples and pre-processing ahead of the technology we present here, see Section S2.2.

**Definition S21 (Genotypes)** *Let  $\mathcal{S}$  be a set of states, ranged over by  $s$ . Let the regulatory expressions be  $\mathcal{S}$  closed under indirection ( $\sim$ ), disjunction ( $\vee$ ), conjunction ( $\&$ ), and inhibition ( $\dashv$ ), and let  $e$  range over  $\mathcal{E}$ :*

$$E ::= \mathcal{S} \mid \sim E \mid E : E \mid E \& E \mid E \dashv E$$

*Let an influence (i.e., an  $I$ ) be a guarded subject change, specifically a polarity (i.e., a direction of change), a subject list (i.e., a list of  $\mathcal{S}$ s), and a regulatory expression, and let a genotype (i.e., a  $G$ ) be an influence-list:*

$$\begin{aligned} Y &::= + \mid - \\ I &::= Y \xrightarrow{\mathcal{S}} E \\ G &::= \vec{I} \end{aligned}$$

Our formal notion of genotype will be used to capture the molecular programming of real-life genomes. This is a non-trivial task, see Section S2.1. In particular, we can assume nothing about the structure of regulatory expressions in a formal genotype. Instead, we convert them to a uniform format that this work shows facilitates molecular-biology reasoning, specifically discretely-regulated changes, with no structure between the regulating states.

**Definition S22 (Causations)** *A causation is a state becoming a state as guarded by a list of literals, see Def.S7:*

$$C ::= \mathcal{S} \xrightarrow{\vec{L}} \mathcal{S}$$

*We will write a causation as  $R \xrightarrow[M]{I} P$ , where the  $M$  and  $I$  partition the guarding literals, i.e., the  $L$ s:  $M$  (the mediators) contains the evenly-negated literals and  $I$  (the inhibitors) the oddly-negated literals minus one negation.*

Regulatory expressions are processed in two steps: 1) view the expressions as propositional formulas, which is trivial except for indirection and inhibition; 2) convert the propositional form to DNF, see Section S1.1.7. **Causations are constructed by stepping through the subject and using each disjunctive clause/maximal conjunctions in the regulatory DNF as guards for each step.**

**Definition S23 (Form-to-function compilation)** *We write  $g \models R \xrightarrow[M]{I} P$  when a genotype,  $g$ , codes for a causation as outlined in bold just above.*

We pursue the specifics of propositional regulation in a bigger context.

**Definition S24 (Propositional CEq)** Assume  $\mathcal{S} \subseteq \mathcal{V}$ . Let the  $[\_]\_$  recursively map genotype syntax to propositional formulas and write  $[\_]$  if we do not distinguish between categories:

$$\begin{aligned}
[o.s]_E &\doteq o.s \\
[\neg e]_E &\doteq \neg\neg[e]_E \\
[e1 : e2]_E &\doteq [e1]_E \vee [e2]_E \\
[e1 \& e2]_E &\doteq [e1]_E \wedge [e2]_E \\
[e1 |-- e2]_E &\doteq ([e1]_E \vee \neg\neg[e2]_E) \wedge \neg[e2]_E \\
[+ s e]_I &\doteq \bigwedge_{\langle o1.s1, o2.s2 \rangle \in s} ((o1.s1 \wedge [e]_E) \rightarrow o2.r2) \\
[- s e]_I &\doteq \bigwedge_{\langle o1.s1, o2.s2 \rangle \in s} ((o2.s2 \wedge [e]_E) \rightarrow o1.r1) \\
[\ ]_G &\doteq \neg \mathbf{F} \\
[i\ g]_G &\doteq [i]_I \wedge [g]_G \\
[R \xrightarrow[M]{I} P]_C &\doteq (\bigwedge_{r \in R} r) \rightarrow (\bigwedge_{m \in M} [m]_E) \rightarrow (\bigwedge_{i \in I} \neg[i]_E) \rightarrow (\bigwedge_{p \in P} p)
\end{aligned}$$

Propositional indirection is motivated in Theorem S4: we make weaker claims for the non-inhibiting states in indirected  $e$  but if they are required to be either present or absent, we guarantee that they are present. The obvious definition of propositional inhibition may appear to be  $[e1] \wedge \neg[e2]$ . When converting nested inhibition:  $o2.s \text{ |-- } (o1.s \text{ |-- } o0.s)$ , to propositional DNF with the shortened form, however, we would get:  $(o2.s \wedge \neg o1.s) \vee (o2.s \wedge \neg\neg o0.s)$ . This reveals a problem:  $o2.s \wedge \neg o1.s$  may enable the changes it is guarding when  $o0.s$  is present and  $o1.s$  ought to be prevented from serving as an inhibitor by the stipulated  $o0.s$ -inhibition. Although also  $o2.s \wedge \neg\neg o0.s$  would enable the changes in question, meaning the changes should be able to go ahead, we would permit false-positive argumentation for otherwise-correct conclusions, cf. Section S2.3.3:NB12. With our translation, we get the following DNF, instead:

$$(o2.s \wedge \neg o1.s \wedge \neg\neg\neg o0.s) \vee (o2.s \wedge \neg\neg o0.s)$$

Recursively, our translation exactly guarantees that the introduced disjunctions are mutually exclusive, as guarded by the deeper inhibitor. While this matches extant molecular-biology reasoning, a stronger case for the definition is that CE-qEA's life-cycle prediction technology only works correctly if it ignores triple and more negated states as sustainers for the reason that the particular change may still be performed, meaning no sustaining takes place, see Section S1.5. **Our regulatory form-to-function compilation guarantees that the disjunctive clauses/maximal conjunctions in a considered DNF may be taken as guards for separate causations in the strong sense that the causations will operate independently of each other:**  $o2.s \wedge \neg o1.s \wedge \neg\neg\neg o0.s$  operates independently of  $o2.s \wedge \neg\neg o0.s$ , as guaranteed by  $o0.s$ .

It is worth noting that the disjunction in the definition of propositional inhibition will never be used as such in the DNF: by distributivity,  $\neg\neg[\mathbf{e2}]$  and  $\neg[\mathbf{e2}]$  are conjuncted and cancel out, leaving the disjunction trivial. Instead, the disjunction becomes a conjunction in case of nested inhibition, as seen.

The big picture:

**Proposition S25** *If  $g \models R \xrightarrow[I]{M} P$  then the propositional formula*

*$(\bigwedge_{o.s \in g} (\neg o.s \vee \neg\neg o.s)) \rightarrow [g] \rightarrow [R \xrightarrow[I]{M} P]$  is provable in intuitionistic logic.*

**Proof:** By Lemma S11, it suffices to prove  $[g] \rightarrow [R \xrightarrow[I]{M} P]$  in De Morgan logic. For simplicity, we will write  $r, m, p, i$  for the propositional forms of  $R, M, P, I$ . By definition,  $[g]$  is a big conjunction of implications. As part of  $\models$ , the implications have their guards turned into DNFs and the formula guarding the implication in the result of  $[R \xrightarrow[I]{M} P]$  is a disjunctive clause of one of them. In other words,  $[g] = X \wedge (r \wedge Y \rightarrow p)$ , for some  $X$  and  $Y$  (under  $\wedge$ -symmetry), with  $m \wedge \neg i$  a disjunctive clause in the constructed DNF of  $Y$ , i.e.,  $Y \leftrightarrow ((m \wedge \neg i) \vee Z)$  in De Morgan logic, for some  $Z$ , per Theorems S9, S10. With this notation, we are trying to prove  $(Y \leftrightarrow ((m \wedge \neg i) \vee Z)) \rightarrow (X \wedge (r \wedge Y \rightarrow p)) \rightarrow r \wedge m \wedge \neg i \rightarrow p$ , which is straightforward in intuitionistic (and De Morgan) logic, see `coext.v`.

Recursive translations are of worst-case exponential asymptotic complexity when a case duplicates terms. Because both steps in the conversion of regulatory expressions perform duplication and the steps are nested, **the worst-case complexity of our regulatory form-to-function compilation will be between exponential and double-exponential**: for a regulatory expression of length  $n$ , we may need to consider on the order of  $2^n$  to  $2^{(2^n)}$  many causations, depending on how the conversion steps interact. It is not obvious if the complexity can be improved upon. (Conversely, it allows for a lot of subtlety to be packed into regulation, see article.) The key mitigating factor is that the uppermost exponent,  $n$ , is for the size of individual regulatory expressions, with the complexity for a genotype being the summation across influences.

### S1.3.2 Coextension logic: causations to phenotypes

The objective of molecular-biology reasoning is to justify phenotype properties from genotype specifics. In CEq, this is done with coextension logic (Figure 2) over automatically-determined causations. The meta-theoretic properties of coextension logic we discuss here have been formally verified using the Coq Proof Assistant [22], see `coext.v` and Sections S1.1–S1.2. We have included “Sub-intuitionism” as a gentle overview. For the formal proofs, e.g., reflexive causations (non-homeostatic fixating regulation) require some attention but there are other points of interest in the details.

**Sub-intuitionism** The (*interference*) rule is intuitionistically valid essentially by the following three properties, with causations seen as implications, see Def-

inition S24. We would apply the first property in the lemma to include the reactants and mediators for all causations in each causation, the second to join the padded causations, and the last to include context.

**Lemma S26 (Propositional interference)** *For any  $p_a, p_b, p_c$ :*

$$\vdash (p_a \rightarrow p_b) \rightarrow ((p_a \wedge p_c) \rightarrow p_b)$$

and

$$\vdash ((p_a \rightarrow p_b) \wedge (p_a \rightarrow p_c)) \rightarrow (p_a \rightarrow p_b \wedge p_c)$$

and

$$\vdash (p_a \rightarrow p_b) \rightarrow ((p_a \wedge p_c) \rightarrow (p_b \wedge p_c))$$

**Proof:** See supporting file `coext.v`.

The (*sequence*) rule is intuitionistically valid essentially by the following.

**Lemma S27 (Propositional sequence)** *For any  $p_1, p_2, p_3$ :*

$$\vdash ((p_1 \rightarrow p_2) \wedge (p_2 \rightarrow p_3)) \rightarrow (p_1 \rightarrow p_3)$$

**Proof:** See supporting file `coext.v`.

**Formal definitions** We represent CEqEA's schema-instance states by *instance sorting* in the Coq Proof Assistant: we postulate the existence of a set of instances (schemas at specific categories) and, for each instance, a set of states.

**Variable** *insts* : Set.

**Variable** *stts* : *insts* → Set.

Collections of states are represented by a boolean truth value for each state: Coq's *bool*, i.e., *true* or *false*, with `||` (disjunction), `&&` (conjunction), and *negb* (negation). We also need some basic binary operations (*merge* and *minus*) and predicates (*disjoint* and *subcllctn*), and a specific predicate for homogeneity (*homgen*): no instance has more than one state assigned to *true*.

**Definition** *cllctn* :=  $\forall i : \text{insts}, \text{stts}(i) \rightarrow \text{bool}$ .

**Definition** *nilcllctn* : *cllctn* := `fun i s => false`.

**Definition** *merge* (*A1 A2* : *cllctn*) : *cllctn*

:= `fun i s => A1(i)(s) || A2(i)(s)`.

**Definition** *minus* (*A1 A2* : *cllctn*) : *cllctn*

:= `fun i s => A1(i)(s) && negb(A2(i)(s))`.

**Definition** *disjoint* (*A1 A2* : *cllctn*) : **proposition**

:=  $\forall i s, A1(i)(s) \ \&\& \ A2(i)(s) = \text{false}$ .

**Definition** *subcllctn* (*A1 A2* : *cllctn*) : **proposition**

:=  $\forall i s, A1(i)(s) = \text{true} \rightarrow A2(i)(s) = \text{true}$ .

**Definition** *homgen* (*A* : *cllctn*) : **proposition** :=  $\forall i s1 s2, A(i)(s1) = \text{true} \rightarrow A(i)(s2) = \text{true} \rightarrow s1 = s2$ .

Causations (*CSTNs*) are represented as 4-tuples of collections, and we need functions that merge together the specific tuple-entries across a list of *CSTNs*:

```

Inductive CSTN : Set :=
| cstn (Rcntnt Mdtr Prdct Inhb : cllctn) : CSTN.

Definition rctnts (C : list CSTN) : cllctn :=
  fold_right (fun h t' =>
    merge (match h with
      | cstn Rcntnt _ _ => Rcntnt
    end) t') nilcllctn C.
Definition mdtrs (C : list CSTN) : cllctn :=
  fold_right (fun h t' =>
    merge (match h with
      | cstn _ Mdtr _ _ => Mdtr
    end) t') nilcllctn C.
Definition prdcts (C : list CSTN) : cllctn :=
  fold_right (fun h t' =>
    merge (match h with
      | cstn _ _ Prdct _ => Prdct
    end) t') nilcllctn C.
Definition inhbs (C : list CSTN) : cllctn :=
  fold_right (fun h t' =>
    merge (match h with
      | cstn _ _ _ Inhb => Inhb
    end) t') nilcllctn C.

```

For convenience, we index derivations by intermediate compartments.

```

Inductive Intermediates : Set :=
| nilInt : Intermediates
| seqInt : Intermediates → cllctn → Intermediates → Intermediates.

```

*nilInt* is for (*interference*), which has no intermediate compartments. *seqInt* is for (*sequence*): we will take the intermediates from the left premise, the intermediate compartment ( $A_2/A_2$ ) in this occurrence, and the intermediates from the right premise, and create the new intermediates.

For simplicity, we do not consider coinhibition in the formal developments, instead putting a trivial predicate in its place. *True* is **propositional** true: trivial provability (not *boolean true*: a definite value in and of itself).

```

Definition coinhbFree (C : list CSTN) : proposition := True.

```

There is one difference in how we define coextension derivations compared to Figure 2: we have removed the form-to-function compilation listed in the figure,  $\models$ , to work directly with causations, *C*. This makes our properties stronger in that we cannot rely on any  $\models$ -particulars: our properties must hold for any and all lists of causations, which includes the lists produced by  $\models$ .

**Inductive** *coext* : (list CSTN) → clctn → clctn → Intermediates → Set :=  
| *intCo* : ∀ C0 C A,  
    (∀ c, (In c C0) → (In c C))  
    → subclctn (rctnts C0) A  
    → subclctn (mdtrs C0) A  
    → disjoint (inhbs C0) A  
    → coinhbFree C0  
    → homgen (merge (minus A (rctnts C0)) (prdcts C0))  
    → coext C A (merge (minus A (rctnts C0)) (prdcts C0)) nilInt  
| *seqCo* : ∀ C A1 A2 A3 t1 t2,  
    coext C A1 A2 t1  
    → coext C A2 A3 t2  
    → coext C A1 A3 (seqInt t1 A2 t2).

In *intCo*, C0 is for the left-hand side of the first line in the condition for (*interference*) in Figure 2.

**Regular causations: state to state within instances** Structurally, we make a particular simplifying assumption in a few locations: all CSTNs go from one state to one state of the same instance. CEqEA obeys one-to-one by design as it stands but not necessarily instance preservation. However, instance preservation is guaranteed by the act of MIG/RI specification, see Section S2.1. In particular, all of Section S2 (covering [28]) falls within the simplification.

**Definition** *singlesorted* (A : clctn) : proposition := ∀ i1 i2 s1 s2,  
    A(i1)(s1)=true  
    → A(i2)(s2)=true  
    → i1=i2.

**Definition** *singleton* (A : clctn) : proposition := ∃ i s1, A(i)(s1)=true  
    ∧ (∀ s2, A(i)(s2)=true → s1=s2).

**Definition** *regular* (C : list CSTN) : proposition := ∀ c, In c C →  
match c with  
| cstn Rctnt \_ Prdct \_  
    ⇒ singleton(Rctnt) ∧ singleton(Prdct) ∧ singlesorted(merge Rctnt Prdct)  
end.

**Consequence and Cut** We prove that coextension logic is a logic, i.e., a *consequence relation*. An implication of being a consequence relation is that the so-called cut rule is admissible: adding the cut rule to the definition of coextension logic would not allow us to justify more compartment changes. The introductory definition below is a generalization of the first consequence property, which says that anything assumed follows as a consequence:  $\forall \Gamma. \forall p \in \Gamma. \Gamma \vdash p$ . The generalization splits the two sets of assumptions: one for checking membership and the other for underpinning the derivation behind the targeted consequence. This is used in the second property to express that if the second set of assumptions can establish all parts of the first set of assumptions, it can establish anything that can be established from the first set of assumptions:  $\forall \Gamma_a, \Gamma_c, p. (\forall p_a \in \Gamma_a. \Gamma_c \vdash p_a) \rightarrow (\Gamma_a \vdash p) \rightarrow (\Gamma_c \vdash p)$ . The property estab-

lishes that arguments may be *recomposed* if the most minimal of requirements are met. Here, we use our standard simplification plus homogeneity of the starting compartment.

**Definition** *cnsqnc\_unit* (*Rctnt Mdtr Prdct Inhb* : *cllctn*)  
 (*Ca Cc* : *list CSTN*)(*X* : *cllctn*) :=  
*In* (*cstn Rctnt Mdtr Prdct Inhb*) *Ca*  
 → *subcllctn Rctnt X*  
 → *subcllctn Mdtr X*  
 → *disjoint Inhb X*  
 → *homgen* (*merge* (*minus X Rctnt*) *Prdct*)  
 → *coext Cc X* (*merge* (*minus X Rctnt*) *Prdct*) *nilInt*.

**Proposition** *coext\_unit* :  $\forall$  *Rctnt Mdtr Prdct Inhb C A*,  
*cnsqnc\_unit Rctnt Mdtr Prdct Inhb C C A*.

**Proposition** *coext\_recmps\_simpl*:  $\forall$  *Ca Cc A1 A2 t*,  
*homgen A1*  
 → *regular Ca*  
 → *regular Cc*  
 → ( $\forall$  *Rctnt Mdtr Prdct Inhb X*,  
*homgen X*  
 → *cnsqnc\_unit Rctnt Mdtr Prdct Inhb Ca Cc X*)  
 → *coext Ca A1 A2 t*  
 → *coext Cc A1 A2 t*.

The cut theorem is expressed by means of an advanced feature of Coq: dependent typing. Dependent typing allows us to reference the derivation, *d0*, behind a coextension relationship in order to extract the *CSTNs* that were used in case the most recent rule is (*interference*). Here, too, we use our standard simplification plus homogeneity of the starting compartment.

**Fixpoint** *coCSTN* {*C* : *list CSTN*}{*A1 A2* : *cllctn*}{*t* : *Intermediates*}  
 (*d* : *coext C A1 A2 t*) {**struct** *d*} : *list CSTN* :=

**match** *d* **with**  
 | *intCo C0* - - - - - ⇒ *C0*  
 | *seqCo* - - - - - ⇒ *nil*  
**end**.

**Theorem** *coext\_cut\_simpl* :  $\forall$  *C A1 A2 A0 t*,  
 $\forall$  *d0* : (*coext C A1 A0 nilInt*),  
**let** *C0* := *coCSTN d0* **in**  
**let** *c0* := *cstn* (*rctnts C0*) (*mdtrs C0*) (*prdcts C0*) (*inhbs C0*) **in**  
*homgen A1*  
 → *regular* (*c0::C*)  
 → *coext* (*c0::C*) *A1 A2 t*  
 → *coext C A1 A2 t*.

As explanation of the text of this **Theorem**, the cut rule looks as follows for intuitionistic logic:

$$\frac{\Gamma \vdash p_0 \quad p_0, \Gamma \vdash p}{\Gamma \vdash p} (cut)$$

Behind the scene of these results, we introduce a version of coextension logic

with arbitrarily ordered/distributed, rather than unordered/concurrent, interference, with proofs of equivalence of the definitions:

**Inductive** *coextS* :

- (*list CSTN*) → *cllctn* → *cllctn* → *Intermediates* → (*list CSTN*) → **Set** :=
- | *reflCoS* : ∀ *C A*,
- homgen A*
- *coextS C A A nilInt nil*
- | *cstCoS* : ∀ *C A Rctnt Mdr Prdct Inhb*,
- In (cstn Rctnt Mdr Prdct Inhb) C*
- *subcllctn Rctnt A*
- *subcllctn Mdr A*
- *disjoint Inhb A*
- *homgen (merge (minus A Rctnt) Prdct)*
- *coextS C A (merge (minus A Rctnt) Prdct) nilInt*
- ((*cstn Rctnt Mdr Prdct Inhb*)::*nil*)
- | *parCoS* : ∀ *C A A1 A2 C1 C2*,
- coinhbFree (C1++C2)*
- *homgen (merge (minus A (rctnts (C1++C2))) (prdcts (C1++C2)))*
- *coextS C A A1 nilInt C1*
- *coextS C A A2 nilInt C2*
- *coextS C A (merge (minus A (rctnts (C1++C2))) (prdcts (C1++C2)))*
- nilInt (C1++C2)*
- | *seqCoS* : ∀ *C A1 A2 A3 t1 C1 t2 C2*,
- coextS C A1 A2 t1 C1*
- *coextS C A2 A3 t2 C2*
- *coextS C A1 A3 (seqInt t1 A2 t2) nil*.

**Proposition** *staged\_coext* : ∀ *C A1 A2 t*,

- (*homgen A1*) → {*C0*:- & (*coextS C A1 A2 t C0*)} → *coext C A1 A2 t*.

**Lemma** *coextS\_staging* : ∀ *C A C0*,

- homgen A*
- *regular C*
- (∀ *c* : *CSTN*, *In c C0* → *In c C*)
- *subcllctn (rctnts C0) A*
- *subcllctn (mdtrs C0) A*
- *disjoint (inhbs C0) A*
- *coinhbFree C0*
- *homgen (merge (minus A (rctnts C0)) (prdcts C0))*
- *coextS C A (merge (minus A (rctnts C0)) (prdcts C0)) nilInt C0*.

**Constructivity** We prove that coextension logic is constructive in an indirect sense: anything that can be proved in coextension logic can be proved in the intuitionistic type theory of Coq, see Section S1.2. Below, *environment* takes the place of *cllctn* and *cProp* expresses that a given *environment* is compatible with the given *cllctn*. The assumption saying (∀ *X* ...) lifts the assumed *CSTNs* in the relevant compartments to the level of **proposition**, where the proof uses them as building blocks to mimic the compartment change propositionally.

```

Definition environment :=  $\forall i : \text{insts}, \text{stts}(i) \rightarrow \text{proposition}$ .
Definition cProp (c : cllctn)(env : environment) :=  $\forall i\ s, c\ i\ s = \text{true} \rightarrow \text{env}\ i\ s$ .
Fixpoint InInt(X : cllctn) (i : Intermediates) {struct i} : proposition :=
match i with
| nilInt  $\Rightarrow$  False
| seqInt t1 A t2  $\Rightarrow (A=X) \vee (\text{InInt}\ X\ t1) \vee (\text{InInt}\ X\ t2)$ 
end.

Theorem coext_CoqProp (env : environment) :  $\forall C\ A1\ A2\ t,$ 
      coext C A1 A2 t
       $\rightarrow (\forall X\ R\ M\ P\ I,$ 
        (X=A1  $\vee$  InInt X t)
         $\rightarrow \text{In}\ (\text{cstn}\ R\ M\ P\ I)\ C$ 
         $\rightarrow (\text{subcllctn}\ R\ X)$ 
         $\rightarrow (\text{subcllctn}\ M\ X)$ 
         $\rightarrow (\text{disjoint}\ I\ X)$ 
         $\rightarrow (\text{cProp}\ P\ \text{env}))$ 
       $\rightarrow (\text{cProp}\ A1\ \text{env})$ 
       $\rightarrow (\text{cProp}\ A2\ \text{env})$ .

```

**Consistency** We can now prove that coextension logic does not justify everything considered because some coextension things map to propositional formulas that are not intuitionistically valid, i.e., to things that are not provable in Coq. **Proposition** *coext\_nonempty* is a high-level acknowledgement that coextension logic is not useless (but see Section S2.3).

**Theorem** *coext\_nontrivial* :  $\exists C\ A1\ A2, \text{not } (\exists t, \text{inhabited } (\text{coext}\ C\ A1\ A2\ t))$ .

**Proposition** *coext\_nonempty* :  $\exists C\ A1\ A2, (\exists t, \text{inhabited } (\text{coext}\ C\ A1\ A2\ t))$ .

The *ts* above refer to the shape of the witnessing derivations and are quantified to reflect that we are only interested in whether the eventual conclusions are possible. The *inhabited* predicate is Coq vernacular for something technical that here means ‘has a derivation’.

## S1.4 CEq mechanisms 1: concurrency

The developments in this section are illustrated with formalized monograph material, see Section S2.

### S1.4.1 Cascaded causation diagrams

We visualize the regulatory functionality of Section S1.3 in the form of a *cascaded causation diagram*: the graph of the considered causations, with one exception. The nodes in the diagrams are constructed from reactants/products and necessary mediators, i.e., from the positive information. User-specified seeds and automatically-inferred toggles (see below) are added as extra nodes. Causations are inserted as edges. The exception is that edges are inserted everywhere they apply rather than just in their canonical place. CEqEA’s static kernel verifies that each inserted edge represents a correct cause-and-effect in the given circumstances. For the monograph, this includes a check that parts of connected nodes that are not requirements for the causation are **fixed**/not changed:

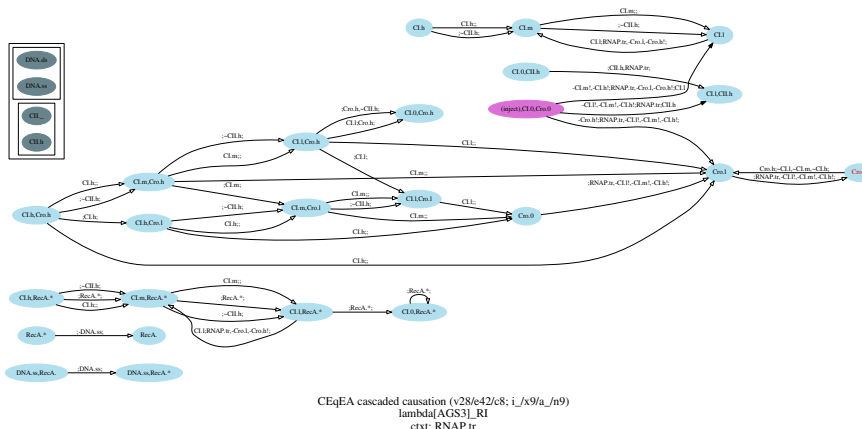

- Light-blue nodes indicate (intra-compartment) situations that constitute the positive conditions for the edges — we refer to these as *points of interaction*, or simply nodes.
- Magenta nodes indicate named inter-compartment *channels* that were user-declared as **entry** or **exit seeds**, see Section S2.1. with the name listed in parentheses.
- Grey-blue nodes indicate *toggles* for each state of a schema instance that has a state that occurs in a causation node without changing across any edge — these will typically represent environmental factors.
- Edges are annotated with their regulators:

<source-only> ; <source+target> ; <target-only>

- Edges with a filled arrow-head have <target-only> mediators and are classified as TargetRequired, see Section S2.3.3:NB3.

Additional information may be displayed by various key-presses in the visualization of these diagrams, see CEqEA/Help/CCP.

#### S1.4.2 CCP: calculus of coextensive processes

Coextension reasoning may be visualized over cascaded causation diagrams. As defined, coextension logic allows us to reason about all that *may* happen in a compartment. Going a step further, CEqEA includes a proof engine based on our *calculus of coextensive processes* (CCP) that attempts to predict what *will* happen in a given situation by pursuing all applicable causations. CCP is defined over cascaded causation diagrams for reasons discussed in the article.

**Definition S28** *Let  $CCP^{[strategy]}$  be a cascaded causation diagram acting on a compartment:*

1. consider a compartment, i.e., a set of instance-sorted states, see Figure 2;
2. enable the blue nodes in the considered diagram with all content in 1.;
3. consider  $[strategy]$  out-edge(s) of 2. — TargetRequired edges must have the contents of both nodes in 2.;
4. block any out-edges in 3. carrying an inhibitor in 1.;
5. block any coinhibited out-edges after 4. — found as a least fixedpoint (cycles are errors: all edges cannot outpace all other edges);
6. denote any remaining out-edges after 5. running;
7. consider the products and retained mediators of the running edges in 6.;
8. add the states of 7. to 1. after removing states with coinciding instances;
9. ensure homogeneity: no two different states of any instance are included.
10. Repeat.

CCP is parameterized by a  $[strategy]$  for choosing out-edges. The CEqEA proof engine uses  $CCP^{all}$  but we prove general properties for arbitrary strategies, denoted by writing just CCP.

**Proposition S29** *CCP generates coextension derivations for cascaded causation diagrams that are constructed with mediators subject to the **intrinsic** modality value for the **source**, meaning with edges that only connect to start nodes containing all causation mediators.*

**Proof:** Figure 2’s (*sequence*) rule accounts for repeat usage. For steps, see Figure 2’s (*interference*) rule: 1. corresponds to  $A$ ; 2.,3. to the right-hand side of  $\subseteq$  in l.1 of the conditions; 4. to l.2; 5. to l.3; 3.,6. account for what may appear on the left-hand side of  $\subseteq$  in l.1; 7. readies the target compartment; 8. corresponds to the chosen left-hand side of  $\subseteq$ , subject to l.4, see 9.

For the mediator issue, note that coextension logic requires mediators to be present in the left (or start) but not in the right (or target) compartment, see Figure 2:Definition 3. For 7., “retained mediators” restricts the parts of the compartments that may change, meaning the condition is stricter than coextension logic’s, i.e., it poses no problem for Proposition S29.

Acting under CCP does not correspond straightforwardly to graph traversal. For example, a running edge may target a node with multiple states, where some may occur in nodes of their own that need not connect to running edges. Supplementing CCP<sup>all</sup>, CEqEA pinpoints implicit targets and nodes-to-be-abandoned, and temporarily inserts implied edges to suggest the graph-traversal mechanics in play to help clarify the deeper interference structure, see Section S1.5.

### S1.4.3 CCP visualization in CEqEA

In CEqEA, Definition S28 is visualized as follows, see video:

- Nodes with a black bolded border have their content subsumed by a given compartment — we refer to these as *enabled*.
- Nodes with a black dashed border are candidates for the ensuing compartment, see also Section S2.3.3:NB7.
- Nodes with a red dashed border are also such candidates but they jointly contain multiple states for some schema instance, i.e., they point to a divergent update that must be resolved, see, e.g., Section S2.3.2:3/b/ii/CII. { $-, h$ }+SOS+Cro.h/ll.9–11.
- Nodes with a magenta bolded border are nodes that are enabled by virtue of an enabled channel, see, e.g., Section S2.3.3:NB9 — we refer to these as (inter-compartment) *boosters*, see Section S2.3.3:NB2.
- Dashed (moving) edges indicate *active* edges: causations whose positive conditions are met and whose negative conditions are not violated:
  - Blue indicates covariant causations.
  - Violet contravariant causations (from MIG-specified !s).
  - Magenta channel activity, see Section S2.3.3:NB2.
- Dotted (stationary) edges indicate *blocked* edges: causations whose positive conditions are met but whose negative conditions are violated:
  - Red indicates inhibition.
  - Orange coinhibition, see Section S2.3.2:2/c/CII.  $-$ +CI.1/ll.13–15.

– Magenta latent inhibition, see Section S2.3.3:NB10.

- Only edges out of enabled nodes may be active or blocked but they may also be neither, see Section S2.3.3:NB3 (TargetRequired). See also Section S2.3.3:NB1-vs-7 (implied edges).

The CEqEA implementation of CCP<sup>all</sup> adds several practical features that may be used at the cost of starting a new derivation, see Sections S1.4.4–S1.4.5.

#### S1.4.4 Standard and non-standard progress in CEqEA

By default, the CEqEA implementation of CCP<sup>all</sup> proceeds automatically at the rate of a step per second. In case of problems in Definition S28:9., the execution stops by default (with the problem visualized) but it is also possible to request that CEqEA resolves divergences at random. Execution may also be halted by kill switches, see Section S2.1. More, 7. may be overridden by a user, e.g., to account for perturbation or external signals, at the cost of starting a new derivation.

#### S1.4.5 Inter-compartment activity in CEqEA

As defined, CCP executions just run, meaning they do not have designated start and end points. This and other characteristics make CCP a *process calculi*, a class of models of concurrent computation. Process calculi tend to address open-system issues, where input is not input per se but interaction that may occur at any time, see Section S1.4.4. CEqEA’s proof engine has special provisions for starting from and for the interaction given by something entering into the considered compartment. Coextension logic allows for this by not requiring the first considered compartment to be homogeneous. CEqEA’s mechanism is called inter-compartment channels: the magenta nodes in cascaded causation diagrams, see Section S1.4.1. Unlike CCP proper, the use of inter-compartment channels are by graph-traversal mechanisms: when pursuing a running out-edge, the magenta nodes get abandoned and their content must orderly integrate itself in order for CCP to continue. Inter-compartment channels may recruit intra-compartment nodes and their edges: the compartment solution has an injected solution mixed in, as it were, at the cost of starting a new derivation. See also Section S2.3.3:NB2, NB3, NB9, NB10.

## S1.5 CEq mechanisms 2: sequentialization

We adapt the notion of ‘trace monoids’ from the study of concurrency and process calculi to CCP<sup>all</sup>. The result predicts observable states and life cycles.

### S1.5.1 Observable states in isolation: interpolation

As stressed in Section S2.1, the states for the schema instances we work with, e.g., the considered protein concentrations, are physiologically determined: they nominally transpose binding affinities, and similar. This is seen in the “RI (Regulation Interface) modeling methodology” moniker, see Section S2.1. In particular, the specified states need not be observable at any time.

[[28]:92:-3]/App.SB :

SUPPRESSED

To move to observable states, we take advantage of the exception in the construction of cascaded causation diagrams, see Section S1.4.1. Nodes in cascaded causation diagrams are constructed as exactly those situations that fulfill the positive requirements for some causation, which implies that each causation has a canonical place to occur in a diagram. However, the causations are inserted everywhere they apply. If some mediator changes a schema instance in one way and the schema instance changes itself back, e.g., under auto-mediation, constitutive transcription, or similar, the cascaded causation diagram will contain a loop in the relevant location. This loop will represent conflicting causations and any observable concentration will be intermediate between the states in the looped nodes, see [[28]:92:-3]/App.SB. With our discrete level of detail, we cannot say which causations will dominate and to what extent, meaning we cannot say how close the observed concentration is likely to be to either of the extreme concentrations. If we are more to one side, any outgoing causations from there will be more relevant to the development of the system than outgoing causations from the disfavoured node. To address observability, we first impose a “loop” granularity, meaning we no longer allow for distinguishing nodes that are connected by looping edges. In graph-theory terminology this means that we do not distinguish nodes within strongly-connected components of the graph: *a collection of nodes is a strongly-connected component if there is a (directed) path of edges from any member of the collection to any other member and no additional node can be included in the collection without breaking this requirement.*

- The reasoning in Section S2.3 specifically does not respect “loop” granularity: it proceeds at the physiological level of abstraction. One of our contributions is to observe that reasoning induces the granularity of the level above it: we have the technical means to move from the (individually) physiological to the (collectively) observable.
- The above ignores negative conditions, see *sustained equilibria* below.



occupying an operator within the relevant promoter) and is able to direct the overall course of action as a result. In defining sustained equilibria, we first classify all states, i.e., all potential sustainers, as either always present, transitory, or never present. We call this an ATN-classification. The classification scheme implies that there will be three to the number of states many different types of sustained equilibria but they exhibit strong regularities that we are able to take advantage of. Any state classified as never present for a given type of sustained equilibria sees all its inhibition occurrences ignored. Any state classified as always present sees all edges that carry it as inhibitor ignored.

**Definition S30** *Given a classification of the considered states as ATN sustainers, we first find all strongly-connected components over the graph without A-inhibited edges. We then classify any found component as a sustained equilibrium of the given ATN type if it has no out-edges in the graph without A- and/or T-inhibited edges. By default, we consider only direct inhibitors for sustaining: indirect inhibition tends to express precedence, i.e., other action dominates.*

CEqEA allows for the identification of all types of sustained equilibria but has special support for two particular types.

**Definition S31**

- *Sustained equilibria with all states classified as transitory are referred to as max equilibria and are annotated to cascaded causation diagrams as red boxes.*
- *Sustained equilibria with all states classified as always present are referred to as min equilibria and are annotated to cascaded causation diagrams as blue boxes.*

Sustained equilibria with a user-given ATN-classification are annotated as green boxes. Below, CEqEA indicates max, min, and sustained equilibria with all states classified as never present.

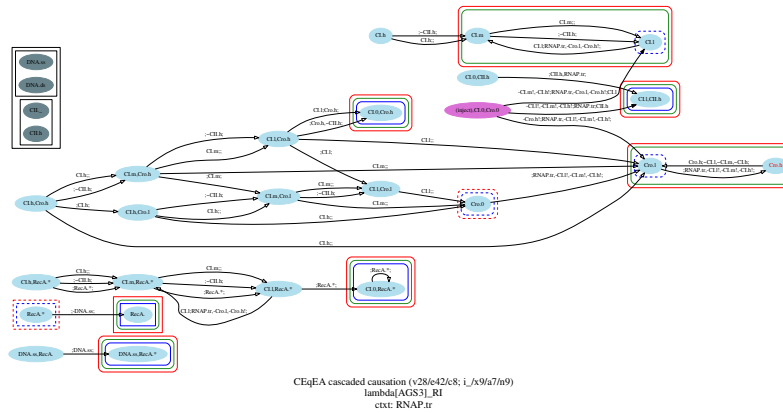

The min/max nomenclature refers to the following properties:

**Proposition S32**

- *No sustained equilibrium can contain a max equilibrium plus strictly more nodes.*
- *No sustained equilibrium plus strictly more nodes is contained in a min equilibrium.*
- *All sustained equilibria contain at least one min equilibrium.*

Min and max equilibria seem to provide sufficient information for the type of analysis we present and we shall not further discuss general sustained equilibria.

**Definition S33**

- *Sustained equilibria with out-edges in the full cascaded causation diagram are called collapsible and are shown as dashed boxes.*
- *Sustained equilibria with no in-edges in the graph without A-/T-inhibited edges are called preventable and are shown as sharp-cornered boxes.*

**S1.5.3 Synchronization**

A main class of models of computation intended for the study of concurrency are called process calculi. They sometimes come with communication primitives that, e.g., require processes to hand-shake. Combinations of processes that are not involved in hand-shaking or similar are independent of each other, and nothing can be assumed about their order of execution. Trace monoids are a way of capturing the sequential ordering imposed on a given system as a whole by the various types of synchronization that explicitly or implicitly are in play.

**Definition S34 (Idealized)** *By synchrotype, we mean an account of how a collection of causations may interleave with each other under  $CCP^{all}$  where 1) we do not distinguish different execution orders of causations that are independent of each other and 2) vectors for environmental influences and similar are retained as conditionals.*

CCP contains no synchronization primitive in the traditional sense, and we instead need to attempt to infer when and how causations align with each other. The central idea behind our approach is that a causation exiting a sustained equilibrium stands in a dependency relationship with (i.e., is not independent from) the causations that affect the attendant sustainers: the one can only come after the others. We abstract the problem by targeting box-based independence between causations: we have already discussed how we cannot distinguish conflicting causations, i.e., edges within sustained equilibria, and what remains is to determine when causations in different boxes are independent of each other. The question is: when may different boxes interleave their causations, i.e., when may boxes coexist under  $CCP^{all}$ . Our particular definition of coexistability seems to approximate synchrotyping well in practice but it is clearly not perfect.

**Definition S35** A collection of sustained equilibria are orthogonal if no schema instance is in different states in different equilibria and if no equilibrium loses strong-connectivity under inhibition by the content of the other equilibria.

This definition, e.g., does not allow for lock-stepped interleaving, but it mostly suffices for the monograph. We shall not pursue the issue of a perfect definition here, other than mentioning that CEqEA also comes with a notion that is too lax, called *reconcilable equilibria*: each node in an equilibrium must be able to pair up with a node from each of the other equilibria without having some schema instance be in two states. We can now approximate synchrotypes.

**Definition S36** Given a cascaded causation diagram, typically with min and max equilibria, and a notion of coexistability, the associated synchronization diagram is given by

- lifted nodes that
  - are the maximal collections of coexistable equilibria plus any nodes not in boxes whose content is in the content of the equilibria, where
  - each collection includes at least one state for each considered instance
- along with any nodes in the given graph that are not in one of these collections but can be reached from a node in them in the base diagram, and
- edges from the cascaded causation diagram that go from a node in a lifted node to a node in a lifted node, with preference given to edges within a lifted node by default.

Note that no inhibition is enforced in the last step in this definition, meaning that edges in synchronization diagrams are opportunistic by default. This is an open-system consideration. If we modelled closed systems where all changes, say, to CI that we are interested in were accounted for, we would enforce inhibition and more when constructing synchronization diagrams, but we consider open systems where, e.g., a host's SOS response may remove all of a given  $\lambda$ 's CI protein. We proceed as we do because we wish to understand, e.g.,  $\lambda$ 's programming in its own right rather than, say, how a combined *E. coli* and  $\lambda$  cell behaves in a fixed environment.

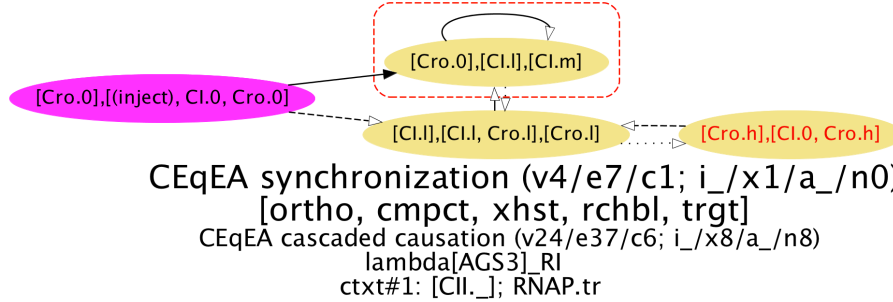

**Definition S37**

- *A node in a synchronization diagram is written with yellow background by default and*
  - *may expire the system if a node inside it may expire the base diagram — red text*
  - *is a channel if a node inside it is a base-diagram channel — magenta background*
  - *is a particular type of equilibrium if the nodes inside it make up the same type of equilibria in the base diagram — indicated with red boxes for max equilibria, blue for min, and green for user-given*
  - *is collapsible/preventable if the equilibria inside it are in the base diagram — indicated with dashed and sharp-cornered boxes, respectively.*
- *A reachable base node that is not in a coexistability situation retains its blue background.*
- *An edge in a synchronization diagram*
  - *may reflect multiple edges in the base diagram,*
  - *is constrained by the TargetRequired condition if all base edges it reflects are TargetRequired — indicated with a filled arrow head,*
  - *is inhibited in the source node if all base edges it reflects are inhibited by all states some schema instance occur with in the source lifted node — indicated with a dotted edge,*
  - *is inhibited in the target node if all base edges it reflects are inhibited by all states some schema instance occur with in the target lifted node — indicated with a dashed edge (provided the edge is not dotted).*

## S1.6 CEq diagrams

CEqEA is able to generate several types of diagrams. We will not give full details of their differing semantics but we outline the basics and make some general remarks. Our principal approach is *intensional* as opposed to the *extensional* one of state spaces: we focus on causations rather than their manifestations, see Sections S1.1,S1.3 for the logic side and Section S1.5 for physiological vs. observable.

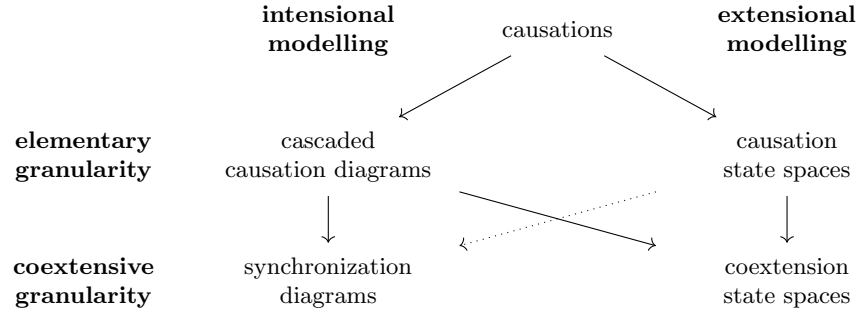

Several of the constructions we use are presented as graph transformations. This means they apply freely to the different diagrams even if only some make sense. Only those represented by arrows above are enabled in CEqEA: essentially, their application must proceed bottom-up (in the scientific sense; not according to the figure's layout). As we discuss, the dotted arrow violates this by going from an extensional back to an intensional understanding. This is a problem because a given set of manifestations may come from different collections of causations. This has important consequences for life-cycle prediction.

### S1.6.1 Elementary: cascaded vs state space for causations

A cascaded causation diagram is the graph of a set of causations: the nodes meet the causations' positive conditions and the edges carry the negative ones.

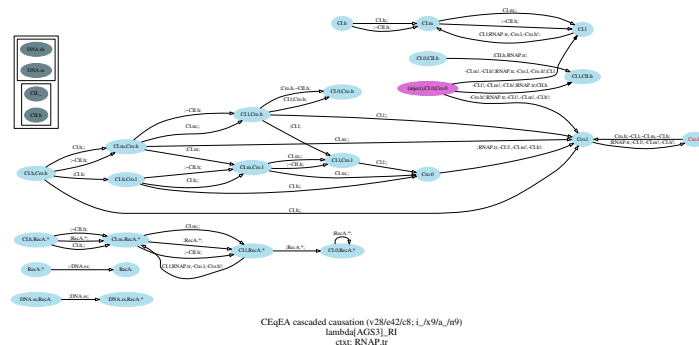

A *causation state space* is constructed by inserting causations as edges, as done for cascaded causation diagrams, except over nodes with all state combinations rather than only pivotal ones, according to the considered coding.

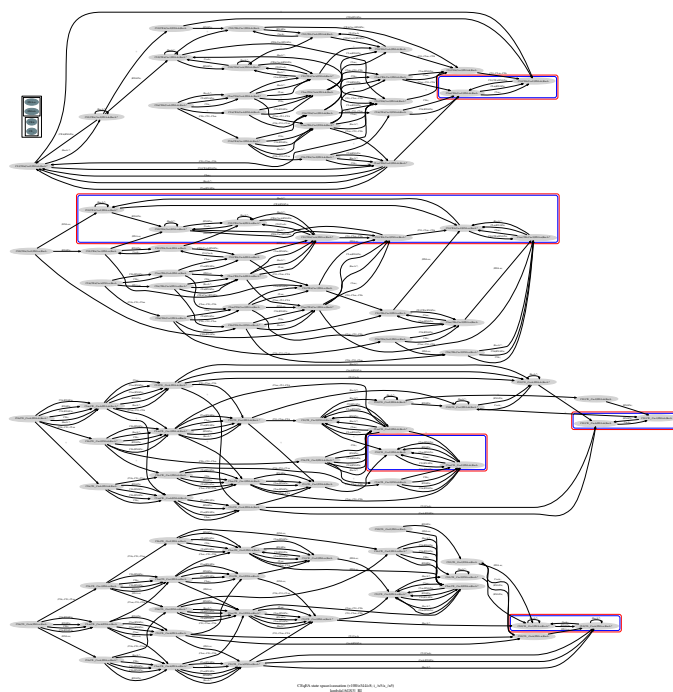

This renders the bulk of CEqEA’s modal theory (for addressing the consequences of different types of molecular interaction) moot and has the effect of statically resolving any and all negative conditions for the inserted causations: edges in causation state spaces do not carry inhibitors. If we attempt to insert an edge so that it starts from a node that contains an inhibitor of the causation at hand, the causation can never run and the edge is not inserted.

Otherwise, the start node contains a different state for the inhibitor’s schema instance, which means we can guarantee that the inhibition is irrelevant and CEqEA suppresses the inhibitor on the edge. This has the effect of collapsing our hierarchy of sustained equilibria down to just one type: sustained equilibria with all states classified as never-present, see Section S1.5. These always sit at the “end” of the generated graph: they are exactly the terminal strongly connected components. No collapsible equilibria “within” the graph are possible, i.e., there are no dashed boxes. There are also no channels, partly because it would require the resolution of a range of technical issues about hybrid intensional/extensional modeling that it is not clear how to think about.

CEqEA treats cascaded causation diagrams and causation state spaces identically, meaning all code is shared, except for the respective node generation. This includes one piece of code for CCP<sup>all</sup> traversals of both types of graphs. Technically, causation state spaces are always of combinatorial size while cascaded causation diagrams will tend to be of low polynomial size. Practically, causation state spaces are less comprehensible than cascaded causation diagrams for reasoning purposes and can even be difficult to inspect visually. This is partly due to their closed-system nature (everything is always accounted for), which, e.g., means that a change in an environmental condition will force a CCP<sup>all</sup> traversal over to a distinctly different part of the whole graph, and it is left to the user to infer the meaning of the topological differences between the two locations. For cascaded causation diagrams, changes in environmental conditions overwhelmingly allow us to stay in place in the graph, which means we only need to think about changes in the conditionals at hand. A related problem is that sub-system analysis with causation state spaces will often require re-generation of the right graph. For cascaded causation diagrams, sub-system analysis is subsumed by the open-system assumption, see article.

### S1.6.2 Coextensive + extensional: coextension state spaces

*Coextension state spaces* are constructed from the elementary diagrams by

- designating a set of schema instances to consider (see CEqEA\Help\CCP),
- constructing a node for each combination of a state from each,
- CCP-evaluating each constructed node as a compartment,
- inserting an edge for each partial or complete set of changes, where
- edges that capture a maximal number of changes are bolded.

(Coextension state spaces do not allow us to work with channels, either.)

Like for causation state spaces, all sustained equilibria collapse to one type. However, coextension state spaces contain two graphs: the bolded, max-change one, representing things that are most likely to happen, and the full graph including what may happen if updates proceed asynchronously. In particular,

boxes in the former may have out-edges in the latter and we reuse the full-lined/dashed box notation of Section S1.5 (for ‘collapsible’), except the boxes are grey to indicate their different semantics. Both graphs may contain divergences.

When constructing a coextension state space from a causation state space, the effect will be that all non-local CCP<sup>all</sup> steps (see Section S2.3.3:NB1) will give rise to a new edge while all pre-existing edges are retained (but collapsed to at most one per node pair). To keep our examples to an illustrative size, we proceed from the specializations considered in Section S2.4:

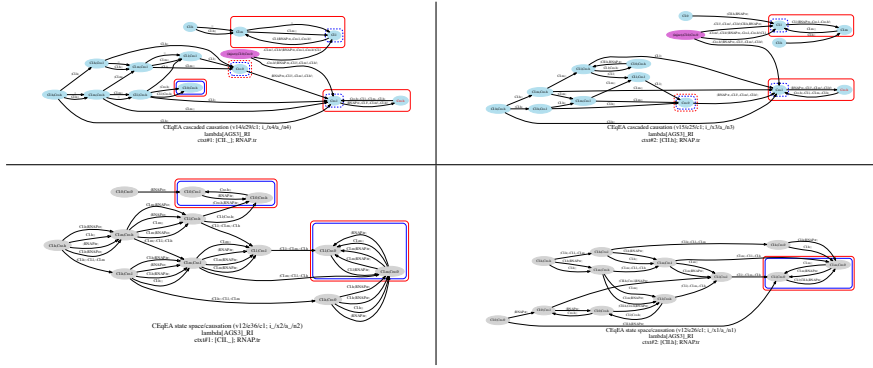

In the top row below, we have the two specialized coextension state spaces constructed via cascaded causation diagrams. At the bottom, we have the two coextension state spaces constructed via causation state spaces. The graphs are pairwise identical; this is likely a theorem.

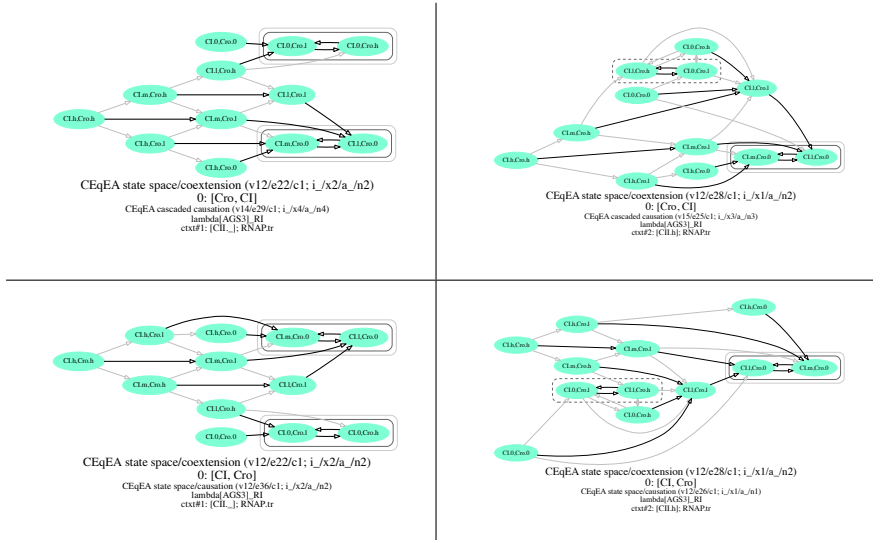

### S1.6.3 Coextensive + intensional: synchronization diagrams

As argued above, state spaces obfuscate the molecular pathway deciders we discuss in Section S2.4: the relevant information would need to be extracted back out from topological differences across a state space, assuming we can decide what places to compare. In particular, we can not predict causation synchronization from something as simple as looking at boxes within causation state spaces. For example, the following life-cycle predictions are from the just-considered cascaded causation diagrams (top) and causation state spaces (bottom):

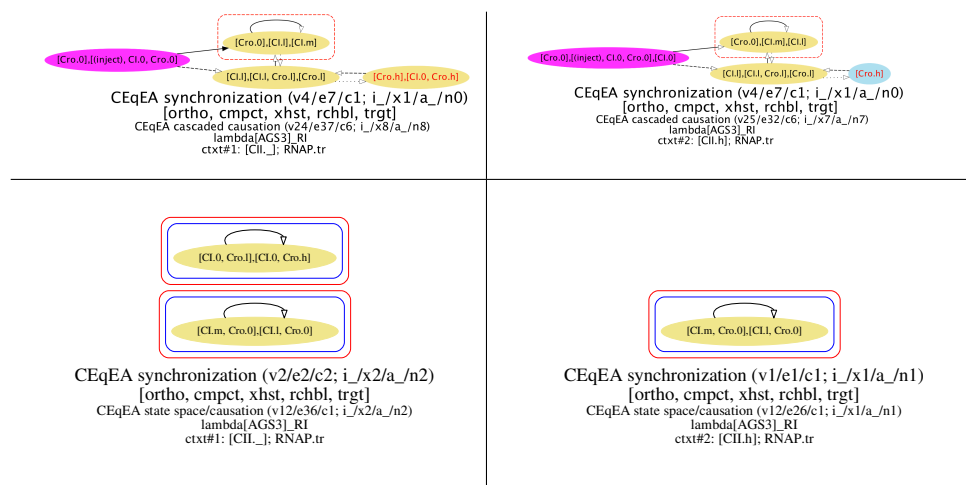

For the top graphs, see the article. The dotted arrow at the start of this section (S1.6) reflects the degeneracy of the bottom (outcome-/extensionality-derived) graphs as compared to the information captured by the top (process-/intensionality-derived) graphs. A life cycle, like reasoning but unlike properties, is an intensional notion that is not easily recovered from extensional data.

## S2 CEq practice: ab-intra reasoning

Our starting point is the observation that there is a community-wide molecular-biology reasoning style, connecting molecules and biology. The style proceeds bottom-up but is also used counterfactually/for inverse problems: what molecular premises would (not) justify a given biological conclusion.

**App.SA** [28]’s ‘motivation’: aims of the reasoning style.

**App.SB** [28]’s ‘axioms’: means of the reasoning style.

**App.SC** [28]’s ‘molecular basis’: organism-specific premises.

**App.SD** [28]’s ‘population inferences’: anonymizing individuals in populations.

**App.SE** [28]’s ‘causation arguments’: discrete regulatory causes and effects.

**App.SF** [28]’s ‘pathway arguments’: interference between causes and effects.

**App.SG** [28]’s ‘cell behaviors’: observable properties of given cell types.

**App.SH** [28]’s ‘superseded’ aspects of earlier editions due to recent discoveries.

The CEq framework axiomatizes the reasoning, see article.

We refer to our formal treatment of the monograph organism as  $\lambda^{[AGS3]}$ .

**Section S2.1** presents a general modeling methodology for capturing an organism’s ‘molecular basis’ formally and applies it to the relevant factual statements from [28], see Appendix SC, resulting in the  $\lambda^{[AGS3]}$ -*genotype*.

**Section S2.2** bridges Appendix SC to Appendix SE, via Appendix SD: a key contribution is to show that the bridging can be done automatically, aka (regulatory) form-to-function compilation to physiology changes. Our presentation here focuses on the operational aspects. The logic side is developed in Section S1.3.

**Section S2.3** presents a body of CEqEA-verified formal reasoning that dissects the reasoning space underlying [28]: the  $\lambda^{[AGS3]}$ -*phenotype*. The considered properties sit between Appendices SF–SG in a way that covers both. We reason over the abstraction introduced for Appendix SE: causations, see Figure 3.

**Section S2.4** applies our *synchronotyping* technology to  $\lambda^{[AGS3]}$ , see Section S1.5, to predict observable concentrations and organism life cycles by sequentializing the permissible open-system concurrent reasoning.

**Section S2.5** applies our technology first-principle style: purely computationally.

The appendices show that [28] is subsumed by our development, see article.

## S2.1 A programmed Genetic Switch: the $\lambda^{[AGS3]}$ genotype

We transliterate [28]’s ‘molecular basis’ into formal form. This covers the monograph organism’s molecule interactions: recruiting, inhibition, transcription, activation, proteolysis, etc.

### S2.1.1 MIG/RI specification

In order to faithfully capture an organism’s molecular programming, CEqEA’s *MIG (Modal Influence Graph) specification language* is intended to be used with our *RI (Regulation Interface) modeling methodology*:

|                                                                     |    |
|---------------------------------------------------------------------|----|
| S2.1.2 Modality defaults (fixed)                                    | 42 |
| S2.1.3 Categories (incremental)                                     | 45 |
| S2.1.4 Schemas, instances, states (incremental)                     | 46 |
| S2.1.5 Intrinsic affinities: transposing individuals to populations | 48 |
| S2.1.6 Regulatory bindings: precedence and cooperativity offsets    | 50 |
| Technology overview: operator macros and state ranges               | 50 |
| S2.1.7 Regulation: inhibition and active contravariance             | 57 |
| Technology overview: heuristic for binding vs contravariance        | 59 |
| S2.1.8 Influences: coinhibition and passive contravariance          | 64 |
| S2.1.9 Special circumstances and seeds                              | 69 |

We are considering information with the following kind of illustration, see [[28]:xiv:21]/App.SA.

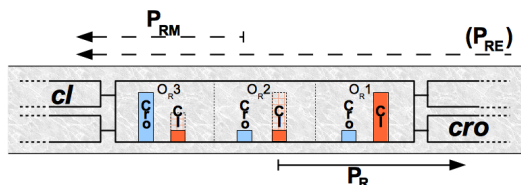

The illustration is for a part of Bacteriophage  $\lambda$ 's genome, i.e., the monograph organism, with recognizable genes ( $cI$ ,  $cro$ ), operators ( $O_{R1}$ ,  $O_{R2}$ ,  $O_{R3}$ ), and specific transcription (from promoters  $P_{RM}$ ,  $P_{RE}$ ,  $P_R$ ). The information includes the direction of transcription (arrows), possibly the outermost RNAP contact point (flat arrow tails), the name of the originating promoter (with upstream sites in parentheses), whether the transcription requires RNAP recruitment to be physiological (dashed arrows), the relative intrinsic affinities of specific molecules<sup>4</sup> for the operators (histograms), and the possibility of variable effective affinities (dashed histograms) owing to cooperative binding or similar. CEqEA is a bottom-up modeling environment and information that can not be captured by this type of illustration is likely to belong to the output of CEqEA. It is not uncommon to get this directionality wrong but even minor slips can be problematic: “[*nucleosome modifiers*], like the very many proteins recruited to genes by specific transcription regulators, are parts of a response, not a cause [...] Labeling histone modifications “epigenetic,” moreover, obscures what we know” [30].

Language purity and abstraction were prioritized in the design of the MIG language over any attempt to make it safe or just right for any particular (type of) application. This was done for parsimony and semantic transparency: clean concepts, processing, and execution. The RI modeling methodology is based on established molecular-biology practice but also contains prescripts due to us. For example, Sections S2.1.7–S2.1.8 comprehensively address: “one of the often unnoted complexities of biological systems is the imposition of inhibitors or other strategies to suppress basal reactions” [29]. Of course, RI needs to be backed by language features and, e.g., the ‘modal’ in MIG refers to part of our treatment of “the detailed biochemistry of protein-DNA interactions” [12]. See the technology overview in Section S2.1.7 for a broad exposition of these issues and note that the referenced complexity is substantial, see Section S1.3.1.

**A fundamental principle of RI is that all differential molecule interactions are specified explicitly and independently, and that**

<sup>4</sup>We refer to the protein product of the  $cI$  gene as ‘CI’. It is also known as ‘repressor’.

**each governing regulatory expression is assigned to a suitably-named *MIG macro*.**

MIG macros are named regulatory expressions that may be inlined in later expressions. They will be iteratively composed and assigned names in the structured manner of molecular biologists until we have accounted for the molecular underpinnings of gene expression and any similar effects. This implies that the depth of macro dependency will vary from case to case and, while it is not too deep for  $\lambda^{[AGS3]}$ , we trust the general pattern is clear [29]. For example, neither translation to nor dimerization of **CI** and **Cro** are differential aspects of  $\lambda$  gene regulation, only overall expression to the regulatory dimer form is. This implies that mRNA and monomers will not occur explicitly in the specification we are about to construct. Following [28],  $\lambda^{[AGS3]}$  treats the intermediate forms transparently, see [[28]:5:-5]/App.SB.

A MIG specification consists of a number of distinct types of information that we now discuss in their recommended order of appearance. Except for a few special cases, such as declaration before usage, MIG sentences may appear in any order without having their meaning affected. Each piece of MIG syntax we present here references the main factual statement in [28] (or similar) that it transliterates under RI. File `lambda[AGS3]_RI.mig` contains the full MIG/RI specification for  $\lambda$  following [28], called the  $\lambda^{[AGS3]}$  genotype. Section S2.1.10 references all ‘molecular basis’ statements in [28] from the MIG syntax they are associated with. Appendix SC does the converse. There is considerable redundancy in [28] but no contradictions.

### S2.1.2 Modality defaults (fixed)

*Modalities instantiate the CEq theory, with the defaults listed here likely to be shared by all MIG/RI specifications of molecular biology. It is reasonable to reuse the provided syntax.*

CEqEA captures an abstract theory of cause, effect, and emergence from their interconnectedness, called *the CEq theory*. The theory with its various modal instantiations goes beyond our consideration of [28] and we shall merely articulate and justify the specific semantics of molecular biology we commit to by our choice of modality values, as opposed to spelling out the details. This includes discussing only the modalities that we vary or otherwise need to know about.

The general meaning of the default modality values we present is that molecule populations in cells are governed by interacting processes that behave discretely, as if they could be expressed as information flowing between and affecting individuals (but see Section S1.5). Exceptionally, molecular kin-on-kin interaction will be specified using a MIG construct that resembles but is distinct from the constructs used for regulation proper. The kin-on-kin construct (`excl`) is governed by classical logic, see Section S1.1.6, meaning we are concerned only with whether a kin is present or not: no information flow is being considered for kin-on-kin interactions and they are not subject to the modalities. What we advocate for molecular biology more precisely is to extrapolate population behaviors from the behavior of individuals without the ability to distinguish individuals within populations. Our axiomatization of the “information flow” part of molecular-biology reasoning is a fragment of intuitionistic logic, see Section S1.1, with non-standard proof theory of independent interest, see article. CEqEA’s “there-or-not” logic is effected statically as the ‘population inference’ part of the parsing of MIG macros, see Appendix SD.

```

1  /*****
2  /* modality      = default ; */
3  *****/

5  Instantiation    = coherent ;           //[12:7]
6  Regulation      = intrinsic ;          //[Ptashne:NatChemBio7]
7  Causation       = pushpull ;           //[Ptashne:NatChemBio7]
8  Termination     = endpoint ;           //[Ptashne:NatChemBio7]
10 Solution        = fixed ;              //[8:-16][94:12]

```

**[Ptashne:NatChemBio7] :**

*“In general, recruiting reactions require the continuous action of recruiters for maintenance. For example, a gene does not stay on once activated unless polymerase is continually recruited by the action of an activator.”*

The **Termination** modality ranges over **approximate**, **endpoint**, **ceaseless** — in order, these do not target the extreme of a specified sequence of changes, target it exactly, and target the extreme plus maintain it, see below. Having **endpoint** as default value establishes a contract that the RI modeling methodology must ensure is met, or an alternative modality value must be specified locally, using the appropriate syntax. We use this modality value because the norm is that causes get terminated: we reach zero concentration, (auto-)inhibition becomes the dominant effect, etc. The **Causation** modality ranges over **push**, **pull**, **pushpull** — in order, these say to treat potential change sources, targets, or both as *points of interaction* (PoIs), which amounts to checking that all requisite mediators are supplied in the relevant end(s). (The principal way this is done here is by constructing corresponding cascaded-causation-diagram nodes, see Section S1.4.1.) The quotation explicitly calls for **pushpull**. The **Regulation** modality ranges over **intrinsic**, **extrinsic**, **incidental** — in order, these say that given regulators must, will not, or may serve in that role in the specified locations in and around the processes of change: here, in all locations. (Inhibitors may not be **incidental**.)

**[[28]:12:7]/App.SC :**

SUPPRESSED

The **Instantiation** modality ranges over **coherent**, **mixed** — in order, these say that it is or is not enforced that a ‘schema instance’ may be in only one ‘state’ at a time, see Section S2.1.4: are we looking at uniform population behaviors, say, within a compartment?

**[[28]:8:-16]/App.SB :**

SUPPRESSED

**[[28]:94:12]/App.SC :**

SUPPRESSED

The **Solution** modality ranges over **empty**, **fixed**, **appear**, **appearOK**, **vanish**, **vanishOK**, **change**, **changeOK** — in order, these enforce that parts of PoIs that are not involved in a physiology-changing interaction, i.e., solution, are empty, unchanged, will/may be added to, will/may disappear, will/may change in some way during the resulting effect, see Section S1.4.1. The **fixed** value is appropriate when all changes proceed at a single time scale within a compartment. It is not appropriate for DNA traversal across membranes into new compartments, see Section S2.1.9. Generally speaking, PoIs allow for non-negative role re-assignment for molecule populations as changes cascade onto each other, e.g., product to mediator.

### S2.1.3 Categories (incremental)

This section is problem(-domain) specific: it declares the user-named categories of entities that may occur in a particular MIG/RI specification. This will typically mean the classes of considered molecules. The content is added incrementally under RI as the remainder of the specification is developed. [28] explicitly summarizes the information we end up adding for  $\lambda$ , and we include the quotations for reference. We recommend annotating categories, e.g., with **I** and **C** to distinguish between individuals and concentrations, and similar for any other distinctions that apply. For molecular biology, **\$genomeI** and **\$proteinC** will always be included. The distinction between **\$dnaCI** and **\$genomeI** below is between generic DNA and particular genomes: **\$dna\_I** and **\$genomeI** are not treated as one to reflect that [28] does not explicitly discuss, e.g., DNA repair. Making up regulatory mechanisms that it seems could be behind specific effects will almost certainly fail to work as intended and is likely to create problems.

```
13  /*****  
14  /* categories      = $abstraction ; */  
15  *****/  
17  categories        = $dnaCI, $genomeI, $proteinC ;           //[95:2][11:1][12:-8]
```

**Category names should be ordered left-to-right according to how the molecules give rise to each other, in line with Crick's Sequence Hypothesis [5]. They must be prefixed with the reserved symbol '\$'.**

[[28]:95:2]/App.SC :

SUPPRESSED

[[28]:11:1]/App.SC :

SUPPRESSED

[[28]:12:-8]/App.SC :

SUPPRESSED

**categories** should be used meticulously: they delineate subtleties, prevent many kinds of modeling mistakes, and catch inadvertent misconceptions. In other words, they prevent category mistakes. This means that they are the reasoning equivalents of units of measurement in calculations. From the formal-reasoning perspective, **categories** are the relevant types although CEqEA does not currently implement a type system proper.

### S2.1.4 Schemas, instances, states (incremental)

Also this section is built incrementally from details we consider later under RI. As above, [28] summarizes the relevant information, which we include for reference here, too. For molecular biology, the section declares the relationships between any genes we consider, represented by *MIG schemas*, and their various relevant products, represented by MIG schema *instances* at the corresponding categories. The section may also list regulatory factors without consideration of their origin. Each declaration pivots around a ‘.’ — on its left are the schema name and a base category; on the right are its not-further-named instances at specified categories, with a listing of the relevant differential states within each (see later for the states to add).

```
$baseCat / schema . $instCat1 / [s1...sA]
...
$instCatL / [sM...sN] ;
```

If no category is listed to the right of the ‘.’, the category on the left carries over.

**Each listed category must be included in the categories declaration.**

A `$proteinC` instance will typically have symbolic representations of certain nominal concentrations as states but may also express whether a sufficient concentration of a protein is activated, or similar, see Section S2.1.5. States with a default regulatory effect are enclosed in `{ }` — these are called *active* states. A default order in which the states may change into each other may be indicated within `[ ]`. Alternatives may be indicated by infix `%`, and `[ ]` and `%` may be arbitrarily nested. Explicitly-unordered states may be declared within `[ [ ] ]`.

We already know that we will add the `cI` and `cro` genes, meaning entities with `$genomeI` base category. We also know about RNAP with `$proteinC` instance category and a `tr(-anscribing)` state. By listing only one state for RNAP, we implicitly stipulate that the enzyme is always available for transcription, see [[28]:15:11]/App.SC. For all other schema instances, we explicitly introduce a non-active state: zero, unactivated, double-stranded (generic DNA), or similar.

**By default, include a regulatorily-neutral state when starting each instance declaration and suitably rename it at the end to match the naming scheme of the active states — ensure that the introduced states in a schema instance follow a single naming scheme and that the scheme matches the instance category.**

```
20 | /*-----*/
21 | /* $level/schema . $level/states [l modalities] ; */
22 | /*-----*/
24 | /*regulatory factors: E. coli*/
25 | $dnaCI / DNA . [ {ss} ds ] ; // [95:2] + intrinsic
```

```

26 | $proteinC / RNAP . {tr} ; // [15:11]
28 | /*regulated components: E. coli*/
29 | $proteinC / RecA . [ "" {s} ] ; // [24:5] + intrinsic
32 | /*regulatory factors: lambda*/
33 | $proteinC / CII . [ _ {h} ] ; // [56:-1a] + intrinsic
35 | /*regulated components: lambda*/
36 | $genomeI / cI . $proteinC / [ 0 {1} {m} {h} ] ; // [12:-8] + intrinsic+induced
37 | $genomeI / cro . $proteinC / [ 0 {1} {h} ] ; // [12:-8] + intrinsic

```

In the above, "" represents the empty string, meaning we distinguish `RecA.` and `RecA.*`: whether the `RecA` population includes a physiological concentration of activated individuals.

`[[28]:95:2]/App.SC :`

SUPPRESSED

`[[28]:15:11]/App.SC :`

SUPPRESSED

`[[28]:24:5]/App.SC :`

SUPPRESSED

`[[28]:56:-1a]/App.SC :`

SUPPRESSED

`[[28]:12:-8]/App.SC :`

SUPPRESSED

State names must be unique within schemas and, e.g., the `h` state of the `$proteinC` instance of the `cro` schema will automatically be capitalized by CE-qEA as `Cro.h`. This is done when a state belongs to an instance at a category that is declared to the right of the schema's base category. Technically, schemas (and only schemas) are case-insensitive.

### S2.1.5 Intrinsic affinities: transposing individuals to populations

Stipulate the existence of nominal interface-transposing states for molecules that bind differentially to operators and similar. Declare and categorize the states above, enclose them in { }, and assign them to *domain-free* macros, see below. Macro names must be prefixed with the reserved symbol '@'.

For example, introduce an *h* state, for high concentration, for any molecule that binds to some site with low affinity: the nominal concentration represents when the particular binding may start having a material effect. This constitutes a firm commitment to the considered states being physiological in nature. Everything will still work at the technical level if other types of states are used but the expressed semantics will not match the expected semantics downstream and no specific type of meaning can be assigned to any results: using other types of states would constitute a fundamental category mistake within the CEqEA universe. For example, we explicitly predict observable states at the end of our formal treatment, once all the physiological factors that affect the issue have been brought together, see Section S1.5.

```

40  /*****
41  /* @macro<>      = transposed interface ; */
42  *****/
44  @OR1_CI_int<>    = CI.l ;                //[86:F4.18:1]
45  @OR2_CI_int<>    = CI.h ;                //[86:F4.18:1]
46  @OR3_CI_int<>    = CI.h ;                //[86:F4.18:1]
48  @OR1_Cro_int<>   = Cro.h ;               //[25:F1.23:1]
49  @OR2_Cro_int<>   = Cro.h ;               //[25:F1.23:1]
50  @OR3_Cro_int<>   = Cro.l ;               //[25:F1.23:1]
52  @ORE_CII_int<>   = CII.h ;               //[55:6][56:-1a]
54  @UV_irr_int<>    = DNA.ss ;              //[60:-7]
55  @SOS_int<>       = RecA.* ;              //[60:-7]

```

As seen in the '2' below 'OR1' in the first figure below, CI will bind to this site with relatively high intrinsic affinity. We represent this formally by introducing an *l* state for the *\$proteinC* instance of the *cI* schema, i.e., we assert that the binding may be physiological at a symbolic low concentration of *CI*. We assign this state to a macro named according to the pattern:

@[site]\_[molecule]\_int<>

The suffixed '<>' is not part of the name but makes the macro *domain-free*: the name only applies within the MIG specification. If the suffix is omitted, CEqEA will emit the defined name whenever this binding plays a regulatory role in subsequent reasoning. In later sections, we introduce macro names that capture in what circumstances a binding like this does play a regulatory role, including a macro called @OR1\_CI. As we shall see, the regulatory macro is different from the intrinsic-binding macro above.

[[28]:86:Fig.4.18:1]/App.SC :

SUPPRESSED

[[28]:25:Fig.1.23:1]/App.SC :

SUPPRESSED

[[28]:55:6]/App.SC :

SUPPRESSED

[[28]:56:-1a]/App.SC :

SUPPRESSED

[[28]:60:-7]/App.SC :

SUPPRESSED

We introduce the name `ORE` for a putative CII-binding `ORE` operator although [28] does not discuss or provide evidence that such a site exists: this is the best we can do with [[28]:55:6]/App.SC. Similarly, we conflate various physical steps in the naming of `@UV_irr_int`, for reasons of argumentation nomenclature: in effect, we follow [28]. Neither is desirable in general.

## S2.1.6 Regulatory bindings: precedence and cooperativity offsets

### *Technology overview: operator macros and state ranges*

---

An important aspect of RI's recommended use of the MIG macro system concerns the referencing of macros for (regulatory) operators in combination with MIG's two types of ranges, namely ranges proper: `--`, `+-`, `-+`, `++`, and next-to constructors: `+`, `(+)`.

**Macros:** Domain-free macros for operators ending in `_rng` (for 'range') always occur by themselves. Those ending in `_int` (for 'intrinsic') may occur with a next-to constructor. Macro references for operators that are not domain-free always occur with a range proper. This may be as part of a collection of occurrences, see Section S2.1.7.

**Ranges:** A dash: `-`, means end-inclusive, a plus: `+`, means end-exclusive. Ranges are evaluated relative to the active states (in `{ }`) within `[ ]` in schema declarations — plus takes precedence and non-active end-points may be explicitly included. Ranges proper may have arguments on either side, or on both sides. Next-to constructors must have an argument on exactly one side. The difference between the two next-to constructors is in their treatment of extreme active states. Consider `e . [0 {1} {2} {3}] ;:`

|                         |                |                                    |                      |                |                  |
|-------------------------|----------------|------------------------------------|----------------------|----------------|------------------|
| <code>e.1 -- e.3</code> | <code>=</code> | <code>e.1 : e.2 : e.3</code>       | <code>e.1 +</code>   | <code>=</code> | <code>e.2</code> |
| <code>e.1 +-</code>     | <code>=</code> | <code>e.2 : e.3</code>             | <code>e.1 (+)</code> | <code>=</code> | <code>e.2</code> |
| <code>e.1 -+</code>     | <code>=</code> | <code>e.1 : e.2</code>             | <code>+ e.1</code>   | <code>=</code> |                  |
| <code>++ e.2</code>     | <code>=</code> |                                    | <code>(+) e.1</code> | <code>=</code> | <code>e.1</code> |
| <code>e.2 ++</code>     | <code>=</code> |                                    |                      |                |                  |
| <code>e.2 -+ e.2</code> | <code>=</code> |                                    |                      |                |                  |
| <code>e.0 --</code>     | <code>=</code> | <code>e.0 : e.1 : e.2 : e.3</code> |                      |                |                  |

**Range exclusion:** Macros may be declared with a set of states that will be excluded from ranges applied to the macro using the `excl` keyword:

- `@loc1_e = e.1 excl e.2 -- ;` results in `@loc1_e --` being `e.1`.
  - `@loc2_e = e.1 excl e.1 ;` results in `@loc2_e` defined to be no state; note that `loc2_e --` will also be no states, as opposed to `e.2 : e.3`, say.
-

```

58 /*****
59 /* @macro      = regulatory binding [precedence] ; */
60 /*****/

```

Earlier, we addressed the possibility of molecular binding and, where applicable, made a symbolic transition from individuals' affinities for the binding to the nominal population concentrations for which such bindings may be physiological. Now we address the population-specific aspects of those bindings, partly by using CEqEA's state-range technology, see above.

Macros for regulatory bindings must be written in order of precedence due to declaration-before-usage. For auto-cooperative bindings, this typically means in order of widest physical range. (CEqEA also has support for mutually-exclusive bindings, see Section S2.5.2.)

**CI octamer+tetramer** For  $\lambda^{[AGS3]}$ , we first address the recently uncovered possibility of long-distance and DNA-looping CI octamerization facilitating simultaneous and similarly long-distance CI tetramerization, i.e., we specify the possibility of joint octamer+tetramer binding. (See Section S2.5.1 for the consequences of the absence of this mechanism.)

**State assignments for cooperative bindings should be offset from the relevant intrinsic values, see technical overview above, and new (typically lower and implicitly-transposed) states should be declared to accommodate the offset, where warranted.**

```
63 | @OLR123_CI      =  (+) @OR3_CI_int  ;           //[112:9]
```

[[28]:112:9]/App.SC :

SUPPRESSED

Given the gap between ‘2’ and ‘25’ in [[28]:86:Fig.4.18:1]/App.SC below, we add an intermediate active state, *m* for *medium* concentration, to the CI declaration to represent the implied binding.

**CI octamer** Octamer binding to  $O_{\{L,R\}}\{1,2\}$  may happen without the  $O_{\{L,R\}}3$  tetramer: the octamer binds before the tetramer, and we specify it independently. We use the state-offset notation from above but we do not stipulate the existence of a distinct concentration below low (but still wish to be able to extend our analysis to mutants, and similar, see Section S2.5). We deem a lower state unwarranted partly because the ‘2’ binding is intrinsically but not regulatorily relevant in a way that means we re-purpose the 1 state at the regulatory level.<sup>5</sup>

**When precedence among regulatory bindings involves a single schema instance, express it with the `excl` construct of MIG’s macro-declaration facility.**

64

```
@OLR12_CI = (+) @OR1_CI_int excl @OLR123_CI-- ; // [86:F4.18][110:-4]%subsumed
```

Here, we express that the octamer-only binding is subsumed by the octamer+tetramer binding: the binding is not octamer-only when the tetramer binding is also physiological.

[[28]:86:Fig.4.18:1]/App.SC :

SUPPRESSED

[[28]:110:-4]/App.SC :

SUPPRESSED

---

<sup>5</sup>A future version of the RI modeling methodology will address this issue in a principled way.

**Shorthands** CI will have pervasive effects when it is bound physiologically to  $O_{\{L,R\}}\{1,2\}$ , irrespective of whether it also binds to  $O_{\{L,R\}}3$ . We capture this with a domain-free macro ( $\langle \rangle$ ):

```
66 | @OLR12?_CI_rng<> = @OLR123_CI-- : @OLR12_CI-- ; // %abbreviation
```

## Non-cooperative bindings with precedence

When precedence among regulatory bindings involves different schema instances, express it with the inhibition connective: |--.

We stress that `excl` vs |-- is a fundamental modeling distinction with concrete reasoning consequences, and the two should not be used interchangeably.

```
69 /*OR1*/
70 @OR1_CI      = @OR1_CI_int      excl @OLR12?_CI_rng ; //intrinsic%subsumed
71 @OR1_Cro     = @OR1_Cro_int      |-- @OLR12?_CI_rng ; //intrinsic[17:6]

73 /*OR2*/
74 @OR2_CI      = @OR2_CI_int      excl @OLR12?_CI_rng ; //intrinsic%subsumed
75 @OR2_Cro     = @OR2_Cro_int      |-- @OLR12?_CI_rng ; //intrinsic[17:6]

77 /*OR3*/
78 @OR3_CI      = @OR3_CI_int      excl @OLR123_CI-- ; //intrinsic%subsumed
79 @OR3_Cro     = @OR3_Cro_int      |-- @OLR123_CI-- ; //intrinsic[17:6]
```

[[28]:17:6]/App.SC :

SUPPRESSED

In the above, the states referenced by `@OLR12?_rng` are guaranteed to include the state referenced by `@OR1_CI_int`, which means that the `@OR1_CI` declaration is null-and-void, i.e., it refers to no states. CeqEA allows for this and references to the macro will simply contribute nothing to their local context. For maintainability during development and readability after, it is best to specify all possible bindings and let CeqEA deal with issues of vacuity, etc.

## Non-cooperative bindings without precedence

When an operator binding does not involve cooperativity or precedence, promote the intrinsic binding directly to a regulatory binding.

```
81  /*"ORE"*/  
82  @ORE_CII      = @ORE_CII_int ;                %%intrinsic  
  
84  /*cytosol*/  
85  @UV_irr      = @UV_irr_int ;                  %%intrinsic  
86  @SOS         = @SOS_int ;                      %%intrinsic
```

## S2.1.7 Regulation: inhibition and active contravariance

```

89  /*****
90  /* @macro = regulation ; */
91  /*****

```

MIG/RI specification of promoter action, and similar, also follows a standard format:

```

@[promoter]_tr = RNAP.tr
    & ^([recruiting1] : ... : [recruitingM])
    |-- [inhibition1]
        : ...
        : [inhibitionN]
    ;

```

Inhibition, |--, has widest scope and the text codes for the following abstract syntax tree:

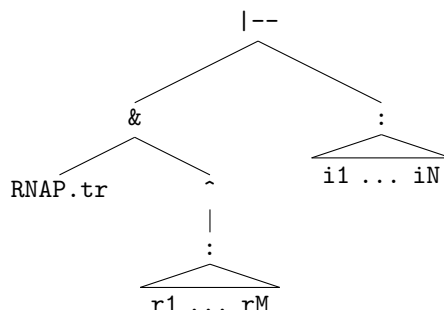

Each [recruiting\_] represents a distinct molecule complex that is able to attach RNAP to the promoter, or similar. In case of constitutive transcription, there should be no [recruiting\_]s. The ‘~’ symbol is MIG’s indirect operator. It is annotated to things that help with but do not undertake considered work. Direct and indirect regulators may be subject to different default modality values but this does not appear to be warranted for molecular biology, see Section S2.1.2 and [29]. Direct and indirect inhibitors are subject to different presumptions in our subsequent computational analysis and indirection should not be omitted, see Section S1.5.

The main conceptual challenge in this section is to specify the [inhibition\_] expressions in such a way that we account not for when transcription may or may not go ahead in a physical sense, as this would be part of the individual-molecule world we considered earlier, in contrast to the population world we have already transitioned to. Rather, we need to pinpoint the net effects on transcription that different types of inhibition allow for, taking into account also transient loss of binding and the rates of natural dilution (meaning decay, transport, etc.) of the expressed products. Without the capacity for hybrid discrete and kinetics modeling, CEqEA cannot yet compute these types of net

effects precisely. Instead, the technology overview below provides a heuristic for how to anticipate net effects that seems to cover a large number of cases. Of particular note is the fact that the heuristic applies to the individual inhibition occurrences in isolation and that CEqEA automatically does the heavy lifting of putting these together across promoters to sort out the different combined effects that may result, see Section S2.2.<sup>6</sup>

---

<sup>6</sup>CEqEA does not currently cater to the so-far unsubstantiated possibility of higher-order regulation whereby the combined effect of multiple regulation sites is more than the sum of the parts, see [15].

The states we have introduced are physiological: they account nominally for when the associated bindings may have material effects. In terms of effect functions, this typically means the mid-point between the lowest and highest gross/in-vacuo effects. We take this point to balance out natural dilution by default in case of inhibiting bindings, i.e., for the specified physiological state to correlate with a neutral net/in-situ effect on the inhibited products. Our task here is to model this approximation correctly for different binding configurations and to pinpoint when opposite net effects, i.e., contravariance, can be expected.

First, we note that there will be a wide concentration range with an intermediate gross/neutral net effect for bindings with linear effect functions. For bindings with non-linear effect functions, there will be an increasingly narrower range with intermediate effect.

| binding    | [inhibition]                                                                                                                                                                                                                                                              |
|------------|---------------------------------------------------------------------------------------------------------------------------------------------------------------------------------------------------------------------------------------------------------------------------|
| single     | <code>@op_I</code><br><code>: @op_I +- !</code>                                                                                                                                                                                                                           |
| dual       | <code>@op1and2_I&lt;@op1_I,@op2_I&gt; = max&amp;(@op1_I,@op2_I) ;</code><br><code>@op1xor2_I&lt;&gt; = min: (@op1_I,@op2_I) excl @op1and2_I-- ;</code><br><code>...</code><br><code>@op1xor2_I</code><br><code>: @op1xor2_I +- !</code><br><code>: @op1and2_I -- !</code> |
| coop.      | <code>((+) min: (@op1_I_int,@op2_I_int)) -- !</code>                                                                                                                                                                                                                      |
| high coop. | <code>((+) min: (@op1_I_int,@op2_I_int)) -- ! {  incdnt1(I)&lt;mdtr,sink&gt;}</code>                                                                                                                                                                                      |

(‘dual’ is motivated by [[28]:93:Fig.4.24:1]/App.SC; ‘high coop.’ by [[28]:24:-8]/App.SC.)

- a single inhibiting binding results in a neutral net effect in the physiological state and contravariance (!) at any higher states;
- dual (non-cooperative) bindings are basically consistent with the single case but will also exhibit contravariance when both inhibitors are in or above their physiological states — this is accounted for by the macro with ‘and’ while the macro with ‘xor’, for exclusive-or, is for when exactly one site is occupied
  - `min/max` followed by `&` is null-and-void if one argument is null-and-void,
  - `min/max` followed by `:` skips null-and-void arguments,
  - the `<...>`s list the domains given to the macros, i.e., the names CEqEA emits (along with any ‘deeper’ names), when the bindings are used; if omitted, the defined name is emitted; for the ‘xor’-macro, the “min” name will be emitted:

- cooperative bindings are contravariant from one lower than the physiological states and, being associated with a non-linear response function, has no neutral net effect;
  - highly cooperative bindings may outlast depletion of their non-bound concentration, see [[28]:24:-8]/App.SC: the inhibitor is an **incidental** (**incdntl**) **mediator** (**mdtr**) at the **sink** (target) of any contravariant change; this modality value captures that the binding is comparable to the time it takes to effect a physiological change, with the qualified concentration referring to free concentration, i.e., not the binding.
-

**P<sub>RE</sub> transcription** For P<sub>RE</sub> transcription, and absent information for the means of the inhibition in [[28]:55:-2]/App.SC, we specify that it must involve octamer binding: we surmise further to the NB! in Section S2.3.2:3/d/ that only the octamer binding is strong enough to prevent progress of the intra-helix traversal by RNAP from the upstream P<sub>RE</sub>. See also [[28]:37:15]/App.SC. [[28]:24:-8]/App.SC implies that the inhibition follows the highly-cooperative case in the technology overview.

```

105 | @PRE_tr = RNAP.tr //[136:21][6:-9a]
106 | & ~@ORE_CII-- // [136:21]
107 | |-- @OLR12?_CI_rng ! { |incdnt1(CI)<mdtr,sink>} // [55:-2][24:-8]
108 | ;

```

[[28]:136:21]/App.SC :

SUPPRESSED

[[28]:6:-9a]/App.SC :

SUPPRESSED

[[28]:55:-2]/App.SC :

SUPPRESSED

[[28]:24:-8]/App.SC :

SUPPRESSED

**P<sub>RM</sub> transcription** For P<sub>RM</sub> transcription, [[28]:24:-8]/App.SC implies that the CI octamer+tetramer inhibition involving O<sub>{L,R}</sub>{1,2,3} follows the highly-cooperative case in the technology overview. We note that highly-cooperative CI is specified as **incidental** (`incdnt1`) in any contravariant effects from its inhibitor role, i.e., when decay of the gene product becomes physiological, see Section S2.2, but not as recruiter. This is in accordance with [[28]:24:-8]/App.SC because of the coinhibition we discuss in Section S2.1.8: the binding may remain in place but it is disconnected from the concentration of CI during the host SOS response, specifically during **RecA.\*** cleavage of the CI product of **cI**.

```

110 @PRM_tr = RNAP.tr // [14:6] [6:-9a]
111 & ^(@OLR12_CI-- : @OR2_CI--) // [19:6]
112 |-- @OR3_Cro // [44:9]
113 : @OR3_Cro +- ! // [44:9]
114 : @OR3_CI // [44:9]
115 : @OR3_CI +- ! // [44:9]
116 : @OLR123_CI -- ! { |incdnt1(CI)<mdtr,sink> } // [44:9] [113:F5.5] [24:-8]
117 ;

```

[[28]:14:6]/App.SC :

SUPPRESSED

[[28]:6:-9a]/App.SC :

SUPPRESSED

[[28]:19:6]/App.SC :

SUPPRESSED

[[28]:44:9]/App.SC :

SUPPRESSED

[[28]:113:Fig.5.5:1]/App.SC :

SUPPRESSED

[[28]:24:-8]/App.SC :

SUPPRESSED

**P<sub>R</sub> transcription** For P<sub>R</sub> transcription, [[28]:24:-8]/App.SC implies that the CI octamer inhibition involving  $O_{\{L,R\}}\{1,2\}$  follows the highly-cooperative case in the technology overview. [[28]:93:Fig.4.24:1]/App.SC implies that the other bindings follow the dual (non-cooperative) case of the technology overview, which explains the macros prior to the PR\_tr macro proper.

```

125 @OR1and2_Cro<@OR1_Cro,@OR2_Cro> = max&(@OR1_Cro,@OR2_Cro) ; //[93:F4.24:1]
126 @OR1xor2_Cro<> = min: (@OR1_Cro,@OR2_Cro) excl @OR1and2_Cro-- ;//[93:F4.24:1]

128 @OR1and2_CI<@OR1_CI,@OR2_CI> = max&(@OR1_CI,@OR2_CI) ; //([93:F4.24:1])
129 @OR1xor2_CI<> = min: (@OR1_CI,@OR2_CI) excl @OR1and2_CI-- ; //([93:F4.24:1])

131 PR_tr = RNAP.tr // [14:6] [6:-9a]
132 /*& no recruiter*/ // [15:-4]
133 |-- @OR1xor2_Cro // [94:1] [93:F4.24:1]
134 : @OR1xor2_Cro +- ! // [94:1] [93:F4.24:1]
135 : @OR1and2_Cro -- ! // [94:1] [93:F4.24:1]
136 : @OR1xor2_CI // [94:1] ([93:F4.24:1])
137 : @OR1xor2_CI +- ! // [94:1] ([93:F4.24:1])
138 : @OR1and2_CI -- ! // [94:1] ([93:F4.24:1])
139 : @OLR12?_CI_rng ! { |incdnt1(CI)<mdtr,sink>} // [111:F5.3:1] [24:-8]
140 ;

```

[[28]:14:6]/App.SC :

SUPPRESSED

[[28]:6:-9a]/App.SC :

SUPPRESSED

[[28]:15:-4]/App.SC :

SUPPRESSED

[[28]:94:1]/App.SC :

SUPPRESSED

[[28]:93:Fig.4.24:1]/App.SC :

SUPPRESSED

[[28]:111:Fig.5.3:1]/App.SC :

SUPPRESSED

[[28]:24:-8]/App.SC :

SUPPRESSED

### S2.1.8 Influences: coinhibition and passive contravariance

(We have juxtaposed the related parts of Sections S2.1.7–S2.1.8 in the MIG/RI specification: `lambda[AGS3]_RI.mig`, for ease of reference. This may not always work.)

For the abstract case, see Section S1.3.1. Concretely, influences are specified as follows:

```
91  /*-----*/
92  /* +- | level / subject
93      | influence_expr
94      [| modalities] ; */
95  /*-----*/
```

We organize our specification of the effects of interface interactions around categories.

**On the right of the ‘/’ in an influence, specify how a regulatory expression applies to some (often lower-level) schema instance and, on the left, specify the effect this will have on named (often higher-level) schema instances that are not differentially regulated at some intermediate level.**

In our case, this means that we are interested in the effects for `$proteinC` (only). While intermediate categories exist, they are considered to be transparent in [28], see [[28]:5:-5]/App.SB.

**UV-irradiation** UV-irradiation damages DNA, which makes RecA change to its higher (+) activated state.

When going from a more stable to a less stable state of a schema instance, indicate that any products will be subject to (passive) contravariance by inserting a ‘!’ after the specified polarity: the opposite effect will be physiological in the absence of mediators and/or enzymes for the specified effect, see Section S2.2.

```
98 | + ! | $proteinC / RecA | @UV_irr ; // [24:1]
```

[[28]:24:1]/App.SC :

SUPPRESSED

The “manner not fully understood” appears to be conformation changes by binding of short single-stranded DNA but the details are not relevant here.

**SOS response** The SOS response from above mediates a negative (–) effect on CI, which affects not just the existing CI population but any CI that may continue to be expressed: **ceaseless**. The salient point behind the change of modality value is that gene expression is independent of RecA’s SOS actions and that it is only the gene product that is affected here. (Although the specifics are not detailed in [28], it should be noted that RecA cleaves CI monomers, see [[28]:24:5]/App.SC, while it is CI dimers that are physiological; this warrants further investigation.)

100

-
|
\$proteinC
/
CI
|
^@SOS
|
ceaseless
;
//[132:7]

[[28]:132:7]/App.SC :

SUPPRESSED

**CI expression** Transcription applies to the `$genomeI` base instance of `cI`, i.e., to the `cI` gene, which will have a positive effect on its considered product at the `$proteinC` level. This positive effect is coinhibited by `SOS`-mediated `CI` decay (`>@SOS<`): when also the `SOS` response is active, proteolysis will outpace any synthesis and the net effect will be negative.

Assemble all influences on a given schema instance in a pair of positive and negative influence declarations, and specify any coinhibition effect one may have on the other.

See Section S2.2 for how the actual contravariance is determined in cases like this.

119  
120

+>@SOS< ! | \$proteinC / cI | @PRE\_tr // [60:-7] [132:7] [56:1]  
: @PRM\_tr ; // [15:13]

[[28]:60:-7]/App.SC :

SUPPRESSED

[[28]:132:7]/App.SC :

SUPPRESSED

[[28]:56:1]/App.SC :

SUPPRESSED

[[28]:15:13]/App.SC :

SUPPRESSED

**Cro expression** For `cro` transcription, note that we specify that **Cro** is subject to passive contravariance: the synthesised protein decays naturally, i.e., the higher states the `+` takes us to are less stable than any of the lower states we come from, in and off themselves. CEqEA will automatically infer that a negative net effect will never result specifically from lacking recruitment because the transcription is constitutive, see Section S2.2.

```
142 | + !          | $proteinC / cro    | @PR_tr ;          |[15:13]
```

[[28]:15:13]/App.SC :

SUPPRESSED

### S2.1.9 Special circumstances and seeds

```

145  /*****
146  /* seed | modalities ; */
147  *****/

```

Some situations are special. This may be expressed by seeds and seed modalities. For example, by listing exit or entry, situations may be specified as (named) *channels* from or to a considered compartment.<sup>a</sup> Channels are subject to distinct processing in CEqEA and do not shadow non-channels or each other.

<sup>a</sup>CEqEA allows for any number of channels but only one compartment at this time.

[28] does not give details for how the observed host lysis is effected other than stating that it happens after **Cro** begins to bind to  $O_R\{1,2\}$ . We specify this with **expire**, to happen one step (the second 1) after **Cro** has reached its **h** state for the first time (the first 1).

```

149  "Cro.h"                | expire(1,1) ;                //[52:5/Late lytic]

```

[[28]:52:5/Late lytic]/App.SE :

SUPPRESSED

The considered host infection happens across a membrane, with no **CI** and **Cro** **\$proteinC** injected along the monograph organism's **\$genomeI**: we specify that either gene may be inert after **injection** (**vanishOK**<out>), that the lack of injected **CI** and **Cro** **\$proteinC** need not be representative of the entered environment (**mix**(**CI**,**Cro**)<out,src>), and that any pre-existing **\$proteinC** may impose mediating effects on the **injectee** (**incidental**<out,mdtr,src>).<sup>7</sup>

```

152  "CI.0, Cro.0" entry(inject) | vanishOK<out>,          //[12:7]
153                                mix(CI,Cro)<out,src>,      //[12:7]
154                                incidental<out,mdtr,src>;  //[12:7]

```

[[28]:12:7]/App.SC :

SUPPRESSED

The **out** qualifier is superfluous in this case: the seed is defined to be an **entry** channel, which means it is prevented from having effects going into it.

<sup>7</sup>Inhibitors cannot be **incidental**; they must be either **intrinsic** or **extrinsic**.

## S2.1.10 Complete references

### Preamble

#### Default modalities

```
5 Instantiation    = coherent ;                      //[12:7]
6 Regulation      = intrinsic ;                      //[Ptashne:NatChemBio7]
7 Causation       = pushpull ;                      //[Ptashne:NatChemBio7]
8 Termination     = endpoint ;                      //[Ptashne:NatChemBio7]
10 Solution        = fixed ;                          //[8:-16][94:12]
```

App.SC:[6:-9a, 11:1, 12:7, 12:-8, 94:12]

[[28]:8:-16]/App.SB is classified as an axiom, see Section S2.1.2.

For [Ptashne:NatChemBio7], meaning [29], see Section S2.1.2.

#### Categories

```
17 categories      = $dnaCI, $genomeI, $proteinC ;    //[95:2][11:1][12:-8]
```

App.SC:[6:-9a, 11:1, 12:-8, 95:2]

### Ground objects

#### Regulatory factors: E. coli

```
25 $dnaCI / DNA    . [ {ss} ds ] ;                  //[95:2] + intrinsic
```

App.SC:[95:2]

```
26 $proteinC / RNAP . {tr} ;                       //[15:11]
```

App.SC:[6:-9a, 12:-8, 15:11]

#### Regulated components: E. coli

```
29 $proteinC / RecA . [ " {*} ] ;                  //[24:5] + intrinsic
```

App.SC:[24:5]

#### Regulatory factors: lambda

```
33 $proteinC / CII . [ _ {h} ] ;                   //[56:-1a] + intrinsic
```

App.SC:[56:-1a, 57:3]

## Regulated components: lambda

```
36 | $genomeI / cI . $proteinC / [ 0 {l} {m} {h} ] ; // [12:-8] + intrinsic+induced
```

App.SC:[11:1, 12:-8]

```
37 | $genomeI / cro . $proteinC / [ 0 {l} {h} ] ; // [12:-8] + intrinsic
```

App.SC:[11:1, 12:-8]

## Transposed affinities

### CI intrinsic binding/operators

```
44 | @OR1_CI_int<> = CI.l ; // [86:F4.18:1]
45 | @OR2_CI_int<> = CI.h ; // [86:F4.18:1]
46 | @OR3_CI_int<> = CI.h ; // [86:F4.18:1]
```

App.SC:[12:-8, 17:2, 20:14, 86:1, 86:F4.18:1]

### Cro intrinsic binding/operators

```
48 | @OR1_Cro_int<> = Cro.h ; // [25:F1.23:1]
49 | @OR2_Cro_int<> = Cro.h ; // [25:F1.23:1]
50 | @OR3_Cro_int<> = Cro.l ; // [25:F1.23:1]
```

App.SC:[12:-8, 17:6, 24:-3, 25:F1.23:1, 84:12, 92:1a, 93:F4.24:1, 93:T4.4:1, 94:9, 94:11, 94:13]

### CII intrinsic binding/operators

```
52 | @ORE_CII_int<> = CII.h ; // [55:6] [56:-1a]
```

App.SC:[55:6, 56:-1a]

### Intrinsic cytosol bindings/“operators”

```
54 | @UV_irr_int<> = DNA.ss ; // [60:-7]
```

App.SC:[23:-1, 60:-7, 95:2]

```
55 | @SOS_int<> = RecA.* ; // [60:-7]
```

App.SC:[60:-7, 95:2]

## Regulatory binding

## Cooperative regulatory bindings

```
63 @OLR123_CI = (+) @OR3_CI_int ; // [112:9]
```

App.SC:[109:-6, 110:1, 110:3, 112:9, 112:F5.4:1, 114:F5.7:1]

```
64 @OLR12_CI = (+) @OR1_CI_int excl @OLR123_CI-- ; // [86:F4.18][110:-4]%subsumed
```

App.SC:[20:10b, 20:15, 21:-3, 86:1, 86:10, 86:F4.18:1, 109:10, 109:-6, 110:1, 110:3, 110:-4, 111:F5.2:1, 114:F5.7:1, 121:box:4, 146:4]

## Cooperative regulatory alternatives

```
66 @OLR12?_CI_rng<> = @OLR123_CI-- : @OLR12_CI-- ; // %abbreviation
```

(This is an abbreviation.)

## Singular regulatory bindings

```
69 /*OR1*/
70 @OR1_CI = @OR1_CI_int excl @OLR12?_CI_rng ; // %intrinsic%subsumed
71 @OR1_Cro = @OR1_Cro_int |-- @OLR12?_CI_rng ; // %intrinsic [17:6]

73 /*OR2*/
74 @OR2_CI = @OR2_CI_int excl @OLR12?_CI_rng ; // %intrinsic%subsumed
75 @OR2_Cro = @OR2_Cro_int |-- @OLR12?_CI_rng ; // %intrinsic [17:6]

77 /*OR3*/
78 @OR3_CI = @OR3_CI_int excl @OLR123_CI-- ; // %intrinsic%subsumed
79 @OR3_Cro = @OR3_Cro_int |-- @OLR123_CI-- ; // %intrinsic [17:6]

81 /*"ORE"*/
82 @ORE_CII = @ORE_CII_int ; // %intrinsic

84 /*cytosol*/
85 @UV_irr = @UV_irr_int ; // %intrinsic
86 @SOS = @SOS_int ; // %intrinsic
```

App.SC:[17:6, 94:9]

## Regulation + Influences

### Cytosol

```
98 + ! | $proteinC / RecA | @UV_irr ; // [24:1]
```

App.SC:[24:1, 60:-7, 94:-5]

```
100 - | $proteinC / CI | ~@SOS | ceaseless ; // [132:7]
```

App.SC:[24:5, 24:10, 26:1, 60:-7, 94:-7a, 94:-5, 95:2, 132:7]

## Genome: cI

```

105 @PRE_tr = RNAP_tr //[136:21][6:-9a]
106 & ^@OLR12_CII-- // [136:21]
107 |-- @OLR12?_CI_rng ! {lincdnt1(CI)<mdtr,sink>} // [55:-2][24:-8]
108 ;

```

App.SC:[6:-9a, 12:-8, 15:11, 18:-3, 24:-8, 24:F1.21:1, 37:15, 55:6, 55:-2, 68:-5a, 99:26, 136:21, 146:4]

```

110 @PRM_tr = RNAP_tr // [14:6][6:-9a]
111 & ^(@OLR12_CII-- : @OR2_CII-- // [19:6]
112 |-- @OR3_Cro // [44:9]
113 : @OR3_Cro +- ! // [44:9]
114 : @OR3_CII // [44:9]
115 : @OR3_CII +- ! // [44:9]
116 : @OLR123_CII -- ! {lincdnt1(CI)<mdtr,sink>} // [44:9][113:F5.5][24:-8]
117 ;

```

App.SC:[6:-9a, 12:-8, 14:6, 14:11, 14:F1.4:1, 15:11, 15:13, 15:-4, 15:-2, 18:5, 18:11, 18:-3, 18:F1.12:2, 19:2, 19:6, 19:-5, 19:-2, 20:3b, 20:10a, 20:-9, 24:-8, 24:F1.21:1, 25:2b, 26:1, 43:-5, 44:9, 44:-5, 45:4, 94:1, 94:2, 94:16, 99:-10, 102:-2, 103:7, 109:10, 111:2, 112:F5.4:1, 113:F5.5:1, 122:1, 123:3, 130:box:-17, 130:box:-7, 146:4]

```

119 +>@SOS< ! | $proteinC / cI | @PRE_tr // [60:-7][132:7][56:1]
120 : @PRM_tr ; // [15:13]

```

App.SC:[14:6, 14:F1.4:1, 15:13, 18:5, 18:11, 18:-3, 18:F1.12:2, 55:-2, 56:1, 60:-7, 68:-5a, 99:-10, 132:7]

## Genome: cro, w/simultaneous+independent binding

```

125 @OR1and2_Cro<@OR1_Cro,@OR2_Cro> = max&(@OR1_Cro,@OR2_Cro) ; //[93:F4.24:1]
126 @OR1xor2_Cro<> = min:(@OR1_Cro,@OR2_Cro) excl @OR1and2_Cro-- ;//[93:F4.24:1]
128 @OR1and2_CII<@OR1_CII,@OR2_CII> = max&(@OR1_CII,@OR2_CII) ; //([93:F4.24:1])
129 @OR1xor2_CII<> = min:(@OR1_CII,@OR2_CII) excl @OR1and2_CII-- ; //([93:F4.24:1])

```

App.SC:[93:F4.24:1, 94:15]

```

131 @PR_tr = RNAP_tr // [14:6][6:-9a]
132 /*& no recruiter*/ // [15:-4]
133 |-- @OR1xor2_Cro // [94:1][93:F4.24:1]
134 : @OR1xor2_Cro +- ! // [94:1][93:F4.24:1]
135 : @OR1and2_Cro -- ! // [94:1][93:F4.24:1]
136 : @OR1xor2_CII // [94:1]([93:F4.24:1])
137 : @OR1xor2_CII +- ! // [94:1]([93:F4.24:1])
138 : @OR1and2_CII -- ! // [94:1]([93:F4.24:1])
139 : @OLR12?_CI_rng ! {lincdnt1(CI)<mdtr,sink>} // [111:F5.3:1][24:-8]
140 ;

```

App.SC:[6:-9a, 12:-8, 14:6, 14:11, 14:F1.4:1, 15:11, 15:13, 15:-4, 18:5, 18:8, 18:-3, 18:F1.12:2, 19:6, 19:-5, 19:-2, 19:F1.13:1, 20:3b, 24:-8, 24:F1.21:1, 26:-1, 43:-5, 44:6, 44:-5, 44:-4, 45:13a, 93:F4.24:1, 94:1, 94:15, 109:10, 111:2, 111:4, 111:F5.3:1, 112:F5.4:1, 114:F5.7:1, 123:3, 146:4]

```

142 + ! | $proteinC / cro | @PR_tr ; // [15:13]

```

App.SC:[14:6, 14:F1.4:1, 15:13, 18:5, 18:8, 18:-3, 18:F1.12:2]

---

### Seeds

|     |                                              |
|-----|----------------------------------------------|
| 149 | "Cro.h"   expire(1,1) ; // [52:5/Late lytic] |
|-----|----------------------------------------------|

[[28]:52:5]/App.SE/Late lytic is classified as a ‘causation argument’, see Section S2.3.2.

---

|     |                                                        |
|-----|--------------------------------------------------------|
| 152 | "CI.0, Cro.0" entry(inject)   vanishOK<out>, // [12:7] |
| 153 | mix(CI,Cro)<out,src>, // [12:7]                        |
| 154 | incidental<out,mdtr,src> ; // [12:7]                   |

App.SC:[12:7]

---

## S2.2 A compiled Genetic Switch: $\lambda^{[AGS3]}$ physiology changes

We outline CEqEA’s interpretation of the  $\lambda^{[AGS3]}$  genotype in Section S2.1, aka (regulatory) form-to-function compilation, see Section S1.3.1. Concretely, the compiler sends [28]’s ‘molecular basis’ to the justified causations, meaning our (unifying) axiomatization of [28]’s ‘causation arguments’, see Appendix SE. It also effects [28]’s ‘population inferences’, see Appendix SD. The interpretation works like compilation for any other programming language, including the use of a multi-staged workflow to address each of the many requisite concerns at the most conducive intermediate level of representation. The start and end points of form-to-function compilation can reasonably be considered the extreme perspectives on regulatory units: one concerns their chemical backbone, the other the coded-for population effects in vacuo. The particular nature of CEqEA’s causations: the concept of a discretely-regulated physiology change, is due to us but the aim is to represent in a unified manner a range of interwoven notions that [28]’s ‘causation arguments’ address either in isolation or synthetically across changes.

The compiler can certify each step of change it makes. This information is indispensable for serious modeling but we do not discuss all details here. In particular, logical issues (including the fairly simple axiomatic structure) are addressed in Section S1.3.1 and we gloss over MIG modalities. Instead, we focus on operational matters (which have a less simple appearance) and ensuring transparency for  $\lambda^{[AGS3]}$ : the compiler starts from 67 lines of MIG syntax (without comments and empty lines; 159 with): `lambda[AGS3]_RI.mig`, and produces as output a graph with 28 nodes/vertices and 42 edges, namely the cascaded causation diagram we proceed over in Section S2.3. The associated certificate: `lambda[AGS3]_cert.txt`, is 2,593 lines.

A certificate includes a reconstituted MIG specification that directly reflects the edges in the final diagram(s). We call the particular form *physiological influences*. While expressed in the MIG language, these are simpler and more regulatorily disjointed than those that result from RI. For example, physical mutations are no longer localized in the MIG syntax and inhibition never appears nested. Physiological influences match the graph notation called Gene Regulation Networks (but are still bottom-up), see Discussion.

We focus on the essential part of CEqEA’s treatment of  $\lambda^{[AGS3]}$ , namely form-to-function compilation of MIG regulatory expressions. We do so “in the large”: *compound contravariance*, *elementarity*, *cleanup*, *physiological influences*, *regulatory function*, and the assembly of *cascaded causation diagrams*. Regulatory expressions may be freely composed from schema-instance states using indirection (^), disjunction (:), conjunction (&), and inhibition (|--), see Section S1.3. This includes arbitrary regulation of and with inhibition, including nested inhibition. Contravariance (!) may be used under any number of disjunctions and exactly one inhibition (in any order), as well as in one other place, see Sections S2.1.7–S2.1.8.

To avoid notation overload and to be explicit about regulatory roles, we

proceed by example over generic schema declarations before turning to  $\lambda^{\text{[AGS3]}}$ -specifics:

```
S . [ 0 1 ] ;

W . {""} ;
W1 . {""} ;
W2 . {""} ;
R . [ _ {""} ] ;
R1 . [ _ {""} ] ;
R2 . [ _ {""} ] ;

I . [ _ {""} ] ;
I1 . [ _ {""} ] ;
I2 . [ _ {""} ] ;
C . [ _ {""} ] ;
C1 . [ _ {""} ] ;
C2 . [ _ {""} ] ;

X . [ _ {*1} {*2} ] ;
```

The intention, see Section S2.1, is that the **S** is the *subject* (the thing that will change), the **Ws** are *workers* (e.g., `RNAP.tr`), the **Rs** are *recruiters*, the **Is** are (plain) *inhibitors*, the **Cs** are inhibitors with presumptive contravariant effects, and the **X** will be used for miscellany. The **Ws** are specified with one state (the empty string, written ""). CEqEA will assume singleton states to be present at all times. This will, e.g., render null-and-void any putative changes that are inhibited by a **W**. Instead, the **Rs** will indicate how their shared position is treated.

### S2.2.1 Contravariance

The word contravariance refers to occurrences of the ! MIG connective, to the formal effects that result from them, and to the real-world effects that these are modeling. Conceptually, contravariance is the opposite of some effect we have explicitly specified: the *covariant* effect. Concretely, contravariance is, e.g., net dilution of a protein population due to decay outpacing inhibited expression. This means that we need to determine the exact physiological conditions, e.g., for transcription, and when, concretely, product concentrations increase, and similar. We also need to determine, at least implicitly, when there is a neutral effect, not just due to absence of action but also and especially when positive and negative effects cancel out. Finally, we will then be in a position to determine when, e.g., dilution is the dominant effect. Under RI, we use a single regulatory expression to express what becomes the full range of effects that derive from a given influence polarity on a given schema instance. Coinhibition, see Section S2.1, may be used to prioritize different kinds of effects, e.g., expression+dilution vs proteolysis. *Compound contravariance* refers to how CEqEA does the net-effect determination.

**Active contravariance** The most basic principle is that this:

```
+ | S | (W & ^R |-- I : C!) ;
```

is unfolded to this — in which the & and : are associative and commutative, with a grouping of occurrences of either referred to as a *big conjunction* or a *big disjunction*:

```
1355 + | S.0 S.1 | ^R.&W. |-- C.:I. | ;
1364 - | S.0 S.1 | ^C. | ;
```

In words: a positive effect (+) on S with a contravariant inhibitor will happen exactly as specified, only without the ! connective. Additionally, the contravariant inhibitor will indirectly mediate an opposite effect, in this case a negative (-) one. This type of contravariance is referred to as *active*, e.g., as directed by the presence of C.

**Passive contravariance** We may also specify *passive* contravariance. This ! (next to the +):

```
+! | S | (W & ^R |-- I : C) ;
```

is unfolded to this:

```
1373 + | S.0 S.1 | ^R.&W. |-- C.:I. | ;
1382 - | S.0 S.1 | |-- ^R. | ;
```

Again, the covariant effect is as specified while, now, a contravariant effect is always at the ready but only goes ahead in the absence of the recruiter. (For “inhibition-of-null”, see Section S2.2.4.)

Implicit in this, we note that CEqEA omits passive contravariance for one-state workers (via ‘cleanup’) because the applicable inhibition is always in effect, meaning that this:

```
+! | S | (W |-- I : C) ;
```

is unfolded to just this:

```
1391 + | S.0 S.1 | W. |-- C.:I. | ;
```

**Compound contravariance** The word compound comes from the fact that a given effect on some subject may come from several distinct causes. For example, a gene may be transcribed from multiple promoters (as is the case for *cI*), with contravariance following when neither of these are active. CEqEA deals with this combinatorially, by mixing what would be the passive and active contravariations in each of the different causes. Concretely, this:

```
+! | S | (W1 & ^R1 |-- I1 : C1!) : (W2 & ^R2 |-- I2 : C2!) ;
```

is unfolded to this:

```
1400 + | S.0 S.1 | ^R1.&W1. |-- C1.:I1. | ;
1409 + | S.0 S.1 | ^R2.&W2. |-- C2.:I2. | ;
1418 - | S.0 S.1 | ^C1.&^C2. | ;
1427 - | S.0 S.1 | ^C1. |-- ^R2. | ;
1436 - | S.0 S.1 | ^C2. |-- ^R1. | ;
1445 - | S.0 S.1 | |-- ^R1.:^R2. | ;
```

The split of the covariant effects is described in Section S2.2.2. The first contravariant effect is active/active, the next two are active/passive, and the last is passive/passive. The +! pertains to all compound occurrences of passive contravariance: passive/passive, active/passive, as well as any more complex forms as determined by the contributing clauses. We are not seeing a contravariant effect regulated by ^C1. |-- ^R1. for two reasons: this would not rule out a covariant effect from the 2s and either of the two 1 regulators would be enough on its own.

### S2.2.2 Elementarity

We define an influence to be *elementary* if its regulatory expression consists of an inhibition at the top level, with a big conjunction of *mediating* schema-instance states on the left and a big disjunction of *inhibiting* schema-instance states on the right, where all states may be arbitrarily indirected. When there are no inhibitors, we will typically omit the inhibition constructor. The idea is that, in elementary form, the regulators operate discretely: (locally) positive is (globally) positive, negative is negative, and there is no further structure (except as prescribed by the subtler notion of modalities). A regulatory expression is first viewed and then converted as a propositional formula to disjunctive normal form, see Section S1.3.1. After, the arrived-at formulas are decoupled into multiple elementary influences:

|                                                                                     |
|-------------------------------------------------------------------------------------|
| $+ \quad   \quad S \quad   \quad (W1 : W2) \quad \& \quad \wedge (R1 : R2) \quad ;$ |
|-------------------------------------------------------------------------------------|

is unfolded to this:

|      |   |  |     |     |  |                   |  |   |
|------|---|--|-----|-----|--|-------------------|--|---|
| 1454 | + |  | S.0 | S.1 |  | $\wedge R1.\&W1.$ |  | ; |
| 1463 | + |  | S.0 | S.1 |  | $\wedge R2.\&W1.$ |  | ; |
| 1472 | + |  | S.0 | S.1 |  | $\wedge R1.\&W2.$ |  | ; |
| 1481 | + |  | S.0 | S.1 |  | $\wedge R2.\&W2.$ |  | ; |

and this:

|                                                                                                                        |
|------------------------------------------------------------------------------------------------------------------------|
| $+ \quad   \quad S \quad   \quad W \quad \& \quad \wedge R \quad   \quad \text{--} \quad I1 \quad \& \quad I2 \quad ;$ |
|------------------------------------------------------------------------------------------------------------------------|

is unfolded to this:

|      |   |  |     |     |  |                 |  |    |     |  |   |
|------|---|--|-----|-----|--|-----------------|--|----|-----|--|---|
| 1490 | + |  | S.0 | S.1 |  | $\wedge R.\&W.$ |  | -- | I1. |  | ; |
| 1499 | + |  | S.0 | S.1 |  | $\wedge R.\&W.$ |  | -- | I2. |  | ; |

The principles discussed here may look simple but the presence of an axiomatization is deceptive: the combined effect for realistic cases involving deeply-nested regulation may be convoluted (and should not be second-guessed or inferred in a top-down manner).

### S2.2.3 Cleanup

A large proportion of the elementary influences that are generated from real-life MIG/RI specifications will contain contradictory or impossible prescripts for the interaction of schema-instance states. For  $\lambda^{[AGS3]}$ , we start from 4 influences, see Section S2.1, and CEqEA then constructs 47 influences that meet the elementarity requirements, see `lambda[AGS3]_cert.txt`. After the cleanup we describe here, we are left with 15 that are deemed meaningful, i.e., that are physiological proper, see Section S2.2.4. A basic cleanup concern is that it is typically not possible for a schema instance to be in two different states at one time. This particular influence, for example:

```
+ | S | X.*1 & X.*2 ;
```

will be deemed null-and-void and will not be used in the final diagram while, e.g., this influence:

```
+ | S | X.*1 |-- X.*2 ;
```

will typically have the inhibitor suppressed because presence of the mediator is enough to guarantee that the inhibitor will be absent (but see Section S2.3.3:NB10). A complication is that these determinations can only be made once the full range of modalities for both the influences and any seeds have been resolved, see Section S2.2.5. One modality, for example, allows for **mixed Instantiation**, meaning that schema instances are allowed to be in more than one state at a time, say, for modeling membrane traversal, see Sections S2.1,S2.3. Other cleanup actions include abandoning presumptive changes that have an empty regulatory expression (e.g., due to ‘population inference’ — this happens prior to elementarity considerations to avoid removing fully-passive contravariations) or that are inhibited by schema-instance states that are guaranteed to be present (singleton states, the subject, mediators, etc.), consumption of mediators that are the subject (i.e., handling of auto-mediation irrespective of the **Regulation** modality), and suppression of the deeper of regulators that are present with a multitude of levels of indirection.

While essentially an orthogonal concern, CEqEA’s ‘population-inference’ engine that is tied to the `excl` keyword also performs a form of cleanup. For example, several of the macro declarations we made for  $\lambda^{[AGS3]}$  refer to no states:

```
75 //null-and-void macro declarations
76 // [OR1_CI,OR2_CI,OR3_CI,OR1xor2_Cro,OR1and2_CI,OR1xor2_CI]
```

For the details of ‘population inference’, see Section S1.1.6 on classical logic and Appendix SD.

### S2.2.4 $\lambda^{[AGS3]}$ physiological influences

We now discuss the concrete elementary influences that pass cleanup and are used in the  $\lambda^{[AGS3]}$  cascaded causation diagram, see `lambda[AGS3]_cert.txt`. The presented physiological influences are not self-contained: things like modalities still need to be enacted. We have included a re-parseable version of the physiological influences as `lambda[AGS3]_phys.mig`, where we have replaced empty mediation with auto-mediation (to work around particulars of CEqEA's MIG parser and cleanup action) and have re-added modalities by hand. The reconstituted version results in the same graph layout and the same (behavioral) synchronization diagrams but does not yet include enough information to allow CEqEA to present it and the  $\lambda^{[AGS3]}$  cascaded causation diagram as identical. In particular, active domains are not included, meaning noun-based reasoning, see Section S2.3, and coinhibition are not covered.

**RecA activation** No surprises here.

```
+ ! | $proteinC / RecA | @UV_irr ;
```

In the presence of short single-stranded DNA (ssDNA or `DNA.ss`) from UV irradiation (`UV_irr`), the host RecA protein will activate (`RecA*` or `RecA.*`). In the absence of ssDNA, the active complexes will gradually dissociate (`RecA.`).

```
244 1.1:
245 + | RecA. RecA.* | DNA.ss | ;
246     active domains:
247         [UV_irr]
274 1a1:
275 - | RecA. RecA.* | |-- DNA.ss | ;
```

**Host SOS response** No surprises here.

```
- | $proteinC / CI | ^@SOS | ceaseless ;
```

Activated RecA (`RecA.*`) will mediate auto-cleavage of CI as part of the host's SOS response. This process operates independently of CI expression and, although we do not show it here, the `ceaseless` modality value that expresses the ongoing nature of the process is inherited through the elementary influence down to the later functional forms, see **2.1:4** in Section S2.2.5.

```
302 2.1:
303 - | CI.0 CI.1 CI.m CI.h | ^RecA.* | ;
304     active domains:
305         [SOS]
```

**cI expression** The cI gene may be expressed from two different promoters.

```
+>@SOS< ! | $proteinC / cI | @PRE_tr : @PRM_tr ;
```

3.1 expresses that initiated transcription from P<sub>RE</sub> (PRE\_tr) may be halted at the downstream O<sub>R</sub>{1,2,3} sites owing to the complex binding mechanism of CI at all physiological concentrations we have specified. 3.2 expresses that transcription from P<sub>RM</sub> (PRM\_tr) requires RNAP recruitment (RNAP.tr) by CI at O<sub>R</sub>{1,2}. Crucially, the relevant CI binding happens at all physiological concentrations but the recruited RNAP only complexes with DNA when the O<sub>R</sub>3 operator site is not occupied, which it is at all but the lowest concentration of CI. Internally, CEqEA also considers recruitment at higher CI concentrations but these all fail to pass cleanup. Neither transcription will increase CI's concentration if the host SOS response is active.

```
335 3.1:
336 +>@SOS< | CI.0 CI.1 CI.m CI.h | ^CII.h&RNAP.tr |--
      CI.m:CI.h:CI.1 | ;
337     active domains:
338         [PRE_tr, ORE_CII]
339     coinhibition domains:
340         [SOS]
371 3.2:
372 +>@SOS< | CI.0 CI.1 CI.m CI.h | ^CI.1&RNAP.tr |--
      Cro.h:Cro.1:CI.m:CI.h:^CI.m:^CI.h | ;
373     active domains:
374         [OLR12_CI, PRM_tr]
375     coinhibition domains:
376         [SOS]
785 3a3:
786 - | CI.0 CI.1 CI.m CI.h | ^Cro.h&^CI.1 |-- ^CI.m:^CI.h
      | ;
787     active domains:
788         [OLR12_CI, OR3_Cro]
821 3b1:
822 - | CI.0 CI.1 CI.m CI.h | ^CI.m | ;
823     active domains:
824         [OLR123_CI]
913 3b4:
914 - | CI.0 CI.1 CI.m CI.h | ^CI.h | ;
915     active domains:
916         [OLR123_CI]
1235 3d2:
1236 - | CI.0 CI.1 CI.m CI.h | ^Cro.h |-- ^CII.h:^CI.m:^CI.h
      | ;
1237     active domains:
1238         [OR3_Cro]
1477 3f4:
1478 - | CI.0 CI.1 CI.m CI.h | | |-- ^CII.h:^CI.1 | ;
```

For contravariance, **3a3** (active/active) expresses that **CI**'s concentration will drop when  $O_R\{1,2\}$  are occupied by **CI** and  $O_R3$  is occupied by **Cro**, which it can be only when the operator is not preferentially occupied by **CI**. **3b1** and **3b4** (active/active) cover when **CI** occupy  $O_R\{1,2,3\}$ . **3d2** (passive/active) covers when there is no **PRE\_tr** recruitment and **Cro** prevents **RNAP**-DNA complexation at  $O_R3$ . Lastly, **3f4** (passive/passive) expresses that **cI** is not constitutively transcribed: **CI**'s concentration will drop in the absence of the listed recruiters. In all, 28 elementary influences following our MIG/RI specification of **cI** expression are abandoned through cleanup.

**cro expression** Expression of the **cro** gene is mostly straightforward.

|                                                                     |
|---------------------------------------------------------------------|
| <pre>+ !            \$proteinC / cro            @PR_tr      ;</pre> |
|---------------------------------------------------------------------|

Transcription of **cro** is constitutive, meaning **RNAP.tr** occurs without a recruiter, but cannot go ahead in case either or both of  $O_R\{1,2\}$  are occupied with sufficiently high regularity.

```

1508 4.1:
1509 + | Cro.0 Cro.1 Cro.h | RNAP.tr |--
      Cro.h:CI.m:CI.h:CI.l:^CI.m:^CI.h:^CI.l | ;
1510     active domains:
1511         [PR_tr]
1649 4a1:
1650 - | Cro.0 Cro.1 Cro.h | ^Cro.h |-- ^CI.m:^CI.h:^CI.l |
      ;
1651     active domains:
1652         [OR2_Cro, OR1_Cro]
1685 4b1:
1686 - | Cro.0 Cro.1 Cro.h | ^CI.m | ;
1687     active domains:
1688         [OLR123_CI]
1716 4b2:
1717 - | Cro.0 Cro.1 Cro.h | ^CI.h | ;
1718     active domains:
1719         [OLR123_CI]
1747 4b3:
1748 - | Cro.0 Cro.1 Cro.h | ^CI.l | ;
1749     active domains:
1750         [OLR12_CI]
```

4b1, 4b2, and 4b3 (active) express that any occupancy of  $O_R\{1,2\}$  by **CI** will have a contravariant effect. 4a1 (active) expresses that **Cro** at high concentration will have the same effect, with the proviso that **CI** will bind preferentially to the operators in question. No passive contravariance is included because there are no recruiters that can be absent.

### S2.2.5 $\lambda^{[AGS3]}$ regulatory function

After elementary influences, form-to-function compilation turns to the functional view. To effect the various modalities, multiple formats, or granularities, for the functionality are used successively: *causations*, *transitions*, and *changes*. In principle, there is also a fourth format: the visualized edges in the cascaded causation diagrams, see Section S1.4.1. These will correspond exactly to changes. Causations are the principled view. Transitions, the process view. Changes, the in-vacuo view up-to any PoI solution. Additionally, the use of causation information in the linearized coextension derivations in Section S2.3 are the in-situ view. We refer to them collectively as regulatory functionality. Here, we discuss transitions to ensure all formats are covered.

We define transitions to be binary relationships between 6-tuples of information:

$\dots, d(\dots), i(\dots), p(\dots), -(\dots), \sim(\dots)$

For example:

```
"DNA.ss,RecA., d(), i(), p(), -(), ~()"
====> "DNA.ss,RecA.*, d(), i(), p(), -(), ~()"
```

The  $\dots$ s above represent collections of schema-instance states. The first, free-standing group of schema-instance states are the explicit requirements, e.g., reactant/product and any mediators that are modality-stipulated to be needed, see Section S2.1.2. (Everywhere-present mediators are not listed: these are written infix in  $==>$ , e.g.,  $==RNAP.tr=>$ .) Schema-instance states within  $-(\sim)$  are direct/indirect inhibitors. Schema-instance states within  $i()$  are *implicit* requirements, which is a concept that is governed by modalities that we do not discuss here. Schema-instance states within  $d()$  are *dynamic* requirements, meaning either explicit or implicit. Neither implicit nor dynamic requirements are used here. Last, schema-instance states within  $p()$  are *possibles*: these states are not requirements but they are also not counted as solvent if they are present in some context where this transition is applied, see Section S1.4.1. Tuples enclosed in  $"_"$  are Points of Interaction (PoIs). When using the **pushpull Causation** modality value, both ends in a transition will become a PoI. PoIs have cascaded-causation-diagram nodes created for their explicit requirements: the free-standing group of  $\dots$ .

**RecA activation** No surprises here.

```
2393 1.1:
2394 + | RecA. RecA.* | DNA.ss | ;

2396 * [s1/e1:pure]: "RecA.,DNA.ss, d(), i(), p(), -( ), ~( )"
      ==> "DNA.ss,RecA.*, d(), i(), p(), -( ), ~( )"
2397     1.1:1
2398     <no suppression takes place>

2402 1a1:
2403 - | RecA. RecA.* | |-- DNA.ss | ;

2405 * [s1/e1:pure]: "RecA.*, d(), i(), p(), -(DNA.ss), ~( )"
      ==> "RecA., d(), i(), p(), -(DNA.ss), ~( )"
2406     1a1:1
2407     <no suppression takes place>
```

**Host SOS response** 2.1:4 represents the ceaseless proteolytic effect of RecA.\* on CI.

|      |                                       |
|------|---------------------------------------|
| 2411 | 2.1:                                  |
| 2412 | -   CI.0 CI.1 CI.m CI.h   ^RecA.*   ; |

  

```

2414 * [s1/e1:pure]: "CI.h,RecA.*, d(), i(), p(), -(), ~()"
      ==> "CI.m,RecA.*, d(), i(), p(), -(), ~()"
2415      2.1:1
2416      <no suppression takes place>

2418 * [s1/e1:pure]: "CI.m,RecA.*, d(), i(), p(), -(), ~()"
      ==> "RecA.*,CI.1, d(), i(), p(), -(), ~()"
2419      2.1:2
2420      <no suppression takes place>

2422 * [s1/e1:pure]: "RecA.*,CI.1, d(), i(), p(), -(), ~()"
      ==> "CI.0,RecA.*, d(), i(), p(), -(), ~()"
2423      2.1:3
2424      <no suppression takes place>

2426 * [s1/e1:pure]: "CI.0,RecA.*, d(), i(), p(), -(), ~()"
      ==> "CI.0,RecA.*, d(), i(), p(), -(), ~()"
2427      2.1:4
2428      <no suppression takes place>

```

## cI expression

**3.1:1** This and other changes are present in two distinct versions, named **seed** and **pure**:

- **pure** is the default manifestation of the original influence while
- **seed** is an adapted form deriving from the fact that the considered regulatory functionality may connect in a non-standard way to the **inject entry** channel,
- where the **inject seed** modalities imply that **CII.h** need not be injected in order to effect  $P_{RE}$ -transcription: it is classified as a possible mediator on the left, and
- suppression of superfluous inhibitors may be different between the transition-related blocks of information, while
- no steps beyond this one are well-formed due to inhibition: there are no 3.1:2, etc.

**3.2:1** The folding of deeper into lesser levels of indirection, and more, is performed at the point of graph-edge insertion, see Section S1.4.1, to allow for seed-modality overrides.

**3.2:2** Auto-mediators are allowed to disappear across the change they effect.

```

2432 3.1:
2433 +>@SOS< | CI.0 CI.1 CI.m CI.h | ^CII.h&RNAP.tr |--
        CI.m:CI.h:CI.1 | ;

```

```

2435 * [s1/e1:seed]: "CI.0, d(), i(), p(CII.h),
                   -(CI.m,CI.h,CI.1), ~()" ==RNAP.tr=> "CII.h,CI.1, d(),
                   i(), p(), -(), ~()"
2436     3.1:1
2437     suppressed:
2438         @sink,direct,inhbt: CI.m,CI.h,CI.1

2440 * [s1/e1:pure]: "CII.h,CI.0, d(), i(), p(), -(), ~()"
                   ==RNAP.tr=> "CII.h,CI.1, d(), i(), p(), -(), ~()"
2441     3.1:1
2442     suppressed:
2443         @srce,direct,inhbt: CI.m,CI.h,CI.1
2444         @sink,direct,inhbt: CI.m,CI.h,CI.1

```

```

2448 3.2:
2449 +>@SOS< | CI.0 CI.1 CI.m CI.h | ^CI.1&RNAP.tr |--
        Cro.h:Cro.1:CI.m:CI.h:^CI.m:^CI.h | ;

```

```

2451 * [s1/e1:seed]: "CI.0, d(), i(), p(CI.1),
                    -(Cro.h,Cro.l,CI.m,CI.h), ~(CI.m,CI.h)" ==RNAP.tr=>
                    "CI.1, d(), i(), p(), -(Cro.h,Cro.l), ~()"
2452                    3.2:1
2453                    suppressed:
2454                        @sink,direct,inhbt: CI.m,CI.h
2455                        @sink,indrct,inhbt: CI.m,CI.h

2457 * [s1/e1:pure]: "CI.1, d(), i(), p(), -(Cro.h,Cro.l), ~()"
                    ==RNAP.tr=> "CI.m, d(), i(), p(), -(Cro.h,Cro.l), ~()"
2458                    3.2:2
2459                    suppressed:
2460                        @srce,direct,inhbt: CI.m,CI.h
2461                        @srce,indrct,inhbt: CI.m,CI.h
2462                        @sink,direct,inhbt: CI.m,CI.h
2463                        @sink,indrct,inhbt: CI.m,CI.h

2467 3a3:
2468 - | CI.0 CI.1 CI.m CI.h | ^Cro.h&^CI.1 |-- ^CI.m:^CI.h
    | ;

2470 * [s1/e1:pure]: "Cro.h,CI.1, d(), i(), p(), -(), ~()" ==>
                    "Cro.h,CI.0, d(), i(), p(), -(), ~()"
2471                    3a3:3
2472                    suppressed:
2473                        @srce,indrct,inhbt: CI.m,CI.h
2474                        @sink,indrct,inhbt: CI.m,CI.h

2478 3b1:
2479 - | CI.0 CI.1 CI.m CI.h | ^CI.m | ;

2481 * [s1/e1:pure]: "CI.m, d(), i(), p(), -(), ~()" ==>
                    "CI.1, d(), i(), p(), -(), ~()"
2482                    3b1:2
2483                    <no suppression takes place>

2487 3b4:
2488 - | CI.0 CI.1 CI.m CI.h | ^CI.h | ;

2490 * [s1/e1:pure]: "CI.h, d(), i(), p(), -(), ~()" ==>
                    "CI.m, d(), i(), p(), -(), ~()"
2491                    3b4:1
2492                    <no suppression takes place>

2496 3d2:
2497 - | CI.0 CI.1 CI.m CI.h | ^Cro.h |-- ^CII.h:^CI.m:^CI.h
    | ;

```

```

2499 * [s1/e1:pure]: "Cro.h,CI.l, d(), i(), p(), -(), ~(CII.h)"
      ==> "Cro.h,CI.0, d(), i(), p(), -(), ~(CII.h)"
2500      3d2:3
2501      suppressed:
2502          @srce,indrct,inhbt: CI.m,CI.h
2503          @sink,indrct,inhbt: CI.m,CI.h

```

|      |                                                |
|------|------------------------------------------------|
| 2507 | 3f4:                                           |
| 2508 | -   CI.0 CI.l CI.m CI.h    -- ^CII.h:^CI.l   ; |

```

2510 * [s1/e1:pure]: "CI.h, d(), i(), p(), -(), ~(CII.h)" ==>
      "CI.m, d(), i(), p(), -(), ~(CII.h)"
2511      3f4:1
2512      suppressed:
2513          @srce,indrct,inhbt: CI.l
2514          @sink,indrct,inhbt: CI.l

2516 * [s1/e1:pure]: "CI.m, d(), i(), p(), -(), ~(CII.h)" ==>
      "CI.l, d(), i(), p(), -(), ~(CII.h)"
2517      3f4:2
2518      suppressed:
2519          @srce,indrct,inhbt: CI.l
2520          @sink,indrct,inhbt: CI.l

```

cro expression 4b1:1, 4b1:2, 4b2:1, 4b2:2, 4b3:1, and 4b3:2 have CI as a possible mediator in the target end in order to capture that causation by CI involves highly-cooperative binding, which means that the considered regulatory functionality need not reflect the concentration of free CI for their duration.

```

2524 4.1:
2525 + | Cro.0 Cro.1 Cro.h | RNAP.tr |--
      Cro.h:CI.m:CI.h:CI.l:~CI.m:~CI.h:~CI.l | ;

2527 * [s1/e1:seed]: "Cro.0, d(), i(), p(),
                    -(Cro.h,CI.m,CI.h,CI.l), ~(CI.m,CI.h,CI.l)" ==RNAP.tr=>
                    "Cro.1, d(), i(), p(), -(CI.m,CI.h,CI.l),
                    ~(CI.m,CI.h,CI.l)"
2528     4.1:1
2529     suppressed:
2530         @sink,direct,inhbt: Cro.h

2532 * [s1/e1:pure]: "Cro.0, d(), i(), p(), -(CI.m,CI.h,CI.l),
                    ~(CI.m,CI.h,CI.l)" ==RNAP.tr=> "Cro.1, d(), i(), p(),
                    -(CI.m,CI.h,CI.l), ~(CI.m,CI.h,CI.l)"
2533     4.1:1
2534     suppressed:
2535         @srce,direct,inhbt: Cro.h
2536         @sink,direct,inhbt: Cro.h

2538 * [s1/e1:pure]: "Cro.1, d(), i(), p(), -(CI.m,CI.h,CI.l),
                    ~(CI.m,CI.h,CI.l)" ==RNAP.tr=> "Cro.h, d(), i(), p(),
                    -(CI.m,CI.h,CI.l), ~(CI.m,CI.h,CI.l)"
2539     4.1:2
2540     suppressed:
2541         @srce,direct,inhbt: Cro.h
2542         @sink,direct,inhbt: Cro.h

2546 4a1:
2547 - | Cro.0 Cro.1 Cro.h | ^Cro.h |-- ^CI.m:~CI.h:~CI.l |
      ;

2549 * [s1/e1:pure]: "Cro.h, d(), i(), p(), -(),
                    ~(CI.m,CI.h,CI.l)" ==> "Cro.1, d(), i(), p(), -(),
                    ~(CI.m,CI.h,CI.l)"
2550     4a1:1
2551     <no suppression takes place>

2555 4b1:
2556 - | Cro.0 Cro.1 Cro.h | ^CI.m | ;

2558 * [s1/e1:pure]: "Cro.h,CI.m, d(), i(), p(), -(), ~()" ==>
                    "Cro.1, d(), i(), p(CI.m), -(), ~()"

```

```

2559         4b1:1
2560         <no suppression takes place>

2562 * [s1/e1:pure]: "Cro.l,CI.m, d(), i(), p(), -(), ~()" ==>
        "Cro.0, d(), i(), p(CI.m), -(), ~()"
2563         4b1:2
2564         <no suppression takes place>

2568 4b2:
2569 - | Cro.0 Cro.l Cro.h | ^CI.h | ;

2571 * [s1/e1:pure]: "Cro.h,CI.h, d(), i(), p(), -(), ~()" ==>
        "Cro.l, d(), i(), p(CI.h), -(), ~()"
2572         4b2:1
2573         <no suppression takes place>

2575 * [s1/e1:pure]: "Cro.l,CI.h, d(), i(), p(), -(), ~()" ==>
        "Cro.0, d(), i(), p(CI.h), -(), ~()"
2576         4b2:2
2577         <no suppression takes place>

2581 4b3:
2582 - | Cro.0 Cro.l Cro.h | ^CI.l | ;

2584 * [s1/e1:pure]: "Cro.h,CI.l, d(), i(), p(), -(), ~()" ==>
        "Cro.l, d(), i(), p(CI.l), -(), ~()"
2585         4b3:1
2586         <no suppression takes place>

2588 * [s1/e1:pure]: "Cro.l,CI.l, d(), i(), p(), -(), ~()" ==>
        "Cro.0, d(), i(), p(CI.l), -(), ~()"
2589         4b3:2
2590         <no suppression takes place>

```

### S2.3 An emergent Genetic Switch: the $\lambda^{[AGS3]}$ phenotype

We present a verified development of the monograph organism’s behavioral properties: the  $\lambda^{[AGS3]}$  phenotype. As discussed in the article, formally-developed properties naturally reflect the structure of the considered reasoning space. The units of information we work to: ‘pathway properties’, are not in [28] in an explicit sense but see Figure 4. ‘Pathway properties’ bridge a may-/will-happen gap between [28]’s ‘pathway arguments’ (coming from the “inside”, i.e., involving molecules and chemistry) and [28]’s ‘cell behaviors’ (coming from the “outside”, i.e., involving biology and observations):

- [28]’s ‘causation arguments’ correspond to synthesized aspects of our regulatory functionality: causations, i.e., the graph edges of Section S1.4.1, see Section S2.2.5 and Appendix SE;
- [28]’s ‘pathway arguments’, in effect, are human-centred highlights of our coextension derivations seemingly intended to illustrate key interferences, see Figure 4 and Appendix SF;
- our ‘pathway properties’ are invariants over the presented coextension derivations, stated in natural language, for molecular-biology consumption: they cover the nature of the visited compartments and any decisive regulatory structure or events along the way;
- [28]’s ‘cell behaviors’ account for biological observations and, in effect, are executive summaries of collections of our ‘pathway properties’, see Appendix SG.

See [[28]:52:5]/App.SE vs [[28]:50:6]/App.SF for ‘causation argument’ vs ‘pathway argument’.

Our reasoning proceed in two ways:

- by means of specific coextension derivations generated with CEqEA’s proof engine, see Section S1.4: this is for properties about concrete behaviors, typically under perturbation in order to account for environmental effects or stochastic fluctuations. These arguments are listed with full details in the linearized form discussed in Figure 4 and each step is visualized over the cascaded causation diagram of Section S1.4.1, see Section S1.4.3 and video. We give instructions for their replication by means of graph interactions, for ease of use.
- by considering a coextension state space over some fixed set of circumstances, see Section S1.6.2: this is for properties that quantify over behaviors:  $2/a/\alpha/$ ,  $2/b/i/$ ,  $3/b/i/$ ,  $3/d/$ . These either establish a baseline or complement principal properties. This type of argumentation summarizes all reasoning that may take place within a non-perturbable set of scenarios: coextension state spaces are graphs that are constructed by exhaustive use of CEqEA’s proof engine over the relevant aspects of the given cascaded

causation diagram, see Section S1.6. This implies that supporting coextension derivations exist but they are not listed and the reasoning ignore their details (intensionality) to focus on outcomes (extensionality).

For documentation, each specific linearized coextension derivation is included below an attendant discussion. The discussions are for human consumption and may have their style changed to suit different audiences. Our style is compact, as seen in mathematics, to showcase the level of detail and focus we enable and to complement [28]. Our discussions refer into the linearized derivations in the form  $\langle \text{Prop/Case/l.n,ll.n}_1\text{--n}_2 \text{ --- possible disambiguation} \rangle$ . As noted, each reasoning step is also visualized over the given cascaded causation diagram, which is referred to in the form  $\lceil \text{Prop/Case/ll.n}_1\text{--n}_2 \rceil$ . Section S2.3.3 discusses a range of structural issues that are annotated onto the visualizations (in off-palette black) and that have decisive and/or subtle bearing on the properties, referred to in the form  $\lceil \text{NBn @ Prop/Case/ll.n}_1\text{--n}_2 \rceil$ .

We recommend having watched the article video before continuing.

### S2.3.1 The $\lambda^{[AGS3]}$ phenotype

Rather than following [28], we establish the  $\lambda^{[AGS3]}$  phenotype paradigmatically, specifically to reflect the reasoning-space structure. The most obvious differences between the two accounts are the properties in *italics*, which are not/indirectly considered in [28]: 0/ is the pivot while the others are for in-vitro scenarios without host expiration. See the article.

**Host is healthy or not:**  $\heartsuit$  stands for “absent a host SOS response (with **RecA**.)” and  $\neg\heartsuit$  stands for its negation “during a host SOS response (with **RecA**.)”;

**Host is doomed or not:**  $\spadesuit$  stands for “with **CII** below high concentration (**CII**.)” and **CI** below physiological concentration (**CI**.)” and  $\neg\spadesuit$  stands for its negation “with **CII** at high concentration (**CII**.) or with **CI** at physiological concentration (**CI**.)”.

In the  $\lambda^{[AGS3]}$  phenotype, inner properties are part of outer properties:

- 0/ *lysogeny's means take precedence over a lytic attack*  $\heartsuit$
- 1/ **CII** determines  $\lambda$ 's pathway at fresh infection  $\heartsuit$ : lysogeny at high vs lytic attack below
  - 2/ the lysogenic cycle is homeostatic, i.e., is sustainable and absorbs perturbations
    - a/ protein concentrations are **CI** controlled in the lysogenic cycle
      - $\alpha$ / an initial **CI** concentration is and must be established by high **CII**  $\heartsuit$
      - $\beta$ / once established, **CI** remains physiological and **Cro** non-physiological  $\heartsuit$
    - b/ a switch to the lytic attack is not effected by
      - i/ natural or operative means  $\heartsuit$  — this is the basis of sustainability
      - ii/ **Cro**-perturbation  $\heartsuit$  — this is the key means of homeostasis
      - iii/ super-infection  $\heartsuit$  — this is  $\lambda$ -immunity
    - c/ a switch to the lytic attack is effected by UV-irradiation (via  $\neg\heartsuit$ )
  - 3/ the lytic attack expires the host and, else, is sustainable but *not homeostatic*
    - a/ protein concentrations are programmatic during a lytic attack
      - $\alpha$ / the lytic attack is constitutive  $\neg\heartsuit$  or  $\spadesuit$
      - $\beta$ / once initiated, **Cro** remains physiological and **CI** inoperative  $\neg\heartsuit$  or  $\spadesuit$
      - $\gamma$ / a lytic attack expires the host after **Cro** has reached high  $\neg\heartsuit$  or  $\spadesuit$
    - b/ *ignoring host expiration, a switch to the lysogenic cycle is not effected by*
      - i/ *natural or operative means*  $\neg\heartsuit$  or  $\spadesuit$  — this is the basis of sustainability
      - ii/ **CI**-perturbation  $\neg\heartsuit$ , although the lytic attack may be set back
      - iii/ *super-infection*  $\neg\heartsuit$  or  $\spadesuit$  — an aspect of anti-immunity, see article:Retro.(V)
    - c/ *ignoring host expiration, a switch to lysogeny is likely to be effected by*
      - ii/ **CI**-perturbation  $\heartsuit$  (and  $\spadesuit$  in order for the lytic attack to be viable, see 3/d/)

d/ a lytic attack is unlikely  $\heartsuit$  and  $\neg\spadesuit$

Dormant  $\lambda$ -lysogeny is associated with healthy hosts that are not doomed: ' $\heartsuit$  and  $\neg\spadesuit$ '. The lytic attack is associated with hosts that are not healthy or are doomed: ' $\neg\heartsuit$  or  $\spadesuit$ '. An unhealthy lysogenic host triggers its own doom, see 2/c/, meaning the two conditions are not independent. This makes the apparent symmetry between the two modes of growth seem more natural than it is, see 2/b/iii/ vs 3/b/iii/, 3/b/ii/ vs 3/c/ii/, and article:Retrodictions. Note the decomposition of  $\neg\spadesuit$  in 2/'s premises and that 3/d/ complements 3/{a,b,c}/.

Unless contradicted by the details at hand, we consider two scenarios for each property: with "CII. \_" and with "CII.h". We treat the cases with CII below or at high concentration separately because [28] does not account for the details of how CII state changes take place. Within CEqEA, this type of scenario is what triggers the inclusion of toggles in the generated cascaded causation diagram, see Section S1.4.1. In addition to using distinguishing labels, the documentation for the case of CII. \_, i.e., for CII below high concentration, uses a narrower frame border than the documentation for the case of CII.h, i.e., for CII at high concentration.

By default, the compartments we use include RNAP.tr, whose singleton transcribing state is assumed present everywhere and is not mentioned, and DNA.ds, meaning the physiological absence of the short single-stranded DNA whose presence is indicative of DNA damage.

The earlier properties we present introduce terminology and connect it to particulars in the visualization snapshots and linearized coextension derivations.

### S2.3.2 $\lambda^{\text{[AGS3]}}$ coextension reasoning

0/ lysogeny's means take precedence over a lytic attack  $\heartsuit$

App.SC:[(9:-8, 12:10a, 92, Figure 4.23:1)]

WE ADDRESS THIS BY ENABLING THE “CI.L” AND “Cro.L” NODES, THE CII TOGGLES, AND THE “RECA.” NODE, SEE  $\heartsuit$  (PLUS THE DEFAULT COMPARTMENT).

This is a low-level property that underpins other properties: 1/, 2/a/ $\alpha$ /, 2/b/ii/, 3/c/ii/, and 3/d/. The property is straightforward in isolation but its effects may be surprising in context: it does not constitute a stand-alone observation but it does play a pivotal role for the referenced properties, all of which have observable aspects.

The lysogenic cycle is characterized by the presence of CI and the lytic attack is characterized by the presence of Cro, see [[28]:136:15]/App.SG — see {2,3}/a/ $\beta$ / for the (differing) details. When enabling the “CI.1” node (the weakest of lysogeny's means, see 2/) and the “Cro.1” node (the early stage of a lytic attack, see 3/), CEqEA automatically enables also the “CI.1, Cro.1” node, by coextension. This means we are considering the interference among causations that derive from these protein concentrations acting in isolation or in combination, under the default compartment.

- The concentration-increasing edges from the “CI.1” and “Cro.1” nodes are blocked (dotted)  $\lceil 0/\text{CII}.\{-,h\}/1.1-3 \rceil$ . From the linearized coextension derivations  $\langle 0/\text{CII}.\{-,h\}/1.3 \rangle$ , we see that this means that neither *cro* nor *cI* is physiologically transcribed because of inhibition by CI bound to  $O_{\{L,R\}}\{1,2\}$  and Cro bound to  $O_R3$   $\langle 0/\text{CII}.\{-,h\}/1.3 \rangle$ .
- From the “CI.1, Cro.1” node and its active out-edge, we see that the CI binding to  $O_{\{L,R\}}\{1,2\}$  is strong  $\langle 0/\text{CII}.\{-,h\}/1.3 \rightarrow \text{CI.1!} \rangle$ , meaning Cro is subject to a contravariant effect  $\langle 0/\text{CII}.\{-,h\}/1.2 \rangle$ : dilution becomes the dominant factor for Cro, and Cro turns non-physiological  $\langle 0/\text{CII}.\{-,h\}/1.5 \rangle$ . Conversely, CI is not subject to a contravariant effect  $\langle 0/\text{CII}.\{-,h\}/1.2 \rangle$ , meaning CI is being sufficiently replenished to match its dilution rate  $\langle 0/\text{CII}.\{-,h\}/1.5 \rangle$ .

The outcome is CI.1, Cro.0  $\langle 0/\text{CII}.\{-,h\}/1.5 \rangle$ , with the “CI.1” and “Cro.0” nodes enabled (along with toggles and the default compartment)  $\lceil 0/\text{CII}.\{-,h\}/1.5-7 \rceil$ . This outcome is a direct consequence of the different binding mechanisms for the two proteins: compared to Cro, CI's binding occupies the relevant operators for a larger fraction of time and may remain in effect longer than warranted by the concentration of free protein.

⟨Linearized coextension derivation: 0/CII.⟨\_⟩⟩

```

1 [CI.1, Cro.1] + [CII.⟨_⟩, DNA.ds, RecA.]
2 -> ![OLR12_CI]
3 x> [PR_tr] |-- [CI.1!@[OLR12]] ; [OLR12_CI, PRM_tr] |--
   [Cro.1@[OR3]]

5 [CI.1, Cro.0] + [CII.⟨_⟩, DNA.ds, RecA.]
6 -> [OLR12_CI, PRM_tr]
7 x> [PR_tr] |-- [CI.1!@[OLR12]]

```

⌈Visualization: 0/CII.⟨\_⟩⌋

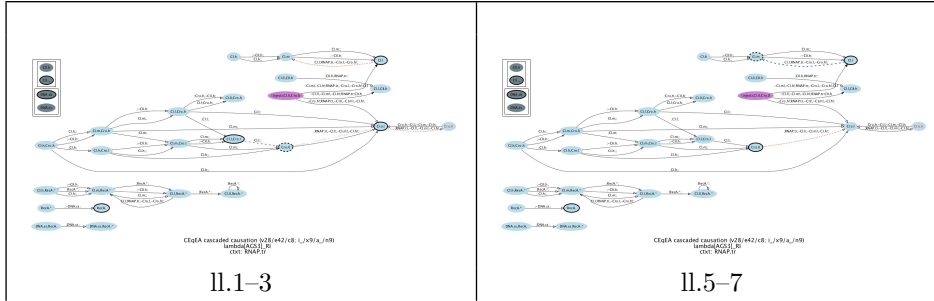

⟨Linearized coextension derivation: 0/CII.h⟩

```

1 [CI.1, Cro.1] + [CII.h, DNA.ds, RecA.]
2 -> ![OLR12_CI]
3 x> [PR_tr] |-- [CI.1!@[OLR12]] ; [OLR12_CI, PRM_tr] |--
   [Cro.1@[OR3]]

5 [CI.1, Cro.0] + [CII.h, DNA.ds, RecA.]
6 -> [OLR12_CI, PRM_tr]
7 x> [PR_tr] |-- [CI.1!@[OLR12]]

```

⌈Visualization: 0/CII.h⌋

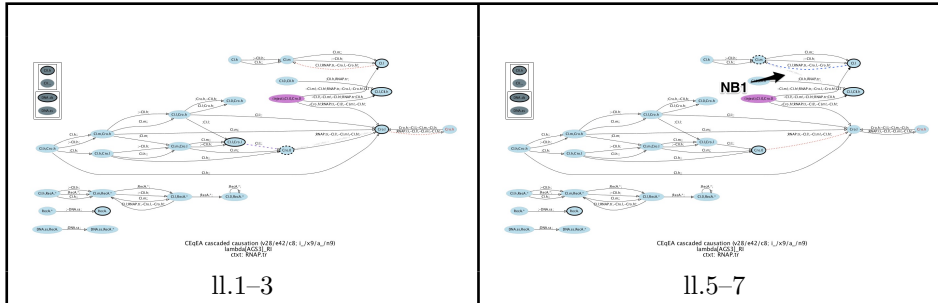

1/ CII determines  $\lambda$ 's pathway at fresh infection ♡: lysogeny at high vs lytic attack below

---

App.SC:[1:7, 9:-8, 11:8, 11:9, 11:14, 13:Fig.1.2:1, 48:1, 50:6, 52:5, 56:-3, 56:-1b, 57:22, 64:1, 64:8, 68:-7]

WE ADDRESS THIS BY ENABLING THE (INJECT) CHANNEL, THE CII TOGGLES, AND THE “RECA.” NODE, SEE ♡ (PLUS THE DEFAULT COMPARTMENT).

- In case CII is below high concentration, i.e., in case “CII.-” is toggled, a fresh  $\lambda$ -infection leads directly to a lytic attack:  $P_R$  is constitutively activated immediately upon infection  $\langle 1/CII.-/l.2 \rangle$ , with ‘constitutive’ corresponding to  $PR_{tr}$  occurring by itself within  $[\ ]_s$ , i.e., without RNAP recruiters, and it remains activated until the host expires/lyses  $\langle 1/CII.-/l.17 \rangle$ , with a single (physiologically important) exception  $\langle 1/CII.-/l.9-11 \rangle$ . See  $3/a/\{\alpha,\beta\}/$  for details of how the lytic attack unfolds  $\langle 1/CII.-/l.1-15 \rangle$  and  $3/a/\gamma/$  for details of the host destruction  $\langle 1/CII.-/l.9,l.17 \rangle$ . Absent the requisite recruiters,  $P_{RE}$  and  $P_{RM}$  are not (physiologically) activated at any point  $\langle 1/CII.-/l.1-17 \rangle$ , and  $cI/CI$  plays no (physiological) role in a fresh infection with CII below high concentration: the injected  $cI$  remains *inert* in state  $CI.0$ , i.e., is not subject to causation,<sup>8</sup> see  $\langle 1/CII.-/l.1,l.5,l.9,l.13 - + [CI.0\dots] \rangle$ .
- In case CII is at high concentration, i.e., in case “CII.h” is toggled, a fresh  $\lambda$ -infection invariably establishes the lysogenic cycle: initially, either pathway appears possible following immediate CII-mediated  $P_{RE}$ -activation and constitutive  $P_R$ -activation  $\langle 1/CII.h/l.2 \rangle$ . However, this sees both  $CI$  and  $Cro$  become physiological  $\langle 1/CII.h/l.5 \rangle$  and 0/ tells us that (pure) lysogeny will result.

---

<sup>8</sup>More precisely: a schema instance is inert if, given a compartment that includes a state for the instance, the instance state is not part of an enabled node with an out-edge (modulo TargetRequired but irrespective of active/blocked) that leads to a node with either no state or a different state for the schema instance, i.e., if it is not a subject in a causation whose positive conditions are met, i.e., if it is not meaningfully regulated upon.

⟨Linearized coextension derivation: 1/CII.⟦\_⟩

```

1  [Cro.0] + [(inject), CI.0, CII.⟦_, DNA.ds, RecA.]
2  -> [PR_tr]
3  x>

5  [Cro.1] + [CI.0, CII.⟦_, DNA.ds, RecA.]
6  -> [PR_tr]
7  x>

9  [Cro.h] + [CI.0, CII.⟦_, DNA.ds, RecA.]
10 -> ![OR2_Cro, OR1_Cro]
11 x>

13 [Cro.1] + [CI.0, CII.⟦_, DNA.ds, RecA.]
14 -> [PR_tr]
15 x>

17 <expired>

```

⌈Visualization: 1/CII.⟦\_⌋

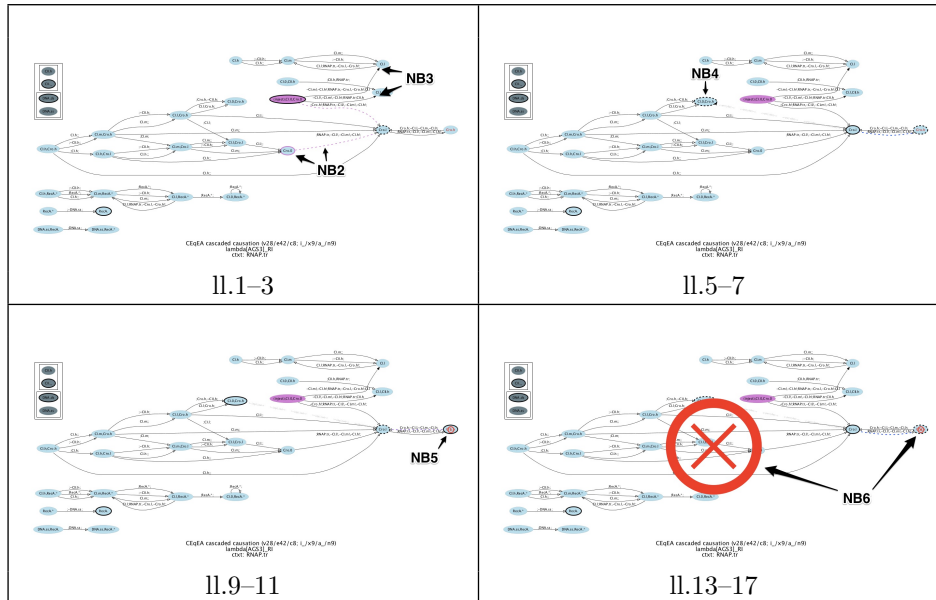

⟨Linearized coextension derivation: 1/CII.h⟩

```

1 [CI.0, Cro.0] + [(inject), CII.h, DNA.ds, RecA.]
2 -> [PR_tr] ; [PRE_tr, ORE_CII]
3 x>

5 [CI.1, Cro.1] + [CII.h, DNA.ds, RecA.]
6 -> ![OLR12_CI]
7 x> [PR_tr] |-- [CI.1!@[OLR12]] ; [OLR12_CI, PRM_tr] |--
    [Cro.1@[OR3]]

9 [CI.1, Cro.0] + [CII.h, DNA.ds, RecA.]
10 -> [OLR12_CI, PRM_tr]
11 x> [PR_tr] |-- [CI.1!@[OLR12]]

13 [CI.m, Cro.0] + [CII.h, DNA.ds, RecA.]
14 -> ![OLR123_CI]
15 x> ![ ] |-- [CII.h] ; [PR_tr] |-- [CI.m!@[OLR123]]

```

⌈Visualization: 1/CII.h⌋

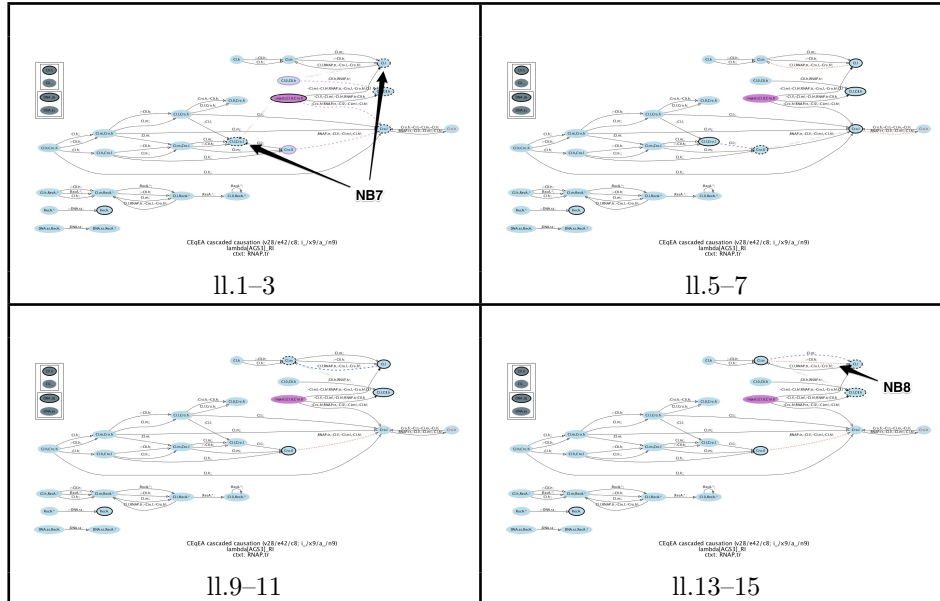

2/ the lysogenic cycle is homeostatic, i.e., is sustainable and absorbs perturbations

App.SC:[11:14, 23:6, 47:11, 64:17, 133:15, (1:3, 1:7)]

a/ protein concentrations are CI controlled in the lysogenic cycle

App.SC:[15:8, 15:Fig.1.5:2]

$\alpha$ / an initial CI concentration is and must be established by high CII  $\heartsuit$

App.SC:[50:6, 52:5, 56:-3]

WE ADDRESS THIS PARTLY BY CONSIDERING A COEXTENSION STATE SPACE OVER **CI**, **CII**., **Cro**, **DNA.ds**, AND NOT OVER **RECA.\***, SEE  $\heartsuit$ .

For the ‘is’ part of the property, see the **CII.h** case of 1/.

The ‘must’ part of the property includes a universal quantification: among all pathways, none exhibit a specific feature in case **CII** is below high concentration. Properties of this nature are difficult to address by considering specific derivations: we would need to guarantee consideration of all possibilities, which include more than those suggested by the CEqEA proof engine, e.g., the partial changes. Instead, we use a coextension state space that shows all that may happen in a situation-based rather than a causation-based manner, see Section S1.6.2: bolded edges indicate our approximation of what will happen, which may involve a non-deterministic choice between multiple edges. With a state space, we will not have access to the molecular details that otherwise make up our reasoning. As is common for quantified properties, those details are not needed here.

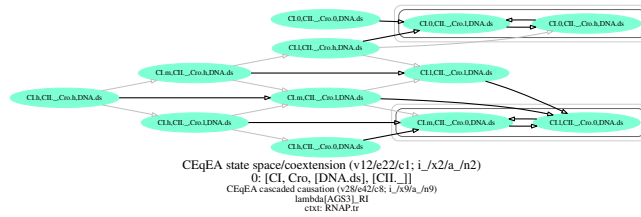

We can note in the above coextension state space that the “**CI.0,CII. ,Cro.0,DNA.ds**” node only has a path that takes it to nodes that have **CI** at zero concentration and **Cro** at physiological concentration. As the considered injections are precisely characterized by the “**CI.0,CII. ,Cro.0,DNA.ds**”

situation, **CI** cannot reach physiological concentration (without other help) in case **CII** is below high concentration.

$\beta/$  once established, CI remains physiological and Cro non-physiological  $\heartsuit$

App.SC:[11:14, 12:1, 12:2, 12:-5, 15:8, 15:-10, 20:4, 22:1, 22:2, 22:4, 23:1, 23:4, 23:6, 23:Fig.1.19:1, 28:10, 47:6, 47:-4, 50:6, 52:5, 68:-8, 68:-7, 87:1, 87:-13, 87:-9, 103:6, 111:Fig.5.3:1, 112:17, 136:15]

WE ADDRESS THIS BY ENABLING THE “CI.L” AND “Cro.O” NODES, THE CII TOGGLES, AND THE “RECA.” NODE, SEE  $\heartsuit$  (PLUS THE DEFAULT COMPARTMENT).

The lysogenic cycle is independent of CII’s concentration, i.e., the following holds for the lysogenic cycle both with CII below and at high concentration.

- CI alternates between low and medium concentration  $\langle 2/a/\beta/CII.\{-,h\}/1.1,1.5,1.9 \rangle$ , with  $\langle 2/a/\beta/CII.\{-,h\}/11.1-3 \rangle = \langle 2/a/\beta/CII.\{-,h\}/11.9-11 \rangle$  (but see Sections S1.5,S2.4),
- CI continuously binds  $O_{\{L,R\}}\{1,2\}$   $\langle 2/a/\beta/CII.\{-,h\}/1.2,1.6 \rangle$ ,
- at low concentration, CI mediates transcription (of  $cI$ ) from  $P_{RM} \langle 2/a/\beta/CII.\{-,h\}/1.2 - [OLR12\_CI, PRM\_tr] \rangle$
- at medium concentration, CI strongly inhibits  $P_{RM}$  by binding also  $O_{\{L,R\}}3$ , which lowers the CI-concentration from medium by an auto-contravariant effect  $\langle 2/a/\beta/CII.\{-,h\}/1.6 - ![OLR123\_CI]s \rangle$ ,
- $P_R$  is strongly inhibited at all times by CI  $\langle 2/a/\beta/CII.\{-,h\}/1.3,1.7 - CI.\{1,m\}! \rangle$ , i.e., Cro is subject to a standing contravariant effect, meaning Cro dilution is physiological.

The two cases differ only as discussed for “NB8 @  $1/CII.h/11.13-15$ ”, including its discussion of the encountered contravariant effect due to the absence of requisite mediators, i.e., due to non-physiological RNAP-recruitment  $\langle 2/a/\beta/CII._-/1.6 - ![] \rangle$ .

⟨Linearized coextension derivation: 2/a/β/CII.⟩

```

1 [CI.1, Cro.0] + [CII., DNA.ds, RecA.]
2 -> [OLR12_CI, PRM_tr]
3 x> [PR_tr] |-- [CI.1!@[OLR12]]

5 [CI.m, Cro.0] + [CII., DNA.ds, RecA.]
6 -> ![] ; ![OLR123_CI]
7 x> [PR_tr] |-- [CI.m!@[OLR123]]

9 [CI.1, Cro.0] + [CII., DNA.ds, RecA.]
10 -> [OLR12_CI, PRM_tr]
11 x> [PR_tr] |-- [CI.1!@[OLR12]]

```

⌈Visualization: 2/a/β/CII.⌋

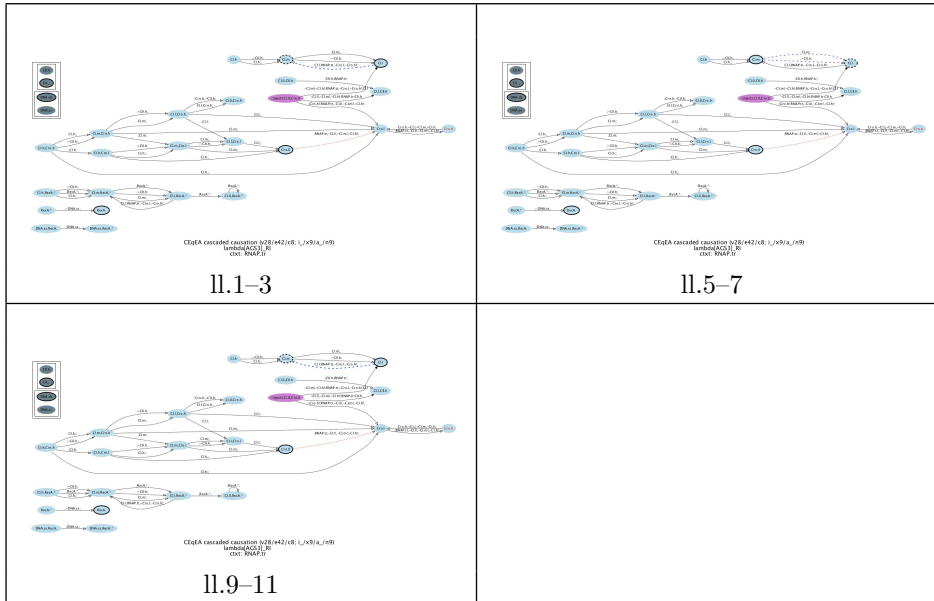

⟨Linearized coextension derivation: 2/a/β/CII.h⟩

```

1 [CI.1, Cro.0] + [CII.h, DNA.ds, RecA.]
2 -> [OLR12_CI, PRM_tr]
3 x> [PR_tr] |-- [CI.1!@[OLR12]]

5 [CI.m, Cro.0] + [CII.h, DNA.ds, RecA.]
6 -> ![OLR123_CI]
7 x> ![ ] |-- [CII.h] ; [PR_tr] |-- [CI.m!@[OLR123]]

9 [CI.1, Cro.0] + [CII.h, DNA.ds, RecA.]
10 -> [OLR12_CI, PRM_tr]
11 x> [PR_tr] |-- [CI.1!@[OLR12]]

```

「Visualization: 2/a/β/CII.h」

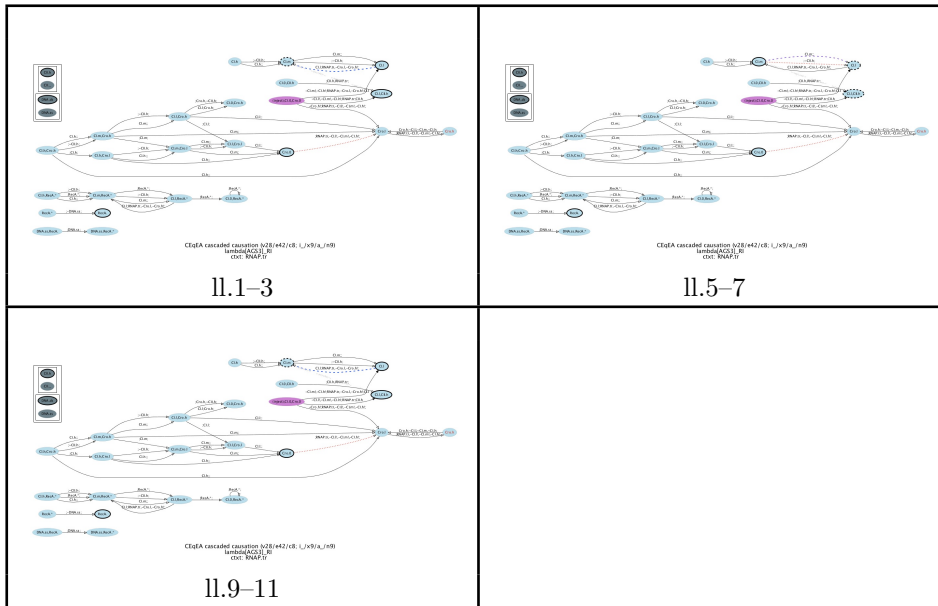

b/ a switch to the lytic attack is not effected by

App.SC:[11:14, 23:6]

i/ natural or operative means  $\heartsuit$  — this is the basis of sustainability

App.SC:[11:14, 22:2, 22:4, 23:1, 47:6, 133:17]

WE ADDRESS THIS PARTLY BY CONSIDERING A COEXTENSION  
STATE SPACE OVER **CI**, **CII**, **Cro**, **DNA.ds**, AND NOT OVER  
**RECA.\***, SEE  $\heartsuit$ .

(See comments at 2/a/ $\alpha$ /.)

The ‘operative’ part of this property follows from observing that  
boxes exist (around the “**CI**.{1,m},**CII**.{\_,h},**Cro**.0,**DNA.ds**”  
nodes) that precisely account for the lysogenic cycle, see 2/a/ $\beta$ /,  
and that the boxes have no out-edges/are not dashed in either  
CII case.

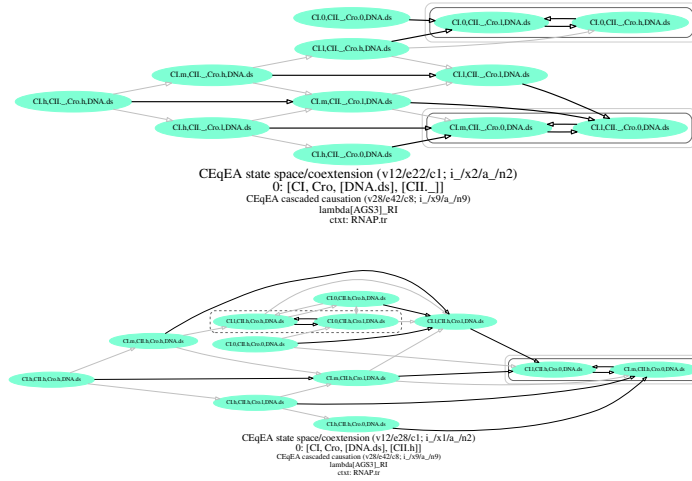

The ‘natural’ part follows by noting that [28] does not discuss  
(and, as implied, Section S2.1 does not include) the possibility  
of a dramatic host size change, or similar, that suddenly leaves  
CI at non-physiological concentration.

ii/ Cro-perturbation ♡ — this is the key means of homeostasis

App.SC:[133:17]

WE ADDRESS THIS BY INTERACTIVELY ENABLING THE “**Cro.L**” NODE IN THE DISCRETE SCENARIOS OF A LYSOGENIC CYCLE, SEE 2/A/ $\beta$ /.

- The interactively-introduced **Cro.1** in the case of **CII.h+CI.1** disappears again immediately:  $\langle 2/b/ii/CII.h+CI.1/ll.1-3 \rangle = \langle 2/b/ii/CII.h+CI.1/ll.9-11 \rangle$ , see 0/CII.h.
- Other than the toggles, the linearized coextension derivation for **CII.\_+CI.1** is identical to that for **CII.h+CI.1**, meaning the reasons (and outcomes) are identical, too, even if the present situation is not addressed in 0/.
- The cases for **Cro**-perturbation of the lysogenic cycle during **CI.m** are identical to each other, except as discussed for “NB8 @ 1/CII.h/ll.13–15”. The **CI.m** cases are largely identical to the **CI.1** cases, except for unrelated issues.

⟨Linearized coextension derivation: 2/b/ii/CII.\_+CI.1⟩

```

1 [CI.1, Cro.0] + [CII._, DNA.ds, RecA.]
2 -> [OLR12_CI, PRM_tr]
3 x> [PR_tr] |-- [CI.1!@[OLR12]]

5 [CI.1, Cro.1] + [CII._, DNA.ds, RecA.]
6 -> ![OLR12_CI]
7 x> [PR_tr] |-- [CI.1!@[OLR12]] ; [OLR12_CI, PRM_tr] |--
   [Cro.1@[OR3]]

9 [CI.1, Cro.0] + [CII._, DNA.ds, RecA.]
10 -> [OLR12_CI, PRM_tr]
11 x> [PR_tr] |-- [CI.1!@[OLR12]]

```

⌈Visualization: 2/b/ii/CII.\_+CI.1⌋

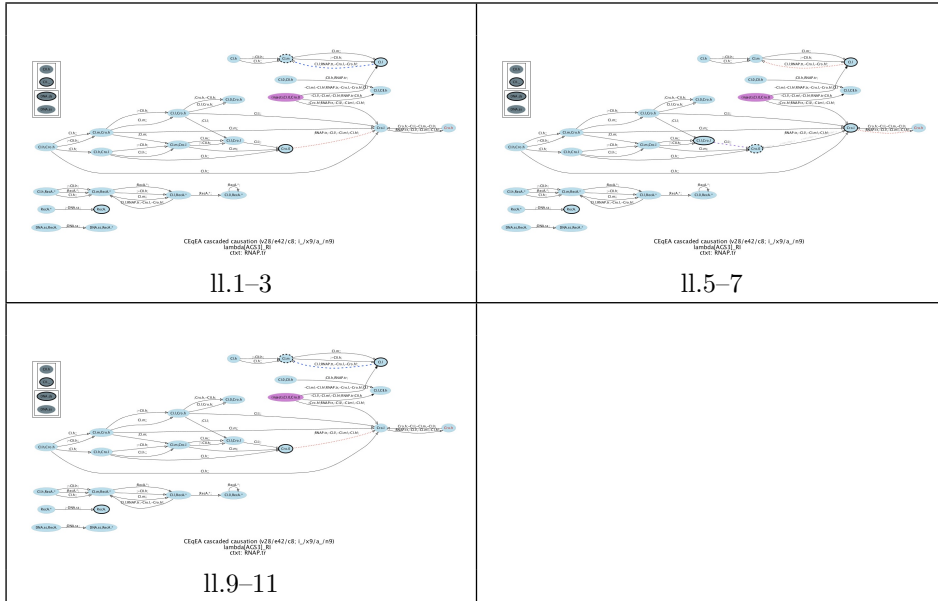

⟨Linearized coextension derivation: 2/b/ii/CII.\_+CI.m⟩

```

1 [CI.m, Cro.0] + [CII._, DNA.ds, RecA.]
2 -> ![] ; ![OLR123_CI]
3 x> [PR_tr] |-- [CI.m!@[OLR123]]

5 [CI.m, Cro.1] + [CII._, DNA.ds, RecA.]
6 -> ![] ; ![OLR123_CI]
7 x> [PR_tr] |-- [CI.m!@[OLR123]]

9 [CI.1, Cro.0] + [CII._, DNA.ds, RecA.]
10 -> [OLR12_CI, PRM_tr]
11 x> [PR_tr] |-- [CI.1!@[OLR12]]

```

⌈Visualization: 2/b/ii/CII.\_+CI.m⌋

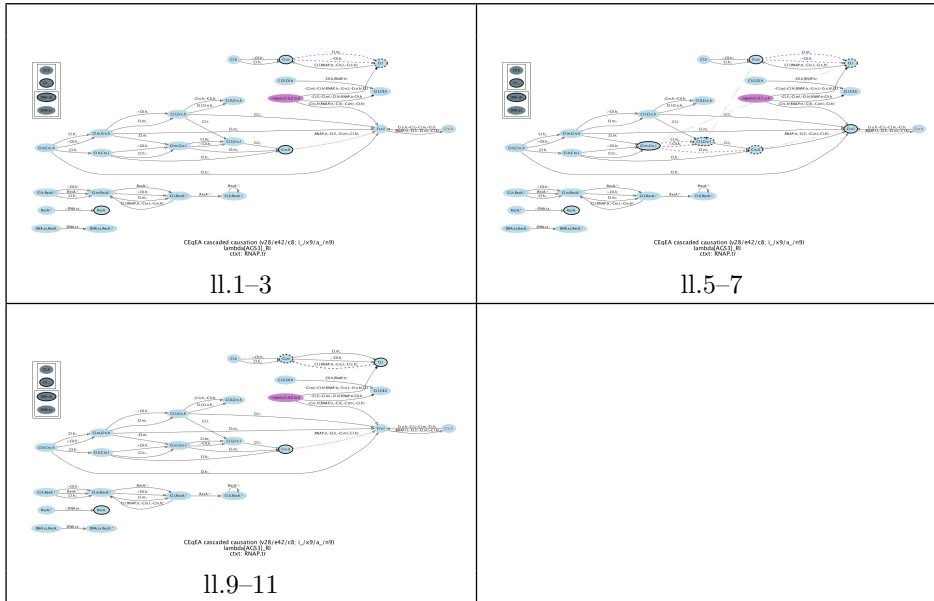

⟨Linearized coextension derivation: 2/b/ii/CII.h+CI.1⟩

```

1 [CI.1, Cro.0] + [CII.h, DNA.ds, RecA.]
2 -> [OLR12_CI, PRM_tr]
3 x> [PR_tr] |-- [CI.1!@[OLR12]]

5 [CI.1, Cro.1] + [CII.h, DNA.ds, RecA.]
6 -> ![OLR12_CI]
7 x> [PR_tr] |-- [CI.1!@[OLR12]] ; [OLR12_CI, PRM_tr] |--
   [Cro.1@[OR3]]

9 [CI.1, Cro.0] + [CII.h, DNA.ds, RecA.]
10 -> [OLR12_CI, PRM_tr]
11 x> [PR_tr] |-- [CI.1!@[OLR12]]

```

⌈Visualization: 2/b/ii/CII.h+CI.1⌋

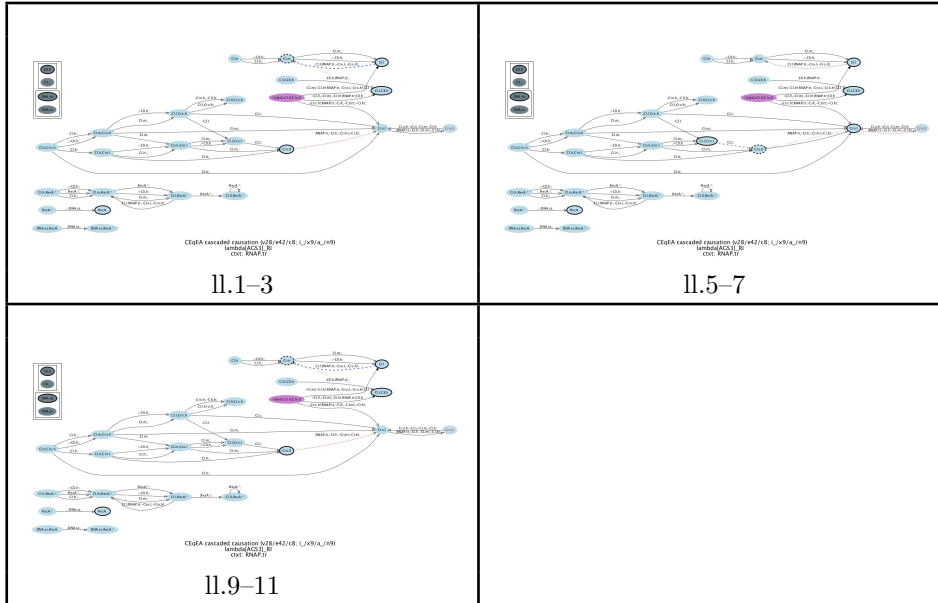

⟨Linearized coextension derivation: 2/b/ii/CII.h+CI.m⟩

```

1 [CI.m, Cro.0] + [CII.h, DNA.ds, RecA.]
2 -> ![OLR123_CI]
3 x> ![[] |-- [CII.h] ; [PR_tr] |-- [CI.m!@[OLR123]]

5 [CI.m, Cro.1] + [CII.h, DNA.ds, RecA.]
6 -> ![OLR123_CI]
7 x> ![[] |-- [CII.h] ; [PR_tr] |-- [CI.m!@[OLR123]]

9 [CI.1, Cro.0] + [CII.h, DNA.ds, RecA.]
10 -> [OLR12_CI, PRM_tr]
11 x> [PR_tr] |-- [CI.1!@[OLR12]]

```

⌈Visualization: 2/b/ii/CII.h+CI.m⌋

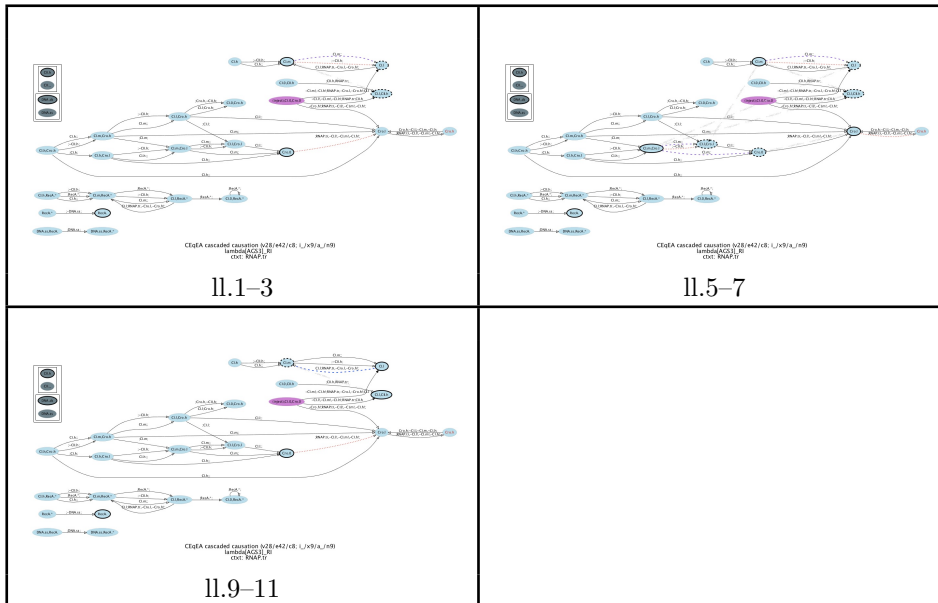

iii/ super-infection ♡ — this is  $\lambda$ -immunity

App.SC:[12:10b, 13:Fig.1.3:1, 67:-1, 133:17, (12:10a)]

WE ADDRESS THIS BY INTERACTIVELY ENABLING THE (INJECT) CHANNEL IN THE DISCRETE SCENARIOS OF A LYSOGENIC CYCLE, SEE 2/A/ $\beta$ /.

The mechanism behind  $\lambda$ -immunity is the same whether CII is below or at high concentration and whether the super-infection takes place while CI is (more) at low or (more) at medium concentration in the lysogenic cycle: in order for a switch to the lytic attack to take place, *cro* must be transcribed from  $P_R$  but CI continuously occupies  $O_{\{L,R\}}\{1,2\}$   $\langle 2/b/iii/CII.\{-,h\}+CI.\{1,m\}/1.2,1.6,1.10 \rangle$ , which effects strong inhibition  $\langle 2/b/iii/CII.\{-,h\}+CI.\{1,m\}/1.3,1.7,1.11 - [CI.\{1,m\}!@[\dots]] \rangle$ .

Each of the four situations is considered below — in each case, the super-infection is simply absorbed into the lysogenic cycle, i.e., the next step in each derivation is the same as what would have been the next step if no super-infection had taken place, see 2/a/ $\beta$ /:  $\langle 2/b/iii/CII._+CI.1/11.9-11 \rangle = \langle 2/b/iii/CII._+CI.m/11.1-3 \rangle$ , and so on.

NB! Due to the absence of regulatory mechanisms that apply to CI.0 in case of CII.\_, the state is noted as being inert at the point of infection  $\langle 2/b/iii/CII._+CI.\{1,m\}/1.5 \rangle$ . At the same time, *cI* is also noted as being active in state CI. $\{1,m\}$   $\langle 2/b/iii/CII._+CI.\{1,m\}/1.5 \rangle$ . This corresponds to the pre-existing *cI* remaining actively regulated-upon while the super-infecting *cI* is awaiting initial regulation — it receives this in the ensuing step, meaning no CI state is counted as a separate (inert) entity at that point  $\langle 2/b/iii/CII._+CI.\{1,m\}/1.9 \rangle$ . A related property holds in case of CII.h.

⟨Linearized coextension derivation: 2/b/iii/CII.\_+CI.1⟩

```

1 [CI.1, Cro.0] + [CII._, DNA.ds, RecA.]
2 -> [OLR12_CI, PRM_tr]
3 x> [PR_tr] |-- [CI.1!@[OLR12]]

5 [CI.1, Cro.0] + [(inject), CI.0, CII._, DNA.ds, RecA.]
6 -> [OLR12_CI, PRM_tr]
7 x> [PR_tr] |-- [CI.1!@[OLR12]]

9 [CI.m, Cro.0] + [CII._, DNA.ds, RecA.]
10 -> ![] ; ![OLR123_CI]
11 x> [PR_tr] |-- [CI.m!@[OLR123]]

```

⌈Visualization: 2/b/iii/CII.\_+CI.1⌋

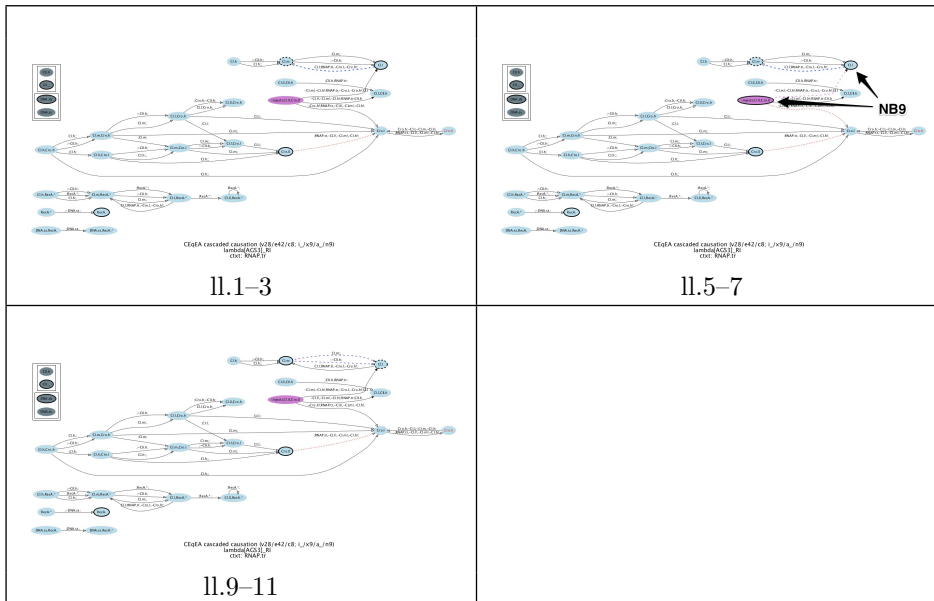

⟨Linearized coextension derivation: 2/b/iii/CII.\_+CI.m⟩

```

1  [CI.m, Cro.0] + [CII._, DNA.ds, RecA.]
2  -> ![] ; ![OLR123_CI]
3  x> [PR_tr] |-- [CI.m!@[OLR123]]

5  [CI.m, Cro.0] + [(inject), CI.0, CII._, DNA.ds, RecA.]
6  -> ![] ; ![OLR123_CI]
7  x> [PR_tr] |-- [CI.m!@[OLR123]]

9  [CI.1, Cro.0] + [CII._, DNA.ds, RecA.]
10 -> [OLR12_CI, PRM_tr]
11 x> [PR_tr] |-- [CI.1!@[OLR12]]

```

⌈Visualization: 2/b/iii/CII.\_+CI.m⌋

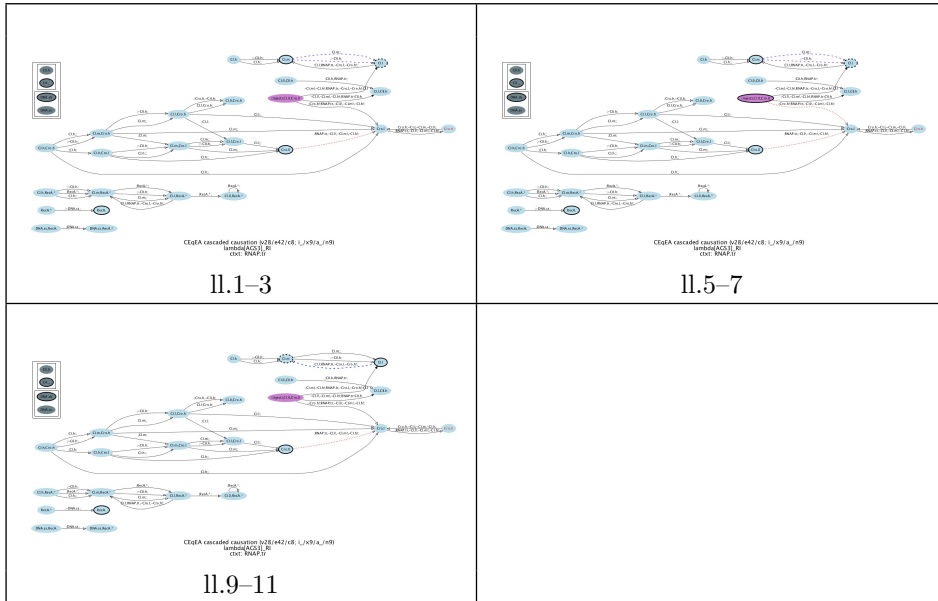

⟨Linearized coextension derivation: 2/b/iii/CII.h+CI.1⟩

```

1  [CI.1, Cro.0] + [CII.h, DNA.ds, RecA.]
2  ->  [OLR12_CI, PRM_tr]
3  x>  [PR_tr] |-- [CI.1!@[OLR12]]

5  [CI.0, CI.1, Cro.0] + [(inject), CII.h, DNA.ds, RecA.]
6  ->  [OLR12_CI, PRM_tr]
7  x>  [PR_tr] |-- [CI.1!@[OLR12]] ; [PRE_tr, ORE_CII] |--
    [CI.1!@[OLR12]]

9  [CI.m, Cro.0] + [CII.h, DNA.ds, RecA.]
10 ->  ![OLR123_CI]
11 x>  ![ ] |-- [CII.h] ; [PR_tr] |-- [CI.m!@[OLR123]]

```

Visualization: 2/b/iii/CII.h+CI.1

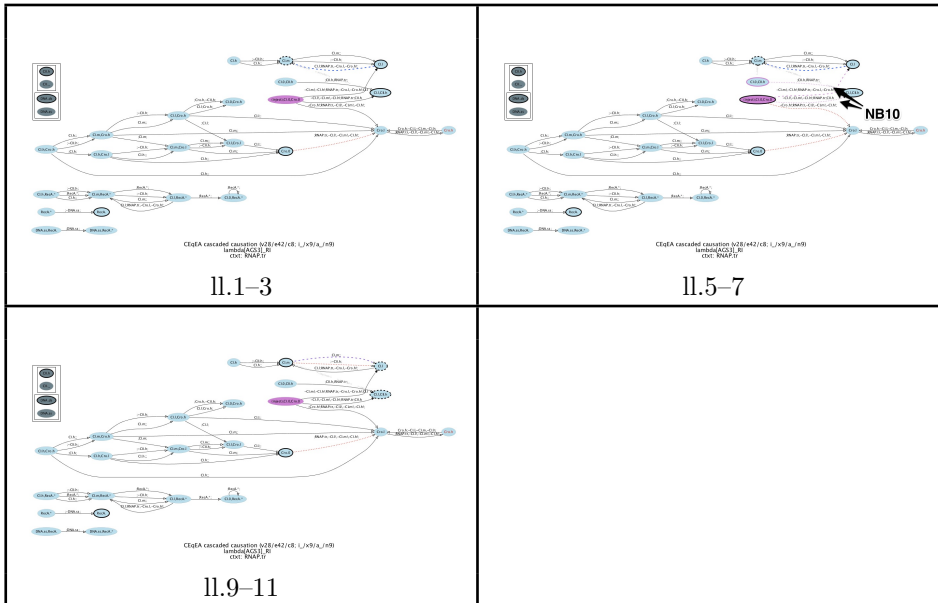

⟨Linearized coextension derivation: 2/b/iii/CII.h+CI.m⟩

```

1  [CI.m, Cro.0] + [CII.h, DNA.ds, RecA.]
2  ->  ![OLR123_CI]
3  x>  ![ ] |-- [CII.h] ; [PR_tr] |-- [CI.m!@[OLR123]]

5  [CI.0, CI.m, Cro.0] + [(inject), CII.h, DNA.ds, RecA.]
6  ->  ![OLR123_CI]
7  x>  ![ ] |-- [CII.h] ; [PR_tr] |-- [CI.m!@[OLR123]] ;
      [PRE_tr, ORE_CII] |-- [CI.m!@[OLR123]]

9  [CI.1, Cro.0] + [CII.h, DNA.ds, RecA.]
10 ->  [OLR12_CI, PRM_tr]
11 x>  [PR_tr] |-- [CI.1!@[OLR12]]

```

Visualization: 2/b/iii/CII.h+CI.m

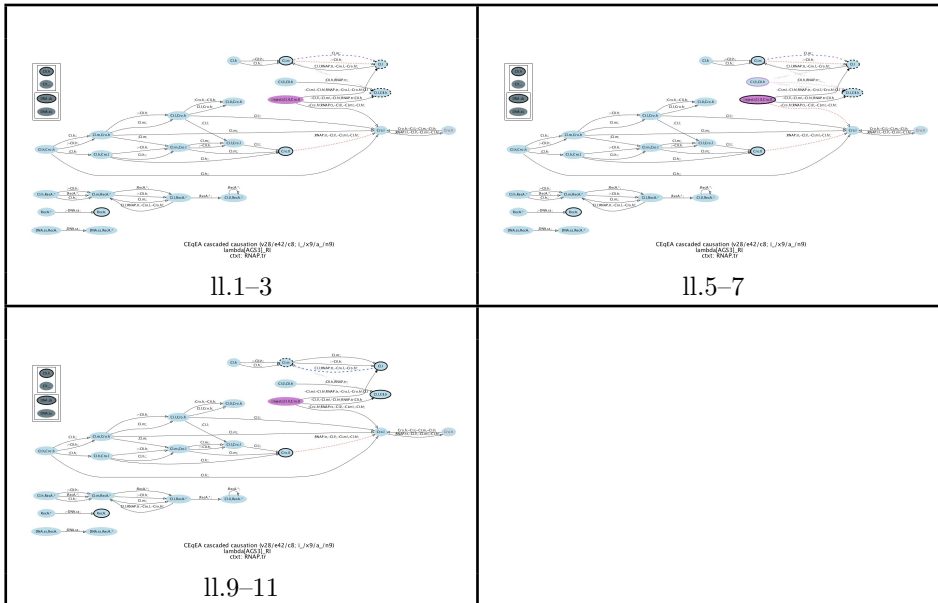

c/ a switch to the lytic attack is effected by UV-irradiation (via  $\neg\heartsuit$ )

App.SC:[1:3, 1:13, 9:1, 11:21, 11:23, 12:-11, 13:Fig.1.2:1, 24:-7, 25:7, 27:19, 27:-7, 47:11, 60:-1, 61:10, 64:1, 64:8, 67:-1, 94:-7b, 133:15, 133:17]

WE ADDRESS THIS BY INTERACTIVELY TOGGING “DNA.ss” IN THE DISCRETE SCENARIOS OF A LYSOGENIC CYCLE, SEE 2/A/ $\beta$ /.

The import of the derivations we discuss is best appreciated in the visualizations or in the video — little additional information is revealed in the details.

When we toggle “DNA.ss”, we activate also the “DNA.ss,RecA.” node’s outgoing edge: [UV\_irr]  $\langle 2/c/CII.\{-,h\}+CI.\{1,m\}/1.6 \rangle$ , see Section S2.1.5. The edge concerns activation of RecA: RecA.\*  $\langle 2/c/CII.\{-,h\}+CI.\{1,m\}/1.9 \rangle$ , which brings the host’s SOS response to bear on  $\lambda \langle 2/c/CII.\{-,h\}+CI.\{1,m\}/1.10 \rangle$ . This leads to a decrease of CI’s concentration  $\langle 2/c/CII.\{-,h\}+CI.\{1,m\}/1.9,1.13 \rangle$  because RecA.\*-mediated CI auto-proteolysis countermands, i.e., coinhibits, any CI contribution from P<sub>RM</sub>- $\langle 2/c/CII.\{-,h\}+CI.1/1.15 \rangle$ ,  $\langle 2/c/CII.\{-,h\}+CI.m/1.11 \rangle$  and P<sub>RE</sub>-transcription  $\langle 2/c/CII.h+CI.1/1.19,1.23,1.27,1.31 \rangle$ ,  $\langle 2/c/CII.h+CI.m/1.15,1.19,1.23,1.27 \rangle$ . Other than inert CI.0 and coinhibition of P<sub>RE</sub>-based *cI*-expression, the last five steps  $\langle 2/c/CII.\{-,h\}+CI.1/1.13-33 \rangle$ ,  $\langle 2/c/CII.\{-,h\}+CI.m/1.9-29 \rangle$  are identical in all cases: CI goes non-physiological, allowing for a constitutive lytic attack, see 3/a/ $\alpha$ /.

⟨Linearized coextension derivation: 2/c/CII.\_+CI.1⟩

---

```

1  [CI.1, Cro.0] + [CII._, DNA.ds, RecA.]
2  -> [OLR12_CI, PRM_tr]
3  x> [PR_tr] |-- [CI.1!@[OLR12]]

5  [CI.1, Cro.0, RecA.] + [CII._, DNA.ss]
6  -> [OLR12_CI, PRM_tr] ; [UV_irr]
7  x> [PR_tr] |-- [CI.1!@[OLR12]]

9  [CI.m, Cro.0, RecA.*] + [CII._, DNA.ss]
10 -> ![] ; ![OLR123_CI] ; [SOS]
11 x> ![] |-- [DNA.ss] ; [PR_tr] |-- [CI.m!@[OLR123]]

13 [CI.1, Cro.0, RecA.*] + [CII._, DNA.ss]
14 -> [SOS]
15 x> ![] |-- [DNA.ss] ; [PR_tr] |-- [CI.1!@[OLR12]] ;
    [OLR12_CI, PRM_tr] |-- [SOS]

17 [Cro.0, RecA.*] + [CI.0, CII._, DNA.ss]
18 -> [PR_tr] ; [SOS]
19 x> ![] |-- [DNA.ss]

21 [Cro.1, RecA.*] + [CI.0, CII._, DNA.ss]
22 -> [PR_tr] ; [SOS]
23 x> ![] |-- [DNA.ss]

25 [Cro.h, RecA.*] + [CI.0, CII._, DNA.ss]
26 -> ![OR2_Cro, OR1_Cro] ; [SOS]
27 x> ![] |-- [DNA.ss]

29 [Cro.1, RecA.*] + [CI.0, CII._, DNA.ss]
30 -> [PR_tr] ; [SOS]
31 x> ![] |-- [DNA.ss]

33 <expired>

```

Visualization: 2/c/CII.-+CI.1

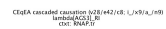

11.1-3

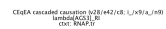

11.5-7

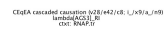

11.9-11

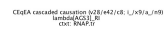

11.13–15

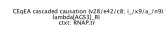

11.17–19

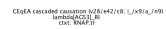

11.21–23

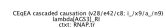

11.25–27

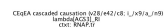

11.29–33

⟨Linearized coextension derivation: 2/c/CII.\_+CI.m⟩

---

```

1  [CI.m, Cro.0] + [CII._, DNA.ds, RecA.]
2  -> ![] ; ![OLR123_CI]
3  x> [PR_tr] |-- [CI.m!@[OLR123]]

5  [CI.m, Cro.0, RecA.] + [CII._, DNA.ss]
6  -> ![] ; ![OLR123_CI] ; [UV_irr]
7  x> [PR_tr] |-- [CI.m!@[OLR123]]

9  [CI.1, Cro.0, RecA.*] + [CII._, DNA.ss]
10 -> [SOS]
11 x> ![] |-- [DNA.ss] ; [PR_tr] |-- [CI.1!@[OLR12]] ;
    [OLR12_CI, PRM_tr] |-- [SOS]

13 [Cro.0, RecA.*] + [CI.0, CII._, DNA.ss]
14 -> [PR_tr] ; [SOS]
15 x> ![] |-- [DNA.ss]

17 [Cro.1, RecA.*] + [CI.0, CII._, DNA.ss]
18 -> [PR_tr] ; [SOS]
19 x> ![] |-- [DNA.ss]

21 [Cro.h, RecA.*] + [CI.0, CII._, DNA.ss]
22 -> ![OR2_Cro, OR1_Cro] ; [SOS]
23 x> ![] |-- [DNA.ss]

25 [Cro.1, RecA.*] + [CI.0, CII._, DNA.ss]
26 -> [PR_tr] ; [SOS]
27 x> ![] |-- [DNA.ss]

29 <expired>

```

Visualization: 2/c/CII.\_+CI.m

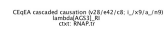

11.1-3

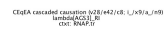

11.5-7

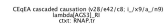

11.9-11

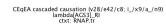

11.13–15

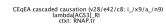

11.17–19

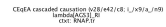

11.21–23

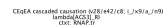

11.25–29

⟨Linearized coextension derivation: 2/c/CII.h+CI.1⟩

---

```

1  [CI.1, Cro.0] + [CII.h, DNA.ds, RecA.]
2  -> [OLR12_CI, PRM_tr]
3  x> [PR_tr] |-- [CI.1!@[OLR12]]

5  [CI.1, Cro.0, RecA.] + [CII.h, DNA.ss]
6  -> [OLR12_CI, PRM_tr] ; [UV_irr]
7  x> [PR_tr] |-- [CI.1!@[OLR12]]

9  [CI.m, Cro.0, RecA.*] + [CII.h, DNA.ss]
10 -> ![OLR123_CI] ; [SOS]
11 x> ![] |-- [DNA.ss, CII.h] ; [PR_tr] |-- [CI.m!@[OLR123]]

13 [CI.1, Cro.0, RecA.*] + [CII.h, DNA.ss]
14 -> [SOS]
15 x> ![] |-- [DNA.ss] ; [PR_tr] |-- [CI.1!@[OLR12]] ;
    [OLR12_CI, PRM_tr] |-- [SOS]

17 [CI.0, Cro.0, RecA.*] + [CII.h, DNA.ss]
18 -> [PR_tr] ; [SOS]
19 x> ![] |-- [DNA.ss] ; [PRE_tr, ORE_CII] |-- [SOS]

21 [CI.0, Cro.1, RecA.*] + [CII.h, DNA.ss]
22 -> [PR_tr] ; [SOS]
23 x> ![] |-- [DNA.ss] ; [PRE_tr, ORE_CII] |-- [SOS]

25 [CI.0, Cro.h, RecA.*] + [CII.h, DNA.ss]
26 -> ![OR2_Cro, OR1_Cro] ; [SOS]
27 x> ![] |-- [DNA.ss] ; [PRE_tr, ORE_CII] |-- [SOS]

29 [CI.0, Cro.1, RecA.*] + [CII.h, DNA.ss]
30 -> [PR_tr] ; [SOS]
31 x> ![] |-- [DNA.ss] ; [PRE_tr, ORE_CII] |-- [SOS]

33 <expired>

```

Visualization: 2/c/CII.h+CI.1

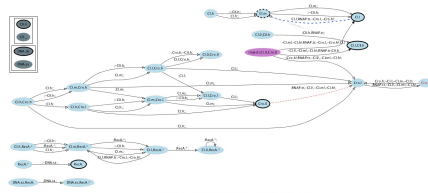

11.1-3

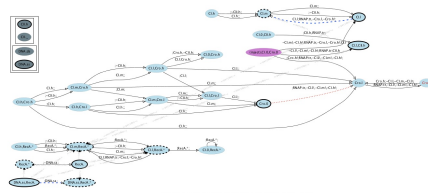

11.5-7

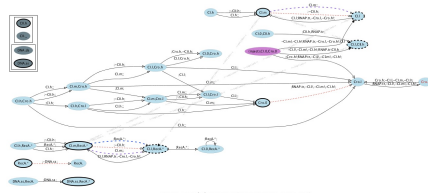

11.9-11

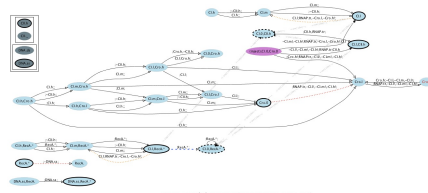

11.13–15

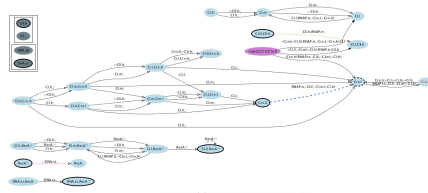

11.17–19

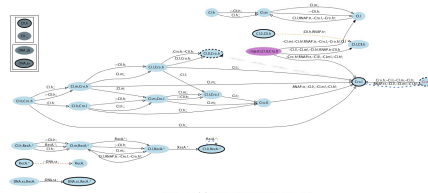

11.21–23

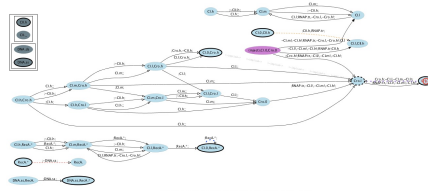

11.25–27

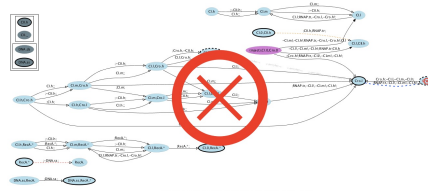

11.29–33

⟨Linearized coextension derivation: 2/c/CII.h+CI.m⟩

---

```

1  [CI.m, Cro.0] + [CII.h, DNA.ds, RecA.]
2  -> ![OLR123_CI]
3  x> ![[] |-- [CII.h] ; [PR_tr] |-- [CI.m!@[OLR123]]

5  [CI.m, Cro.0, RecA.] + [CII.h, DNA.ss]
6  -> ![OLR123_CI] ; [UV_irr]
7  x> ![[] |-- [CII.h] ; [PR_tr] |-- [CI.m!@[OLR123]]

9  [CI.1, Cro.0, RecA.*] + [CII.h, DNA.ss]
10 -> [SOS]
11 x> ![[] |-- [DNA.ss] ; [PR_tr] |-- [CI.1!@[OLR12]] ;
    [OLR12_CI, PRM_tr] |-- [SOS]

13 [CI.0, Cro.0, RecA.*] + [CII.h, DNA.ss]
14 -> [PR_tr] ; [SOS]
15 x> ![[] |-- [DNA.ss] ; [PRE_tr, ORE_CII] |-- [SOS]

17 [CI.0, Cro.1, RecA.*] + [CII.h, DNA.ss]
18 -> [PR_tr] ; [SOS]
19 x> ![[] |-- [DNA.ss] ; [PRE_tr, ORE_CII] |-- [SOS]

21 [CI.0, Cro.h, RecA.*] + [CII.h, DNA.ss]
22 -> ![OR2_Cro, OR1_Cro] ; [SOS]
23 x> ![[] |-- [DNA.ss] ; [PRE_tr, ORE_CII] |-- [SOS]

25 [CI.0, Cro.1, RecA.*] + [CII.h, DNA.ss]
26 -> [PR_tr] ; [SOS]
27 x> ![[] |-- [DNA.ss] ; [PRE_tr, ORE_CII] |-- [SOS]

29 <expired>

```

「Visualization: 2/c/CII.h+CI.m」

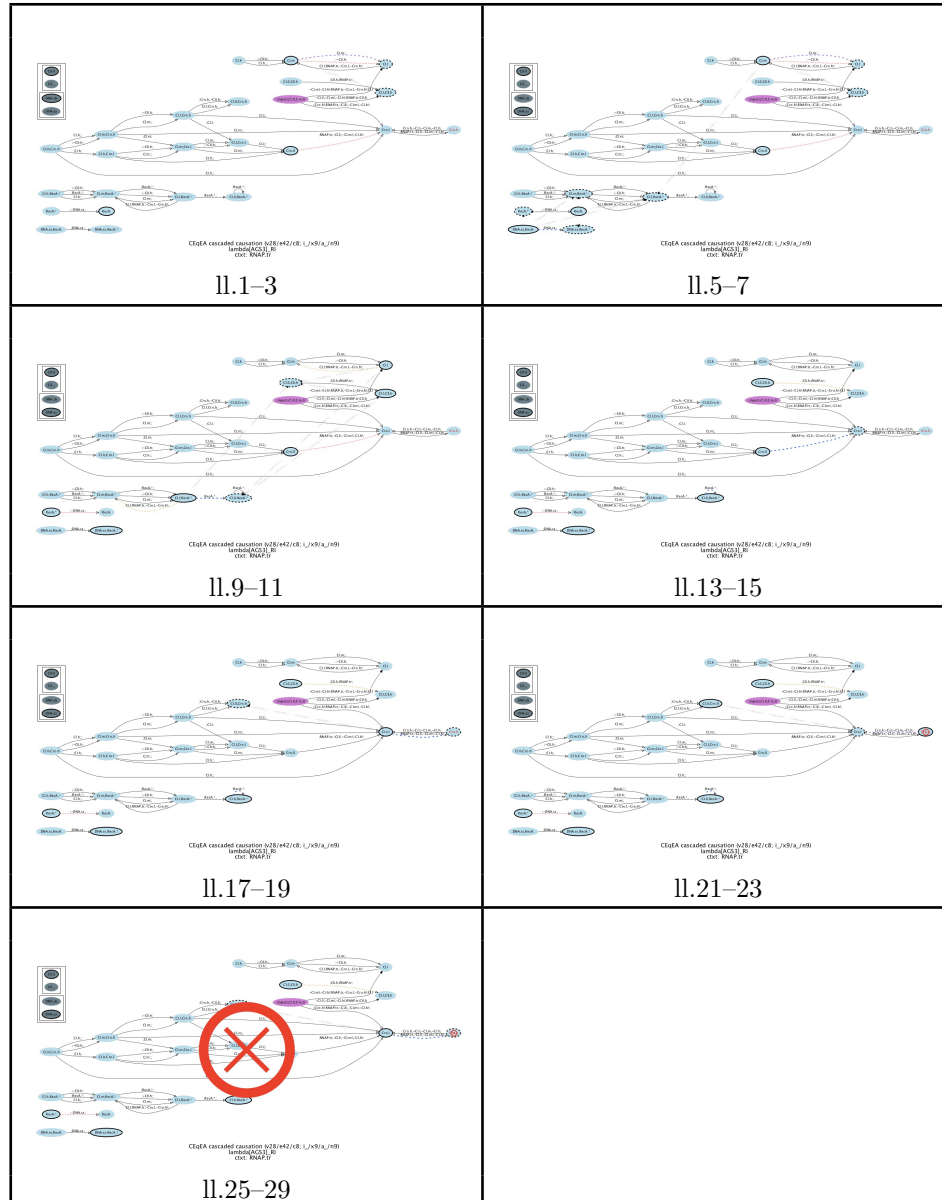

3/ the lytic attack expires the host and, else, is sustainable but *not homeostatic*

App.SC:[1:7, 133:15]

a/ protein concentrations are programmatic during a lytic attack

App.SC:[11:9]

In the simplest form, it suffices to observe that none of the linearized coextension derivations in 3/a/{ $\alpha, \beta, \gamma$ }/ list a divergence but the reasoning details are instructive.

$\alpha$ / the lytic attack is constitutive  $\neg\heartsuit$  or  $\spadesuit$

App.SC:[11:21, 12:-11, 50:6, 52:5]

See 2/c/ for the case of  $\neg\heartsuit$  and 1/CII.\_ for the case of  $\spadesuit$ : the lytic attack is initiated from situations where CI and Cro are non-physiological  $\langle 1/\text{CII}._/1.1 \rangle$ ,  $\langle 2/c/\text{CII}._\{-, \mathbf{h}\} + \text{CI}._1/1.17 \rangle$ ,  $\langle 2/c/\text{CII}._\{-, \mathbf{h}\} + \text{CI}._m/1.13 \rangle$  by means of non-mediated, i.e., constitutive,  $P_R$ -transcription, indicated by  $\text{PR}_{\text{tr}}$  occurring by itself within [...]s in the associated linearized coextension derivations  $\langle 1/\text{CII}._/1.2 \rangle$ ,  $\langle 2/c/\text{CII}._\{-, \mathbf{h}\} + \text{CI}._1/1.18 \rangle$ ,  $\langle 2/c/\text{CII}._\{-, \mathbf{h}\} + \text{CI}._m/1.14 \rangle$ .

$\beta$ / once initiated, Cro remains physiological and CI inoperative  $\neg\heartsuit$  or  $\spadesuit$

App.SC:[12:-5, 15:-10, 25:-2b, 47:-9, 52:5, 136:15]

See 2/c/ for the case of  $\neg\heartsuit$  and 1/CII.\_ for the case of  $\spadesuit$ : Cro remains physiological and CI remains non-physiological throughout the lytic attack in both scenarios  $\langle 1/\text{CII}._/11.5-17 \rangle$ ,  $\langle 2/c/\text{CII}._\{-, \mathbf{h}\} + \text{CI}._1/11.21-33 \rangle$ ,  $\langle 2/c/\text{CII}._\{-, \mathbf{h}\} + \text{CI}._m/11.17-29 \rangle$ . It remains to consider the details and to argue that CI is inoperative and in what sense.

- In case of  $\spadesuit$ , see 1/CII.\_, the injected  $cI$  remains inert in state  $\text{CI}._0$   $\langle 1/\text{CII}._/11.1-15 \rangle$ : the considered scenario is devoid of regulatory functionality that can change the concentration of CI from non-physiological. The concentration of Cro is mostly guided by constitutive  $P_R$ -transcription:  $\langle 1/\text{CII}._/1.2, 1.6, 1.14 \rangle$ , except at high concentration where Cro binds (independently) to both  $O_{R1}$  and  $O_{R2}$  to effect strong inhibition on  $cro$ -transcription  $\langle 1/\text{CII}._/1.10/[O_{R2}\text{-Cro}, O_{R1}\text{-Cro}] \rangle$ , see Section S2.1, resulting in a concentration drop till

constitutive  $P_R$ -transcription becomes physiological again  $\langle 1/CII._/ll.13-14 \rangle$ , but see 3/a/ $\gamma$ / (and Section S1.5).

- In case of  $\neg\heartsuit$ , see 2/c/, control of **Cro**'s concentration is as above, while the host's SOS response continuously keeps the concentration of **CI** at a non-physiological level by countermanding any expression from  $P_{RE}$ - and  $P_{RM}$ -transcription  $\langle 2/c/CII._+CI.1/1.10,1.14,1.15,1.18,1.22,1.26,1.30 \rangle$ ,  $\langle 2/c/CII._+CI.m/1.10,1.11,1.14,1.18,1.22,1.26 \rangle$ ,  $\langle 2/c/CII.h+CI.1/1.10,1.14,1.15,1.18,1.19,1.22,1.23,1.26,1.27,1.30,1.31 \rangle$ ,  $\langle 2/c/CII.h+CI.m/1.10,1.11,1.14,1.15,1.18,1.19,1.22,1.23,1.26,1.27 \rangle$ .

With this, we see that 'inoperative' means that no **CI** is present and none may be produced due to lack of RNAP-recruiting mediators (in case of  $CII._$ ) or that any production is countermanded by proteolysis (in case of  $CII.h$ ).

$\gamma$ / a lytic attack expires the host after Cro has reached high  $\neg\heartsuit$  or  $\spadesuit$

App.SC:[1:3, 11:9, 11:21]

[28] does not discuss the details of the regulatory mechanisms that orchestrate lysis of the host beyond [[28]:52:5]/App.SE/Late lytic, which includes the assertion that lysis happens some time after **Cro** has begun binding to  $O_R3$ , i.e., some time after **Cro.1** has been reached, see Section S2.1, and, in particular, shortly after **Cro** has then begun to bind also  $O_R\{1,2\}$  and, in the process, repressing  $P_R$ , i.e., shortly after **Cro.h** has been reached. In our discretized analysis, this manifests itself as **Cro.1** being re-encountered after **Cro.h**. This is reflected in our [28]-transliterated  $\lambda$ -specification, see Section S2.1, which states that any automated proving will **expire**/terminate one step (the second '1') after the first time (the first '1') the "**Cro.h**"-node has been enabled:

"**Cro.h**" | **expire**(1,1) ;

Expiration is indicated by **<expired>** in the linearized coextension derivations and by a red circle+x icon in the visualizations. See also 3/b/.

b/ ignoring host expiration, a switch to the lysogenic cycle is not effected by

FURTHER TO 3/A/ $\gamma$ /, CEQEA'S PROOF ENGINE HAS THE EXPIRATION MECHANISM TURNED OFF FOR 3/{B,C}. THIS IS DONE BY TYPING CTRL+SHIFT+O IN A CASCADED CAUSATION DIAGRAM AND UNTICKING THE FOLLOWING OPTION:

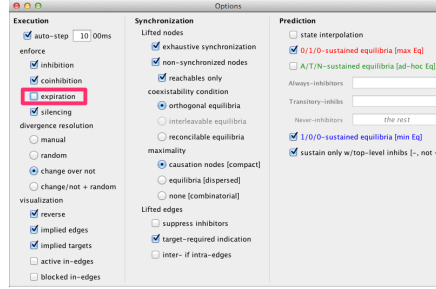

i/ natural or operative means  $\neg\heartsuit$  or  $\spadesuit$  — this is the basis of sustainability

App.SC:[(92, Fig.4.23:1)]

WE ADDRESS THIS PARTLY BY CONSIDERING COEXTENSION STATE SPACES.

(See comments at  $2/a/\alpha/.$ )

For the  $\neg\heartsuit$  case of the ‘operative’ part, we consider coextension state spaces over  $CI$ ,  $CII.\{-,h\}$ ,  $Cro$ ,  $DNA.ss$ , and  $RecA$  (both states). It suffices to observe that boxes exist (around the “ $CI.0, CII.\{-,h\}, Cro.\{1,h\}, DNA.ss, RecA.*$ ” nodes) that precisely account for the lytic attack (ignoring host destruction), see  $3/a/\beta/$ , and that the boxes have no out-edges/are not dashed.

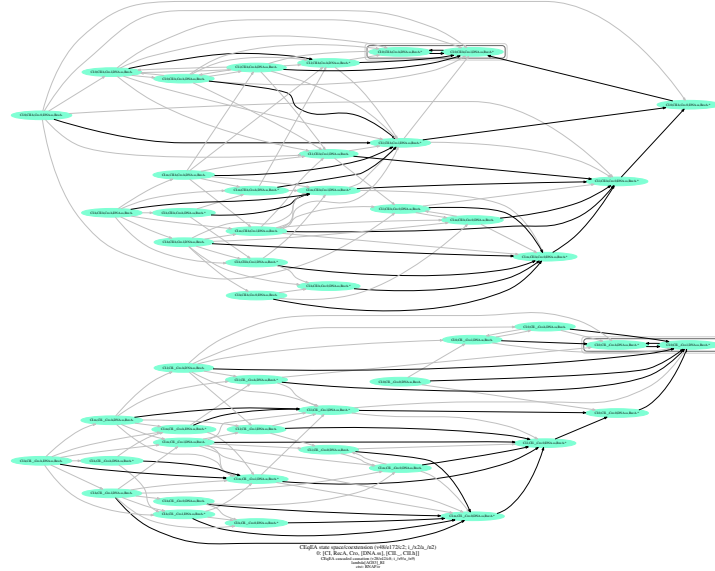

For the  $\heartsuit$  and  $\spadesuit$  case of the ‘operative’ part, we consider a coextension state space over  $CI$ ,  $CII._$ ,  $Cro$ , and

DNA.ds. It suffices to observe that a box exists (around the “CI.O,CII.~,Cro.{1,h},DNA.ds” nodes) that precisely accounts for the lytic attack (ignoring host destruction), see 3/a/ $\beta$ /, and that the box has no out-edges/is not dashed.

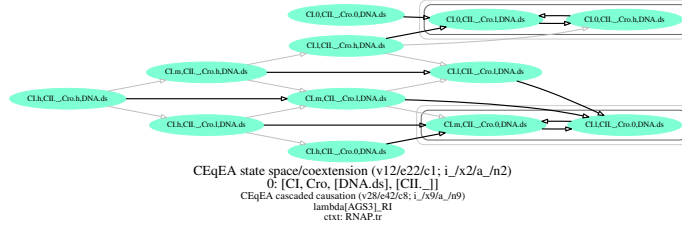

NB! As seen in the coextension state space with CII.h in 2/b/i/, the property we consider here does not hold in case of  $\heartsuit$  and  $\spadesuit$ : the lytic-attack box has out-edges/is dashed in that case.

The ‘natural’ part follows by noting that [28] does not discuss (and Section S2.1 does not include) the possibility of a dramatic host size change, or similar, that suddenly leaves any operative protein at non-physiological concentration.

ii/ CI-perturbation  $\neg\heartsuit$ , although the lytic attack may be set back

App.SC:[62:-1]

WE ADDRESS THIS BY INTERACTIVELY ENABLING THE “CI.L” NODE IN THE DISCRETE SCENARIOS OF A LYTIC ATTACK, SEE 3/A/ $\beta$ /, BUT WITHOUT USING CeqEA’S EXPIRATION MECHANISM, SEE 3/B/.

Following the perturbation, CI is inescapably returned to zero concentration by proteolysis mediated by the host SOS response  $\langle 3/b/ii/CII.\{-,h\}+SOS+Cro.\{1,h\}/11.1-15 \rightarrow [SOS] \rangle$ . Any attempted auto-mediation by CI is also inhibited by Cro  $\langle 3/b/ii/CII.\{-,h\}+SOS+Cro.\{1,h\}/1.7 \rightarrow [OLR12\_CI,PRM\_tr] \dashv\vdash [Cro\dots] \rangle$ . In the Cro.h cases, the inhibition is contravariant  $\langle 3/b/ii/CII.\{-,h\}+SOS+Cro.h/1.6 \rightarrow \neg [OLR12\_CI,OR3\_Cro]; \neg [OR3\_Cro] \rangle$ , meaning Cro mediates a CI-concentration decrease. The introduced CI will contravariantly inhibit Cro expression  $\langle 3/b/ii/CII.\{-,h\}+SOS+Cro.\{1,h\}/1.6 \rightarrow \neg [OLR12\_CI] \rangle$  but may not be present for long enough to see through an explicit lowering of Cro’s concentration, see ‘divergence resolution’ below. In either scenario, the lytic attack

is resumed by constitutive  $P_R$ -transcription of *cro*  
 $\langle 3/b/ii/CII.\{-,h\}+SOS+Cro.l/ll.9-15 - [PR\_tr] \rangle$ ,  
 $\langle 3/b/ii/CII.\{-,h\}+SOS+Cro.h/ll.13-15 - [PR\_tr] \rangle$ . See also  
0/.

The encountered divergences in the  
 $3/b/ii/\{CII.-,CII.h\}+SOS+Cro.h$  cases pertain to  
CI and Cro mediating contravariance. These effects undermine  
each other: there is a need for the conflicting state changes  
to not happen in order for each their mediated effect  
to be seen through. For CI, however, also SOS actively  
lowers the concentration and the correct CI resolution  
is to zero. If this happens quickly, CI loses its effect  
on Cro but Cro auto-contravariance will then take over  
 $\langle 3/b/ii/CII.\{-,h\}+SOS+Cro.h/l.7 - ![OR2\_Cro,OR1\_Cro] |-- [CI.1\dots] \rangle$   
and the correct divergence resolution is again downward. See  
also 3/c/ii/.

⟨Linearized coextension derivation: 3/b/ii/CII.\_+SOS+Cro.1⟩

```

1 [Cro.1, RecA.*] + [CI.0, CII._, DNA.ss]
2 -> [PR_tr] ; [SOS]
3 x> ![] |-- [DNA.ss]

5 [CI.1, Cro.1, RecA.*] + [CII._, DNA.ss]
6 -> ![OLR12_CI] ; [SOS]
7 x> ![] |-- [DNA.ss] ; [PR_tr] |-- [CI.1!@[OLR12]] ;
  [OLR12_CI, PR_tr] |-- [Cro.1@[OR3]]

9 [Cro.0, RecA.*] + [CI.0, CII._, DNA.ss]
10 -> [PR_tr] ; [SOS]
11 x> ![] |-- [DNA.ss]

13 [Cro.1, RecA.*] + [CI.0, CII._, DNA.ss]
14 -> [PR_tr] ; [SOS]
15 x> ![] |-- [DNA.ss]

```

⌈Visualization: 3/b/ii/CII.\_+SOS+Cro.1⌋

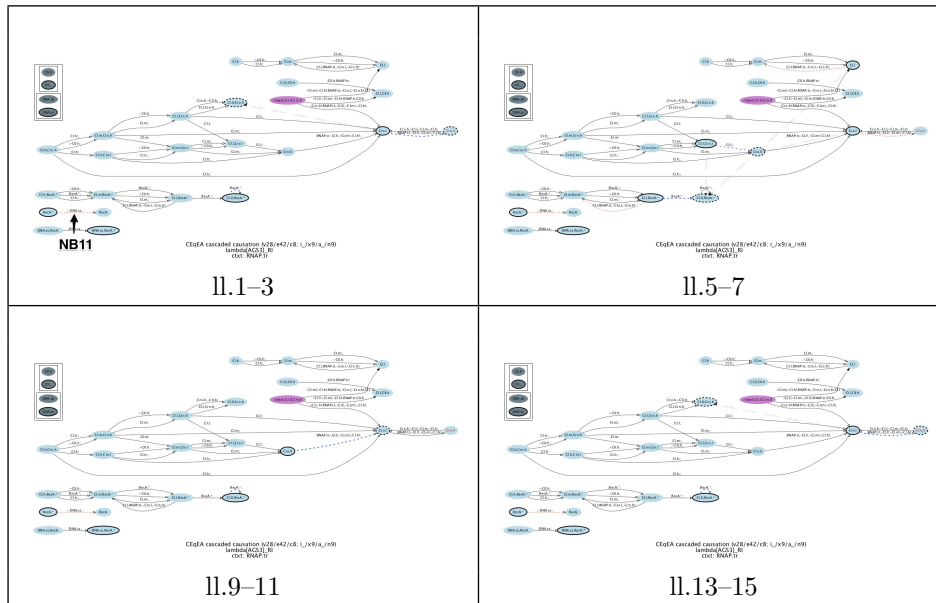

(Linearized coextension derivation: 3/b/ii/CII.\_+SOS+Cro.h)

```

1 [Cro.h, RecA.*] + [CI.0, CII._, DNA.ss]
2 -> ![OR2_Cro, OR1_Cro] ; [SOS]
3 x> ![[] |-- [DNA.ss]

5 [CI.1, Cro.h, RecA.*] + [CII._, DNA.ss]
6 -> ![OLR12_CI, OR3_Cro] ; ![OLR12_CI] ; [SOS] ;
  ![OR3_Cro]
7 x> ![[] |-- [DNA.ss] ; ![OR2_Cro, OR1_Cro] |--
  [CI.1@[OLR12]] ; [OLR12_CI, PRM_tr] |-- [Cro.h!@[OR3]]

9 <divergence>
10 [CI.0, CI.1, Cro.1, Cro.h]
11 * resolution required

13 [Cro.1, RecA.*] + [CI.0, CII._, DNA.ss]
14 -> [PR_tr] ; [SOS]
15 x> ![[] |-- [DNA.ss]

```

Visualization: 3/b/ii/CII.\_+SOS+Cro.h

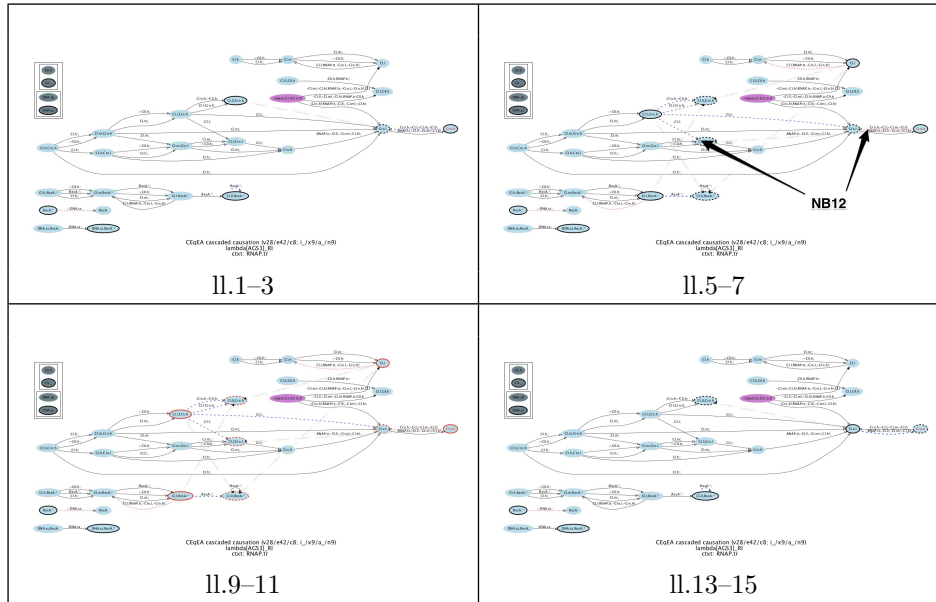

⟨Linearized coextension derivation: 3/b/ii/CII.h+SOS+Cro.1⟩

```

1 [CI.0, Cro.1, RecA.*] + [CII.h, DNA.ss]
2 -> [PR_tr] ; [SOS]
3 x> ![[] |-- [DNA.ss] ; [PRE_tr, ORE_CII] |-- [SOS]

5 [CI.1, Cro.1, RecA.*] + [CII.h, DNA.ss]
6 -> ![OLR12_CI] ; [SOS]
7 x> ![[] |-- [DNA.ss] ; [PR_tr] |-- [CI.1!@[OLR12]] ;
  [OLR12_CI, PRM_tr] |-- [Cro.1@[OR3]]

9 [CI.0, Cro.0, RecA.*] + [CII.h, DNA.ss]
10 -> [PR_tr] ; [SOS]
11 x> ![[] |-- [DNA.ss] ; [PRE_tr, ORE_CII] |-- [SOS]

13 [CI.0, Cro.1, RecA.*] + [CII.h, DNA.ss]
14 -> [PR_tr] ; [SOS]
15 x> ![[] |-- [DNA.ss] ; [PRE_tr, ORE_CII] |-- [SOS]

```

⌈Visualization: 3/b/ii/CII.h+SOS+Cro.1⌋

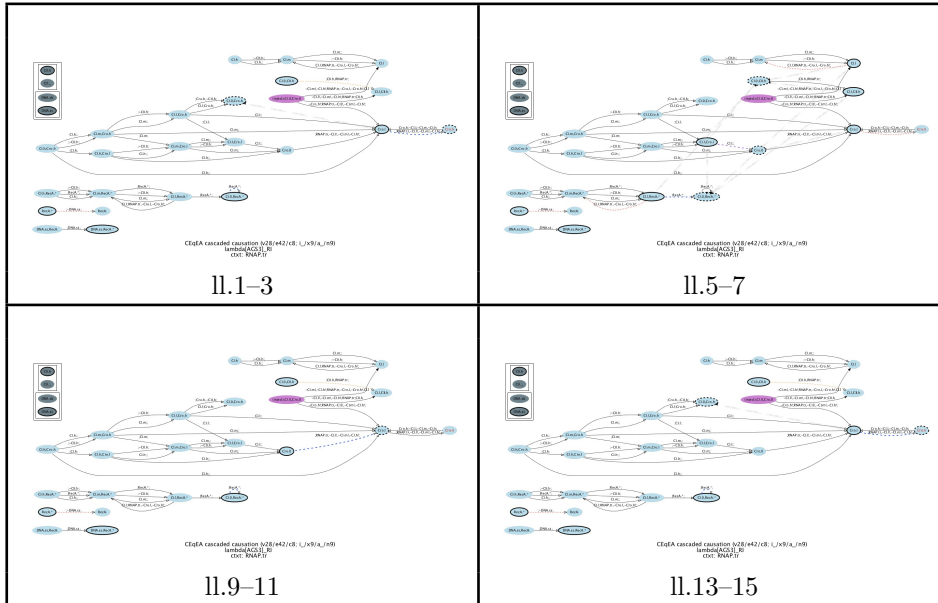

⟨Linearized coextension derivation: 3/b/ii/CII.h+SOS+Cro.h⟩

```

1 [CI.0, Cro.h, RecA.*] + [CII.h, DNA.ss]
2 -> ![OR2_Cro, OR1_Cro] ; [SOS]
3 x> ![ ] |-- [DNA.ss] ; [PRE_tr, ORE_CII] |-- [SOS]

5 [CI.1, Cro.h, RecA.*] + [CII.h, DNA.ss]
6 -> ![OLR12_CI, OR3_Cro] ; ![OLR12_CI] ; [SOS]
7 x> ![ ] |-- [DNA.ss] ; ![OR2_Cro, OR1_Cro] |--
  [CI.1@[OLR12]] ; ![OR3_Cro] |-- [CII.h] ; [OLR12_CI,
  PRM_tr] |-- [Cro.h!@[OR3]]

9 <divergence>
10 [CI.0, CI.1, Cro.1, Cro.h]
11 * resolution required

13 [CI.0, Cro.1, RecA.*] + [CII.h, DNA.ss]
14 -> [PR_tr] ; [SOS]
15 x> ![ ] |-- [DNA.ss] ; [PRE_tr, ORE_CII] |-- [SOS]

```

⌈Visualization: 3/b/ii/CII.h+SOS+Cro.h⌋

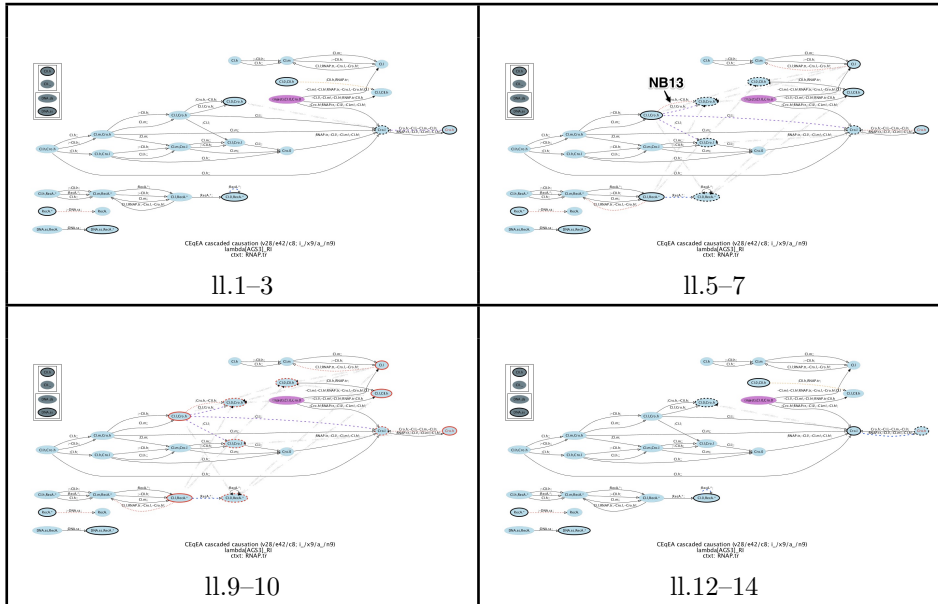

iii/ *super-infection*  $\neg\heartsuit$  or  $\spadesuit$  — an aspect of anti-immunity, see article:Retro.(V)

App.SC:[(92, Fig.4.23:1)]

WE ADDRESS THIS BY INTERACTIVELY ENABLING THE (INJECT) CHANNEL IN THE DISCRETE SCENARIOS OF A LYTIC ATTACK, SEE 3/A/ $\beta$ /, BUT WITHOUT USING CEQEA'S EXPIRATION MECHANISM, SEE 3/B/.

Owing to the specifics of 2/c/, we can assume that  $\neg\heartsuit$  means  $\text{SOS}+\text{CI}.0$ , meaning a compartment that includes  $\text{RecA}.*$ ,  $\text{CI}.0$ . We also need to consider the case of  $\spadesuit$ , meaning a compartment that includes  $\text{CII}.*$ ,  $\text{CI}.0$ . Because there is and can be no CI that can proteolyse in case of  $\text{CII}.*$ ,  $\text{CI}.0$ , the dynamics are not affected by  $\text{RecA}.*$  v  $\text{RecA}.*$ , and we case-split with just  $\text{CII}.*$  and  $\text{CII}.h+\text{SOS}$ : part of  $\neg\heartsuit$  is addressed in the first case (for  $\spadesuit$ ) and the remainder is addressed in the second.

- In case of  $\text{CII}.*$ , no (physiological) CI-expression/*cI*-transcription (from either  $\text{P}_{\text{RM}}$  or  $\text{P}_{\text{RE}}$ ) is possible  $\langle 3/b/iii/\text{CII}.*+\text{Cro}.1/l.1-15 \rangle$   $\langle 3/b/iii/\text{CII}.*+\text{Cro}.h/l.1-11 \rangle$  and the lytic attack continues unimpeded, i.e., as it would have without the super-infection, see 3/a/ $\beta$ /. In the case of super-infection at  $\text{Cro}.1$ , the prior and the super-infecting phage are (physiologically)  $\text{P}_{\text{R}}$ -transcribed  $\langle 3/b/iii/\text{CII}.*+\text{Cro}.1/l.6 \rangle$ . In the case of super-infection at  $\text{Cro}.h$ , the prior and the super-infecting phage are not (physiologically)  $\text{P}_{\text{R}}$ -transcribed  $\langle 3/b/iii/\text{CII}.*+\text{Cro}.h/l.7 \rangle$  because of inhibition by the  $\text{Cro}$  already present in the host.
- In case of  $\text{CII}.h+\text{SOS}$ , any  $\text{P}_{\text{RE}}$ -based CI-expression is coinhibited by the host  $\text{SOS}$  response, i.e., is countermanded by  $\text{RecA}.*$  mediated CI-autoproteolysis  $\langle 3/b/iii/\text{CII}.h+\text{SOS}+\text{Cro}.1,2,3,4,5,6,7,8,9,10,11 \rangle$ . Because of this, the case behaves as the  $\text{CII}.*$  case, i.e., any physiological effect  $\text{CII}.h$  would normally have is rendered irrelevant.

⟨Linearized coextension derivation: 3/b/iii/CII.\_+Cro.1⟩

```

1 [Cro.1] + [CI.0, CII._, DNA.ds, RecA.]
2 -> [PR_tr]
3 x>

5 [Cro.0, Cro.1] + [(inject), CI.0, CII._, DNA.ds, RecA.]
6 -> [PR_tr]
7 x>

9 [Cro.h] + [CI.0, CII._, DNA.ds, RecA.]
10 -> ![OR2_Cro, OR1_Cro]
11 x>

13 [Cro.1] + [CI.0, CII._, DNA.ds, RecA.]
14 -> [PR_tr]
15 x>

```

⌈Visualization: 3/b/iii/CII.\_+Cro.1⌋

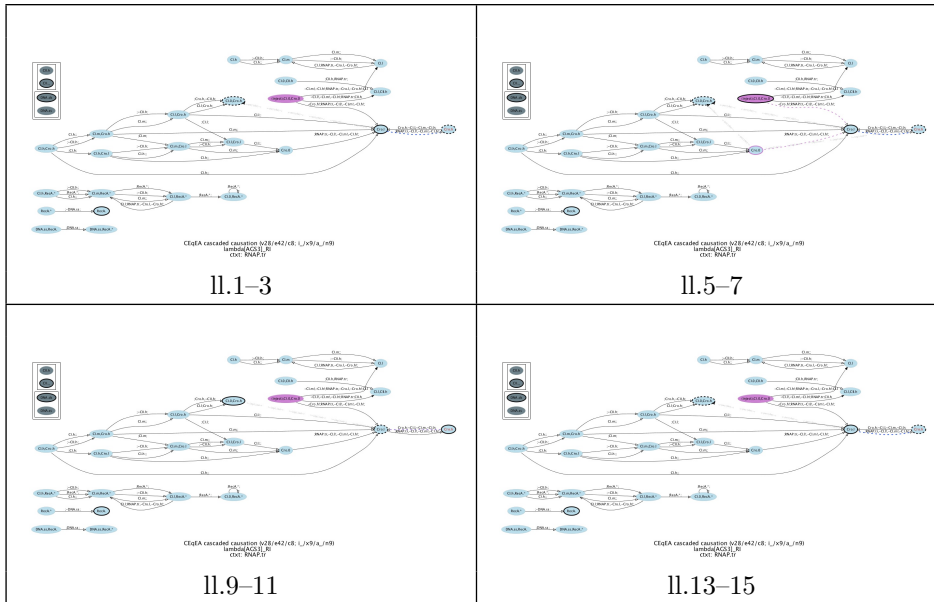

⟨Linearized coextension derivation: 3/b/iii/CII.\_+Cro.h⟩

```

1  [Cro.h] + [CI.0, CII.~, DNA.ds, RecA.]
2  ->  ![OR2_Cro, OR1_Cro]
3  x>

5  [Cro.0, Cro.h] + [(inject), CI.0, CII.~, DNA.ds, RecA.]
6  ->  ![OR2_Cro, OR1_Cro]
7  x>  [PR_tr] |-- [Cro.h!@[OR1, OR2]]

9  [Cro.1] + [CI.0, CII.~, DNA.ds, RecA.]
10 ->  [PR_tr]
11 x>

```

Visualization: 3/b/iii/CII.\_+Cro.h

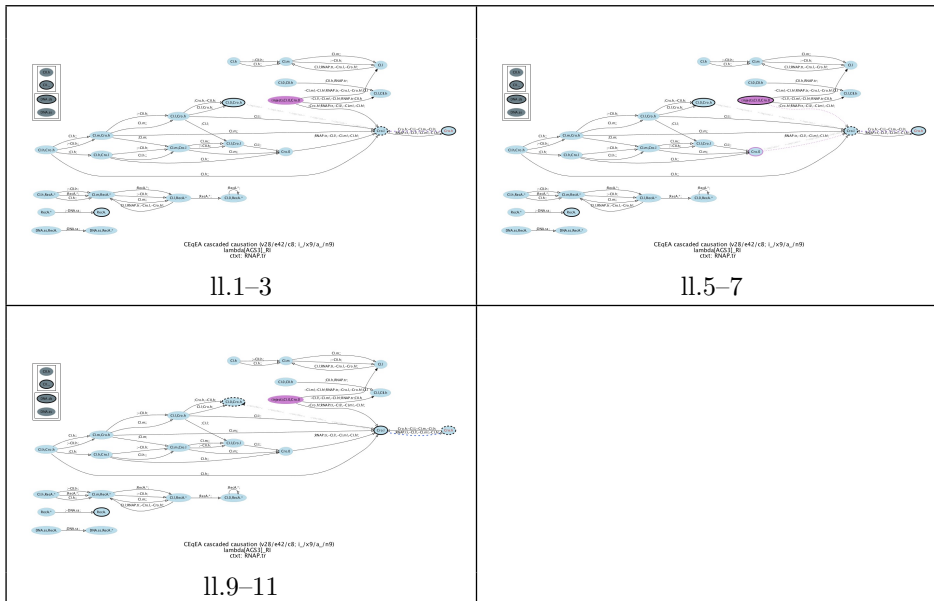

⟨Linearized coextension derivation: 3/b/iii/CII.h+SOS+Cro.1⟩

```

1 [CI.0, Cro.1, RecA.*] + [CII.h, DNA.ss]
2 -> [PR_tr] ; [SOS]
3 x> ![] |-- [DNA.ss] ; [PRE_tr, ORE_CII] |-- [SOS]

5 [CI.0, Cro.0, Cro.1, RecA.*] + [(inject), CII.h, DNA.ss]
6 -> [SOS] ; [PR_tr]
7 x> ![] |-- [DNA.ss] ; [PRE_tr, ORE_CII] |-- [SOS]

9 [CI.0, Cro.h, RecA.*] + [CII.h, DNA.ss]
10 -> ![OR2_Cro, OR1_Cro] ; [SOS]
11 x> ![] |-- [DNA.ss] ; [PRE_tr, ORE_CII] |-- [SOS]

```

⌈Visualization: 3/b/iii/CII.h+SOS+Cro.1⌋

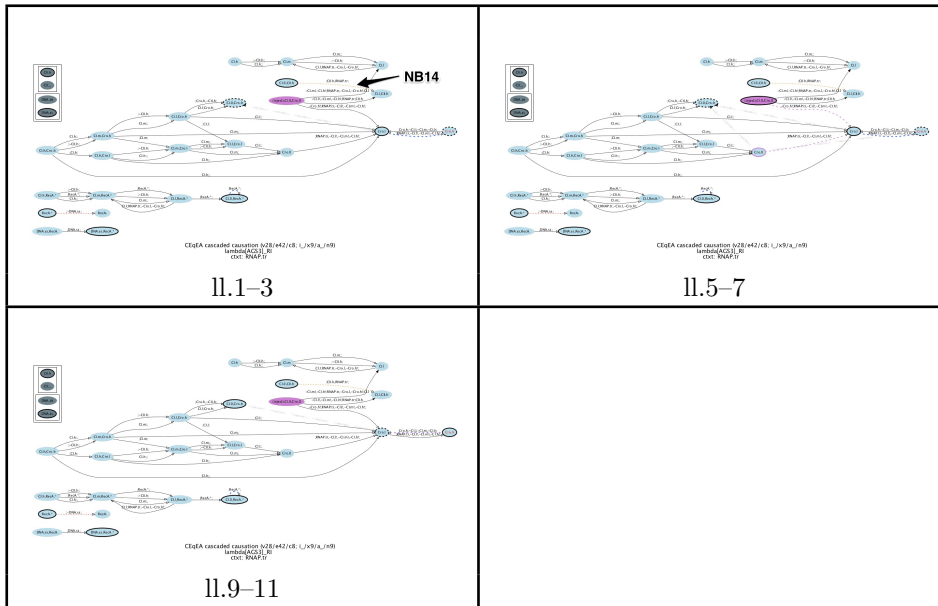

⟨Linearized coextension derivation: 3/b/iii/CII.h+SOS+Cro.h⟩

```

1  [CI.0, Cro.h, RecA.*] + [CII.h, DNA.ss]
2  -> ![OR2_Cro, OR1_Cro] ; [SOS]
3  x> ![[] |-- [DNA.ss] ; [PRE_tr, ORE_CII] |-- [SOS]

5  [CI.0, Cro.0, Cro.h, RecA.*] + [(inject), CII.h, DNA.ss]
6  -> ![OR2_Cro, OR1_Cro] ; [SOS]
7  x> ![[] |-- [DNA.ss] ; [PR_tr] |-- [Cro.h!@[OR1, OR2]] ;
    [PRE_tr, ORE_CII] |-- [SOS]

9  [CI.0, Cro.1, RecA.*] + [CII.h, DNA.ss]
10 -> [PR_tr] ; [SOS]
11 x> ![[] |-- [DNA.ss] ; [PRE_tr, ORE_CII] |-- [SOS]

```

⌈Visualization: 3/b/iii/CII.h+SOS+Cro.h⌋

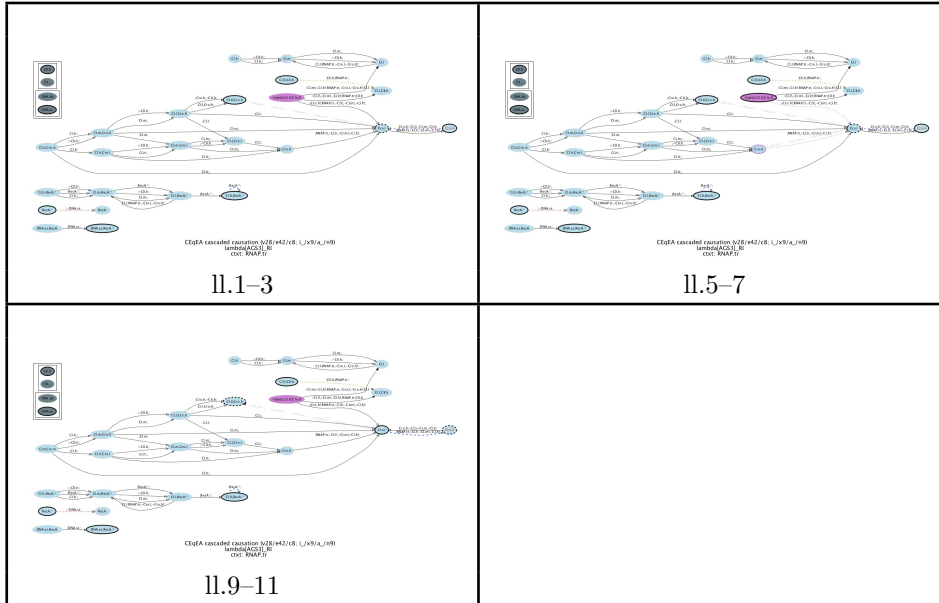

*c/ ignoring host expiration, a switch to lysogeny is likely to be effected by*

*ii/ CI-perturbation ♡ (and ♠ in order for the lytic attack to be viable, see 3/d/)*

App.SC:[(92, Fig.4.23:1)]

WE ADDRESS THIS BY INTERACTIVELY ENABLING THE “CI.L”  
NODE IN THE DISCRETE SCENARIOS OF A LYTIC ATTACK,  
SEE 3/A/ $\beta$ /, BUT WITHOUT USING CEQEA’S EXPIRATION  
MECHANISM, SEE 3/B/.

- In case of perturbation at **Cro.l**, **CI** and **Cro** are both at low concentration  $\langle 3/c/ii/CII._+Cro.l/1.5 \rangle$ , which leads to a lysogenic cycle, see 0/.
- In case of perturbation at **Cro.h**, we end up in a similar situation to the **Cro.h** cases of 3/b/ii/, except now there is no host SOS response to guarantee that the **CI** concentration drops. To recapitulate: **CI** and **Cro** both contravariantly inhibit each other  $\langle 3/c/ii/CII._+Cro.h/\{sync, async\}/1.6 \rangle$ , meaning both attempt to change each other downward but both effects diminish in a crossover fashion as this happens, i.e., both need to not change to see the other change through, hence the encountered divergences. If both change, the lytic cycle continues  $\langle 3/c/ii/CII._+Cro.h/sync/1.13 \rangle$ . If the highly-cooperative **CI** binding outlasts **Cro**’s non-cooperative binding, as might be expected seeing that **CI**’s binding is likely to outlast its free concentration, we see a switch to the lysogenic cycle  $\langle 3/c/ii/CII._+Cro.h/async/11.13-19 \rangle$ , see 0/.

⟨Linearized coextension derivation: 3/c/ii/CII.\_+Cro.1⟩

```

1 [Cro.1] + [CI.0, CII._, DNA.ds, RecA.]
2 -> [PR_tr]
3 x>

5 [CI.1, Cro.1] + [CII._, DNA.ds, RecA.]
6 -> ![OLR12_CI]
7 x> [PR_tr] |-- [CI.1!@[OLR12]] ; [OLR12_CI, PRM_tr] |--
    [Cro.1@[OR3]]

9 [CI.1, Cro.0] + [CII._, DNA.ds, RecA.]
10 -> [OLR12_CI, PRM_tr]
11 x> [PR_tr] |-- [CI.1!@[OLR12]]

```

⌈Visualization: 3/c/ii/CII.\_+Cro.1⌋

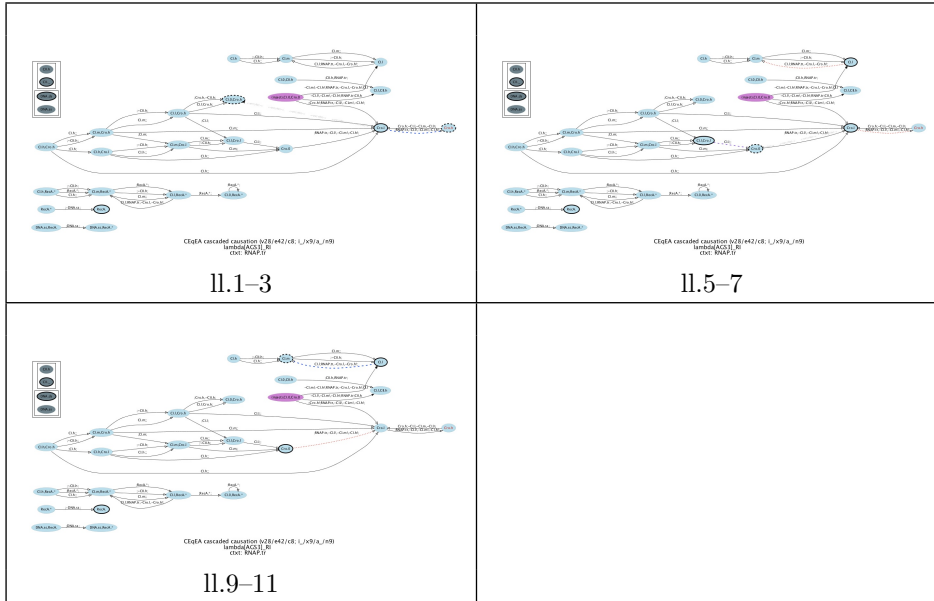

⟨Linearized coextension derivation: 3/c/ii/CII.\_+Cro.h/sync⟩

```

1  [Cro.h] + [CI.0, CII._, DNA.ds, RecA.]
2  -> ![OR2_Cro, OR1_Cro]
3  x>

5  [CI.1, Cro.h] + [CII._, DNA.ds, RecA.]
6  -> ![OLR12_CI] ; ![OLR12_CI, OR3_Cro] ; ![OR3_Cro]
7  x> ![OR2_Cro, OR1_Cro] |-- [CI.1@[OLR12]] ; [OLR12_CI,
    PRM_tr] |-- [Cro.h!@[OR3]]

9  <divergence>
10     [CI.0, CI.1, Cro.1, Cro.h]
11     * resolution required

13  [Cro.1] + [CI.0, CII._, DNA.ds, RecA.]
14  -> [PR_tr]
15  x>

```

⌈Visualization: 3/c/ii/CII.\_+Cro.h/sync⌋

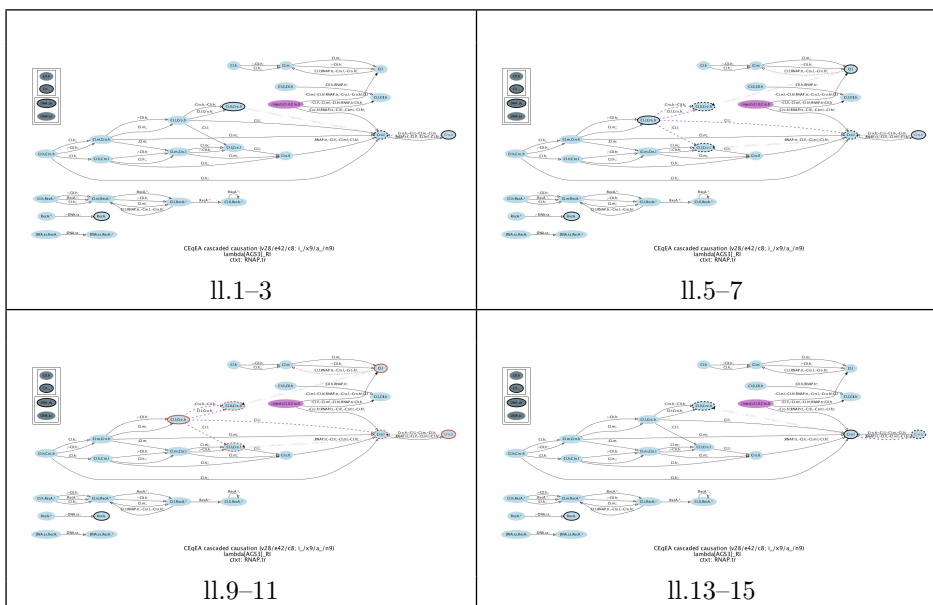

⟨Linearized coextension derivation: 3/c/ii/CII.\_+Cro.h/async⟩

---

```

1  [Cro.h] + [CI.0, CII._, DNA.ds, RecA.]
2  -> ![OR2_Cro, OR1_Cro]
3  x>

5  [CI.1, Cro.h] + [CII._, DNA.ds, RecA.]
6  -> ![OLR12_CI] ; ![OLR12_CI, OR3_Cro] ; ![OR3_Cro]
7  x> ![OR2_Cro, OR1_Cro] |-- [CI.1@[OLR12]] ; [OLR12_CI,
    PRM_tr] |-- [Cro.h!@[OR3]]

9  <divergence>
10     [CI.0, CI.1, Cro.1, Cro.h]
11     * resolution required

13 [CI.1, Cro.1] + [CII._, DNA.ds, RecA.]
14 -> ![OLR12_CI]
15 x> [PR_tr] |-- [CI.1!@[OLR12]] ; [OLR12_CI, PRM_tr] |--
    [Cro.1@[OR3]]

17 [CI.1, Cro.0] + [CII._, DNA.ds, RecA.]
18 -> [OLR12_CI, PRM_tr]
19 x> [PR_tr] |-- [CI.1!@[OLR12]]

```

d/ a lytic attack is unlikely  $\heartsuit$  and  $\neg\spadesuit$

App.SC:[12:10a, 15:Fig.1.5:2]

WE ADDRESS THIS PARTLY BY CONSIDERING A COEXTENSION STATE SPACE OVER **CI**, **CII**, **Cro**, **DNA.ds**, AND NOT OVER **RECA.\***, SEE  $\heartsuit$ .

(See comments at 2/a/ $\alpha$ /.)

The property requires us to rule out that **Cro** may go from below high to high concentration, see 3/a/ $\gamma$ /, in case of  $\neg\spadesuit$ , meaning with **CII** at high concentration or with **CI** at physiological concentration.

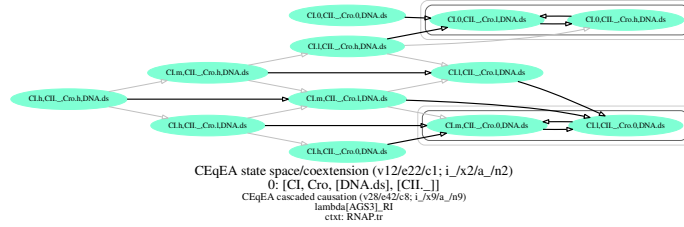

For the case of **CI** at physiological concentration, consider the co-extension state space above, where **CII** is below high concentration. Further to what needs to be shown, mentally discard the four nodes containing **Cro.h** (far left to upper right) as starting points of our analysis. By the specifics of the case, discard also the additional two nodes containing **CI.0** (top). The remaining six nodes (lower right) leave no room for an increase to the concentration of **Cro**, i.e., have no path to one of the discarded nodes containing **Cro.h**.

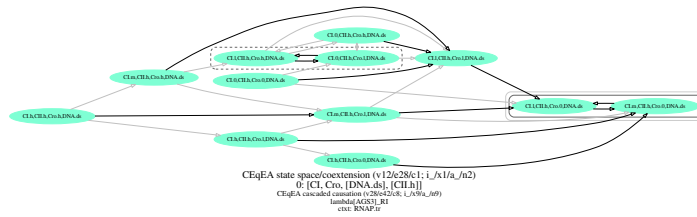

For the case of **CII** at high concentration, we need to consider the diagram above with only the four nodes containing **Cro.h** (upper left) discarded as starting points of our analysis — we have also removed their out- but not their in-edges:

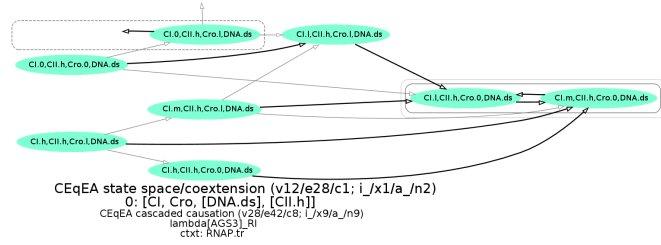

We see that, among the remaining nodes, **Cro.h** can be reached, i.e., a lytic attack can be effected, from “CI.0,CII.h,Cro.1,DNA.ds”. In turn, this node can be reached from the “CI.0,CII.h,Cro.0,DNA.ds” node. If, on fresh infection, **Cro** reaches physiological concentration ahead of **CI**, e.g., because **CII** is in the lower range of high concentration (which, in particular, means that the bold/fully-changing edge from the “CI.0,CII.h,Cro.0,DNA.ds” node to the “CI.1,CII.h,Cro.1,DNA.ds” node is not pursued), we will likely see a lytic attack. Otherwise, a lytic attack cannot happen, i.e., there is no other path to one of the discarded nodes containing **Cro.h**.

NB! In case we are considering a scenario in which host expiration does not take place, we can imagine that we are able to observe an infection that circles around the bold/fully-changing loop between the “CI.1,CII.h,Cro.h,DNA.ds” and “CI.0,CII.h,Cro.1,DNA.ds” nodes, whereby the concentrations of **CI** and **Cro** increase and decrease in lockstep. This loop has an interesting property: an almost complete lack of stability — see, e.g., the NB! in 3/b/i/. Even more interestingly, if either concentration change happens ahead of the other, i.e., if we pursue anything other than a bold/fully-changing edge, we are all but guaranteed to see a switch to the lysogenic cycle. In particular, in the “CI.0,CII.h,Cro.h,DNA.ds” node, the expected change, namely the bold/fully-changing edge, is to the “CI.1,CII.h,Cro.1,DNA.ds” node, which is guaranteed to lead to a lysogenic cycle, see 0/. What we see in the “CI.0,CII.h,Cro.h,DNA.ds” node is that **Cro.h** strongly inhibits  $P_R$ - and  $P_{RM}$ -transcription, but leaves  $cI$ -transcription from the downstream  $P_{RE}$  unaffected: the transcribing RNAP seemingly passes through the **Cro** bindings within the DNA, something which **CI** binding seemingly does not allow for, see Section S2.1. See also our discussion of ‘anti-immunity’ in article:Retrodiction (V).

### S2.3.3 Causation and coextensive-causation particulars

Details for annotations on reasoning visualizations over the  $\lambda^{\text{[AGS3]}}$  cascaded causation diagram:

⌈NB1 @ 0/CII.h/ll.5–7⌋ Proof-engine ( $\text{CCP}^{\text{all}}$ ) traversals of cascaded causation diagrams reflect more than just local effects of individual edges, and CeqEA transiently inserts edges that reveal any implied steps. For example, also the “CI.1,CII.h”-node will be abandoned as we pursue the activated edge from the “CI.1”-node to the “CI.m”-node considered here. ⌈NB7 @ 1/CII.h/ll.1–3⌋ illustrates the dual issue: implied targets.

⌈NB2 @ 1/CII.\_/ll.1–3⌋ When the magenta-coloured (**inject**) channel is enabled, also the blue-coloured “Cro.0” node is enabled, with magenta-coloured border (and out-edge). The magenta-coloured channel refers to a situation that was specified to represent a means of membrane traversal, with nodes with transient magenta colour boosting the incoming signal in cases of active out-edges: the application of standard intra-compartment regulatory machinery to the channel content. Unlike the pure intra-compartment part of the diagrams, the magenta-coloured part is subject to standard graph-traversal mechanics: when channels are used with an existing compartment, they must integrate themselves in one step, either naturally or through resolution of any created divergence. A booster need not be subject to the same regulatory mechanisms as the channel although that is the case here: only one collection of active domains is listed (1/CII.\_/l.2).

See ⌈NB3 @ 1/CII.\_/ll.1–3⌋, ⌈NB9 @ 2/b/iii/CII.\_+CI.1/ll.5–7⌋, and ⌈NB10 @ 2/b/iii/CII.h+CI.1/ll.5–7⌋ for further specifics of the treatment of inter-compartment channels and boosters.

⌈NB3 @ 1/CII.\_/ll.1–3⌋ Although there is an edge from the (**inject**) channel to the “CI.1” node in the causation diagram, it is not considered here. Technically, this is because the edge is subject to CeqEA’s TargetRequired condition, as indicated by the filled arrow head, see Section S1.4.1. TargetRequired edges can only be activated if both nodes are enabled, i.e., when all mediators are present. Activation of TargetRequired edges may, e.g., effect coinhibition on other edges and cannot be ignored. The edge in question pertains to  $P_{\text{RM}}$ -transcription, for which CI must be physiological in order to recruit RNAP. The fact that the listed CI.1 mediator occurs only on the target end of the edge is a direct consequence of the specified modalities and mediation characteristics for the (**inject**) channel: they express that any connected edge involves mixing of solutions in this particular sense. (See also ⌈NB9 @ 2/b/iii/CII.\_+CI.1/ll.5–7⌋.) In real-world terms, the TargetRequired condition for the considered edge captures the fact that an infecting phage may have its *cI*-gene transcribed by RNAP recruited to the  $P_{\text{RM}}$  site by CI that was produced by a prior infection, see [[28]:12:7]/App.SC.

⌈NB4 @ 1/CII.\_/ll.5–7⌋ Although no intra-node with CI.0 was enabled in the previous step, the state was *injected* into the considered compartment, is remembered as inert, and is available for node enabling until the schema-instance state is explicitly changed.

⌈NB5 @ 1/CII.\_/ll.9–11⌋ Further to Section S2.1, and as indicated by the red text in the “Cro.h”-node and the newly-overlaid graphics on the node, something happens the first time the node is enabled: a countdown timer is set (to 1), see 3/a/γ/ and ⌈NB6 @ 1/CII.\_/ll.13–17⌋.

⌈NB6 @ 1/CII.\_/ll.13–17⌋ The countdown timer in ⌈NB5 @ 1/CII.\_/ll.9–11⌋ is a kill-switch and the proof engine stops once it runs out: CEqEA indicates both expiration and cause, see 3/a/γ/.

⌈NB7 @ 1/CII.h/ll.1–3⌋ Further to ⌈NB1 @ 0/CII.h/ll.5–7⌋, CEqEA includes implied edges to certain nodes that are not targeted by activated edges. These are nodes that may be reached a) by virtue of being contained in nodes that *are* targeted, see the “CI.1”-node vs the “CI.1,CII.h”-node, or b) by being composed from multiple targeted nodes, see the “CI.1,Cro.1”-node vs the “CI.1,CII.h”- and “Cro.1”-nodes. These correspond to changes with more elaborate justifications than considered locally and the combined effects of multiple changes with distinct justifications, respectively.

⌈NB8 @ 1/CII.h/ll.13–15⌋ The indicated edge corresponds to  $x > ![] \mid \text{--} [CII.h]$ , which is 3f4:2 in Section S2.2.4, i.e., a passive-passive contravariant effect, see Section S2.2.3.

⌈NB9 @ 2/b/iii/CII.\_+CI.1/ll.5–7⌋ Coherence constraints do not apply in case of inter-compartment activity, i.e., no coherence test is made between nodes with and without magenta colour: a super-infecting phage, for example, arrives without any proteins of its own while earlier infections may have build up a physiological concentration. Any conflict this creates for what might happen next is addressed as part of the ensuing coextensive causation. No conflict is created in this case. (Note that absence of a conflict of this kind does not imply that the course of an ongoing pathway is not altered: a super-infection could coinhibit what would have been the next step of the pathway, for example.)

⌈NB10 @ 2/b/iii/CII.h+CI.1/ll.5–7⌋ For the cases with CII at high concentration not just P<sub>R</sub>-transcription of *cro* but also P<sub>RE</sub>-transcription of *cI* on the super-infecting phage is blocked by inhibition  $\langle 2/b/iii/CII.h+CI.1/1.7 \text{ --- } [PRE\_tr \ \& \ ORE\_CII] \mid \text{--} [CI.1!...] \rangle$ . This may be surprising because the P<sub>RE</sub>-edge from the “CI.0,CII.h”-node carries no visible inhibitors and the P<sub>RE</sub>-edge from the (inject) channel to the “CI.1,CII.h”-node carries only visible inhibitors in the source node where the relevant schema instance is explicitly in a non-inhibiting state. This is a case of CEqEA invoking

its notion of *latent inhibition*. The edges are specified to be inhibited by (physiological) CI bound to  $O_{\{L,R\}}\{1,2\}$ . In normal circumstances, i.e., for intra-compartment activity, the inhibition is not relevant because we are starting from a situation with non-physiological CI, and CEqEA suppresses the (seemingly) vacuous inhibition information. Without suppression as a general mechanism, CEqEA would infer incorrect observable concentrations and life cycles, see Section S1.5. Suppression applies to schema instances that are specified as being coherent, i.e., schema instances that can be in only one state at a time, but coherence does not apply in case of inter-compartment activity, see `⌈NB9 @ 2/b/iii/CII._+CI.1/ll.5-7⌋`. In CEqEA, inhibitors that are suppressed for coherence reasons are retained, as *latent inhibitors*, and are called upon when the node that the edge in question departs from has been enabled as an inter-compartment channel or booster but not when it has been enabled for intra-compartment reasons. (Latent inhibitors can be listed by pressing `CTRL+SHIFT+1` in a visualized cascaded causation diagram.)

`⌈NB11 @ 3/b/ii/CII._+SOS+Cro.1/ll.1-3⌋` The indicated edge corresponds to `x> ![[] |-- [DNA.ss]`, which is **1a1:1** in Section S2.2.4, i.e., a passive contravariant effect.

`⌈NB12 @ 3/b/ii/CII._+SOS+Cro.h/ll.5-7⌋` The indicated blocked edge corresponds to `x> ![OR2_Cro, OR1_Cro] |-- [CI.1@[OLR12]]`, which is **4a1:1** in Section S2.2.4: an active contravariant effect that has retained a nested inhibition. The deeper inhibitor expresses the preferential binding of a long-distance octamer over the natural dimer used by the blocked edge. The preferred binding is also indicated, as active: **4b3:1** in Section S2.2.4

`⌈NB13 @ 3/b/ii/CII.h+SOS+Cro.h/ll.5-7⌋` The indicated edge corresponds to `x> ![OR3_Cro] |-- [CII.h]`, which is **3d2:3** in Section S2.2.4, i.e., a passive-active contravariant effect with nested inhibition to express a preferential effect: contravariance associated with inhibition at one promoter is null and void if other promoters are used.

`⌈NB14 @ 3/b/iii/CII.h+SOS+Cro.1/ll.1-3⌋` Coinhibition of  $P_{RE}$ -based CI-expression by the host SOS response: the latter countermands the former, thereby preventing a switch.

## S2.4 A sequentialized Genetic Switch: the $\lambda^{[AGS3]}$ synchrotype

We show that [28]:Fig.1.2, which is hand-drawn and based on observation:

SUPPRESSED

hides inside the  $\lambda^{[AGS3]}$  cascaded causation diagram, Figure 5, under  $CCP^{all}$ , see Section S1.5:

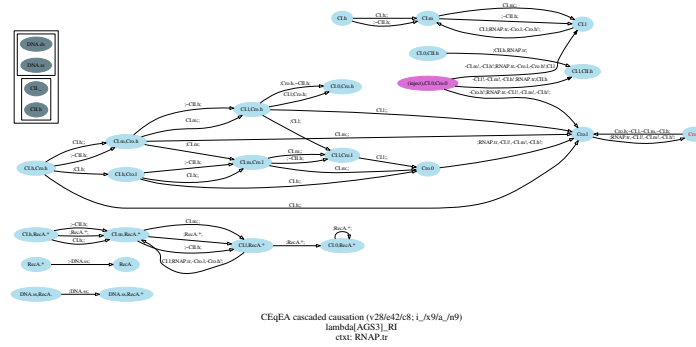

### S2.4.1 The right physiology

We are interested in how the  $\lambda$ -only causations may become synchronized to each other under environmental influences. When working with cascaded causation diagrams in Section S2.3, we simply toggled the environment parts we were interested in and relied on  $CCP^{all}$  to get both positive and negative conditions right. This approach does not (yet) work for synchrotype prediction, see below. Instead, the first thing we do here is to silence the host by commenting out host-related influences from the  $\lambda^{[AGS3]}$  genotype:

```
/*cytosol*/
//+ !      | $proteinC / RecA | @UV_irr ;
//-        | $proteinC / CI   | ^@SOS   | ceaseless ;
```

In this case, we get a cascaded causation diagram that is a sub-graph of the  $\lambda^{[AGS3]}$  diagram — sustained equilibria: the boxes, have been added to prepare for sequentialization, see Section S1.5:

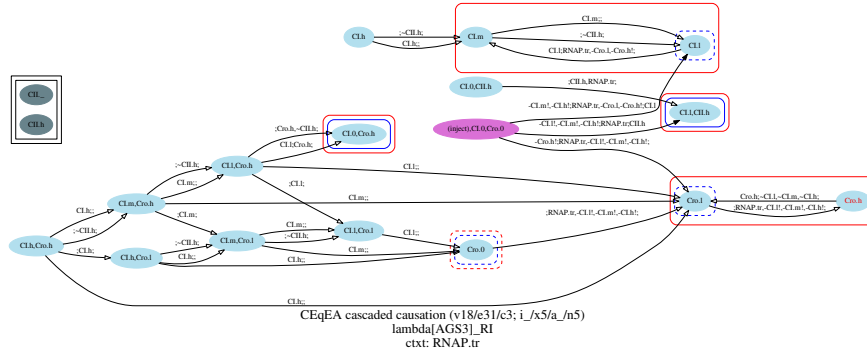

### S2.4.2 Environmental specialization

By adding the **ExogenyInference** directive, CEqEA will specialize this diagram for the various combinations of a state from each of the toggable schema instances (here CII):

```

/*****
/*--- CEqEA directives ---*/
/*****

ExogenyInference ;

```

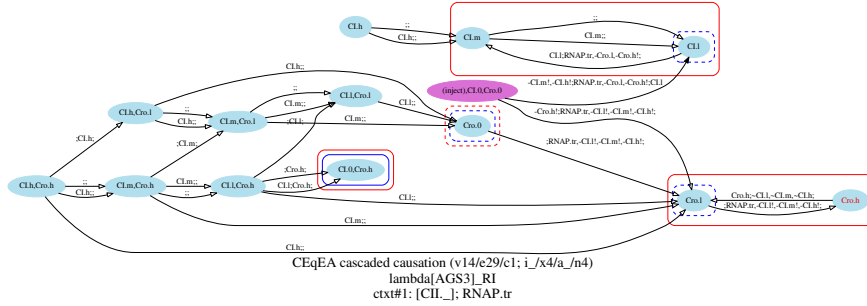

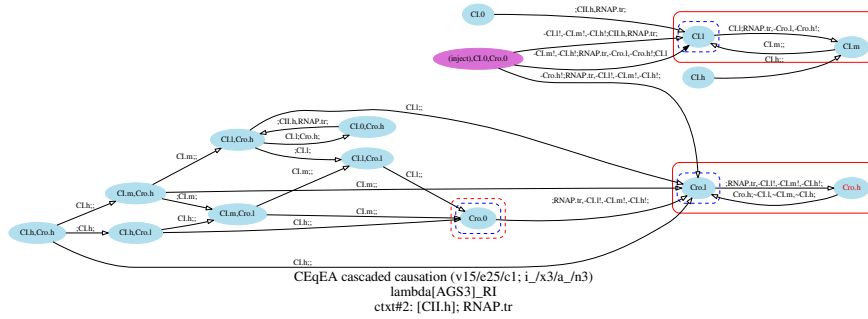

Now we can see the trouble with synchrotyping specific cell types from a more general account. While the top of these graphs, specialized to  $\text{CII.}_-$ , is more or less a sub-graph of the preceding graph (except  $\text{CII.h}$ -inhibition is omitted), the bottom one, specialized to  $\text{CII.h}$ , is not: a box is missing. The issue is that  $\text{CII.h}$  used to be a differential positive condition for  $\text{CI}$ -expression from  $\text{P}_{\text{RE}}$ , see the “ $\text{CI.}\{0,1\}, \text{CII.h}$ ” edge in the non-specialized diagram. With  $\text{CII.h}$  always present, its presence is no longer an explicit condition. This means that we include its effect as an edge from the “ $\text{CI.0}, \text{Cro.h}$ ” node to the “ $\text{CI.1}, \text{Cro.h}$ ” node in the bottom diagram. Conversely, in a coextensive traversal of the non-specialized diagram with  $\text{CII.h}$  in the compartment, an enabled “ $\text{CI.0}, \text{Cro.h}$ ” node would be subject to the same change except as a non-local step back to the “ $\text{CI.1}, \text{Cro.h}$ ” node because the “ $\text{CI.}\{0,1\}, \text{CII.h}$ ” edge will be running.

### S2.4.3 The $\lambda^{\text{[AGS3]}}$ synchrotype

Without improvements to the definition of coexistable equilibria, we can still do synchrotype prediction provided we restrict the considered specification to just the causations we are interested in and, then, have CEqEA combinatorially specialize the specific organism under any environmental influences, as above, in order to consider different cell types separately, see Figure 7:

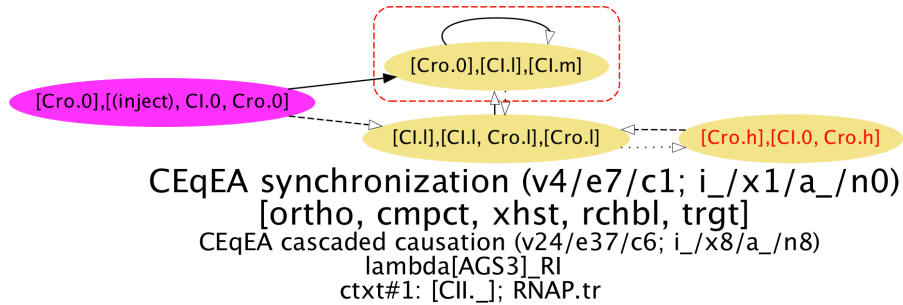

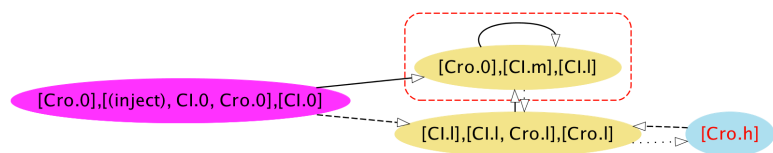

CEqEA synchronization (v4/e7/c1; i\_/x1/a\_/n0)  
 [ortho, cmpct, xhst, rchbl, trgt]  
 CEqEA cascaded causation (v25/e32/c6; i\_/x7/a\_/n7)  
 lambda[AGS3]\_RI  
 ctxt#2: [CII.h]; RNAP.tr

The system-expiring “Cro.h” node is not part of a synchronization point in the CII.h case (bottom) but is included as-is because it is reachable in the base diagram. The non-synchronization reflects the facts that the lytic attack is not systems-level sustainable, see Section S2.3:3/c/, and that the lytic attack is unlikely to be observed in the presence of CII.h., see Section S2.3:3/d/.

## S2.5 A first-principle Genetic Switch: the $\lambda^{[AGS3]}$ combinator

In addition to the wild-type reasoning we addressed in Section S2.3, Ptashne [28] includes *counterfactual* reasoning: arguments saying that if the considered premises were different, the inferences would be different in specific ways. This can, e.g., be used to argue against certain possibilities for a genotype if relevant parts of the phenotype are known or explain why some individuals behave differently than the norm.

### Non-wild phenotypes:

- *$\lambda$ virulent*: always lysis, whether fresh or super-infection, including overriding the  $\lambda$ -immunity of wild-type prophages [28]<sup>pp.68–69,85</sup>.
- *$\lambda$ clear*: always lysis on fresh infection; respects wild-type  $\lambda$ -immunity [28]<sup>p.68</sup>.
- *$\lambda$ anti-immune*: sustained lytic attack absent host lysis; channels wild-type super-infections towards their own lytic attack [28]<sup>p.92</sup>.

### Non-wild genotypes:

- no-*cI*/lesioned-*cI*: always  *$\lambda$ clear* [28]<sup>pp.62,68,72</sup>.
- lesioned-*cII*: typically  *$\lambda$ clear* [28]<sup>p.68</sup>.
- $P_{RM}UP-1$ : recruitment-free  $P_{RM}$ ; no operator change [28]<sup>Fig.4.17,Tab.4.4</sup>.
- $P_{RM}116$ : inactive  $P_{RM}$ ; no operator change [28]<sup>Fig.4.17</sup>.
- no Cro versus no Cro+CI binding at  $O_R3$  (superseded) [28]<sup>p.95</sup>.
- overlapping promoters: RNAP at  $P_R$  preventing RNAP at  $P_{RM}$  [28]<sup>p.103</sup>.
- $OR2^-$  [28]<sup>p.103</sup>.
- $\lambda O_R^{323}$ , aka  $\lambda 323$ , and its decomposition [28]<sup>pp.133–</sup>.
- ‘just-so’ evolution of the  $\lambda$ -switch [28]<sup>pp.134–135</sup>.

### S2.5.1 Examples

We briefly revisit two counterfactual cases from Ptashne [28] to illustrate how mutations work formally.

**No CI-octamer enabled CI-tetramer: weakening 2/c/** The inclusion of 0LR123\_CI in Section S2.1: long-distance binding of a CI tetramer at  $O_{\{L,R\}}3$  mediated by a CI octamer at  $O_{\{L,R\}}\{1,2\}$ , reflects a recent discovery that justified the 3rd edition [28]. At a lecture at Rockefeller University at the time of [28]’s release, Ptashne called it “a scandal” that modellers had not noted that the earlier understanding could not be correct. To illustrate, we null-and-void the macro:

|            |   |   |
|------------|---|---|
| @OLR123_CI | = | ; |
|------------|---|---|

Ptashne's argument is that, in retrospect, no octamer+tetramer will result in CI reaching higher than wild-type observable concentrations. On face value, the emitted cascaded causation diagram appears to support the argument:

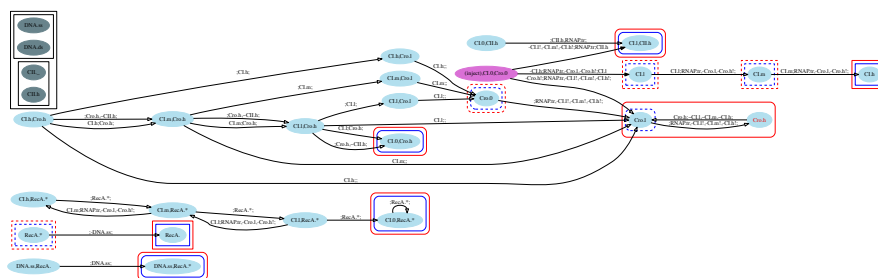

The expectation would be that the corresponding organism would be more difficult to induce than wild-type  $\lambda$ . Indeed, with CEqEA’s proof engine, the switch is now thrown in three steps instead of one to two for  $\lambda^{\text{[AGS3]}}$ , see Section S2.3:2/c/. The change in our predictions matches existing observations:

**[[28]:114:10]** (counterfactual):

SUPPRESSED

**Weak CI-inhibition of *cro*-transcription: breaking 0/** The  $\lambda^{\text{[AGS3]}}$  genotype states that CI has a strong inhibiting effect on *cro*-transcription due to cooperative binding. Here, we consider the possibility that the effect is weak, instead. We specify this by using the **approximative** modality value (in place of **incidental**): the inhibition is not sufficiently strong to guarantee that Cro is maintained at physiologically-zero concentration, see article:Retrodiction (I).

```
@PR_tr      = RNAP.tr
              /*& no recruiter*/
              |-- @OR1xor2_Cro
                : @OR1xor2_Cro +- !
                : @OR1and2_Cro -- !
                : @OR1xor2_CI
                : @OR1xor2_CI +- !
                : @OR1and2_CI -- !
                : @OLR12?_CI_rng ! {|apprx}
                :
```

This variant fails our novel Section S2.3.0/: the conflict between **CI.1** and **Cro.1** is not resolved, and the predicted phenotype is entirely different than the wild-type case.

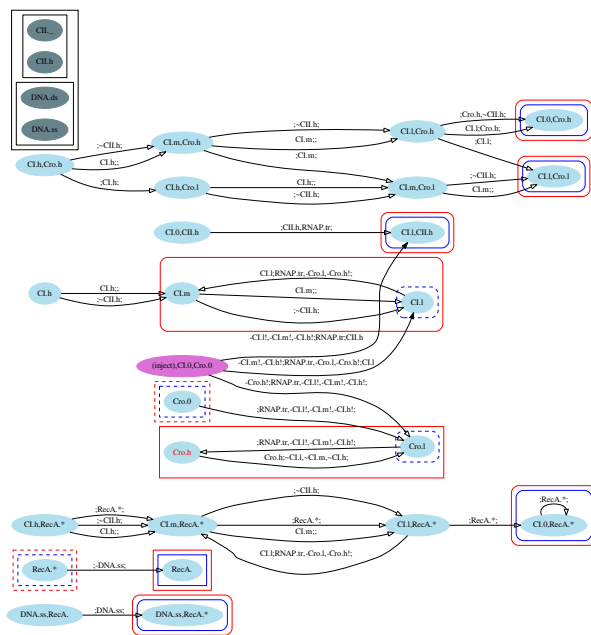

### S2.5.2 Abstracting $\lambda^{[AGS3]}$

We now address more than individual counterfactual arguments. Although not pursued in Ptashne [28], the scenarios are, e.g.,:

[[28]:85:F4.17:1] (counterfactual):

SUPPRESSED

Our  $\lambda^{[AGS3]}$  combinator is a MIG-specification schema that allows for variation in the kind of basic information described in the quotation: different transposed concentrations to match different intrinsic affinities for the operators. Our objective is to account for all consequences these changes may have on the molecular programming within MIG syntax: to program beyond individual organisms. Here, we must principally account for alternate-pairwise binding:

[[28]:21:-2] (counterfactual):

SUPPRESSED

Due to CI's higher affinity for O<sub>R</sub>1 than O<sub>R</sub>3 in the wild type, alternate-pairwise binding has not been directly relevant so far and the  $\lambda^{[AGS3]}$  genotype makes no reference to the possibility:

```
58  /*****  
59  /* @macro      = regulatory binding [precedence] ; */  
60  /***/  
  
62  /*CI cooperative binding*/  
63  @OLR123_CI      = (+) @OR3_CI_int ;                //[112:9]  
64  @OLR12_CI       = (+) @OR1_CI_int excl @OLR123_CI-- ;  
        //[86:F4.18][110:-4]%subsumed  
  
66  @OLR12?_CI_rng<> = @OLR123_CI-- : @OLR12_CI-- ;    //abbreviation
```

Ptashne [28] is not clear on all the general binding and behavioral issues we consider, and our modeling is based partly on surmises and should be considered provisional.

**Possible intrinsic affinities** The  $\lambda^{[AGS3]}$  combinator, see Section S2.5.8, includes one more active CI state and Cro state than does  $\lambda^{[AGS3]}$ , for a total of  $4^3 * 3^3 = 1,728$  possible  $\lambda$ -variants:

```

20 /*****
21 /* $level/schema . $level/states [| modalities] ; */
22 /*****/

35 /*regulated components: lambda*/
36 $genomeI / cI . $proteinC / [ 0 {l} {m} {h} {x} ] ;
37 $genomeI / cro . $proteinC / [ 0 {l} {h} {x} ] ;

```

The two new extra-high states represent the possibility of mutations that weaken the proteins' operator affinities beyond the weakest already found in the wild type. The below  $\square$ s are extra-MIG notation that indicate places that will be combinatorially instantiated by a simple script:

```

40 /*****
41 /* @macro<>      = transposed interface ; */
42 /*****/

44 @OR1_CI_int<>    = CI.  $\square$  ;
45 @OR2_CI_int<>    = CI.  $\square$  ;
46 @OR3_CI_int<>    = CI.  $\square$  ;

48 @OR1_Cro_int<>   = Cro.  $\square$  ;
49 @OR2_Cro_int<>   = Cro.  $\square$  ;
50 @OR3_Cro_int<>   = Cro.  $\square$  ;

```

In what follows, we list only the specific changes we make to the  $\lambda^{[AGS3]}$  genotype, see Section S2.1. Other than using more general macro names, the changes involve cooperative affinities and binding only.

**Cooperativity macros** For our more general scenario where we cannot rely on a particular ordering of CI’s affinities, we first specify how short- and long-distance CI oligomers may form:

```

57 /*cooperative affinities*/
58 @OR12_CI_tetra<> = (+) min&(@OR1_CI_int,@OR2_CI_int) ;
59 @OR23_CI_tetra<> = (+) min&(@OR2_CI_int,@OR3_CI_int) ;

61 @OLR12_CI_octa<> = max&(/*OL12*/(+)CI.l,@OR12_CI_tetra) ;
62 @OLR123_CI_octTtr<> = max&(@OLR12_CI_octa, (+)
    min&(/*OL3*/CI.h,@OR3_CI_int)) ;

```

The tetramerizations are cooperative. One dimer: `min_...`, binds and attaches a second dimer to the other location, with the two stabilizing each other to lower: `(+)`, the effective concentration at which the combined binding will be physiological, see Section S2.1. Both bindings must be possible: `&`, for the tetramerization to be possible.

For the long-distance-cooperativity case, the  $O_L$  side is not being mutated and its bindings will be physiological as before, see Section S2.1 and [[28]:86:15] combined with [[28]:121:box:4]/App.SC.

[[28]:86:15] (incidental):

SUPPRESSED

Octamerization and octamerization followed by tetramerization are only indirectly cooperative: the operator bindings are independent of each other and must both be in effect: `max_...`. For octamerization, tetramers at  $O_L$  and  $O_R$  attract so strongly that they supercoil the DNA across a few thousand base pairs (without lowering the effective affinity). For octamerization+tetramerization, the tetramer forms across a correctly-sized gap created by the DNA-supercoiling octamer but the tetramer and octamer do not make contact (no lowering). We do not name a `@OLR3_CI_tetra` macro to ensure a pre-existing octamer effects the requisite DNA-supercoiling: we surmise that a long-distance tetramer does not form by itself on  $O_{\{L,R\}3}$ .

For physiological bindings, we proceed by cases. First, the wild-type ordering of affinities:

```

69 /*cooperative binding*/
70 cond( @OR1_CI_int << @OR3_CI_int )
71   @OLR123_CI = @OLR123_CI_octTtr ;
72   @O?R12_CI = @OR12_CI_tetra   excl @OLR123_CI-- ;
    //subsume
73   @O?R23_CI = @OR23_CI_tetra   excl @OLR123_CI-- : @O?R12_CI-- ;
    //preclude
74 endcond;

```

The octamer-mediated tetramer: `@OLR123_CI`, is physiological as defined intrinsically. The `@O?R12_CI` macro is defined to ensure we do not act on the assumption of a simpler binding when the binding is likely to be octamer+tetramer. The `@O?R23_CI` macro reflects that the alternate-pairwise binding favors the other side. For the last two macros, we surmise that long-distance cooperativity

need not be in effect: they are based on @OR macros.

In case CI binds more readily to O<sub>R</sub>3 than to O<sub>R</sub>1, the pre-octamer tetramer forms on O<sub>R</sub>{2,3}. We specify that this **excludes** the other two cooperation configurations due to layout. More, we surmise that, following octamerization with @OR23\_CI, the free sites that are brought together by DNA-supercoiling: O<sub>R</sub>1 and O<sub>L</sub>3, will be non-adjacent and unable to bind a third tetramer, leaving @OLR123\_CI null-and-void by definition:

```

69 /*cooperative binding*/
75 cond( @OR1_CI_int >> @OR3_CI_int )
76   @O?R23_CI = @OR23_CI_tetra ;
77   @OLR123_CI = ;// excl @O?R23_CI-- ;
78   //preclude
79   @O?R12_CI = @OR12_CI_tetra excl @O?R23_CI-- : @OLR123_CI-- ;
   //preclude:subsume
endcond;

```

@O?R12\_CI is disfavoured here by a mix of the reasons for the octamer-only cases above.

In case the affinities of CI for O<sub>R</sub>1 and O<sub>R</sub>3 are comparable, either binding may happen and we cannot just rule one out. We also cannot allow for precluding bindings to have simultaneous effects. CEqEA provides a **MutualExclude** construct in the MIG language for this eventuality, which we need to use in place of the **exclusions** we called **preclude** above: the modeling logic carries through. The effects of **MutualExclude** are to not allow any changes by **MutualExcluded** mediations and to suppress an inhibitor if a **MutualExcluded** mediator is used. The latter will typically result in the possibility of CCP<sup>all</sup> divergences: the stochastic choice between **MutualExcluded** bindings gets promoted to the level of CPP<sup>all</sup> traversals.

```

69 /*cooperative binding*/
80 cond( @OR1_CI_int == @OR3_CI_int )
81   @OLR123_CI = @OLR123_CI_octTtr ;
82   @O?R12_CI = @OR12_CI_tetra excl @OLR123_CI-- ;
83   //subsume
84   @O?R23_CI = @OR23_CI_tetra ;
85   MutualExclude ( @O?R23_CI, @O?R12_CI ) ;
86   //stochastic
87   MutualExclude ( @O?R23_CI, @OLR123_CI ) ;
88   //stochastic
endcond;

```

Like for  $\lambda^{[AGS3]}$ , see Section S2.1, we wish to have abbreviations for when the underlying operators are involved in some cooperative binding:

```

88 /*cooperative occupancy*/
89 @O?R12?_CI_rng<> = @OLR123_CI-- : @O?R12_CI-- ;
90 @O?R?23_CI_rng<> = @OLR123_CI-- : @O?R23_CI-- ;
91 @O?R?2?_CI_rng<> = @OLR123_CI-- : @O?R12_CI-- : @O?R23_CI-- ;

```

**Cooperative regulation** For the dimer-only bindings, the abbreviations are used as expected:

```

65  /*****
66  /* @macro      = regulatory binding [precedence] ; */
67  *****/

94  /*OR1*/
95  @OR1_CI      = @OR1_CI_int    excl @0?R12?_CI_rng ;
96  @OR1_Cro     = @OR1_Cro_int   |--  @0?R12?_CI_rng ;

98  /*OR2*/
99  @OR2_CI      = @OR2_CI_int    excl @0?R?2?_CI_rng ;
100 @OR2_Cro     = @OR2_Cro_int   |--  @0?R?2?_CI_rng ;

102 /*OR3*/
103 @OR3_CI      = @OR3_CI_int    excl @0?R?23_CI_rng ;
104 @OR3_Cro     = @OR3_Cro_int   |--  @0?R?23_CI_rng ;

```

For the remainder of the combinator, the new abbreviations refine the earlier macros, see Section S2.5.8:  $P_{RE}$  is cooperatively inhibited in case of any cooperative CI binding,  $P_{RM}$  is cooperatively inhibited if  $O_{R3}$  is involved, and  $P_R$  is cooperatively inhibited if  $O_{R2}$  is involved.

**Wild-type  $\lambda$ :  $lhh/hhl$**  The wild-type variant is the  $lhh/hhl$  genotype, where the letters represent the states substituted in for the  $\square$ s in order. Other than the added states, the cascaded causation diagram is unchanged from the RI version (confirm by adding  $\{x\}$ s to the latter):

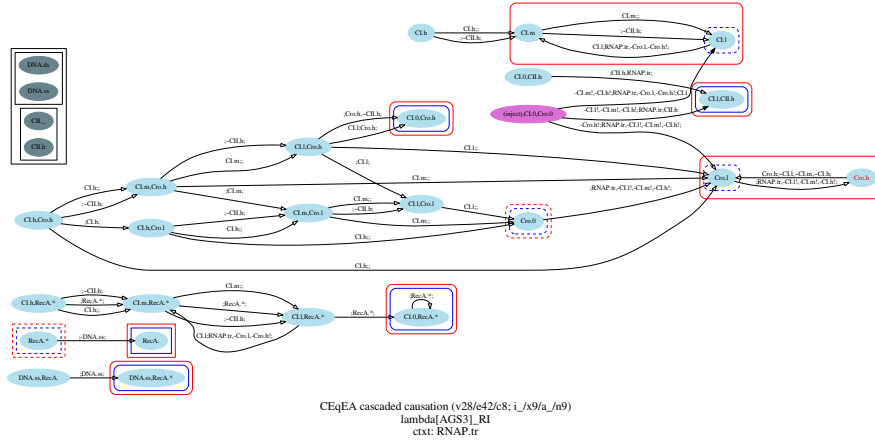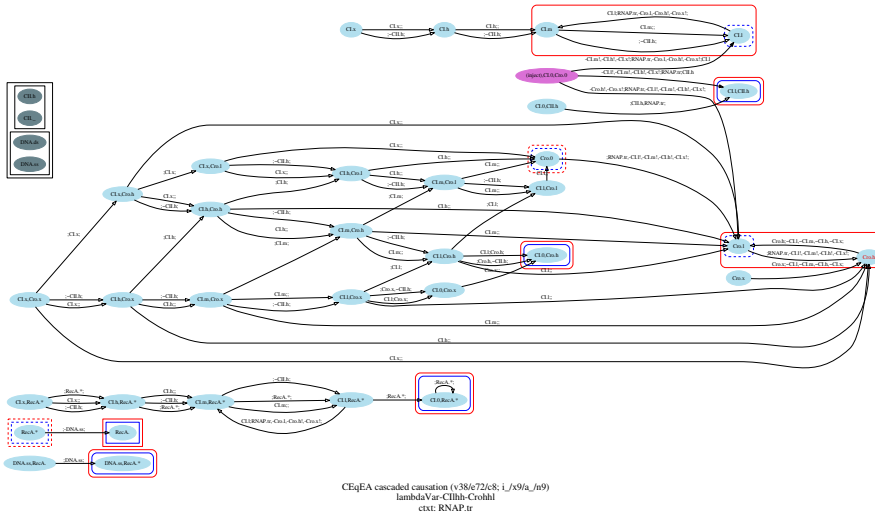

### S2.5.3 Rapid phenotyping

Our development of the  $\lambda^{\text{[AGS3]}}$  phenotype in Section S2.3 was designed to explore the valid argumentation from the given premises. Here, we use an assessment scheme that is intended to test outcomes without concern for the underlying argumentation: to be first-principle modeling, see Proposition 9. The tests are designed to be rapidly applicable across all  $\lambda$ -variants and for the results to enable phenotype classification. For the wild type:

| genotype | $[-]_{\perp}^{\succ}$ | $[h]_{\perp}^{\succ}$ | $[-]_{1_0}^{\vee}$ | $[-]_{m_0}^{\vee}$ | $x_0^{\succ}$ | $(x_0^{\succ})_+^{\succ}$ | $(x_0^{\succ})_{UV}^{\succ}$ | $0_x^{\succ}$  | #v/e/c/x/n  |
|----------|-----------------------|-----------------------|--------------------|--------------------|---------------|---------------------------|------------------------------|----------------|-------------|
| lhh/hhl  | $\otimes$             | $\{m, 1\}_0$          | $1_0$              | $m_0$              | $\{m, 1\}_0$  | $\parallel$               | $\otimes$                    | $0_{\{h, 1\}}$ | 38/72/8/9/9 |

We use  $[-]$  or  $[h]$  to refer to injection with CII. $_{\perp}$  or CII. $_h$  in the start compartment;  $_{\perp}$  to refer to absence of a prior infection (absence of node selection as opposed to selection of nodes with 0 states);  $a_b$  to refer to CI in state a and Cro in state b;  $^{\succ}$  to refer to automated CCP<sup>all</sup> traversals;  $^{\vee}$  to refer to “worst-case” traversals: selective use of running edges (only);  $\otimes$  to refer to expiration; and  $\parallel$  for ditto (relative to the local context).

$[-]_{\perp}^{\succ}$ ,  $[h]_{\perp}^{\succ}$  are for the outcomes, under automated CCP<sup>all</sup> traversal, of freshly enabling the **inject** node with CII below or at high concentration, i.e., with “CII. $_{\perp}$ ” or “CII. $_h$ ” toggled. This is used to distinguish temperate vs virulent and clear variants. Because *cro* transcription is constitutive,  $[-]_{\perp}^{\succ}$  also reveals Cro’s trajectory during a purported lytic attack.

$[-]_{1_0}^{\vee}$ ,  $[-]_{m_0}^{\vee}$  address whether a lytic attack may happen from a super-infection, specifically whether the variant respects  $\lambda$ -immunity. This is used to distinguish virulent vs clear variants. To be clear, we are considering the case where the super-infection is with the variant at hand while the prophage is wild type. Even though we work with just one diagram, that of the variant, we can still simulate the prior infection’s physiological CI-levels: we simply enable the variant’s “CI.1” or “CI.m” nodes and see how far we can raise Cro’s state by manually following running edges and if we can trigger expiration: CI is CI, no matter the source.

$x_0^{\succ}$  is for the outcome, under automated CCP<sup>all</sup> traversal, of freshly enabling the “CI.x” and “Cro.0” nodes. This is used to test if the variant is able to exhibit a lysogenic cycle in and of itself, and to determine the specifics.

$(x_0^{\succ})_+^{\succ}$  is for the outcome, under automated CCP<sup>all</sup> traversal, of perturbing Cro, i.e., of interactively increasing the state of Cro, in any non-trivial  $x_0^{\succ}$  outcome. This is used to test if any exhibited lysogenic cycles are homeostatic.

$(x_0^{\succ})_{UV}^{\succ}$  is for the outcome, under automated CCP<sup>all</sup> traversal, of UV-irradiating any non-trivial  $x_0^{\succ}$  outcome. This is used to test if a lysogen is inducible.

$0_x^>$  is for the outcome, under automated CCP<sup>all</sup> traversal, of starting from a compartment with **CI.0,Cro.x** and with CEqEA's expiration facility turned off. The test adds lysis-relevant information but is designed to establish a property we discuss in Section S2.5.6.

**#v/e/c/x/n** records stats about the cascaded causation diagrams: number of vertices (nodes), edges, weakly-connected components, max equilibria, and min equilibria.

We will use  $\{\mathfrak{m}, \mathfrak{l}\}_0; \otimes$ , to mean that **CI** may loop between its  $\mathfrak{m}$  and  $\mathfrak{l}$  states while keeping **Cro** in its 0 state but also that **CI** may irreversibly (;) change to the next state beyond  $\mathfrak{l}$  (0), in which case expiration ( $\otimes$ ) is inescapable. This implies the presence of a stochastic choice/divergence: the concentration of **CI** may go up or down in  $\mathfrak{l}_0$  depending on the possible bindings. In effect,  $\mathfrak{ll}$  is used to mean homeostasis while we use  $\mathfrak{ll}; \mathfrak{l}_1 \succ \otimes$  to mean homeostasis except that perturbation to  $\mathfrak{l}_1$  results in expiration. In the tables below, we use no entry to mean “not applicable”. Lastly, e.g.,  $\otimes_{\mathfrak{h}}$  means expiration with **Cro** in state  $\mathfrak{h}$  ( $\otimes$  is the wild-type:  $\otimes_1$ ).

## S2.5.4 CI-binding variants: lambdaVar-CI□□□-Crohhl.mig

| genotype      | $[-]_{\perp}^{\perp}$ | $[h]_{\perp}^{\perp}$ | $[-]_{1_0}^{\vee}$ | $[-]_{m_0}^{\vee}$ | $x_0^{\perp}$ | $(x_0^{\perp})_{+}^{\perp}$ | $(x_0^{\perp})_{UV}^{\perp}$ | $0_x^{\perp}$ | #v/e/c/x/n   |
|---------------|-----------------------|-----------------------|--------------------|--------------------|---------------|-----------------------------|------------------------------|---------------|--------------|
| lll/hhl       | $\otimes$             | $0_0, 1_1$            | $1_0$              | $m_0$              | $\otimes$     |                             |                              | $0_{\{h,1\}}$ | 37/107/9/8/8 |
| llm/hhl       | $\otimes$             | $0_0, 1_1$            | $1_0$              | $m_0$              | $\otimes$     |                             |                              | $0_{\{h,1\}}$ | 37/69/9/8/8  |
| llh/hhl       | $\otimes$             | $\{m, 1\}_0$          | $1_0$              | $m_0$              | $\{m, 1\}_0$  | $\parallel$                 | $\otimes$                    | $0_{\{h,1\}}$ | 38/72/8/9/9  |
| llx/hhl       | $\otimes$             | $\{m, 1\}_0$          | $1_0$              | $m_0$              | $\{m, 1\}_0$  | $\parallel$                 | $\otimes$                    | $0_{\{h,1\}}$ | 38/72/8/9/9  |
| lml/hhl       | $\otimes$             | $0_0, 1_1$            | $1_0$              | $m_0$              | $\otimes$     |                             |                              | $0_{\{h,1\}}$ | 37/107/9/8/8 |
| lmm/hhl       | $\otimes$             | $0_0, 1_1$            | $1_0$              | $m_0$              | $\otimes$     |                             |                              | $0_{\{h,1\}}$ | 37/69/9/8/8  |
| lmh/hhl       | $\otimes$             | $\{m, 1\}_0$          | $1_0$              | $m_0$              | $\{m, 1\}_0$  | $\parallel$                 | $\otimes$                    | $0_{\{h,1\}}$ | 38/72/8/9/9  |
| lmx/hhl       | $\otimes$             | $\{m, 1\}_0$          | $1_0$              | $m_0$              | $\{m, 1\}_0$  | $\parallel$                 | $\otimes$                    | $0_{\{h,1\}}$ | 38/72/8/9/9  |
| lhl/hhl       | $\otimes$             | $0_0, 1_1$            | $1_0$              | $m_0$              | $\otimes$     |                             |                              | $0_{\{h,1\}}$ | 37/107/9/8/8 |
| lhm/hhl       | $\otimes$             | $0_0, 1_1$            | $1_0$              | $m_0$              | $\otimes$     |                             |                              | $0_{\{h,1\}}$ | 37/69/9/8/8  |
| lhh/hhl       | $\otimes$             | $\{m, 1\}_0$          | $1_0$              | $m_0$              | $\{m, 1\}_0$  | $\parallel$                 | $\otimes$                    | $0_{\{h,1\}}$ | 38/72/8/9/9  |
| lhx/hhl       | $\otimes$             | $\{m, 1\}_0$          | $1_0$              | $m_0$              | $\{m, 1\}_0$  | $\parallel$                 | $\otimes$                    | $0_{\{h,1\}}$ | 38/72/8/9/9  |
| lxl/hhl       | $\otimes$             | $0_0, 1_1$            | $1_0$              | $m_0$              | $\otimes$     |                             |                              | $0_{\{h,1\}}$ | 37/107/9/8/8 |
| lxm/hhl       | $\otimes$             | $0_0, 1_1$            | $1_0$              | $m_0$              | $\otimes$     |                             |                              | $0_{\{h,1\}}$ | 37/69/9/8/8  |
| lxh/hhl       | $\otimes$             | $\{m, 1\}_0$          | $1_0$              | $m_0$              | $\{m, 1\}_0$  | $\parallel$                 | $\otimes$                    | $0_{\{h,1\}}$ | 38/72/8/9/9  |
| lxx/hhl       | $\otimes$             | $\{m, 1\}_0$          | $1_0$              | $m_0$              | $\{m, 1\}_0$  | $\parallel$                 | $\otimes$                    | $0_{\{h,1\}}$ | 38/72/8/9/9  |
| mlh/hhl       | $\otimes$             | $0_0, 1_1$            | $1_0$              | $m_0$              | $\otimes$     |                             |                              | $0_{\{h,1\}}$ | 39/87/9/9/9  |
| mlm/hhl       | $\otimes$             | $0_0, 1_1$            | $1_0$              | $m_0$              | $\otimes$     |                             |                              | $0_{\{h,1\}}$ | 37/107/9/8/8 |
| mlh/hhl       | $\otimes$             | $\{m, 1\}_0$          | $1_0$              | $m_0$              | $\{m, 1\}_0$  | $\parallel$                 | $\otimes$                    | $0_{\{h,1\}}$ | 38/72/8/9/9  |
| mlx/hhl       | $\otimes$             | $\{m, 1\}_0$          | $1_0$              | $m_0$              | $\{m, 1\}_0$  | $\parallel$                 | $\otimes$                    | $0_{\{h,1\}}$ | 38/72/8/9/9  |
| mml/hhl       | $\otimes$             | $0_0, 1_1$            | $1_0$              | $m_0$              | $\otimes$     |                             |                              | $0_{\{h,1\}}$ | 39/87/9/9/9  |
| mmm/hhl       | $\otimes$             | $0_0, 1_1$            | $1_0$              | $m_0$              | $\otimes$     |                             |                              | $0_{\{h,1\}}$ | 37/107/9/8/8 |
| mmh/hhl       | $\otimes$             | $\{m, 1\}_0$          | $1_0$              | $m_0$              | $\{m, 1\}_0$  | $\parallel$                 | $\otimes$                    | $0_{\{h,1\}}$ | 38/72/8/9/9  |
| mmx/hhl       | $\otimes$             | $\{m, 1\}_0$          | $1_0$              | $m_0$              | $\{m, 1\}_0$  | $\parallel$                 | $\otimes$                    | $0_{\{h,1\}}$ | 38/72/8/9/9  |
| mhl/hhl       | $\otimes$             | $0_0, 1_1$            | $1_0$              | $m_0$              | $\otimes$     |                             |                              | $0_{\{h,1\}}$ | 39/87/9/9/9  |
| mhm/hhl       | $\otimes$             | $0_0, 1_1$            | $1_0$              | $m_0$              | $\otimes$     |                             |                              | $0_{\{h,1\}}$ | 37/107/9/8/8 |
| mhh/hhl       | $\otimes$             | $\{m, 1\}_0$          | $1_0$              | $m_0$              | $\{m, 1\}_0$  | $\parallel$                 | $\otimes$                    | $0_{\{h,1\}}$ | 38/72/8/9/9  |
| mhx/hhl       | $\otimes$             | $\{m, 1\}_0$          | $1_0$              | $m_0$              | $\{m, 1\}_0$  | $\parallel$                 | $\otimes$                    | $0_{\{h,1\}}$ | 38/72/8/9/9  |
| mxl/hhl       | $\otimes$             | $0_0, 1_1$            | $1_0$              | $m_0$              | $\otimes$     |                             |                              | $0_{\{h,1\}}$ | 39/87/9/9/9  |
| mxm/hhl       | $\otimes$             | $0_0, 1_1$            | $1_0$              | $m_0$              | $\otimes$     |                             |                              | $0_{\{h,1\}}$ | 37/107/9/8/8 |
| mxx/hhl       | $\otimes$             | $\{m, 1\}_0$          | $1_0$              | $m_0$              | $\{m, 1\}_0$  | $\parallel$                 | $\otimes$                    | $0_{\{h,1\}}$ | 38/72/8/9/9  |
| mxx/hhl       | $\otimes$             | $\{m, 1\}_0$          | $1_0$              | $m_0$              | $\{m, 1\}_0$  | $\parallel$                 | $\otimes$                    | $0_{\{h,1\}}$ | 38/72/8/9/9  |
| continuing... |                       |                       |                    |                    |               |                             |                              |               |              |

lambdaVar-CI□□□-Crohhl.mig

| genotype      | $[-]_{-}^{\gamma}$ | $[h]_{-}^{\gamma}$ | $[-]_{10}^{\gamma}$ | $[-]_{m0}^{\gamma}$ | $x_0^{\gamma}$        | $(x_0^{\gamma})_{+}^{\gamma}$ | $(x_0^{\gamma})_{UV}^{\gamma}$ | $0_x^{\gamma}$ | #v/e/c/x/n   |
|---------------|--------------------|--------------------|---------------------|---------------------|-----------------------|-------------------------------|--------------------------------|----------------|--------------|
| ... continued |                    |                    |                     |                     |                       |                               |                                |                |              |
| hll/hhl       | $\otimes$          | $0_0, 1_1$         | $1_0$               | $m_0$               | $\otimes$             |                               |                                | $0_{\{h,1\}}$  | 38/81/9/9/9  |
| hlm/hhl       | $\otimes$          | $0_0, 1_1$         | $1_0$               | $m_0$               | $\otimes$             |                               |                                | $0_{\{h,1\}}$  | 38/81/9/9/9  |
| hlh/hhl       | $\otimes$          | $0_0, 1_1$         | $1_0$               | $m_0$               | $\{m, 1\}_0; \otimes$ | $  ; 1_1 \succ \otimes$       | $\otimes$                      | $0_{\{h,1\}}$  | 39/110/8/9/9 |
| hlx/hhl       | $\otimes$          | $\{m, 1\}_0$       | $1_0$               | $m_0$               | $\{m, 1\}_0$          | $  $                          | $\otimes$                      | $0_{\{h,1\}}$  | 38/72/8/9/9  |
| hml/hhl       | $\otimes$          | $0_0, 1_1$         | $1_0$               | $m_0$               | $\otimes$             |                               |                                | $0_{\{h,1\}}$  | 38/81/9/9/9  |
| hmm/hhl       | $\otimes$          | $0_0, 1_1$         | $1_0$               | $m_0$               | $\otimes$             |                               |                                | $0_{\{h,1\}}$  | 38/81/9/9/9  |
| hmb/hhl       | $\otimes$          | $0_0, 1_1$         | $1_0$               | $m_0$               | $\{m, 1\}_0; \otimes$ | $  ; 1_1 \succ \otimes$       | $\otimes$                      | $0_{\{h,1\}}$  | 39/110/8/9/9 |
| hmx/hhl       | $\otimes$          | $\{m, 1\}_0$       | $1_0$               | $m_0$               | $\{m, 1\}_0$          | $  $                          | $\otimes$                      | $0_{\{h,1\}}$  | 38/72/8/9/9  |
| hhl/hhl       | $\otimes$          | $0_0, 1_1$         | $1_0$               | $m_0$               | $\otimes$             |                               |                                | $0_{\{h,1\}}$  | 38/81/9/9/9  |
| hhm/hhl       | $\otimes$          | $0_0, 1_1$         | $1_0$               | $m_0$               | $\otimes$             |                               |                                | $0_{\{h,1\}}$  | 38/81/9/9/9  |
| hhh/hhl       | $\otimes$          | $\otimes$          | $\otimes$           | $m_0$               | $\otimes$             |                               |                                | $0_{\{h,1\}}$  | 35/85/9/8/8  |
| hhx/hhl       | $\otimes$          | $\otimes$          | $\otimes$           | $m_0$               | $\otimes$             |                               |                                | $0_{\{h,1\}}$  | 35/57/9/8/8  |
| hxl/hhl       | $\otimes$          | $0_0, 1_1$         | $1_0$               | $m_0$               | $\otimes$             |                               |                                | $0_{\{h,1\}}$  | 38/81/9/9/9  |
| hxm/hhl       | $\otimes$          | $0_0, 1_1$         | $1_0$               | $m_0$               | $\otimes$             |                               |                                | $0_{\{h,1\}}$  | 38/81/9/9/9  |
| hxx/hhl       | $\otimes$          | $\otimes$          | $\otimes$           | $m_0$               | $\otimes$             |                               |                                | $0_{\{h,1\}}$  | 35/85/9/8/8  |
| hxx/hhl       | $\otimes$          | $\otimes$          | $\otimes$           | $m_0$               | $\otimes$             |                               |                                | $0_{\{h,1\}}$  | 35/57/9/8/8  |
| xll/hhl       | $\otimes$          | $0_0, 1_1$         | $1_0$               | $m_0$               | $\otimes$             |                               |                                | $0_{\{h,1\}}$  | 37/77/9/8/8  |
| xlm/hhl       | $\otimes$          | $0_0, 1_1$         | $1_0$               | $m_0$               | $\otimes$             |                               |                                | $0_{\{h,1\}}$  | 37/77/9/8/8  |
| xlh/hhl       | $\otimes$          | $0_0, 1_1$         | $1_0$               | $m_0$               | $\otimes$             |                               |                                | $0_{\{h,1\}}$  | 37/77/9/8/8  |
| xlx/hhl       | $\otimes$          | $0_0, 1_1$         | $1_0$               | $m_0$               | $\{m, 1\}_0; \otimes$ | $  ; 1_1 \succ \otimes$       | $\otimes$                      | $0_{\{h,1\}}$  | 39/110/8/9/9 |
| xml/hhl       | $\otimes$          | $0_0, 1_1$         | $1_0$               | $m_0$               | $\otimes$             |                               |                                | $0_{\{h,1\}}$  | 37/77/9/8/8  |
| xmm/hhl       | $\otimes$          | $0_0, 1_1$         | $1_0$               | $m_0$               | $\otimes$             |                               |                                | $0_{\{h,1\}}$  | 37/77/9/8/8  |
| xmh/hhl       | $\otimes$          | $0_0, 1_1$         | $1_0$               | $m_0$               | $\otimes$             |                               |                                | $0_{\{h,1\}}$  | 37/77/9/8/8  |
| xmx/hhl       | $\otimes$          | $0_0, 1_1$         | $1_0$               | $m_0$               | $\{m, 1\}_0; \otimes$ | $  ; 1_1 \succ \otimes$       | $\otimes$                      | $0_{\{h,1\}}$  | 39/110/8/9/9 |
| xhl/hhl       | $\otimes$          | $0_0, 1_1$         | $1_0$               | $m_0$               | $\otimes$             |                               |                                | $0_{\{h,1\}}$  | 37/77/9/8/8  |
| xhm/hhl       | $\otimes$          | $0_0, 1_1$         | $1_0$               | $m_0$               | $\otimes$             |                               |                                | $0_{\{h,1\}}$  | 37/77/9/8/8  |
| xhh/hhl       | $\otimes$          | $\otimes$          | $\otimes$           | $m_0$               | $\otimes$             |                               |                                | $0_{\{h,1\}}$  | 35/63/9/8/8  |
| xhx/hhl       | $\otimes$          | $\otimes$          | $\otimes$           | $m_0$               | $\otimes$             |                               |                                | $0_{\{h,1\}}$  | 35/85/9/8/8  |
| xxl/hhl       | $\otimes$          | $0_0, 1_1$         | $1_0$               | $m_0$               | $\otimes$             |                               |                                | $0_{\{h,1\}}$  | 37/77/9/8/8  |
| xxm/hhl       | $\otimes$          | $0_0, 1_1$         | $1_0$               | $m_0$               | $\otimes$             |                               |                                | $0_{\{h,1\}}$  | 37/77/9/8/8  |
| xxh/hhl       | $\otimes$          | $\otimes$          | $\otimes$           | $m_0$               | $\otimes$             |                               |                                | $0_{\{h,1\}}$  | 35/63/9/8/8  |
| xxx/hhl       | $\otimes$          | $\otimes$          | $\otimes$           | $\otimes$           | $\otimes$             |                               |                                | $0_{\{h,1\}}$  | 33/63/9/8/8  |

lambdaVar-CI□□□-Crohhl.mig

An overlapping range of the known phenotypes are being exhibited in silico, see Figure 9:

| phenotype classification                                           | $[-]_{\sim}$ | $[h]_{\sim}$ | $[-]_{10}^{\vee}$ | $[-]_{m0}^{\vee}$ | $x_0^{\vee}$          | $(x_0^{\vee})_+^{\vee}$ | $(x_0^{\vee})_{UV}^{\vee}$ |
|--------------------------------------------------------------------|--------------|--------------|-------------------|-------------------|-----------------------|-------------------------|----------------------------|
| <span style="color: red;">■</span> $\lambda virulent$              | $\otimes$    | $\otimes$    | $\otimes$         | $\otimes$         | $\otimes$             |                         |                            |
| <span style="color: red;">■</span> $\lambda virulent/clear^+$      | $\otimes$    | $\otimes$    | $\otimes$         | $m_0$             | $\otimes$             |                         |                            |
| $\lambda clear^+$                                                  | $\otimes$    | $\otimes$    | $1_0$             | $m_0$             |                       |                         |                            |
| <span style="color: orange;">■</span> $\lambda clear^-$            | $\otimes$    | $0_0, 1_1$   | $1_0$             | $m_0$             | $\otimes$             |                         |                            |
| <span style="color: orange;">■</span> $\lambda temperate; clear^-$ | $\otimes$    | $0_0, 1_1$   | $1_0$             | $m_0$             | $\{m, 1\}_0; \otimes$ | $1_1; \otimes$          | $\otimes$                  |
| <span style="color: green;">■</span> $\lambda temperate$           | $\otimes$    | $\{m, 1\}_0$ | $1_0$             | $m_0$             | $\{m, 1\}_0$          | $\parallel$             | $\otimes$                  |

The difference between  $\lambda clear^+$  and  $\lambda clear^-$  is that the former is the unequivocal  $\lambda clear$  phenotype while the latter must wait for any CI-establishing CII concentration to dilute before its lytic attack commences. None of the considered variants exhibit the  $\lambda clear^+$  phenotype while the  $\lambda clear^-$  phenotype is the most common (genotypes not listed), see [[28]:68:13] below.

The fate of the  $\lambda virulent/clear^+$  phenotype depends on the level of CI maintained by a wild-type prophage but will probably manifest as  $\lambda virulent$  ex silico, as only one needs succeed. It is exhibited by  $\{hhh, hxx, xhh, xxh, hxx, hxx, xhx\}/hhl$ . The pure  $\lambda virulent$  phenotype is exhibited by  $xxx/hhl$ .

The  $\lambda temperate$  phenotype is exhibited by the wild type:  $lhh/hhl$ , and the  $\{llh, llx, lmh, lmx, lhx, lxh, lxx, mlh, mlx, mmh, mmx, mhh, mhx, mxh, mxx, hlx, hmx\}/hhl$  genotypes.

Best case, the  $\lambda temperate; clear^-$  phenotype ends up continually choosing between a lytic attack and a lysogenic cycle after any CII has diluted, meaning it will likely manifest as  $\lambda clear^-$  ex silico. It is exhibited by the  $\{hll, hml, xll, xmx\}/hhl$  genotypes — these have identical affinities for CI binding to  $O_{R1}$  and  $O_{R3}$ , see discussion of CEqEA's **MutualExclude** construct in Section S2.5.2. While it may appear as if the phenotype relies on CI having strictly higher affinity for binding to  $O_{R2}$ , leaving it to  $O_{R2}$  to decide the stochastic direction, the  $\{hhh, hxx, xhx\}/hhl$  genotypes merely lyse before the stochasticity is encountered.

If CI has higher than wild-type affinity for  $O_{R3}$ , meaning if CI occupies the operator physiologically at lower concentrations, the phenotype is  $\lambda clear^-$ : the operation of  $P_{RM}$  is compromised and CI basically works against itself and the lysogenic cycle.

If CI has wild-type or lower affinity for  $O_{R3}$ , the phenotype will start from  $\lambda temperate$  and increasingly tend towards  $\lambda virulent$  as the affinities for  $O_{R1}$  and  $O_{R2}$  get lower, i.e., as it becomes increasingly difficult for CI to prevent a lytic attack from  $P_R$ .

Probably the most interesting open question concerning the above genotypes and data is how we might tell the exhibited temperate phenotypes apart, including if they differ from the wild type.

If long-distance cooperativity across  $O_{\{L,R\}}3$  did not take place, see Section S2.5.1,  $O_R3$  would fill at extra-high CI concentration for the  $\lambda_{\text{c}}x/hhl$  genotypes. This would result in a super-temperate phenotype involving higher CI levels in the lysogenic cycle than the wild type, along with several related hybrid phenotypes that we do not discuss here.

### S2.5.5 Counterfactuals, following Section S2.5.4

We compare the relevant monograph counterfactuals to our analysis in Section S2.5.4 as best as permitted.

[[28]:68:8] (counterfactual):

SUPPRESSED

We have not considered any scenario with changed genes/proteins, only changed protein affinities from operator mutations.

[[28]:68:13] (counterfactual):

SUPPRESSED

The tests above found 34 (plus 4, probably) *clear* and 1 (plus 7, probably) *virulent* variants out of 64 considered. It appears possible to obtain a *virulent* variant by substantially weakening CI's affinity for  $O_R1$  (high instead of low physiological concentration, with medium skipped). We do not know how many mutations this would require. An alternative explanation for the preponderance of *clear* is that any increase to CI's affinity for  $O_R3$  (lower than high physiological concentration) trumps all other mutations and engenders a *clear* phenotype.

[[28]:68:-5b] (counterfactual):

SUPPRESSED

It seems that exactly the right mutations to just  $O_R$  would also result in a *virulent* variant, per our analysis.

[[28]:85:2] (counterfactual):

SUPPRESSED

As tested systematically above.

[[28]:85:4] (counterfactual):

SUPPRESSED

It would seem that mutations to just  $O_R\{1,2\}$  suffice. We cannot immediately mimic the referenced ('first')  $\lambda$ vir because [28] does not supply actionable information that allows us to vary the specifics of the  $O_{\{L,R\}}\{1,2\}$  octamer as a result of changed alternate-pairwise CI-binding involving  $O_L1$ .

We suspect the long-distance octamer still has surprises in store, as witnessed by the many surmises in Section S2.5.2. Of course, this would be a nice alternative target for Ceq-based first-principle analysis.

### S2.5.6 Cro-binding variants: lambdaVar-CI1hh-Cro $\square\square\square$ .mig

| genotype | $[-]_{-}^{\sim}$ | $[h]_{-}^{\sim}$ | $[-]_{10}^{\sim}$ | $[-]_{m0}^{\sim}$ | $x_0^{\sim}$ | $(x_0^{\sim})_{+}^{\sim}$ | $(x_0^{\sim})_{UV}^{\sim}$ | $0_x^{\sim}$  | #v/e/c/x/n    |
|----------|------------------|------------------|-------------------|-------------------|--------------|---------------------------|----------------------------|---------------|---------------|
| lhh/lll  | $0_{\{1,0\}}$    | $\{m,1\}_0$      | $1_0$             | $m_0$             | $\{m,1\}_0$  | $\parallel$               | $0_{\{1,0\}}$              | $0_{\{1,0\}}$ | 38/72/8/8/8   |
| lhh/llh  | $0_{\{1,0\}}$    | $\{m,1\}_0$      | $1_0$             | $m_0$             | $\{m,1\}_0$  | $\parallel$               | $0_{\{1,0\}}$              | $0_{\{1,0\}}$ | 37/70/8/8/8   |
| lhh/llx  | $0_{\{1,0\}}$    | $\{m,1\}_0$      | $1_0$             | $m_0$             | $\{m,1\}_0$  | $\parallel$               | $0_{\{1,0\}}$              | $0_{\{1,0\}}$ | 36/69/8/7/7   |
| lhh/lhl  | $0_1$            | $\{m,1\}_0$      | $1_0$             | $m_0$             | $\{m,1\}_0$  | $\parallel$               | $0_1$                      | $0_1$         | 38/74/8/9/9   |
| lhh/lhh  | $0_1$            | $\{m,1\}_0$      | $1_0$             | $m_0$             | $\{m,1\}_0$  | $\parallel$               | $0_1$                      | $0_1$         | 37/71/8/9/9   |
| lhh/lhx  | $0_1$            | $\{m,1\}_0$      | $1_0$             | $m_0$             | $\{m,1\}_0$  | $\parallel$               | $0_1$                      | $0_1$         | 36/70/8/8/8   |
| lhh/lxl  | $0_1$            | $\{m,1\}_0$      | $1_0$             | $m_0$             | $\{m,1\}_0$  | $\parallel$               | $0_1$                      | $0_1$         | 38/73/8/9/9   |
| lhh/lxh  | $0_1$            | $\{m,1\}_0$      | $1_0$             | $m_0$             | $\{m,1\}_0$  | $\parallel$               | $0_1$                      | $0_1$         | 37/70/8/9/9   |
| lhh/lxx  | $0_1$            | $\{m,1\}_0$      | $1_0$             | $m_0$             | $\{m,1\}_0$  | $\parallel$               | $0_1$                      | $0_1$         | 36/69/8/8/8   |
| lhh/hll  | $0_1$            | $\{m,1\}_0$      | $1_0$             | $m_0$             | $\{m,1\}_0$  | $\parallel$               | $0_1$                      | $0_1$         | 38/74/8/9/9   |
| lhh/hlh  | $0_1$            | $\{m,1\}_0$      | $1_0$             | $m_0$             | $\{m,1\}_0$  | $\parallel$               | $0_1$                      | $0_1$         | 37/71/8/9/9   |
| lhh/hlx  | $0_1$            | $\{m,1\}_0$      | $1_0$             | $m_0$             | $\{m,1\}_0$  | $\parallel$               | $0_1$                      | $0_1$         | 36/70/8/8/8   |
| lhh/hhl  | $\otimes$        | $\{m,1\}_0$      | $1_0$             | $m_0$             | $\{m,1\}_0$  | $\parallel$               | $\otimes$                  | $0_{\{h,1\}}$ | 38/72/8/9/9   |
| lhh/hhh  | $\otimes$        | $\{m,1\}_0$      | $1_0$             | $m_0$             | $\{m,1\}_0$  | $\parallel$               | $\otimes$                  | $0_{\{h,1\}}$ | 37/70/8/9/9   |
| lhh/hhx  | $\otimes$        | $\{m,1\}_0$      | $1_0$             | $m_0$             | $\{m,1\}_0$  | $\parallel$               | $\otimes$                  | $0_{\{h,1\}}$ | 36/69/8/8/8   |
| lhh/hxl  | $\otimes_h$      | $\{m,1\}_0$      | $1_0$             | $m_0$             | $\{m,1\}_0$  | $\parallel$               | $\otimes_h$                | $0_h$         | 38/73/8/10/10 |
| lhh/hxh  | $\otimes_h$      | $\{m,1\}_0$      | $1_0$             | $m_0$             | $\{m,1\}_0$  | $\parallel$               | $\otimes_h$                | $0_h$         | 37/70/8/10/10 |
| lhh/hxx  | $\otimes_h$      | $\{m,1\}_0$      | $1_0$             | $m_0$             | $\{m,1\}_0$  | $\parallel$               | $\otimes_h$                | $0_h$         | 36/69/8/9/9   |
| lhh/xll  | $0_1$            | $\{m,1\}_0$      | $1_0$             | $m_0$             | $\{m,1\}_0$  | $\parallel$               | $0_1$                      | $0_1$         | 38/73/8/9/9   |
| lhh/xlh  | $0_1$            | $\{m,1\}_0$      | $1_0$             | $m_0$             | $\{m,1\}_0$  | $\parallel$               | $0_1$                      | $0_1$         | 37/70/8/9/9   |
| lhh/xlx  | $0_1$            | $\{m,1\}_0$      | $1_0$             | $m_0$             | $\{m,1\}_0$  | $\parallel$               | $0_1$                      | $0_1$         | 36/69/8/8/8   |
| lhh/xhl  | $\otimes_h$      | $\{m,1\}_0$      | $1_0$             | $m_0$             | $\{m,1\}_0$  | $\parallel$               | $\otimes_h$                | $0_h$         | 38/73/8/10/10 |
| lhh/xhh  | $\otimes_h$      | $\{m,1\}_0$      | $1_0$             | $m_0$             | $\{m,1\}_0$  | $\parallel$               | $\otimes_h$                | $0_h$         | 37/70/8/10/10 |
| lhh/xhx  | $\otimes_h$      | $\{m,1\}_0$      | $1_0$             | $m_0$             | $\{m,1\}_0$  | $\parallel$               | $\otimes_h$                | $0_h$         | 36/69/8/9/9   |
| lhh/xxl  | $\otimes_x$      | $\{m,1\}_0$      | $1_0$             | $m_0$             | $\{m,1\}_0$  | $\parallel$               | $\otimes_x$                | $0_{\{x,h\}}$ | 38/73/8/10/10 |
| lhh/xxh  | $\otimes_x$      | $\{m,1\}_0$      | $1_0$             | $m_0$             | $\{m,1\}_0$  | $\parallel$               | $\otimes_x$                | $0_{\{x,h\}}$ | 37/70/8/10/10 |
| lhh/xxx  | $\otimes_x$      | $\{m,1\}_0$      | $1_0$             | $m_0$             | $\{m,1\}_0$  | $\parallel$               | $\otimes_x$                | $0_{\{x,h\}}$ | 36/69/8/9/9   |

lambdaVar-CI1hh-Cro $\square\square\square$ .mig

For the results of varying the intrinsic affinities for Cro binding to  $O_R$ , we note that the  $O_R\{1,2\}$ -bindings are regulatorily indistinguishable: lhh/abc tests identically to lhh/bac, for a,b,c in  $\{1,h,x\}$ . We also note that  $O_R3$  affinity does not affect the outcomes: lhh/abl, lhh/abh, and lhh/abx test identically, for a,b in  $\{1,h,x\}$  (except #v/e/c/x/n). Lastly, we note that Cro's  $O_R$ -affinities do not affect the CI-driven lysogenic cycle or its response to Cro-perturbation.

The Cro-affinities for  $O_R\{1,2\}$ -binding are strongly constrained in order to exhibit the Cro trajectory of the wild type: only lhh/{hhl,hhh,hhx} do so. Strong affinity for either of the  $O_R\{1,2\}$ -bindings (i.e., low physiological concentration) sees the *cro*-transcribing  $P_R$  become too constrained/insufficiently activated while low affinity sees  $P_R$  insufficiently constrained.

### S2.5.7 Anti-immunity, following Section S2.5.6

Anti-immunity is the ability of a (mutant) prophage to channel a super-infecting wild type to lytic growth: the prophage must prevent CI control by the wild type, and constitutive transcription of **cro** (Section S2.3:3/a/ $\alpha$ ) will do the rest, see [[28]:92:-8]. The wild type is not anti-immune. Further to Section S2.3:3/b/iii/ vs 3/c/ii/, ‘channeling’ automatically happens for a super-infecting wild type in case of ‘ $\neg\heartsuit$  or  $\spadesuit$ ’ but not in case of ‘ $\heartsuit$  and  $\neg\spadesuit$ ’. Seemingly because of the differences in these conditions, [28] suggests that a necessary requirement for anti-immunity is that **Cro** must be able to affect **cII**-transcription, see [[28]:92:-7]:

[[28]:92:-8] (counterfactual):

SUPPRESSED

[[28]:92:-7] (counterfactual):

SUPPRESSED

[[28]:92:Fig.4.23:1] (counterfactual):

SUPPRESSED

The lysogenic cycle is established by **CII** mediating **cI**-transcription from  $P_{RE}$  and is maintained by **CI** mediating **cI**-transcription from  $P_{RM}$ . Complementing [28], we investigate the possibility of anti-immunity resulting from intervention in the maintainance part. From Section S2.3:3/c/ii/, we see that certainly **Cro.l** and probably **Cro.h** from a variant will fail to prevent the wild-type entering its lysogenic cycle following **CI.l**, i.e., will fail to ensure anti-immunity. This means most of the considered variants are likely to not exhibit anti-immunity, see  $0_x^>$ . This is in line with the implied rarity of anti-immunity ex silico. However, possibly the **lhh**/**{hxl,hxh,hxx,xhl,xhh,xhx}** but more likely the **lhh**/**{xxl,xxh,xxx}** genotypes may stand a chance against a super-infecting wild-type taking control, depending on how much above **Cro.h** the ex-silico observable state is. Of these, **lhh/xxl** best counteracts  $P_{RM}$ . The possible linearized coextension derivations are as follows, edited for horizontal space and without inhibited processes:

```

[CI.1, Cro.h] + [CII.h]
-> ![OR3_Cro,0?R12_CI] ; ![0?R12_CI]

<divergence>
  [CI.0, CI.1, Cro.1, Cro.h]
  * resolution required

```

```

[CI.0, Cro.1] + [CII.h]
-> [PR_tr] ; [PRE_tr,ORE_CII]

[CI.1, Cro.h] + [CII.h]
-> ![OR3_Cro,0?R12_CI] ; ![0?R12_CI]

```

```

[CI.1, Cro.1] + [CII.h]
-> ![0?R12_CI]

[CI.1, Cro.0] + [CII.h]
-> [PRM_tr,0?R12_CI]

```

```

[CI.0, Cro.h] + [CII.h]
-> [PR_tr] ; [PRE_tr,ORE_CII]

[CI.1, Cro.x] + [CII.h]
-> ![OR3_Cro,0?R12_CI] ; ![0?R12_CI]

```

```

[CI.1, Cro.h] + [CII.h]
-> ![OR3_Cro,0?R12_CI] ; ![0?R12_CI]

<divergence>
  [CI.0, CI.1, Cro.1, Cro.h]

```

```

[CI.1, Cro.x] + [CII.h]
-> ![OR3_Cro,0?R12_CI] ; ![0?R12_CI]

<divergence>
  [CI.0, CI.1, Cro.h, Cro.x]
  * resolution required

```

```

[CI.0, Cro.h] + [CII.h]
-> [PR_tr] ; [PRE_tr,ORE_CII]

[CI.1, Cro.x] + [CII.h]
-> ![OR3_Cro,0?R12_CI] ; ![0?R12_CI]

```

```

[CI.1, Cro.h] + [CII.h]
-> ![OR3_Cro,0?R12_CI] ; ![0?R12_CI]

<divergence>
  [CI.0, CI.1, Cro.1, Cro.h]

```

```

[CI.0, Cro.x] + [CII.h]
-> ![OR2_Cro,OR1_Cro] ;
  [PRE_tr,ORE_CII]

[CI.1, Cro.h] + [CII.h]
-> ![OR3_Cro,0?R12_CI] ; ![0?R12_CI]

```

```

[CI.1, Cro.x] + [CII.h]
-> ![OR3_Cro,0?R12_CI] ; ![0?R12_CI]

<divergence>
  [CI.0, CI.1, Cro.h, Cro.x]

```

Failure to prevent CI takeover, i.e., failure of anti-immunity, happens only in the particular case of [CI.1,Cro.1] + [CII.h]: the super-infection must encounter the lowest possible Cro concentration and, even though this concentration suffices to prevent *cI*-transcription from P<sub>RM</sub> to the extent that any production is less than natural decay (! [OR3\_Cro,0?R12\_CI]), stochastic events must conspire to have P<sub>RM</sub> operate enough to maintain the CI concentration originally produced from P<sub>RE</sub> (which has ceased functioning due to said concentration).

**Article:Retrodiction (V): *cII*-free anti-immunity** The *lhh/xxl* genotype could exhibit anti-immunity absent any Cro inhibition of *cII*.

Experiments are needed to determine if the balances work in Cro's favour.

## S2.5.8 The $\lambda^{[AGS3]}$ combinator

```

1  /*****
2  /* modality      = default ; */
3  *****/

5  Instantiation    = coherent ;
6  Regulation       = intrinsic ;
7  Causation        = pushpull ;
8  Termination      = endpoint ;

10 Solution         = fixed ;

13 /*****
14 /* categories     = $abstraction ; */
15 *****/

17 categories       = $dnaCI, $genomeI, $proteinC ;

20 /*****
21 /* $level/schema . $level/states [l modalities] ; */
22 *****/

24 /*regulatory factors: E. coli*/
25 $dnaCI / DNA      . [ {ss} ds ] ;
26 $proteinC / RNAP . {tr} ;

28 /*regulated components: E. coli*/
29 $proteinC / RecA . [ " {*} ] ;

32 /*regulatory factors: lambda*/
33 $proteinC / CII . [ _ {h} ] ;

35 /*regulated components: lambda*/
36 $genomeI / cI . $proteinC / [ 0 {l} {m} {h} {x} ] ;
37 $genomeI / cro . $proteinC / [ 0 {l} {h} {x} ] ;

40 /*****
41 /* @macro<>      = transposed interface ; */
42 *****/

44 @OR1_CI_int<>    = CI.□ ;
45 @OR2_CI_int<>    = CI.□ ;
46 @OR3_CI_int<>    = CI.□ ;

48 @OR1_Cro_int<>   = Cro.□ ;
49 @OR2_Cro_int<>   = Cro.□ ;
50 @OR3_Cro_int<>   = Cro.□ ;

52 @ORE_CII_int<>   = CII.h ;

54 @UV_irr_int<>    = DNA.ss ;
55 @SOS_int<>       = RecA.* ;

57 /*cooperative affinities*/
58 @OR12_CI_tetra<> = (+) min&(@OR1_CI_int,@OR2_CI_int) ;
59 @OR23_CI_tetra<> = (+) min&(@OR2_CI_int,@OR3_CI_int) ;

61 @OLR12_CI_octa<> = max&(*OL12*/(+)CI.l,@OR12_CI_tetra) ;
62 @OLR123_CI_octTtr<> = max&(@OLR12_CI_octa, (+)
    min&(*OL3*/CI.h,@OR3_CI_int)) ;

65 /*****
66 /* @macro        = regulatory binding [precedence] ; */
67 *****/

```

```

69 /*cooperative binding*/
70 cond( @OR1_CI_int << @OR3_CI_int )
71   @OLR123_CI = @OLR123_CI_octTtr ;
72   @O?R12_CI = @OR12_CI_tetra excl @OLR123_CI-- ;
73   //subsume
74   @O?R23_CI = @OR23_CI_tetra excl @OLR123_CI-- : @O?R12_CI-- ;
75   //preclude
76 endcond;
77 cond( @OR1_CI_int >> @OR3_CI_int )
78   @O?R23_CI = @OR23_CI_tetra ;
79   @OLR123_CI = ;// excl @O?R23_CI-- ;
80   //preclude
81   @O?R12_CI = @OR12_CI_tetra excl @O?R23_CI-- : @OLR123_CI-- ;
82   //preclude:subsume
83 endcond;
84 cond( @OR1_CI_int == @OR3_CI_int )
85   @OLR123_CI = @OLR123_CI_octTtr ;
86   @O?R12_CI = @OR12_CI_tetra excl @OLR123_CI-- ;
87   //subsume
88   @O?R23_CI = @OR23_CI_tetra ;
89   MutualExclude ( @O?R23_CI, @O?R12_CI ) ;
90   //stochastic
91   MutualExclude ( @O?R23_CI, @OLR123_CI ) ;
92   //stochastic
93 endcond;
94
95 /*cooperative occupancy*/
96 @O?R12?_CI_rng<> = @OLR123_CI-- : @O?R12_CI-- ;
97 @O?R?23_CI_rng<> = @OLR123_CI-- : @O?R23_CI-- ;
98 @O?R?2?_CI_rng<> = @OLR123_CI-- : @O?R12_CI-- : @O?R23_CI-- ;
99
100
101 /*OR1*/
102 @OR1_CI = @OR1_CI_int excl @O?R12?_CI_rng ;
103 @OR1_Cro = @OR1_Cro_int |-- @O?R12?_CI_rng ;
104
105 /*OR2*/
106 @OR2_CI = @OR2_CI_int excl @O?R?2?_CI_rng ;
107 @OR2_Cro = @OR2_Cro_int |-- @O?R?2?_CI_rng ;
108
109 /*OR3*/
110 @OR3_CI = @OR3_CI_int excl @O?R?23_CI_rng ;
111 @OR3_Cro = @OR3_Cro_int |-- @O?R?23_CI_rng ;
112
113 /*ORE*/
114 @ORE_CII = @ORE_CII_int ;
115
116 /*cytosol*/
117 @UV_irr = @UV_irr_int ;
118 @SOS = @SOS_int ;
119
120 /*=====*/
121 /* @macro = regulation ; */
122 /*-----*/
123 /* +- | level/subject ;
124 | influence
125 [| modalities] ; */
126 /*=====*/
127
128 /*cytosol*/
129 + ! | $proteinC / RecA | @UV_irr ;
130
131 - | $proteinC / CI | ^@SOS | ceaseless ;
132
133 /*genome: cI*/
134 @PRE_tr = RNAP.tr
135 & ^@ORE_CII--
136 |-- @O?R?2?_CI_rng ! { |incdnt1(CI)<mdtr,sink>}

```

```

133         ;
135 @PRM_tr = RNAP.tr
136         & ^(@0?R12_CI-- : @0R2_CI--)
137         |-- @0R3_Cro
138         : @0R3_Cro +- !
139         : @0R3_CI
140         : @0R3_CI +- !
141         : @0?R?23_CI_rng ! {|incdnt1(CI)<mdtr,sink>}
142         ;
144 +>@SOS< ! | $proteinC / cI | @PRE_tr
145         : @PRM_tr ;
147
148 /*genome: cro, w/simultaneous+independent binding*/
150 @0R1and2_Cro<@0R1_Cro,@0R2_Cro> = max&(@0R1_Cro,@0R2_Cro) ;
151 @0R1xor2_Cro<> = min:(@0R1_Cro,@0R2_Cro) excl @0R1and2_Cro-- ;
152
153 @0R1and2_CI<@0R1_CI,@0R2_CI> = max&(@0R1_CI,@0R2_CI) ;
154 @0R1xor2_CI<> = min:(@0R1_CI,@0R2_CI) excl @0R1and2_CI-- ;
155
156 @PR_tr = RNAP.tr
157         /*& no recruiter*/
158         |-- @0R1xor2_Cro
159         : @0R1xor2_Cro +- !
160         : @0R1and2_Cro -- !
161         : @0R1xor2_CI
162         : @0R1xor2_CI +- !
163         : @0R1and2_CI -- !
164         : @0?R?2?_CI_rng ! {|incdnt1(CI)<mdtr,sink>}
165         ;
167 + ! | $proteinC / cro | @PR_tr ;
169
170 /*=====*/
171 /* seed | modalities ; */
172 /*=====*/
173
174 "Cro.h" | expire(1,1) ;
175
177 "CI.0, Cro.0" entry(inject) | vanishOK<out>,
178         mix(CI,Cro)<out,src>,
179         incidental<out,mdtr,src> ;
180
181
182 /*=====*/
183 /*--- end ---*/
184 /*=====*/

```

## SA ‘Motivation’ of [28]

This appendix lists factual statements in [28] we have classified as ‘motivation’.  
We share in and accomplish or further these, see article.

## *Quotation filter*

- motivations: included
- axioms: excluded

---

- semantics: excluded
- incidentals: excluded

---

- molecular basis: excluded
- population inferences: excluded
- causation arguments: excluded
- pathway arguments: excluded
- cell behaviours: excluded

---

- mutations/counterfactuals: excluded

---

- superseded: excluded

## Preface

**AGS3, Preface, 3rd Ed., p.xi, l.11, motivation :**

**Ptashne:** SUPPRESSED

CEq: Our Retrodiction of [28] in the article provides some reformulation on the outgoing side. The referenced discoveries nixed a line of argumentation that was based on just-so evidence, related to site preservation. The new discoveries explain the preservation. See Section S2.5.1 for the outgoing effects of the ingoing additions.

**AGS3, Preface, 3rd Ed., p.xii, l.5, motivation :**

**Ptashne:** SUPPRESSED

CEq: We verify internal correctness of [28]’s reasoning, see Section S2.3. This is a strong, technical version of coherence. We also show that the reasoning generates the full  $\lambda$  temperate life cycle with conditional responses in a computational sense, see Section S2.4 and article. This is a strong, technical version of completeness.

**AGS3, Preface, 1st Ed., p.xiii, l.11, motivation :**

**Ptashne:** SUPPRESSED

CEq: All technologies we introduce are highly abstract, see, e.g., Figure 2, and CEq is designed for parsimony, see article. There is no reason to think that any part is specific to [28] or, indeed, to  $\lambda$ . CEqEA allows for arbitrary sub-system analysis of cascaded causation diagrams, see Section S2.3 and article. This is the fundamental technical form of cell types. Sub-system analysis in this sense is not permitted in state-space modeling/with reasoning in classical (aka Boolean) logic, see Section S1.1.6 and article. CEqEA contains other technologies to explicitly address cell types, e.g., by automatically generating specialized cascaded causation diagrams, see Section S2.4.

**AGS3, Preface, 1st Ed., p.xiv, l.9, motivation :**

**Ptashne:** SUPPRESSED

CEq: The reasoning in [28] is overwhelmingly (even surprisingly so and when compared to similar work in mathematics) formalizable within an abstract axiomatic framework that enjoys several meta-theoretic properties of interest, including consistency. No part of the axiomatic framework is convoluted, i.e., it reflects a mature tradition: molecular biology, that has been extensively vetted for transparency by peer review over many years.

**AGS3, Preface, 1st Ed., p.xiv, l.21, motivation :**

**Ptashne:** SUPPRESSED

CEq: See our discussion of formal methods and visualization in the article.

**AGS3, Preface, 1st Ed., p.xiv, l.23, motivation :**

**Ptashne:** SUPPRESSED

CEq: See Section S2.1.

**this chapter has** 6 quotations with the present filter.

## Introduction

**AGS3, Introduction, p.2, l.-3, motivation :**

**Ptashne:** SUPPRESSED

CEq: We introduce technologies that capture these mechanisms and that axiomatize their multi-scale interactions, see article, especially our discussion of constructive reasoning.

**AGS3, Introduction, p.10, l.8, motivation :**

**Ptashne:** SUPPRESSED

CEq: The main purpose of this work is to formalize that account, to validate it, e.g., by showing that it constitutes a consistent logic, and to indicate the range of benefits that derive from having a detailed technical understanding of the mechanisms. In effect, we show that such an account is far more valuable than it is likely to be appreciated outside the field of formal reasoning.

**AGS3, Introduction, p.10, l.10, motivation :**

**Ptashne:** SUPPRESSED

CEq: See our discussion of our RI modeling methodology in the article and Section S2.1.

**this chapter has** 3 quotations with the present filter.

## Chapter 1

**AGS3, Chapter 1, p.28, l.-11, motivation :**

**Ptashne:** SUPPRESSED

CEq: It is too early to speculate about this issue as putative theorems about the CEq theory. For one, it is not clear what ‘circuit’ might mean technically when you consider full regulatory form (as opposed to top-down-determined gene regulation networks, or similar) and in what exact ways and circumstances a set of regulatory dependencies might be viewed in isolation and have the resulting behaviours extrapolated to bigger contexts. (State-space modeling does not resolve the matter, appearances notwithstanding — quite the opposite.) Certainly, both the concepts of homeostasis and destability are encountered in our technical treatment of [28]’s reasoning, see Section S2.3.2:2/ and Section S2.3.2:3/d/:NB!.

**this chapter has** 1 quotations with the present filter.

## Chapter 2

**this chapter has** 0 quotations with the present filter.

## Chapter 3

**AGS3, Chapter 3, p.60, l.1, motivation :**

**Ptashne:** SUPPRESSED

CEq: The CEq theory is highly abstract and the CEqEA tool is purely symbolic and designed for parsimony, see article.

**AGS3, Chapter 3, p.60, l.14, motivation :**

**Ptashne:** SUPPRESSED

CEq: The CEq theory is highly abstract and designed for parsimony, see article, is associated with a stepwise modeling methodology, see Section S2.1, and does, in fact, constitute a (purely symbolic) logic that is consistent and more, see article and Section S1.3.

**this chapter has** 2 quotations with the present filter.

## Chapter 4

**this chapter has** 0 quotations with the present filter.

## Chapter 5

AGS3, Chapter 5, p.133, l.12, motivation :

**Ptashne:** SUPPRESSED

CEq: See our discussion of modalities in Sections S2.1,S2.5.1.

this chapter has 1 quotations with the present filter.

## Appendix 1

this chapter has 0 quotations with the present filter.

## Appendix 2

this chapter has 0 quotations with the present filter.

### *Quotation tallies*

- motivations: 13 (included)
- axioms: 10 (excluded)

---

- semantics: 51 (excluded)
- incidentals: 161 (excluded)

---

- molecular basis: 99 (excluded)
- population inferences: 9 (excluded)
- causation arguments: 16 (excluded)
- pathway arguments: 29 (excluded)
- cell behaviours: 27 (excluded)

---

- mutations/counterfactuals: 48 (excluded)

---

- superseded: 18 (excluded)

---

- $\Sigma$ : 13 of 481 (total) quotations included

## **SB ‘Axioms’ of [28]**

This appendix lists factual statements in [28] we have classified as ‘axioms’. These are directly related to the structure and specifics of the CEq theory, which, in turn, provides the organization and underpinning of the CEqEA tool, as outlined below.

### *Quotation filter*

- motivations: excluded
- axioms: included

---

- semantics: excluded
- incidentals: excluded

---

- molecular basis: excluded
- population inferences: excluded
- causation arguments: excluded
- pathway arguments: excluded
- cell behaviours: excluded

---

- mutations/counterfactuals: excluded

---

- superseded: excluded

## Preface

**AGS3, Preface, 3rd Ed., p.xi, l.1, axiom :**

**Ptashne:** SUPPRESSED

CEq: This is both an axiom and a meta-axiom: we affirm the first part logically (in the form of the meta-theoretic property of constructivity) and the word perhaps computationally (in the form of simulation, which follows from constructivity).

**AGS3, Preface, 3rd Ed., p.xii, l.3, axiom :**

**Ptashne:** SUPPRESSED

CEq: This is a meta-axiom, as it were: a declaration that [28] is axiomatically construed and bottom-up. We contribute an axiomatization, apply it, and develop it meta-theoretically, with results and discussion on the technical notions of ab intra and constructivity.

this chapter has 2 quotations with the present filter.

## Introduction

**AGS3, Introduction, p.1, l.16, axiom :**

**Ptashne:** SUPPRESSED

CEq: CEqEA's MIG specifications are based on schemas, see Section S2.1.4. A schema is defined as a hierarchy of collections of states, where each collection is a schema instance at some specific category (e.g., mRNA or protein) and where the schema has a base category (e.g., gene). See Crick's Sequence Hypothesis [5].

**AGS3, Introduction, p.3, l.1, axiom :**

**Ptashne:** SUPPRESSED

CEq: Most fundamentally, the CEq theory is guaranteed to be open-system, see article. CEqEA identifies and makes environmental signals explicit in cascaded causation diagrams by its toggle mechanism, see Section S1.4.1. Additionally, the **ExogenyInference** directive externalizes them in such a way that a technical open-system assumption allows us to retain environmental controls as conditionals in our computational analysis of the possible reasoning, see Section S2.4.

**AGS3, Introduction, p.5, l.-5, axiom :**

**Ptashne:** SUPPRESSED

CEq: The RI modeling methodology allows for schema instances at arbitrary categories to be transparent for reasoning purposes, see Section S2.1. In this particular case, the relevant entities are genes and proteins in dimer form, with everything physically intermediate between them (from RNA onwards) considered transparent. In addition to issues related to coinhibition, see Section S2.1.8, we note that we explicitly account for when any RNAP recruiters are sufficiently absent and inhibition is sufficiently strong to render natural decay physiological, including how this happens in cases of multiple transcription possibilities in Section S2.2. These issues are determined in part by the involved binding mechanisms [29], which means they are strongly affected by the kind of cooperative binding whose discovery prompted [28], see [[28]:121:1]/App.SH.

**AGS3, Introduction, p.5, l.-3a, axiom :**

**Ptashne:** SUPPRESSED

CEq: This issue complements [[28]:1:16]/App.SB. Our RI modeling methodology stipulates that schema-instance states are nominal transpositions (typically concentrations) of binding affinities, as opposed to, say, observable concentrations, see Section S1.5.

**AGS3, Introduction, p.8, l.12, axiom :**

**Ptashne:** SUPPRESSED

CEq: The regulatory aspect of this issue is captured in CEqEA’s modal influences and how they are constructed step-by-step by our RI modeling methodology, see Section S2.1. The operational aspect is captured in CEqEA’s regulatory functionality, i.e., causations, see Section S2.2 and Figure 3. A core difference is that regulators may be arbitrarily combined in regulation’s form while, as implied above, they act discretely in regulation’s (individual-concentration changing) functionality. We seemingly provide the first explicit treatment of the two and their connection.

**AGS3, Introduction, p.8, l.-16, axiom :**

**Ptashne:** SUPPRESSED

CEq: This issue is captured in CEqEA’s notion of states and the fine-grained control of their effects, e.g., by MIG modalities, see Section S2.1. In particular, our RI modeling methodology stipulates that we consider binding-transposing states with attendant usage of MIG ranges and qualified contravariance to address how different types of bindings affect basal transcription differently. See also the comments at [[28]:1:16]/App.SB. More, CEqEA comes with a population-inference engine, via the `excl` keyword, to ensure that auto-regulation is treated correctly under these concerns, see App.SD.

**AGS3, Introduction, p.9, l.-3, axiom :**

**Ptashne:** SUPPRESSED

CEq: This issue is made explicit in our technical notion of cascaded causation diagrams, see Section S1.4.1.

**this chapter has** 7 quotations with the present filter.

## **Chapter 1**

**this chapter has** 0 quotations with the present filter.

## **Chapter 2**

**this chapter has** 0 quotations with the present filter.

## **Chapter 3**

**this chapter has** 0 quotations with the present filter.

## **Chapter 4**

**AGS3, Chapter 4, p.92, l.-3, axiom :**

**Ptashne:** SUPPRESSED

CEq: This distinction between physiological and observable states is one of two issues addressed by CEqEA's notion of sustained equilibria, see Section S1.5.2. The other is sustaining, as effected by discrete inhibitors, see [[28]:8:12]/App.SB. CEqEA's synchronization diagrams to predict life cycles are constructed based on observable states, see Section S1.5.3.

**this chapter has** 1 quotations with the present filter.

## **Chapter 5**

**this chapter has** 0 quotations with the present filter.

## **Appendix 1**

**this chapter has** 0 quotations with the present filter.

## Appendix 2

this chapter has 0 quotations with the present filter.

### *Quotation tallies*

- motivations: 13 (excluded)
- axioms: 10 (included)

---

- semantics: 51 (excluded)
- incidentals: 161 (excluded)

---

- molecular basis: 99 (excluded)
- population inferences: 9 (excluded)
- causation arguments: 16 (excluded)
- pathway arguments: 29 (excluded)
- cell behaviours: 27 (excluded)

---

- mutations/counterfactuals: 48 (excluded)

---

- superseded: 18 (excluded)

---

- $\Sigma$ : 10 of 481 (total) quotations included

## SC ‘Molecular basis’ of [28]

This appendix lists factual statements in [28] we have classified as making up the ‘molecular basis’ of its body of reasoning. As detailed below and in Section S2.1, they are transliterated under our RI modeling methodology into our MIG specification language.

## *Quotation filter*

- motivations: excluded
- axioms: excluded

---

- semantics: excluded
- incidentals: excluded

---

- molecular basis: included
- population inferences: excluded
- causation arguments: excluded
- pathway arguments: excluded
- cell behaviours: excluded

---

- mutations/counterfactuals: excluded

---

- superseded: excluded

## Preface

this chapter has 0 quotations with the present filter.

## Introduction

AGS3, Introduction, p.6, l.-9a, molecular basis :

**Ptashne:** SUPPRESSED

CEq: [lambda[AGS3]\_RI.mig: 1.5–10, 1.17, 1.26, 1.105–108, 1.110–117, 1.131–140]

this chapter has 1 quotations with the present filter.

## Chapter 1

AGS3, Chapter 1, p.11, l.1, molecular basis :

**Ptashne:** SUPPRESSED

CEq: [lambda[AGS3]\_RI.mig: 1.5–10, 1.17, 1.36, 1.37]

AGS3, Chapter 1, p.12, l.7, molecular basis :

**Ptashne:** SUPPRESSED

CEq: [lambda[AGS3]\_RI.mig: 1.5, 1.152–154]

AGS3, Chapter 1, p.12, l.-8, molecular basis :

**Ptashne:** SUPPRESSED

CEq: [lambda[AGS3]\_RI.mig: 1.5–10, 1.17, 1.26, 1.36, 1.37, 1.44–46, 1.48–50, 1.105–108, 1.110–117, 1.131–140]

AGS3, Chapter 1, p.14, l.6, molecular basis :

**Ptashne:** SUPPRESSED

CEq: [lambda[AGS3]\_RI.mig: 1.110–117, 1.119–120, 1.142, 1.131–140]

AGS3, Chapter 1, p.14, l.11, molecular basis :

**Ptashne:** SUPPRESSED

CEq: [lambda[AGS3]\_RI.mig: 1.110–117, 1.131–140]

AGS3, Chapter 1, p.14, Fig.1.4, l.1, molecular basis :

**Ptashne:** SUPPRESSED

CEq: [lambda[AGS3]\_RI.mig: 1.110–117, 1.119–120, 1.142, 1.131–140]

**AGS3, Chapter 1, p.15, l.11, molecular basis :**

**Ptashne:** SUPPRESSED

CEq: [lambda[AGS3]\_RI.mig: 1.26, 1.105–108, 1.110–117, 1.131–140]

**AGS3, Chapter 1, p.15, l.13, molecular basis :**

**Ptashne:** SUPPRESSED

CEq: [lambda[AGS3]\_RI.mig: 1.110–117, 1.119–120, 1.142, 1.131–140]

**AGS3, Chapter 1, p.15, l.-4, molecular basis :**

**Ptashne:** SUPPRESSED

CEq: [lambda[AGS3]\_RI.mig: 1.110–117, 1.131–140]

**AGS3, Chapter 1, p.15, l.-2, molecular basis :**

**Ptashne:** SUPPRESSED

CEq: [lambda[AGS3]\_RI.mig: 1.110–117]

**AGS3, Chapter 1, p.17, l.2, molecular basis :**

**Ptashne:** SUPPRESSED

CEq: [lambda[AGS3]\_RI.mig: 1.44–46]

**AGS3, Chapter 1, p.17, l.6, molecular basis :**

**Ptashne:** SUPPRESSED

CEq: [lambda[AGS3]\_RI.mig: 1.48–50, 1.69–86]

**AGS3, Chapter 1, p.18, l.5, molecular basis :**

**Ptashne:** SUPPRESSED

CEq: [lambda[AGS3]\_RI.mig: 1.110–117, 1.119–120, 1.142, 1.131–140]

**AGS3, Chapter 1, p.18, l.8, molecular basis :**

**Ptashne:** SUPPRESSED

CEq: [lambda[AGS3]\_RI.mig: 1.142, 1.131–140]

**AGS3, Chapter 1, p.18, l.11, molecular basis :**

**Ptashne:** SUPPRESSED

CEq: [lambda[AGS3]\_RI.mig: l.110–117, l.119–120]

**AGS3, Chapter 1, p.18, l.-3, molecular basis :**

**Ptashne:** SUPPRESSED

CEq: [lambda[AGS3]\_RI.mig: l.105–108, l.110–117, l.119–120, l.142, l.131–140]

**AGS3, Chapter 1, p.18, Fig.1.12, l.2, molecular basis :**

**Ptashne:** SUPPRESSED

CEq: [lambda[AGS3]\_RI.mig: l.110–117, l.119–120, l.142, l.131–140]

**AGS3, Chapter 1, p.19, l.2, molecular basis :**

**Ptashne:** SUPPRESSED

CEq: [lambda[AGS3]\_RI.mig: l.110–117]

**AGS3, Chapter 1, p.19, l.6, molecular basis :**

**Ptashne:** SUPPRESSED

CEq: [lambda[AGS3]\_RI.mig: l.110–117, l.131–140]

**AGS3, Chapter 1, p.19, l.-5, molecular basis :**

**Ptashne:** SUPPRESSED

CEq: [lambda[AGS3]\_RI.mig: l.110–117, l.131–140]

**AGS3, Chapter 1, p.19, l.-2, molecular basis :**

**Ptashne:** SUPPRESSED

CEq: [lambda[AGS3]\_RI.mig: l.110–117, l.131–140]

**AGS3, Chapter 1, p.19, Fig.1.13, l.1, molecular basis :**

**Ptashne:** SUPPRESSED

CEq: [lambda[AGS3]\_RI.mig: l.131–140]

**AGS3, Chapter 1, p.20, l.3b, molecular basis :**

**Ptashne:** SUPPRESSED

CEq: [lambda[AGS3]\_RI.mig: 1.110–117, 1.131–140]

**AGS3, Chapter 1, p.20, l.10a, molecular basis :**

**Ptashne:** SUPPRESSED

CEq: [lambda[AGS3]\_RI.mig: 1.110–117]

**AGS3, Chapter 1, p.20, l.10b, molecular basis :**

**Ptashne:** SUPPRESSED

CEq: [lambda[AGS3]\_RI.mig: 1.64]

**AGS3, Chapter 1, p.20, l.14, molecular basis :**

**Ptashne:** SUPPRESSED

CEq: [lambda[AGS3]\_RI.mig: 1.44–46]

**AGS3, Chapter 1, p.20, l.15, molecular basis :**

**Ptashne:** SUPPRESSED

CEq: [lambda[AGS3]\_RI.mig: 1.64]

**AGS3, Chapter 1, p.20, l.-9, molecular basis :**

**Ptashne:** SUPPRESSED

CEq: [lambda[AGS3]\_RI.mig: 1.110–117]

**AGS3, Chapter 1, p.21, l.-3, molecular basis :**

**Ptashne:** SUPPRESSED

CEq: [lambda[AGS3]\_RI.mig: 1.64]

**AGS3, Chapter 1, p.23, l.-1, molecular basis :**

**Ptashne:** SUPPRESSED

CEq: [lambda[AGS3]\_RI.mig: 1.54]

**AGS3, Chapter 1, p.24, l.1, molecular basis :**

**Ptashne:** SUPPRESSED

CEq: [lambda[AGS3]\_RI.mig: 1.98]

**AGS3, Chapter 1, p.24, l.5, molecular basis :**

**Ptashne:** SUPPRESSED

CEq: [lambda[AGS3]\_RI.mig: 1.29, 1.100]

**AGS3, Chapter 1, p.24, l.10, molecular basis :**

**Ptashne:** SUPPRESSED

CEq: [lambda[AGS3]\_RI.mig: 1.100]

**AGS3, Chapter 1, p.24, l.-8, molecular basis :**

**Ptashne:** SUPPRESSED

CEq: [lambda[AGS3]\_RI.mig: 1.105–108, 1.110–117, 1.131–140]

**AGS3, Chapter 1, p.24, l.-3, molecular basis :**

**Ptashne:** SUPPRESSED

CEq: [lambda[AGS3]\_RI.mig: 1.48–50]

**AGS3, Chapter 1, p.24, Fig.1.21, l.1, molecular basis :**

**Ptashne:** SUPPRESSED

CEq: [lambda[AGS3]\_RI.mig: 1.105–108, 1.110–117, 1.131–140]

**AGS3, Chapter 1, p.25, l.2b, molecular basis :**

**Ptashne:** SUPPRESSED

CEq: [lambda[AGS3]\_RI.mig: 1.110–117]

**AGS3, Chapter 1, p.25, Fig.1.23, l.1, molecular basis :**

**Ptashne:** SUPPRESSED

CEq: [lambda[AGS3]\_RI.mig: 1.48–50]

**AGS3, Chapter 1, p.26, l.1, molecular basis :**

**Ptashne:** SUPPRESSED

CEq: [lambda[AGS3]\_RI.mig: 1.100, 1.110–117]

**AGS3, Chapter 1, p.26, l.-1, molecular basis :**

**Ptashne:** SUPPRESSED

CEq: [lambda[AGS3]\_RI.mig: 1.131–140]

this chapter has 40 quotations with the present filter.

## Chapter 2

AGS3, Chapter 2, p.37, l.15, molecular basis :

**Ptashne:** SUPPRESSED

CEq: [lambda[AGS3]\_RI.mig: l.105–108]

AGS3, Chapter 2, p.43, l.-5, molecular basis :

**Ptashne:** SUPPRESSED

CEq: [lambda[AGS3]\_RI.mig: l.110–117, l.131–140]

AGS3, Chapter 2, p.44, l.6, molecular basis :

**Ptashne:** SUPPRESSED

CEq: [lambda[AGS3]\_RI.mig: l.131–140]

AGS3, Chapter 2, p.44, l.9, molecular basis :

**Ptashne:** SUPPRESSED

CEq: [lambda[AGS3]\_RI.mig: l.110–117]

AGS3, Chapter 2, p.44, l.-5, molecular basis :

**Ptashne:** SUPPRESSED

CEq: [lambda[AGS3]\_RI.mig: l.110–117, l.131–140]

AGS3, Chapter 2, p.44, l.-4, molecular basis :

**Ptashne:** SUPPRESSED

CEq: [lambda[AGS3]\_RI.mig: l.131–140]

AGS3, Chapter 2, p.45, l.4, molecular basis :

**Ptashne:** SUPPRESSED

CEq: [lambda[AGS3]\_RI.mig: l.110–117]

AGS3, Chapter 2, p.45, l.13a, molecular basis :

**Ptashne:** SUPPRESSED

CEq: [lambda[AGS3]\_RI.mig: l.131–140]

this chapter has 8 quotations with the present filter.

## Chapter 3

AGS3, Chapter 3, p.55, l.6, molecular basis :

Ptashne: SUPPRESSED

CEq: [lambda[AGS3]\_RI.mig: 1.52, 1.105–108]

AGS3, Chapter 3, p.55, l.-2, molecular basis :

Ptashne: SUPPRESSED

CEq: [lambda[AGS3]\_RI.mig: 1.105–108, 1.119–120]

AGS3, Chapter 3, p.56, l.1, molecular basis :

Ptashne: SUPPRESSED

CEq: [lambda[AGS3]\_RI.mig: 1.119–120]

AGS3, Chapter 3, p.56, l.-1a, molecular basis :

Ptashne: SUPPRESSED

CEq: [lambda[AGS3]\_RI.mig: 1.33, 1.52]

AGS3, Chapter 3, p.57, l.3, molecular basis :

Ptashne: SUPPRESSED

CEq: [lambda[AGS3]\_RI.mig: 1.33]

AGS3, Chapter 3, p.60, l.-7, molecular basis :

Ptashne: SUPPRESSED

CEq: [lambda[AGS3]\_RI.mig: 1.54, 1.55, 1.98, 1.100, 1.119–120]

this chapter has 6 quotations with the present filter.

## Chapter 4

AGS3, Chapter 4, p.68, l.-5a, molecular basis :

Ptashne: SUPPRESSED

CEq: [lambda[AGS3]\_RI.mig: 1.105–108, 1.119–120]

AGS3, Chapter 4, p.84, l.12, molecular basis :

Ptashne: SUPPRESSED

CEq: [lambda[AGS3]\_RI.mig: 1.48–50]

**AGS3, Chapter 4, p.86, l.1, molecular basis :**

**Ptashne:** SUPPRESSED

CEq: [lambda[AGS3]\_RI.mig: 1.44–46, 1.64]

**AGS3, Chapter 4, p.86, l.10, molecular basis :**

**Ptashne:** SUPPRESSED

CEq: [lambda[AGS3]\_RI.mig: 1.64]

**AGS3, Chapter 4, p.86, Fig.4.18, l.1, molecular basis :**

**Ptashne:** SUPPRESSED

CEq: [lambda[AGS3]\_RI.mig: 1.44–46, 1.64]

**AGS3, Chapter 4, p.92, l.1a, molecular basis :**

**Ptashne:** SUPPRESSED

CEq: [lambda[AGS3]\_RI.mig: 1.48–50]

**AGS3, Chapter 4, p.93, Fig.4.24, l.1, molecular basis :**

**Ptashne:** SUPPRESSED

CEq: [lambda[AGS3]\_RI.mig: 1.48–50, 1.125–129, 1.131–140]

**AGS3, Chapter 4, p.93, Table 4.4, l.1, molecular basis :**

**Ptashne:** SUPPRESSED

CEq: [lambda[AGS3]\_RI.mig: 1.48–50]

**AGS3, Chapter 4, p.94, l.1, molecular basis :**

**Ptashne:** SUPPRESSED

CEq: [lambda[AGS3]\_RI.mig: 1.110–117, 1.131–140]

**AGS3, Chapter 4, p.94, l.2, molecular basis :**

**Ptashne:** SUPPRESSED

CEq: [lambda[AGS3]\_RI.mig: 1.110–117]

**AGS3, Chapter 4, p.94, l.9, molecular basis :**

**Ptashne:** SUPPRESSED

CEq: [lambda[AGS3]\_RI.mig: 1.48–50, 1.69–86]

**AGS3, Chapter 4, p.94, l.11, molecular basis :**

**Ptashne:** SUPPRESSED

CEq: [lambda[AGS3]\_RI.mig: 1.48–50]

**AGS3, Chapter 4, p.94, l.12, molecular basis :**

**Ptashne:** SUPPRESSED

CEq: [lambda[AGS3]\_RI.mig: 1.10]

**AGS3, Chapter 4, p.94, l.13, molecular basis :**

**Ptashne:** SUPPRESSED

CEq: [lambda[AGS3]\_RI.mig: 1.48–50]

**AGS3, Chapter 4, p.94, l.15, molecular basis :**

**Ptashne:** SUPPRESSED

CEq: [lambda[AGS3]\_RI.mig: 1.125–129, 1.131–140]

**AGS3, Chapter 4, p.94, l.16, molecular basis :**

**Ptashne:** SUPPRESSED

CEq: [lambda[AGS3]\_RI.mig: 1.110–117]

**AGS3, Chapter 4, p.94, l.-7a, molecular basis :**

**Ptashne:** SUPPRESSED

CEq: [lambda[AGS3]\_RI.mig: 1.100]

**AGS3, Chapter 4, p.94, l.-5, molecular basis :**

**Ptashne:** SUPPRESSED

CEq: [lambda[AGS3]\_RI.mig: 1.98, 1.100]

**AGS3, Chapter 4, p.95, l.2, molecular basis :**

**Ptashne:** SUPPRESSED

CEq: [lambda[AGS3]\_RI.mig: 1.17, 1.25, 1.54, 1.55, 1.100]

**AGS3, Chapter 4, p.99, l.26, molecular basis :**

**Ptashne:** SUPPRESSED

CEq: [lambda[AGS3]\_RI.mig: l.105–108]

**AGS3, Chapter 4, p.99, l.-10, molecular basis :**

**Ptashne:** SUPPRESSED

CEq: [lambda[AGS3]\_RI.mig: l.110–117, l.119–120]

**AGS3, Chapter 4, p.102, l.-2, molecular basis :**

**Ptashne:** SUPPRESSED

CEq: [lambda[AGS3]\_RI.mig: l.110–117]

**AGS3, Chapter 4, p.103, l.7, molecular basis :**

**Ptashne:** SUPPRESSED

CEq: [lambda[AGS3]\_RI.mig: l.110–117]

this chapter has 23 quotations with the present filter.

## Chapter 5

**AGS3, Chapter 5, p.109, l.10, molecular basis :**

**Ptashne:** SUPPRESSED

CEq: [lambda[AGS3]\_RI.mig: l.64, l.110–117, l.131–140]

**AGS3, Chapter 5, p.109, l.-6, molecular basis :**

**Ptashne:** SUPPRESSED

CEq: [lambda[AGS3]\_RI.mig: l.63, l.64]

**AGS3, Chapter 5, p.110, l.1, molecular basis :**

**Ptashne:** SUPPRESSED

CEq: [lambda[AGS3]\_RI.mig: l.63, l.64]

**AGS3, Chapter 5, p.110, l.3, molecular basis :**

**Ptashne:** SUPPRESSED

CEq: [lambda[AGS3]\_RI.mig: l.63, l.64]

**AGS3, Chapter 5, p.110, l.-4, molecular basis :**

**Ptashne:** SUPPRESSED

CEq: [lambda[AGS3]\_RI.mig: l.64]

**AGS3, Chapter 5, p.111, l.2, molecular basis :**

**Ptashne:** SUPPRESSED

CEq: [lambda[AGS3]\_RI.mig: l.110–117, l.131–140]

**AGS3, Chapter 5, p.111, l.4, molecular basis :**

**Ptashne:** SUPPRESSED

CEq: [lambda[AGS3]\_RI.mig: l.131–140]

**AGS3, Chapter 5, p.111, Fig.5.2, l.1, molecular basis :**

**Ptashne:** SUPPRESSED

CEq: [lambda[AGS3]\_RI.mig: l.64]

**AGS3, Chapter 5, p.111, Fig.5.3, l.1, molecular basis :**

**Ptashne:** SUPPRESSED

CEq: [lambda[AGS3]\_RI.mig: l.131–140]

**AGS3, Chapter 5, p.112, l.9, molecular basis :**

**Ptashne:** SUPPRESSED

CEq: [lambda[AGS3]\_RI.mig: l.63]

**AGS3, Chapter 5, p.112, Fig.5.4, l.1, molecular basis :**

**Ptashne:** SUPPRESSED

CEq: [lambda[AGS3]\_RI.mig: l.63, l.110–117, l.131–140]

**AGS3, Chapter 5, p.113, Fig.5.5, l.1, molecular basis :**

**Ptashne:** SUPPRESSED

CEq: [lambda[AGS3]\_RI.mig: l.110–117]

**AGS3, Chapter 5, p.114, Fig.5.7, l.1, molecular basis :**

**Ptashne:** SUPPRESSED

CEq: [lambda[AGS3]\_RI.mig: 1.63, 1.64, 1.131–140]

**AGS3, Chapter 5, p.121, box, 1.4, molecular basis :**

**Ptashne:** SUPPRESSED

CEq: [lambda[AGS3]\_RI.mig: 1.64]

**AGS3, Chapter 5, p.122, 1.1, molecular basis :**

**Ptashne:** SUPPRESSED

CEq: [lambda[AGS3]\_RI.mig: 1.110–117]

**AGS3, Chapter 5, p.123, 1.3, molecular basis :**

**Ptashne:** SUPPRESSED

CEq: [lambda[AGS3]\_RI.mig: 1.110–117, 1.131–140]

**AGS3, Chapter 5, p.130, box, 1.-17, molecular basis :**

**Ptashne:** SUPPRESSED

CEq: [lambda[AGS3]\_RI.mig: 1.110–117]

**AGS3, Chapter 5, p.130, box, 1.-7, molecular basis :**

**Ptashne:** SUPPRESSED

CEq: [lambda[AGS3]\_RI.mig: 1.110–117]

**AGS3, Chapter 5, p.132, 1.7, molecular basis :**

**Ptashne:** SUPPRESSED

CEq: [lambda[AGS3]\_RI.mig: 1.100]

**AGS3, Chapter 5, p.136, 1.21, molecular basis :**

**Ptashne:** SUPPRESSED

CEq: [lambda[AGS3]\_RI.mig: 1.105–108]

**this chapter has** 20 quotations with the present filter.

## **Appendix 1**

**AGS3, Appendix 1, p.146, 1.4, molecular basis :**

**Ptashne:** SUPPRESSED

CEq: [lambda[AGS3]\_RI.mig: 1.64, 1.105–108, 1.110–117, 1.131–140]

**this chapter has** 1 quotations with the present filter.

## Appendix 2

this chapter has 0 quotations with the present filter.

## *Quotation tallies*

- motivations: 13 (excluded)
- axioms: 10 (excluded)

---

- semantics: 51 (excluded)
- incidentals: 161 (excluded)

---

- molecular basis: 99 (included)
- population inferences: 9 (excluded)
- causation arguments: 16 (excluded)
- pathway arguments: 29 (excluded)
- cell behaviours: 27 (excluded)

---

- mutations/counterfactuals: 48 (excluded)

---

- superseded: 18 (excluded)

---

- $\Sigma$ : 99 of 481 (total) quotations included

## SD ‘Population inferences’ of [28]

This appendix lists factual statements in [28] we have classified as ‘population inferences’. These issue are related to the MIG keyword `excl`, see Section S2.1, which is part of CEqEA’s macro system that is fully resolved when first parsing a MIG specification, see Section S2.2.

### *Quotation filter*

- motivations: excluded
- axioms: excluded

---

- semantics: excluded
- incidentals: excluded

---

- molecular basis: excluded
- population inferences: included
- causation arguments: excluded
- pathway arguments: excluded
- cell behaviours: excluded

---

- mutations/counterfactuals: excluded

---

- superseded: excluded

## Preface

this chapter has 0 quotations with the present filter.

## Introduction

this chapter has 0 quotations with the present filter.

## Chapter 1

**AGS3, Chapter 1, p.18, Fig.1.12, l.1, population inference**

:

**Ptashne:** SUPPRESSED

CEq: CEqEA infers in the parsing stage that `OR2_C1` is a null-and-void macro declaration, i.e., that it does not happen physiologically, see Section S2.2.3.

**AGS3, Chapter 1, p.20, l.-10, population inference :**

**Ptashne:** SUPPRESSED

CEq: We see in Section S2.1 that `C1` binding to `OR{1,2}` (as well as to `OL{1,2}`, per the latest edition) is excluded by `C1` binding to `OR{1,2,3}` (as well as to `OL{1,2,3}`, per the latest edition). This implies that CEqEA parsing takes `OLR123_C1--` to be `C1.{m,h}` and `OLR12_C1--` to be `C1.1`. As a result, we can, e.g., note that the linearized coextension derivations throughout Section S2.3.2 list `OLR123_C1` but not `OLR12_C1` within the active-edge information whenever the compartment contains `C1.{m,h}`. See also comments for [[28]:21, Fig.1.16:1]/App.SD.

**AGS3, Chapter 1, p.21, Fig.1.16, l.1, population inference**

:

**Ptashne:** SUPPRESSED

CEq: See [[28]:20:-10]/App.SD: `OLR12_C1--` is inferred to be `C1.1` and `OLR123_C1--` is inferred to be `C1.{m,h}`. While literally correct, the word “continues” suggests that the intention of this quotation is superseded in parts, see [[28]:112:9]/App.SC.

this chapter has 3 quotations with the present filter.

## Chapter 2

AGS3, Chapter 2, p.45, l.14, population inference :

**Ptashne:** SUPPRESSED

CEq: The relevant statement to address is that the outlined binding pattern would be artificial: `@OR2_Cro--` refers to `Cro.h` and `@OR3_Cro--` refers to `Cro.{1,h}`.

this chapter has 1 quotations with the present filter.

## Chapter 3

this chapter has 0 quotations with the present filter.

## Chapter 4

AGS3, Chapter 4, p.86, l.12, population inference :

**Ptashne:** SUPPRESSED

CEq: See comments for [[28]:89, Fig.4.20:1]/App.SD.

AGS3, Chapter 4, p.89, Fig.4.20, l.1, population inference  
:

**Ptashne:** SUPPRESSED

CEq: The figure shows the regulatory effect of CI on  $P_R$  and  $P_{RM}$  as a function of concentration: both positive and negative effects are recorded. The concentration axis is discretized into three distinct ranges, characterized by no CI binding, CI binding to  $O_R\{1,2\}$ , and CI binding to  $O_R\{1,2,3\}$ . For the effects issue, see the discussions in Section S2.1 on mediation vs inhibition by CI and on modalities for the two binding configurations for CI. For the discretization issue, note that among the macros involving CI in Section S2.1: `OLR123_CI`, `OLR12_CI`, `OR1_CI`, `OR2_CI`, `OR3_CI`, `OR1and2_CI`, `OR1xor2_CI`, the latter five are inferred by CEqEA parsing to be null-and-void, i.e., to not bind physiologically, see Section S2.2.3. The first two both occur in Section S2.3.

AGS3, Chapter 4, p.91, Table 4.3, l.1, population inference  
:

**Ptashne:** SUPPRESSED

CEq: See comments for [[28]:89, Fig.4.20:1]/App.SD. The two macros that are not null-and-void occur in Section S2.3 with the depicted effects: OLR123\_CI inhibits both  $P_R$  and  $P_{RM}$ ; OLR12\_CI occurs when  $P_{RM}$  is active and  $P_R$  is inhibited.

**AGS3, Chapter 4, p.94, Table 4.5, 1.1, population inference**  
:

**Ptashne:** SUPPRESSED

CEq: See [[28]:93, Fig.4.24:1]/App.SC. The macros that are not null-and-void occur with the prescribed effects in Section S2.3, with no covariance that is Cro-mediated:

- For Cro at only  $O_{R3}$ , we see, e.g.,  $x > [OLR12\_CI, PR\_tr] | \text{--} [Cro.l@OR3]$  and  $\rightarrow [PR\_tr]$  when the compartment contains  $Cro.l$ .
- For Cro at  $O_{R3}$  and  $O_{R1}$  and/or  $O_{R2}$ , we see only neutral or contravariant effects when the compartment contains  $Cro.h$ : inhibition (as above) or concentration drops from protein decay becoming physiological.

this chapter has 4 quotations with the present filter.

## Chapter 5

**AGS3, Chapter 5, p.133, 1.-9, population inference** :

**Ptashne:** SUPPRESSED

CEq: While no details are discussed here, the word “pattern” is an acknowledgment of the need to do population inference in general.

this chapter has 1 quotations with the present filter.

## Appendix 1

this chapter has 0 quotations with the present filter.

## Appendix 2

this chapter has 0 quotations with the present filter.

### *Quotation tallies*

- motivations: 13 (excluded)
- axioms: 10 (excluded)

---

- semantics: 51 (excluded)
- incidentals: 161 (excluded)

---

- molecular basis: 99 (excluded)
- population inferences: 9 (included)
- causation arguments: 16 (excluded)
- pathway arguments: 29 (excluded)
- cell behaviours: 27 (excluded)

---

- mutations/counterfactuals: 48 (excluded)

---

- superseded: 18 (excluded)

---

- $\Sigma$ : 9 of 481 (total) quotations included

## SE ‘Causation arguments’ of [28]

This appendix lists factual statements in [28] we have classified as ‘causation arguments’. They correspond under the CEq construction to particular or synthesized aspects of the regulatory functionality (causations) from which we assemble the cascaded causation diagrams, see Section S1.4.1. We discuss their appearances within the in-situ view, meaning as stipulations within linearized coextension derivations, see Section S2.3, to make sure we provide meaningful context.

### *Quotation filter*

- motivations: excluded
- axioms: excluded

---

- semantics: excluded
- incidentals: excluded

---

- molecular basis: excluded
- population inferences: excluded
- causation arguments: included
- pathway arguments: excluded
- cell behaviours: excluded

---

- mutations/counterfactuals: excluded

---

- superseded: excluded

## Preface

this chapter has 0 quotations with the present filter.

## Introduction

this chapter has 0 quotations with the present filter.

## Chapter 1

**AGS3, Chapter 1, p.12, l.2, causation argument :**

**Ptashne:** SUPPRESSED

CEq: CI occurs in the active ( $\rightarrow$ ) edges in the linearized coextension derivations, e.g., in Section S2.3.2:2/a/ $\beta$ /, as [OLR12\_CI, PRM\_tr], i.e., as a recruiter for  $P_{RM}$  (by cooperative binding to  $O_{\{L,R\}}\{1,2\}$ ) — these occurrences are covariant (not annotated with !), and are revealed to have a positive effect on CI. CI also occurs as a mediator of active edges that are contravariant, e.g., ![OLR123\_CI], and as the recurrent cause behind blocked ( $\times$ ) edges, e.g., [PR\_tr] |-- [CI.m!@[OLR123]]. These occurrences are as strong inhibitors/with contravariant effects/annotated with !: they are revealed to have explicitly negative effects on CI and Cro, as opposed to merely ensuring, say, the absence of any positive effects.

**AGS3, Chapter 1, p.13, Fig.1.3, l.1, causation argument :**

**Ptashne:** SUPPRESSED

CEq: See the occurrences of [PR\_tr] |-- [CI.{1,m}!@[OLR12, OLR123]] in the linearized coextension derivations of Section S2.3.2:2/b/iii/, and note how they occur both before and after super-infection, i.e., how no *cro* is transcribed at any point. See also the NB! in Section S2.3.2:2/b/iii/ for an explicit distinction between pre-existing and super-infecting genes.

**AGS3, Chapter 1, p.15, l.8, causation argument :**

**Ptashne:** SUPPRESSED

CEq: See the effects on CI of the interactions involving  $P_{RM}$  in the linearized coextension derivations, e.g., in Section S2.3.2:2/a/ $\beta$ /. See also the statement of Section S2.3.1:2/a/ $\alpha$ /.

**AGS3, Chapter 1, p.20, l.4, causation argument :**

**Ptashne:** SUPPRESSED

CEq: See the effects of the interactions involving PR\_tr, PRM\_tr, and OLR12\_CI/CI.1!@[OLR12] in the linearized coextension derivations, e.g., in Section S2.3.2:2/a/ $\beta$ /:  $\rightarrow$  [OLR12\_CI, PRM\_tr] and  $x >$  [PR\_tr] |-- [CI.1!@[OLR12]].

**AGS3, Chapter 1, p.22, l.1, causation argument :**

**Ptashne:** SUPPRESSED

CEq: See the effects of the occurrences of OLR12\_CI and CI.1 in the linearized coextension derivations, e.g., in Section S2.3.2:2/a/ $\beta$ /.

**AGS3, Chapter 1, p.23, Fig.1.19, l.1, causation argument :**

**Ptashne:** SUPPRESSED

CEq: See the effects of the juxtaposition of OLR12\_CI with PRM\_tr and PR\_tr, respectively, in the linearized coextension derivations, e.g., of Section S2.3.2:2/a/ $\beta$ /.

**AGS3, Chapter 1, p.25, l.3a, causation argument :**

**Ptashne:** SUPPRESSED

CEq: The linearized coextension derivations in Section S2.3.2 contain numerous listings, e.g., of  $x >$  [OLR12\_CI, PRM\_tr] |-- [Cro.1@[OR3]], meaning prevention of (physiological) CI synthesis (but see article:Retrodiction (III)).

**AGS3, Chapter 1, p.25, l.7, causation argument :**

**Ptashne:** SUPPRESSED

CEq: See, e.g., the penultimate step in the linearized coextension derivations in Section S2.3.2:2/c/, which lists the implied contravariant effect on/physiological decay of Cro:  $\rightarrow$  ![OR2\_Cro, OR1\_Cro].

**AGS3, Chapter 1, p.28, l.10, causation argument :**

**Ptashne:** SUPPRESSED

CEq: There are occurrences of OLR123\_CI in the active edges in the linearized coextension derivations, e.g., in Section S2.3.2:2/a/ $\beta$ /; they are associated with the referenced contravariant/decaying effect on CI:  $\rightarrow$  ![OLR123\_CI].

this chapter has 9 quotations with the present filter.

## Chapter 2

this chapter has 0 quotations with the present filter.

## Chapter 3

AGS3, Chapter 3, p.52, l.5, causation argument :

**Ptashne:** SUPPRESSED

CEq: See the NB! in the comments for [[28]:50:6]/App.SF for why more subtlety almost certainly is required in the discussion of CII and the role it may have at the different stages in different infection scenarios. See also the details of Section S2.3.2:1/ for the variation suggested here, and see article:Retrodiction (I) for further specifics. Several of the listed actions and interactions are not further detailed in [28], and are not covered here.

- For Very early, see the opening details of Section S2.3.2:1/ and the statement of Section S2.3.1:3/a/ $\alpha$ /.
- For Early lytic, see the details of Section S2.3.2:1/CII.\_ and Section S2.3.2:3/a/ $\alpha$ /. For Early lysogenic, see the details of Section S2.3.2:1/CII.h and Section S2.3.2:2/a/ $\alpha$ /, with the effects of CI becoming active discussed in Section S2.3.2:0/.
- For Late lytic, see the details of Section S2.3.2:3/a/ $\beta$ /. However, see also article:Retrodictions for further particulars of the role of Cro.
- For Late lysogenic, see (the statement of Section S2.3.1:2/a/ $\alpha$ / and) the details of Section S2.3.2:2/a/ $\beta$ /.

this chapter has 1 quotations with the present filter.

## Chapter 4

AGS3, Chapter 4, p.68, l.-8, causation argument :

**Ptashne:** SUPPRESSED

CEq: See the occurrences and effects of CI.{1,m} in the linearized coextension derivations, e.g., in Section S2.3.2:2/a/ $\beta$ /.

AGS3, Chapter 4, p.68, l.-7, causation argument :

**Ptashne:** SUPPRESSED

CEq: See the occurrences and effects of CII.h in the linearized coextension derivations, e.g., in Section S2.3.2:1/, and note that Section S2.3.2:2/a/ $\beta$ / holds also for the case of CII.\_.

**AGS3, Chapter 4, p.87, l.1, causation argument :**

**Ptashne:** SUPPRESSED

CEq: See the occurrences and effects of  $\text{CI}.\{1,\mathfrak{m}\}$  in the linearized coextension derivations, e.g., in Section S2.3.2:2/a/ $\beta$ /.

**AGS3, Chapter 4, p.87, l.-13, causation argument :**

**Ptashne:** SUPPRESSED

CEq: See the occurrences and effects of  $\text{CI}.\{1,\mathfrak{m}\}$  in the linearized coextension derivations, e.g., in Section S2.3.2:2/a/ $\beta$ /.

**AGS3, Chapter 4, p.91, l.4, causation argument :**

**Ptashne:** SUPPRESSED

CEq: See comments for [[28]:86:12]/App.SD: among `OLR123_CI`, `OLR12_CI`, `OR1_CI`, `OR2_CI`, `OR3_CI`, `OR1and2_CI`, `OR1xor2_CI` in Section S2.1 only the former two are not null-and-void, see Section S2.2.3, and they both occur throughout Section S2.3, with the prescribed effects.

**AGS3, Chapter 4, p.103, l.6, causation argument :**

**Ptashne:** SUPPRESSED

CEq: See the occurrences and the effect of `OLR123_CI` in the linearized coextension derivations, e.g., in Section S2.3.2:2/a/ $\beta$ /, and note that `OLR123_CI` does not occur with `PRM_tr`.

this chapter has 6 quotations with the present filter.

## Chapter 5

this chapter has 0 quotations with the present filter.

## Appendix 1

this chapter has 0 quotations with the present filter.

## Appendix 2

this chapter has 0 quotations with the present filter.

### *Quotation tallies*

- motivations: 13 (excluded)
- axioms: 10 (excluded)

---

- semantics: 51 (excluded)
- incidentals: 161 (excluded)

---

- molecular basis: 99 (excluded)
- population inferences: 9 (excluded)
- causation arguments: 16 (included)
- pathway arguments: 29 (excluded)
- cell behaviours: 27 (excluded)

---

- mutations/counterfactuals: 48 (excluded)

---

- superseded: 18 (excluded)

---

- $\Sigma$ : 16 of 481 (total) quotations included

## SF ‘Pathway arguments’ of [28]

This appendix lists factual statements in [28] we have classified as ‘pathway arguments’. They correspond to human-centred highlights of our coextension derivations. See also Figure 4.

### *Quotation filter*

- motivations: excluded
- axioms: excluded

---

- semantics: excluded
- incidentals: excluded

---

- molecular basis: excluded
- population inferences: excluded
- causation arguments: excluded
- pathway arguments: included
- cell behaviours: excluded

---

- mutations/counterfactuals: excluded

---

- superseded: excluded

## Preface

this chapter has 0 quotations with the present filter.

## Introduction

AGS3, Introduction, p.9, l.-8, pathway argument :

**Ptashne:** SUPPRESSED

CEq: See the linearized coextension derivations and discussion in Section S2.3.2:1/, and note that not all “first steps” have their molecular underpinnings covered in [28]. The parts that are not covered in [28] are not covered here, either. Note, also, that the “decision” point is diffuse: “sensing” amounts to whether CII reaches high concentration, in which case the lysogenic cycle invariably is established, and, else, a lytic attack destroys the host. With CII at high, both pathways are pursued in parallel from the outset, which is the Section S2.3 version of “identical first steps”, and lysogeny results further to Section S2.3.2:0/.

this chapter has 1 quotations with the present filter.

## Chapter 1

AGS3, Chapter 1, p.11, l.23, pathway argument :

**Ptashne:** SUPPRESSED

CEq: See the linearized coextension derivations and discussions in Section S2.3.2:2/c/, and note the progression of UV\_irr, SOS, CI dropping to non-physiological concentration, Cro becoming physiological, and, finally, <expired>.

AGS3, Chapter 1, p.12, l.1, pathway argument :

**Ptashne:** SUPPRESSED

CEq: See the linearized coextension derivations and discussions in Section S2.3.2:2/a/ $\beta$ /, and note that only the  $P_{RM}$  promoter (for *cI*-transcription) occurs among the active (->) edges in the linearized coextension derivations: PRM\_tr.

AGS3, Chapter 1, p.12, l.-11, pathway argument :

**Ptashne:** SUPPRESSED

CEq: See the linearized coextension derivations and discussions in Section S2.3.2:2/c/ and the statement of Section S2.3.1:3/a/ $\alpha$ /. Note the progression of UV\_irr, SOS, CI dropping to non-physiological concentration, Cro becoming physiological, and <expired> in Section S2.3.2:2/c/.

### AGS3, Chapter 1, p.15, l.-10, pathway argument :

**Ptashne:** SUPPRESSED

CEq: This statement may be understood in two different senses: at the level of individual molecules or whether the considered bindings may be physiological at the same time. We surmise that the statement is not, in fact, correct in the former sense. For the latter sense, note that no linearized coextension derivation in Section S2.3 lists PR\_tr and PRM\_tr as being active at the same time, i.e., nowhere do we see  $\rightarrow$  [PR\_tr] ; [OLR12\_CI, PRM\_tr], or similar. See also Section S2.3.2:{2,3}/a/ $\beta$ /.

### AGS3, Chapter 1, p.15, Fig.1.5, l.2, pathway argument :

**Ptashne:** SUPPRESSED

CEq: This statement may be understood in two different senses: at the level of individual molecules or whether the considered bindings may be physiological at the same time. We surmise that the statement is not, in fact, correct in the former sense. For the latter sense, note that no linearized coextension derivation in Section S2.3.2 lists PR\_tr as active, i.e., nowhere do we see  $\rightarrow$  [PR\_tr], or similar, unless the compartment contains CI.0. We do, however, see, e.g.,  $\rightarrow$  [OLR12\_CI, PRM\_tr] with CI.1 in the compartment. See also Section S2.3.2:{2,3}/a/ $\beta$ /.

### AGS3, Chapter 1, p.15, Fig.1.5, l.3, pathway argument :

**Ptashne:** SUPPRESSED

CEq: This statement may be understood in two different senses: at the level of individual molecules or whether the considered bindings may be physiological at the same time. We surmise that the statement is not, in fact, correct in the former sense. For the latter sense, note that no linearized coextension derivation in Section S2.3.2 lists PRM\_tr as active, i.e., nowhere do we see  $\rightarrow$  [OLR12\_CI, PRM\_tr], or similar, unless the compartment contains Cro.0. We do, however, see, e.g.,  $\rightarrow$  [PR\_tr] with Cro.1 in the compartment. See also Section S2.3.2:{2,3}/a/ $\beta$ /.

### AGS3, Chapter 1, p.20, l.2, pathway argument :

**Ptashne:** SUPPRESSED

CEq: We note that in the linearized coextension derivations in Section S2.3.2 there is no compartment containing `CI.l`, `CI.m`, or `CI.h` that does not also list `OLR12_CI` or `OLR123_CI` somewhere within the associated active or blocked edges.

**AGS3, Chapter 1, p.20, l.3a, pathway argument :**

**Ptashne:** SUPPRESSED

CEq: See comments for [[28]:20, Fig.1.15:1]/App.SF: this statement may or may not be correct.

**AGS3, Chapter 1, p.20, Fig.1.15, l.1, pathway argument :**

**Ptashne:** SUPPRESSED

CEq: There are 28 occurrences of `OLR12_CI` throughout Section S2.3.2:2/ and sub-items, and 18 of `OLR123_CI`. There are no occurrences of other `_CI` macros.

**AGS3, Chapter 1, p.22, l.4, pathway argument :**

**Ptashne:** SUPPRESSED

CEq: See the linearized coextension derivations and discussions in Section S2.3.2:2/a/ $\beta$ /. See also the statement of Section S2.3.1:2/b/i/.

**AGS3, Chapter 1, p.23, l.1, pathway argument :**

**Ptashne:** SUPPRESSED

CEq: See our treatment of state interpolation in Section S1.5. relative to Section S2.3.2:2/a/ $\beta$ /. See also the statement of Section S2.3.1:2/b/i/.

**AGS3, Chapter 1, p.23, l.4, pathway argument :**

**Ptashne:** SUPPRESSED

CEq: Note that `OLR12_CI` or `OLR123_CI` occur in each collection of active edges: `->`, in the linearized coextension derivations in Section S2.3.2:2/a/ $\beta$ /.

**AGS3, Chapter 1, p.24, l.-7, pathway argument :**

**Ptashne:** SUPPRESSED

CEq: See Figure 4.

**AGS3, Chapter 1, p.25, l.-2b, pathway argument :**

**Ptashne:** SUPPRESSED

CEq: See the discussions in Section S2.3.2:3/a/ $\beta$ /. See also the latter parts of the linearized coextension derivations in Section S2.3.2:2/c/.

**AGS3, Chapter 1, p.27, l.19, pathway argument :**

**Ptashne:** SUPPRESSED

CEq: See the linearized coextension derivations and discussions in Section S2.3.2:2/c/, and note that there is no mention of PRM\_tr after CI has reached zero concentration, CI.0.

**AGS3, Chapter 1, p.27, l.-7, pathway argument :**

**Ptashne:** SUPPRESSED

CEq: See the pivotal nature of the [Cro.0, RecA.\*] + [CI.0, ...]/[CI.0, Cro.0, RecA.\*] compartment in the linearized coextension derivations of Section S2.3.2:2/c/: prior to it CI is physiological, Cro is not; vice versa after.

this chapter has 16 quotations with the present filter.

## Chapter 2

this chapter has 0 quotations with the present filter.

## Chapter 3

**AGS3, Chapter 3, p.47, l.6, pathway argument :**

**Ptashne:** SUPPRESSED

CEq: See the linearized coextension derivations and discussions in Section S2.3.2:2/a/ $\beta$ / and note in particular that Cro remains at zero concentration, Cro.0, due to CI inhibition of *cro*-transcription from P<sub>R</sub>, e.g., x> [PR\_tr] |-- [CI.1!@[OLR12]]. See also the statement of Section S2.3.1:2/b/i/.

**AGS3, Chapter 3, p.47, l.-9, pathway argument :**

**Ptashne:** SUPPRESSED

CEq: Further to Section S2.3.2:1/CII.~, see the linearized coextension derivations and discussions in Section S2.3.2:3/a/ $\beta$ /, and see article:Retrodiction (III) for the precise situation with repressor. (Note that the molecular underpinnings of the referenced cell-level effects are not presented in [28], and are not discussed here, either.)

**AGS3, Chapter 3, p.47, l.-4, pathway argument :**

**Ptashne:** SUPPRESSED

CEq: Further to Section S2.3.2:1/CII.h, see the linearized coextension derivations and discussions in Section S2.3.2:2/a/ $\beta$ /. See also article:Retrodiction (I) for further specifics. Note that the molecular underpinnings of the referenced cell-level effects are not presented in [28], and are not discussed here, either.

**AGS3, Chapter 3, p.50, l.6, pathway argument :**

**Ptashne:** SUPPRESSED

CEq: See the linearized coextension derivations and discussions of Section S2.3.2:1/ (with explication for the Late stage provided in Section S2.3.2:3/a/ $\alpha$ / and Section S2.3.2:2/a/{ $\alpha,\beta$ }/) — not all molecule changes are justified from basic interactions in [28]; these are not covered here, either. For an example that is covered, note that the linearized coextension derivations shown in Section S2.3.2:3/a/ $\alpha$ / reveal that *cro* is not transcribed in the Late lytic stage/the penultimate step before the host expires and that, as a result, the concentration of Cro drops: ! [OR2-Cro, OR1-Cro]. See also article:Retrodiction (I) for further specifics.

NB! There appears to be a subtlety in this quotation: the Very early description seems to pertain to a first infection while Late lysogeny seemingly requires several reasonably-simultaneous infections to have taken place for sufficient CII to have built up to allow that protein to mediate *P<sub>RE</sub>*-transcription. In Section S2.3.2, the distinction between the different levels of CII concentration is made by an environment toggle because [28] does not give sufficient details for how the change is effected.

**AGS3, Chapter 3, p.57, l.22, pathway argument :**

**Ptashne:** SUPPRESSED

CEq: See the linearized coextension derivations and discussions in Section S2.3.2:1/. See also article:Retrodiction (I) for further specifics.

**AGS3, Chapter 3, p.60, l.-1, pathway argument :**

**Ptashne:** SUPPRESSED

CEq: See the linearized coextension derivations and discussions in Section S2.3.2:2/c/.

**AGS3, Chapter 3, p.61, l.10, pathway argument :**

**Ptashne:** SUPPRESSED

CEq: See the linearized coextension derivations and discussions in Section S2.3.2:2/c/.

**AGS3, Chapter 3, p.64, l.8, pathway argument :**

**Ptashne:** SUPPRESSED

CEq: CEqEA provides two principled mechanisms for external signals: toggles (see Section S1.4.1) and externalization (see Section S2.4). CEqEA's ability to do sub-system analysis can also often be used, by including or excluding nodes with particular types of content. See the particulars at Section S2.3.2:2/c/ and Section S2.3.2:1/ for the discussed examples.

**this chapter has** 8 quotations with the present filter.

## Chapter 4

**AGS3, Chapter 4, p.87, l.-9, pathway argument :**

**Ptashne:** SUPPRESSED

CEq: See our discussion of state interpolation in Section S1.5.

**AGS3, Chapter 4, p.94, l.-7b, pathway argument :**

**Ptashne:** SUPPRESSED

CEq: See the linearized coextension derivations and discussions in Section S2.3.2:2/c/, and note the details also noted for [[28]:11:23]/App.SF: the progression of UV\_irr, SOS, CI dropping to non-physiological concentration, Cro becoming physiological, and, finally, <expired>.

**this chapter has** 2 quotations with the present filter.

## Chapter 5

**AGS3, Chapter 5, p.111, Fig.5.3, l.-3, pathway argument :**

**Ptashne:** SUPPRESSED

CEq: The figure shows that  $P_R$  is maximally repressed in lysogens. While we do not establish maximality, the interpolation discussion in Section S1.5 is relevant.

**AGS3, Chapter 5, p.112, l.17, pathway argument :**

**Ptashne:** SUPPRESSED

CEq: Section S2.3.2:2/a/ $\beta$ / shows an otherwise-unimpeded alternation of CI's concentration between low and high. See also state interpolation in Section S1.5.

**this chapter has** 2 quotations with the present filter.

## Appendix 1

**this chapter has** 0 quotations with the present filter.

## Appendix 2

**this chapter has** 0 quotations with the present filter.

### *Quotation tallies*

- motivations: 13 (excluded)
- axioms: 10 (excluded)

---

- semantics: 51 (excluded)
- incidentals: 161 (excluded)

---

- molecular basis: 99 (excluded)
- population inferences: 9 (excluded)
- causation arguments: 16 (excluded)
- pathway arguments: 29 (included)
- cell behaviours: 27 (excluded)

---

- mutations/counterfactuals: 48 (excluded)

---

- superseded: 18 (excluded)

---

- $\Sigma$ : 29 of 481 (total) quotations included

## SG ‘Cell behaviours’ of [28]

This appendix lists factual statements in [28] we have classified as ‘cell behaviours’. They are structured according to observations of cell cultures but, as we show below, can also be composed (in various ad-hoc ways) from our ‘pathway properties’, see Section S2.3.

### *Quotation filter*

- motivations: excluded
- axioms: excluded

---

- semantics: excluded
- incidentals: excluded

---

- molecular basis: excluded
- population inferences: excluded
- causation arguments: excluded
- pathway arguments: excluded
- cell behaviours: included

---

- mutations/counterfactuals: excluded

---

- superseded: excluded

## Preface

this chapter has 0 quotations with the present filter.

## Introduction

**AGS3, Introduction, p.1, l.3, cell behaviour :**

**Ptashne:** SUPPRESSED

CEq: The individuals in question are lysogens, i.e., *E. coli* with  $\lambda$ -prophages: see the statements of Section S2.3.1:2/c/ and Section S2.3.1:3/a/ $\gamma$ /, as well as of Section S2.3.1:2/.

**AGS3, Introduction, p.1, l.7, cell behaviour :**

**Ptashne:** SUPPRESSED

CEq: See the statement of Section S2.3.1:1/, as well as those of Section S2.3.1:3/ and Section S2.3.1:2/.

**AGS3, Introduction, p.1, l.13, cell behaviour :**

**Ptashne:** SUPPRESSED

CEq: See the statement of Section S2.3.1:2/c/, and note that we establish the property by molecular reasoning based on the cascading of conditional population changes, meaning the stepwise turning on and off of genes by specific gene products.

**AGS3, Introduction, p.9, l.1, cell behaviour :**

**Ptashne:** SUPPRESSED

CEq: See the statement of Section S2.3.1:2/c/, and note that we elicit the behaviour of a “genetic switch” based solely on interactions of the (molecular) components in question.

this chapter has 4 quotations with the present filter.

## Chapter 1

**AGS3, Chapter 1, p.11, l.8, cell behaviour :**

**Ptashne:** SUPPRESSED

CEq: See the statement of Section S2.3.1:1/ as well as Figure 7 for CE-qEA's automatic generation of the referenced figure as the approximate sequentialization of all Section S2.3 behaviours, specifically an approximation of the  $\lambda$  *synchrotype* (a concept we introduce to complement genotype and phenotype), see Section S2.4.

**AGS3, Chapter 1, p.11, l.9, cell behaviour :**

**Ptashne:** SUPPRESSED

CEq: See the statements of Section S2.3.1:1/, Section S2.3.1:3/a/, and Section S2.3.1:3/a/ $\gamma$ /.

**AGS3, Chapter 1, p.11, l.14, cell behaviour :**

**Ptashne:** SUPPRESSED

CEq: See the statements of Section S2.3.1:1/, Section S2.3.1:2/, Section S2.3.1:2/a/ $\beta$ /, and Section S2.3.1:2/b/+Section S2.3.1:2/b/i/.

**AGS3, Chapter 1, p.11, l.21, cell behaviour :**

**Ptashne:** SUPPRESSED

CEq: See the statements of Section S2.3.1:2/c/, Section S2.3.1:3/a/ $\alpha$ /, and Section S2.3.1:3/a/ $\gamma$ / and note the discussion of how the *cro* gene is turned on in the relevant parts of Section S2.3.2.

**AGS3, Chapter 1, p.12, l.10a, cell behaviour :**

**Ptashne:** SUPPRESSED

CEq: See the statement of Section S2.3.1:3/d/, as well as those of Section S2.3.1:0/ and Section S2.3.1:2/b/iii/.

**AGS3, Chapter 1, p.12, l.10b, cell behaviour :**

**Ptashne:** SUPPRESSED

CEq: See the statement of Section S2.3.1:2/b/iii/.

**AGS3, Chapter 1, p.12, l.-5, cell behaviour :**

**Ptashne:** SUPPRESSED

CEq: See the statements of Section S2.3.1:2/a/ $\beta$ / and Section S2.3.1:3/a/ $\beta$ /.

**AGS3, Chapter 1, p.13, Fig.1.2, l.1, cell behaviour :**

**Ptashne:** SUPPRESSED

CEq: See the statements of Section S2.3.1:1/ and Section S2.3.1:2/c/.

**AGS3, Chapter 1, p.22, l.2, cell behaviour :**

**Ptashne:** SUPPRESSED

CEq: See the statements of Section S2.3.1:2/a/ $\beta$ / and Section S2.3.1:2/b/i/.

**AGS3, Chapter 1, p.23, l.6, cell behaviour :**

**Ptashne:** SUPPRESSED

CEq: See the statements of Section S2.3.1:2/, Section S2.3.1:2/a/ $\beta$ /, and Section S2.3.1:2/b/, along with the specifics in Section S2.3.2:2/b/.

this chapter has 10 quotations with the present filter.

## Chapter 2

this chapter has 0 quotations with the present filter.

## Chapter 3

**AGS3, Chapter 3, p.47, l.11, cell behaviour :**

**Ptashne:** SUPPRESSED

CEq: See the statements of Section S2.3.1:2/ and Section S2.3.1:2/c/, and the linearized coextension derivations in Section S2.3.2:2/c/.

**AGS3, Chapter 3, p.48, l.1, cell behaviour :**

**Ptashne:** SUPPRESSED

CEq: See the statement of Section S2.3.1:1/, with the specifics of the decision clarified in the attendant argumentation in Section S2.3.2:1/ and the environment dependency reflected in the automatic inclusion of the CII toggles. See also article:Retrodiction (I) for further specifics.

**AGS3, Chapter 3, p.48, l.7, cell behaviour :**

**Ptashne:** SUPPRESSED

CEq: Indeed, see Section S2.3.2:. See also Section S2.4.

**AGS3, Chapter 3, p.56, l.-3, cell behaviour :**

**Ptashne:** SUPPRESSED

CEq: See the statements of Section S2.3.1:1/ and Section S2.3.1:2/a/ $\alpha$ /.

**AGS3, Chapter 3, p.56, l.-1b, cell behaviour :**

**Ptashne:** SUPPRESSED

CEq: See the statement of Section S2.3.1:1/.

**AGS3, Chapter 3, p.62, l.-1, cell behaviour :**

**Ptashne:** SUPPRESSED

CEq: See the statement of Section S2.3.1:3/b/ii/ and article:Retrodiction (III).

**AGS3, Chapter 3, p.64, l.1, cell behaviour :**

**Ptashne:** SUPPRESSED

CEq: See the statements of Section S2.3.1:2/c/ and Section S2.3.1:1/. See comments for [[28]:64:8]/App.SF for how CEqEA handles these types of signals, including the listed specifics.

**AGS3, Chapter 3, p.64, l.17, cell behaviour :**

**Ptashne:** SUPPRESSED

CEq: See the statements of Section S2.3.1:2/, along with the specifics of the sub-items in Section S2.3.2:2/. See also article:Retrodiction (II).

**this chapter has** 8 quotations with the present filter.

## Chapter 4

**AGS3, Chapter 4, p.67, l.-1, cell behaviour :**

**Ptashne:** SUPPRESSED

CEq: See the statements of Section S2.3.1:2/b/iii/ and Section S2.3.1:2/c/.

**this chapter has** 1 quotations with the present filter.

## Chapter 5

**AGS3, Chapter 5, p.133, l.15, cell behaviour :**

**Ptashne:** SUPPRESSED

CEq: See the statements of Section S2.3.1:2/, Section S2.3.1:2/c/, and Section S2.3.1:3/.

**AGS3, Chapter 5, p.133, l.17, cell behaviour :**

**Ptashne:** SUPPRESSED

CEq: See the statements of Section S2.3.1:2/b/{i,ii,iii}/ and Section S2.3.1:2/c/.

**AGS3, Chapter 5, p.136, l.15, cell behaviour :**

**Ptashne:** SUPPRESSED

CEq: See the statements of Section S2.3.1:3/a/ $\beta$ / and Section S2.3.1:2/a/ $\beta$ /.

**AGS3, Chapter 5, p.136, l.-7, cell behaviour :**

**Ptashne:** SUPPRESSED

CEq: See the statement of Section S2.3.1:1/.

**this chapter has** 4 quotations with the present filter.

## Appendix 1

**this chapter has** 0 quotations with the present filter.

## Appendix 2

**this chapter has** 0 quotations with the present filter.

### *Quotation tallies*

- motivations: 13 (excluded)
- axioms: 10 (excluded)

---

- semantics: 51 (excluded)
- incidentals: 161 (excluded)

---

- molecular basis: 99 (excluded)
- population inferences: 9 (excluded)
- causation arguments: 16 (excluded)
- pathway arguments: 29 (excluded)
- cell behaviours: 27 (included)

---

- mutations/counterfactuals: 48 (excluded)

---

- superseded: 18 (excluded)

---

- $\Sigma$ : 27 of 481 (total) quotations included

## SH ‘Superseded issues’ of [28]

This appendix lists factual statements carried over from previous editions of [28] that are ‘superseded’ by new discoveries according to additions to the most recent edition.

The superseded statements revolve around  $O_{\{L,R\}}3$ . The sites are conserved and the earlier editions surmised that this was because  $O_R3$  was subject to important action by Cro, see Appendix SH:121:1. The new the monograph edition [28] is motivated by the discovery that  $O_{\{L,R\}}3$  are the sites of long-distance CI cooperativity, see Appendix SC:112:9. The added statements in [28] do not completely repudiate the earlier Cro action at  $O_R3$ , see Appendix SH:121:-4. We show that Cro action at  $O_R3$  is not a part of the remainder of the reasoning and stress that any such action is contradicted by our pivotal Section S2.3:0/, whose ‘molecular basis’ and coextension reasoning appear beyond reproach: known properties would fail without the new property while Section S2.3 is an internally-correct model of  $\lambda$  that overwhelmingly has been confirmed to be externally correct, see Appendix SA:xiv:9, and does not need Cro binding to trigger the switch. See article:Retrodictions (especially article:Retrodiction (I)) for discussion and Appendix SH:24:-5 for what appears to be corroboration.

We comment only at principal quotations for distinct aspects. This ensures that the commenting accurately reflects the negative information we wish to convey.

### *Quotation filter*

- motivations: excluded
- axioms: excluded

---

- semantics: excluded
- incidentals: excluded

---

- molecular basis: excluded
- population inferences: excluded
- causation arguments: excluded
- pathway arguments: excluded
- cell behaviours: excluded

---

- mutations/counterfactuals: excluded

---

- superseded: included

## Preface

this chapter has 0 quotations with the present filter.

## Introduction

this chapter has 0 quotations with the present filter.

## Chapter 1

**AGS3, Chapter 1, p.12, l.-10, superseded :**

**Ptashne:** SUPPRESSED

CEq: The fact that **Cro** binds the same operator sites as **CI** is discussed in Section S2.1. It is not clear what is meant by “opposite physiological effects”: see article:Retrodiction (II) for the higher levels of possible meaning, where the statement almost certainly is not correct.

**AGS3, Chapter 1, p.15, l.7, superseded :**

**Ptashne:** SUPPRESSED

**AGS3, Chapter 1, p.20, l.-8, superseded :**

**Ptashne:** SUPPRESSED

CEq: The newly discovered cooperativity across  $O_{\{L,R\}}3$  changes **CI**’s effective affinity for  $O_R3$ .

**AGS3, Chapter 1, p.21, l.7a, superseded :**

**Ptashne:** SUPPRESSED

**AGS3, Chapter 1, p.24, l.-5, superseded :**

**Ptashne:** SUPPRESSED

CEq: This quotation is missing from later printing of [28].

**AGS3, Chapter 1, p.25, l.2a, superseded :**

**Ptashne:** SUPPRESSED

**AGS3, Chapter 1, p.25, l.3b, superseded :**

**Ptashne:** SUPPRESSED

**AGS3, Chapter 1, p.25, l.-2a, superseded :**

**Ptashne:** SUPPRESSED

**AGS3, Chapter 1, p.27, l.5, superseded :**

**Ptashne:** SUPPRESSED

this chapter has 9 quotations with the present filter.

## **Chapter 2**

this chapter has 0 quotations with the present filter.

## **Chapter 3**

this chapter has 0 quotations with the present filter.

## **Chapter 4**

**AGS3, Chapter 4, p.85, l.-6, superseded :**

**Ptashne:** SUPPRESSED

**AGS3, Chapter 4, p.86, l.13, superseded :**

**Ptashne:** SUPPRESSED

**AGS3, Chapter 4, p.92, l.1b, superseded :**

**Ptashne:** SUPPRESSED

**AGS3, Chapter 4, p.95, l.14, superseded :**

**Ptashne:** SUPPRESSED

**AGS3, Chapter 4, p.95, l.19, superseded :**

**Ptashne:** SUPPRESSED

**AGS3, Chapter 4, p.95, l.24, superseded :**

**Ptashne:** SUPPRESSED

CEq: The switch appears efficient in practice, which could be explained by strong inhibition. Cro, however, inhibits but does not strongly inhibit *cI*-transcription from  $O_R3$  at the considered (lower) concentrations, meaning the effect on CI will not be lower concentration. The switch efficiency instead appears to be the result of the highly-cooperative CI-binding across  $O_{\{L,R\}}\{1,2\}$  being abandoned at a time when free CI concentration is effectively zero, following host-based proteolysis, see article:Retrodictions.

this chapter has 6 quotations with the present filter.

## Chapter 5

AGS3, Chapter 5, p.110, l.6, superseded :

Ptashne: SUPPRESSED

CEq: “The moment” refers to the specific place in [28]. See article:Retrodictions and [[28]:112:1], [[28]:112:9]/App.SC, [[28]:112:20] for “the role”.

AGS3, Chapter 5, p.121, l.1, superseded :

Ptashne: SUPPRESSED

AGS3, Chapter 5, p.121, l.-4, superseded :

Ptashne: SUPPRESSED

CEq: Cro binding to  $O_R3$  to trigger the transition to lytic growth is explicitly excluded from our formal model, see article:Retrodictions.

this chapter has 3 quotations with the present filter.

## Appendix 1

this chapter has 0 quotations with the present filter.

## Appendix 2

this chapter has 0 quotations with the present filter.

### *Quotation tallies*

- motivations: 13 (excluded)
- axioms: 10 (excluded)

---

- semantics: 51 (excluded)
- incidentals: 161 (excluded)

---

- molecular basis: 99 (excluded)
- population inferences: 9 (excluded)
- causation arguments: 16 (excluded)
- pathway arguments: 29 (excluded)
- cell behaviours: 27 (excluded)

---

- mutations/counterfactuals: 48 (excluded)

---

- superseded: 18 (included)

---

- $\Sigma$ : 18 of 481 (total) quotations included
